# Supplementary material for: A New Graph Grammar Formalism for Robust Syntactic Pattern Recognition
Source: arXiv:2504.15975 source file (2025-04-24)
Supplement: Supplementary file 1 [file supplement.tex]

% This is the main file. It is in plain TeX.

\input My.sty
\elevenpoint  % use Postscript New Century (pncr) fonts

\def\title#1{\centerline{\bf #1}}
\def\author#1{\centerline{#1}}
\def\address#1{\centerline{#1}}
\def\thanks#1{\f{#1}}

\title{SUPPLEMENT}

\bigskip

\title{Mathematical Theory of Networks for Syntactic Pattern Recognition}

\bigskip

\author{Peter Fletcher}
\address{School of Computer Science and Mathematics,}
\address{Keele University,}
\address{Keele,}
\address{Staffordshire, ST5 2BG, U.K.}
\address{Email: p.fletcher@keele.ac.uk}

\bigskip

\thanks{This research did not receive any specific grant from funding agencies 
in the public, commercial, or not-for-profit sectors.}

\bigskip

\thanks{There are no conflicts of interest.}

\subhead{Abstract}
This is a mathematical supplement to the paper \ic{A New Graph Grammar
Formalism for Robust Syntactic Pattern Recognition}, available at
https://doi.org/10.48550/arXiv.2504.15975. It provides the full mathematical
theory and complete proofs.

\vfill\supereject
\head{Table of Contents}

\vskip1cm

\def\conline#1#2{\par\medpagebreak\noindent#1 \dotfill\,#2\hskip20pt\null}
\def\subconline#1#2{\par#1 \dotfill\,#2\hskip20pt\null}

\conline{1. Introduction}{4}

\conline{2. Functions and Relations}{6}
\subconline{2.1 Introduction}{6}
\subconline{2.2 Basic definitions and theorems}{6}
\subconline{2.3 Acyclic and connected relations}{11}
\subconline{2.4 Minimal relations relative to a function}{18}

\conline{3. Networks and Homomorphisms}{20}
\subconline{3.1 Introduction}{20}
\subconline{3.2 Definition of network and homomorphism}{20}
\subconline{3.3 Minimal relations relative to a network}{23}
\subconline{3.4 Semi-definite and definite networks}{25}
\subconline{3.5 Properties preserved by homomorphisms}{28}
\subconline{3.6 Theorems on definiteness}{31}
\subconline{3.7 Subnetworks}{40}
\subconline{3.8 The recognition problem and process (initial statement)}{42}

\conline{4. Embeddings and the Definite Match Function}{43}
\subconline{4.1 Introduction}{43}
\subconline{4.2 Embedding tokens and types}{43}
\subconline{4.3 Symmetries}{46}
\subconline{4.4 Templates and saturation}{49}
\subconline{4.5 The definite match function}{50}
\subconline{4.6 Invariance theorems}{51}
\subconline{4.7 The recognition problem -- definitive statement}{56}

\conline{5. Inclusion Functions}{57}
\subconline{5.1 Introduction}{57}
\subconline{5.2 Definition of inclusion functions}{57}
\subconline{5.3 The recognition process}{59}

\conline{6. The Indefinite Match Function}{60}
\subconline{6.1 Introduction}{60}
\subconline{6.2 Template matching}{60}
\subconline{6.3 The indefinite match function}{61}
\subconline{6.4 Invariance theorems}{62}
\subconline{6.5 Adjustment of the embedding token}{63}
\subconline{6.6 The recognition process}{63}

\conline{7. How the Inclusion Functions are Determined}{64}
\subconline{7.1 Introduction}{64}
\subconline{7.2 The inclusion vector, $\bold i$}{64}
\subconline{7.3 How $\bold i$ is determined}{66}
\subconline{7.4 Algorithm for finding $\bold i$}{66}
\subconline{7.5 The recognition process}{69}

\conline{8. The Structural Operations}{70}
\subconline{8.1 Introduction}{70}
\subconline{8.2 Pruning operations}{70}
\subconline{8.3 Unprunability and its consequences}{76}
\subconline{8.4 Extension operations}{81}
\subconline{8.5 Inextendability and its consequences}{85}
\subconline{8.6 Merging two symbol tokens}{86}
\subconline{8.7 Partitioning a symbol token into two}{87}
\subconline{8.8 The outcome of the recognition process}{89}

\conline{9. The Whole Recognition Process}{90}
\subconline{9.1 Introduction}{90}
\subconline{9.2 Line operations}{90}
\subconline{9.3 How temperature is determined}{91}
\subconline{9.4 How the bareness function $B$ is determined}{92}
\subconline{9.5 Summary of the entire recognition process}{93}
\subconline{9.6 The outcome of recognition}{93}

\conline{Summary of Notation and Terminology}{96}

\vfill\supereject

\runninghead{1. Introduction}

\head{1. Introduction}

\bigskip\f
The purpose of this project is to develop a new graph grammar formalism for
error-tolerant syntactic pattern recognition.  This paper provides the
mathematical theory in full. It should be read in conjunction with the paper
\i{A New Graph Grammar Formalism for Robust Syntactic Pattern Recognition},
available at https://doi.org/10.48550/arXiv.2504.15975,
which provides a broader account of the context, purpose and application of 
this project, with example grammars and runs.

This paper develops further the mathematical framework in my 2004 technical
report, \i{Mathematical Theory of Recursive Symbol Systems} (Technical Report
GEN-0401, Keele University, Computer Science Department, available at
https://eprints.keele.ac.uk/id/eprint/63/), which I shall cite here simply as
\ic{(2004)}.  Sections 1--5 of (2004) are still valid, but section 6 (Networks
and Homomorphisms) and section 7 (The Recognition Problem) are inadequate and
this report supersedes them.  In particular, I have extended the concept of
network, mainly by the addition of \i{subsymbols}, and developed the
mathematical theory to define the pattern recognition process fully.

The contents of this report are as follows.

Section 2 develops the general theory of functions and relations that will be
needed in the subsequent sections.

Section 3 gives new definitions of \i{network}, \i{homomorphism} and
\i{definite} and \i{semi-definite} networks, superseding those in (2004, \S6).

Section 4 extends the theory of embeddings, introduced in (2004, \S6.4). The
$Match$ function, which was introduced in (2004, \S7.3), is treated more
satisfactorily here as two functions, a \i{definite match function} $DM$ and an
\i{indefinite match function} $IM$ (defined in \S6). 
The subject of symmetries is treated more
thoroughly and several theorems are proved on the affine invariance of the
grammatical framework. The theory of templates (introduced in (2004, \S4)) is
extended here by introducing the concept of \i{saturation}, which expresses the
notion that when several templates overlap in the image plane they interfere
with one another. The recognition problem can now be formally stated.

Section 5 develops the theory of inclusion functions, which were introduced in
(2004, \S7.2).

Section 6 defines the \i{indefinite match function} $IM$, which applies to
networks that are not necessarily definite, with inclusion functions.
The invariance theorems of \S4 are generalised to $IM$. The calculation of the
adjustment of the embeddings by gradient ascent in (2004) is adapted to $IM$.

Section 7 states the mechanism by which the inclusion functions are determined
during recognition.

Section 8 defines the \i{structural operations} by which the pattern grows during
recognition.

Section 9 states the entire recognition algorithm.

The whole theory is built up by a process of stepwise refinement. The first
four sections establish the underlying framework and specify the recognition
problem. Sections~5--9 develop the algorithm for solving it incrementally,
starting with an abstract account of the recognition process and refining it
step by step with each chapter. Stepwise refinement is a valuable method for
managing the complexity of the mathematical theory and the algorithm: it allows
for a separation of concerns, particularly between the structural and geometric
aspects of the theory, and enables the theory to be built up one layer at a
time, with the whole recognition process in view at each stage, at
ever-increasing levels of detail.

At each stage of the theory I shall make explicit the correctness conditions
the recognition algorithm must satisfy to solve the recognition problem,
culminating in theorem~48. The earlier, more fundamental stages (\S\S2--6) are
clean, rigorous and provably correct; the subsequent stages are progressively
messier, with arbitrary parameters and algorithms not guaranteed to converge to
the optimum solution. I distinguish clearly between those properties of the
recognition process that are guaranteed to hold, those that are likely to hold,
and those that one merely hopes will hold.

\vfill\supereject 
\runninghead{2. Functions and relations}

\head{2. Functions and Relations}

\subhead{2.1 Introduction}
This section introduces some concepts involving functions and relations that
will be needed in the theory of networks to follow, especially the concept of an
\i{acyclic} relation, a \i{connected} relation relative to a function, and a
\i{minimal} relation relative to a function. Relations will be used in the
following section to express the way in which subsymbols are glued to
supersymbols.

\subhead{2.2 Basic definitions and theorems}
A \i{function} $f:X\to Y$ maps every element of the set $X$ to a unique element
of the set $Y$. $X$ is called the \i{domain} of $f$, $\dom(f)$.

\defn For any function $f:X\to Y$ and any sets $A,B$,
$$ f(A) = \comp{f(x)}{x \in X \cap A}, \qquad
f\pre B = \comp{x \in X}{f(x) \in B}. $$
The \i{range} of $f$, $\ran(f)$, is defined as $f(X)$.

\defn For any function $f:X\to Y$ and any set $A \subseteq X$, the
\i{restriction} of $f$ to $A$, $f|_A:A \to Y$, is defined by
$$ \forall x\from A\ f|_A(x) = f(x). $$

\defn For any functions $f:A\to B$ and $g:C\to D$, the \i{composition} of $f$
and $g$, $f \circ g:C \cap g\pre A \to B$, is defined by
$$ \forall x\from C \cap g\pre A \quad (f\circ g)(x) = f(g(x)). $$

\medskip\f
The term \i{relation} will be understood to mean a binary relation applicable to
all objects: for any relation $R$ and every pair of objects $a,b$, either
$R(a,b)$ holds or it does not.

\defn The \i{domain} $\dom(R)$ and \i{range} $\ran(R)$ of a relation $R$ are
defined by
$$ \dom(R) = \comp{a}{\exists b\ R(b,a)}, \qquad
\ran(R) = \comp{b}{\exists a\ R(b,a)}. $$

\defn A relation $R$ is said to be \i{on} a set $A$ iff $\dom(R) \subseteq A$
and $\ran(R) \subseteq A$.

\defn For any set $A$, the \i{identity} relation $id_A$ is defined by
$$ \forall a,b\quad (id_A(a,b) \ \iff \ a=b\in A). $$

\defn The empty relation $\bot$ is defined by $\forall a,b \ \neg\, \bot(a,b)$.

\defn For any relations $R$ and $S$,
$$\eqalign{
R = S \ &\iff \ \forall a,b\ (R(a,b) \iff S(a,b)) \cr
R \subseteq S \ &\iff \ \forall a,b\ (R(a,b) \Rightarrow S(a,b)) \cr 
R \subset S \ &\iff \ R \subseteq S \and R \ne S.
}$$

\defn For any relations $R$ and $S$, the relations $R \cap S$, $R \cup S$ and
$R\setdiff S$ are defined by
$$\forall a,b\ \ \left\lbrace\eqalign{
(R \cap S)(a,b) &\iff R(a,b) \wedge S(a,b), \cr
(R \cup S)(a,b) &\iff R(a,b) \vee S(a,b), \cr
(R \setdiff S)(a,b) &\iff R(a,b) \wedge \neg S(a,b).
}\right.$$

\defn For any relations $R$ and $S$, the \i{composed} relation $R \circ S$ is
defined by
$$ \forall a,c\ \ 
((R \circ S)(a,c) \ \iff \ \exists b\ (R(a,b) \wedge S(b,c))).
$$
(In all expressions, the composition operator $\circ$ has higher syntactic
precedence than $\cap$, $\cup$ and $\setdiff$.)

\defn For any relation $R$, the \i{inverse} relation $R\inv$ is defined
by
$$ \forall a,b\ \ (R\inv (b,a) \ \iff \ R(a,b)). $$

\defn The \i{graph} of a function $f$ is the relation $\overline f$ defined by
$$ \forall a,b\ \ (\overline f(b,a) \ \iff \ a \in \dom(f) \wedge b=f(a)). $$

\theorem 1. (Obvious properties of relations.) For any relations $R,S,T$,
any functions $f,g$, and any sets $A,X,Y$,

\item{(i)} $\overline{f \circ g} = \overline f \circ \overline g$,
$\dom(\overline f) = \dom(f)$, and $\ran(\overline f) = \ran(f)$

\item{(ii)} if $f:X \to Y$ then $\overline f \circ id_X = \overline f = id_Y
\circ \overline f$,

\item{(iii)} if $f,g:X\to Y$ and $\overline f \subseteq \overline g$ then
$f=g$,

\item{(iv)} $\overline{f|_A} = \overline f \circ id_A$,

\item{(v)} $id_A \circ \overline f = \overline f \circ id_{f\pre A}$,

\item{(vi)} $id_A \circ R \subseteq R$ and $R \circ id_A \subseteq R$, with
equality if $R$ is on $A$,

\item{(vii)} $id_X \circ id_Y = id_{X \cap Y} = id_X \cap id_Y$ and $id_{X \cup
Y} = id_X \cup id_Y$,

\item{(viii)} $\bot \circ R = \bot = R \circ \bot$,

\item{(ix)} $T \subseteq R \cap S$ iff $T \subseteq R$ and $T \subseteq S$
(in particular, $R \cap S \subseteq R$ and $R \cap S \subseteq S$),

\item{(x)} $R \cup S \subseteq T$ iff $R \subseteq T$ and $S \subseteq T$
(in particular, $R \subseteq R \cup S$ and $S \subseteq R \cup S$),

\item{(xi)} $(R \circ S)\inv = S\inv \circ R\inv$, $(R \cap S)\inv = R\inv
\cap S\inv$, $(R \cup S)\inv = R\inv \cup S\inv$,

\item{(xii)} if $R \subseteq S$ then $R\inv \subseteq S\inv$, $R \circ T
\subseteq S \circ T$ and $T \circ R \subseteq T \circ S$,

\item{(xiii)} if $R \subseteq S$ then $\dom(R) \subseteq \dom(S)$ and $\ran(R)
\subseteq \ran(S)$,

\item{(xiv)} if $R \circ S = \bot$ then $\dom(R) \cap \ran(S) = \emptyset$,

\item{(xv)} $\ran(R) = \dom(R\inv)$,

\item{(xvi)} $id_{\dom(R)} \subseteq R\inv \circ R$ and $id_{\ran(R)} \subseteq
R \circ R\inv$,

\item{(xvii)} $\dom(R \circ id_A) = \dom(R) \cap A$ and $\ran(id_A \circ R) = A
\cap \ran(R)$.

\theorem 2. If $f:X\to Y$, and $R$ and $S$ are relations, then

\item{(i)} $\overline f \circ \overline f\inv \subseteq id_Y$,

\item{(ii)} $id_X \subseteq \overline f\inv \circ \overline f$,

\item{(iii)} if $R \subseteq S \circ \overline f$ then $R \circ \overline f\inv
\subseteq S \circ id_Y$,

\item{(iv)} if $\overline f \circ R \subseteq S$ then $id_X \circ R \subseteq
\overline f\inv \circ S$.

\proof (i) For any $y,y'$ such that $(\overline f \circ \overline f\inv)(y,y')$,
we have $y,y' \in Y$ and $\exists x \from X\ (y = f(x) \wedge f(x) = y')$, which
implies that $y=y'$, and hence $id_Y(y,y')$.

(ii) For any $x\from X$, there exists $y$ (namely $f(x)$) such that $f(x) = y$
and $y = f(x)$, and hence $(\overline f\inv \circ \overline f)(x,x)$.

(iii) If $R \subseteq S \circ \overline f$ then $R \circ \overline f\inv
\subseteq S \circ \overline f \circ \overline f\inv \subseteq S \circ id_Y$, by
part (i).

(iv) If $\overline f \circ R \subseteq S$ then $id_X \circ R \subseteq \overline
f\inv \circ \overline f \circ R \subseteq \overline f\inv \circ S$, by part
(ii). \qed

\theorem 3. For any relations $R,S,T$ and any function $f$,

\item{(i)} $(R \cup S) \circ T = R \circ T \ \cup\ S \circ T$,

\item{(ii)} $T \circ (R \cup S) = T \circ R \ \cup\ T \circ S$,

\item{(iii)} $(R \cap S) \circ T \subseteq R \circ T \ \cap\ S \circ T$,

\item{(iv)} $T \circ (R \cap S) \subseteq T \circ R \ \cap\ T \circ S$,

\item{(v)} $(R \cap S) \circ \overline f = R \circ \overline f \ \cap\ S \circ
\overline f$,

\item{(vi)} $\overline f\inv \circ (R \cap S) = \overline f\inv \circ R \ \cap\
\overline f\inv \circ S$.

\proof (i) For any $a,c$,
$$\eqalign{
((R \cup S) \circ T)(a,c)
&\text{ iff } \exists b\ ((R \cup S)(a,b) \wedge T(b,c)) \cr
&\text{ iff } \exists b\ ((R(a,b) \vee S(a,b)) \wedge T(b,c)) \cr
&\text{ iff } \exists b\ (R(a,b) \wedge T(b,c)) \vee
\exists b\ (S(a,b) \wedge T(b,c)) \cr
&\text{ iff } (R \circ T \ \cup\ S \circ T)(a,c).
}$$

(ii) For any $a,c$,
$$\eqalign{
(T \circ (R \cup S))(a,c)
&\text{ iff } \exists b\ (T(a,b) \wedge (R \cup S)(b,c)) \cr
&\text{ iff } \exists b\ (T(a,b) \wedge (R(b,c) \vee S(b,c))) \cr
&\text{ iff } \exists b\ (T(a,b) \wedge R(b,c)) \vee \exists b\ (T(a,b) \wedge
S(b,c)) \cr
&\text{ iff } (T \circ R \ \cup\ T \circ S)(a,c).
}$$

(iii) From $R \cap S \subseteq R$ and $R \cap S \subseteq S$ we infer $(R \cap
S) \circ T \subseteq R \circ T$ and $(R \cap S) \circ T \subseteq S \circ T$,
and hence $(R \cap S) \circ T \subseteq R \circ T \ \cap\ S \circ T$.

(iv) From $R \cap S \subseteq R$ and $R \cap S \subseteq S$ we infer $T \circ (R
\cap S) \subseteq T \circ R$ and $T \circ (R \cap S) \subseteq T \circ S$, and
hence $T \circ (R \cap S) \subseteq T \circ R \ \cap\ T \circ S$.

(v) For any $a,c$,
$$\eqalign{
((R \cap S) \circ \overline f)(a,c)
&\text{ iff } \exists b\ ((R \cap S)(a,b) \wedge c \in \dom(f) \wedge b=f(c)) \cr
&\text{ iff } c \in \dom(f) \wedge (R \cap S)(a,f(c)) \cr
&\text{ iff } c \in \dom(f) \wedge R(a,f(c)) \wedge S(a,f(c)) \cr
&\text{ iff } \exists b\ (R(a,b) \wedge c \in \dom(f) \wedge b=f(c)) \ \wedge\ 
\exists b'\ (S(a,b') \wedge c \in \dom(f) \wedge b'=f(c)) \cr
&\text{ iff } (R \circ \overline f)(a,c) \ \wedge\ (S \circ \overline f)(a,c)
\cr
&\text{ iff } (R \circ \overline f \ \cap\ S \circ \overline f)(a,c).
}$$

(vi) Part (v) gives $(R\inv \cap S\inv) \circ \overline f = R\inv \circ
\overline f \ \cap\ S\inv \circ \overline f$, and taking the inverse gives
$\overline f\inv \circ (R \cap S) = \overline f\inv \circ R \ \cap\ \overline
f\inv \circ S$. \qed

\theorem 4. For any relations $R,S,T$, and any sets $A,B$,

\item{(i)} $R \circ S \ \cap\ T \subseteq (R \ \cap\ T \circ S\inv) \circ S$,

\item{(ii)} $R \circ S \ \cap\ T \subseteq R \circ (S \ \cap\ R\inv \circ T)$,

\item{(iii)} $R \circ id_A \ \cap\ S = (R \cap S) \circ id_A$,

\item{(iv)} $id_A \circ R \ \cap\ S = id_A \circ (R \cap S)$,

\item{(v)} if $id_A \circ R \subseteq S \circ id_B$ then $id_A \circ R
\subseteq R \circ id_B$,

\item{(vi)} if $R \circ id_A \subseteq id_B \circ S$ then $R \circ id_A
\subseteq id_B \circ R$.

\proof (i) For any $x,z$,
$$\eqalign{
(R \circ S \ \cap\ T)(x,z)
&\text{ iff } \exists y\ (R(x,y) \wedge S(y,z) \wedge T(x,z)) \cr
&\text{ implies } \exists y,z'\ (R(x,y) \wedge T(x,z') \wedge S(y,z') \wedge
S(y,z))
\quad\text{by taking $z'=z$} \cr
&\text{ iff } \exists y\ (R(x,y) \wedge (T \circ S\inv)(x,y) \wedge S(y,z)) \cr
&\text{ iff } ((R \ \cap\ T \circ S\inv) \circ S)(x,z).
}$$

(ii) Applying part (i), with $S\inv$ substituted for $R$, $R\inv$ substituted
for $S$, and $T\inv$ substituted for $T$,
$$ S\inv \circ R\inv \ \cap\ T\inv
\subseteq (S\inv \ \cap\ T\inv \circ R) \circ R\inv $$
and then inverting this gives
$$ R \circ S \ \cap\ T \subseteq R \circ (S \ \cap\ R\inv \circ T). $$

(iii) Using part (i), $R \circ id_A \ \cap\ S \subseteq (R \cap S \circ id_A)
\circ id_A \subseteq (R \cap S) \circ id_A$. Conversely, using theorem~3(iii),
$(R \cap S) \circ id_A \subseteq R \circ id_A \ \cap\ S \circ id_A \subseteq R
\circ id_A \ \cap\ S$.

(iv) Applying part (iii) with $R\inv$ substituted for $R$ and $S\inv$
substituted for $S$ gives $R\inv \circ id_A \ \cap\ S\inv = (R\inv \cap S\inv)
\circ id_A$, and inverting this gives $id_A \circ R \ \cap\ S = id_A \circ (R
\cap S)$.

(v) If $id_A \circ R \subseteq S \circ id_B$ then, combining this with $id_A
\circ R \subseteq R$ gives
$$\eqqalign\quad{
id_A \circ R &\subseteq S \circ id_B \ \cap\ R
&\cr
&= (S \cap R) \circ id_B
&\text{by part (iii)}\cr
&\subseteq R \circ id_B
&\text{since $S \cap R \subseteq R$.}\cr
}$$

(vi) If $R \circ id_A \subseteq id_B \circ S$ then, combining this with $R \circ
id_A \subseteq R$ gives
$$\eqqalign\quad{
R \circ id_A &\subseteq id_B \circ S \ \cap\ R
&\cr
&= id_B \circ (S \cap R)
&\text{by part (iv)}\cr
&\subseteq id_B \circ R
&\text{since $S \cap R \subseteq R$.}\cr
}$$
\qed

\theorem 5. For any relation $R$, $R=\overline f$ for some function $f:X\to
Y$ iff $R \circ R\inv \subseteq id_Y$ and $id_X \subseteq R\inv \circ R$.

\proof ($\Rightarrow$) If $R = \overline f$ then $R \circ R\inv \subseteq
id_Y$ and $id_X \subseteq R\inv \circ R$ by theorem~2(i),(ii).

($\Leftarrow$) Suppose $R \circ R\inv \subseteq id_Y$ and $id_X \subseteq R\inv
\circ R$. For any $x\from X$, $id_X(x,x)$ holds, so $(R\inv \circ R)(x,x)$
holds, so there exists $y$ such that $R(y,x)$.

For any $x\from X$ and any $y$, if $R(y,x)$ then $(R\circ R\inv)(y,y)$, so
$id_Y(y,y)$, so $y\from Y$.

For any $x\from X$ and $y,y'\from Y$, if $R(y,x)$ and $R(y',x)$ then $(R\circ
R\inv)(y,y')$, so $id_Y(y,y')$, so $y=y'$.

These facts show that $R = \overline f$ for a function $f:X\to Y$. \qed

\theorem 6. A rectangle of functions $\displaystyle\rectangleA DCBAgfqp$ is a
pullback in the category of sets iff
$$ \overline f \inv \circ \overline g = \overline p \circ \overline q\inv
\quad\text{and}\quad
\overline p\inv \circ \overline p \ \cap\ \overline q\inv \circ \overline q
= id_A. $$

\proof I shall use the standard characterisation of a pullback in the category
of sets, namely $f \circ p = g \circ q$ and $\forall b\from B\ \forall c\from
C\ (f(b)=g(c) \Rightarrow \exists!a\from A\ (p(a)=b \wedge q(a)=c))$.

($\Rightarrow$) Suppose the rectangle is a pullback. I shall verify the two
equations.

$\underline{\overline f \inv \circ \overline g \subseteq \overline p \circ
\overline q\inv}$. For any $b$ and $c$, if $(\overline f \inv \circ \overline
g)(b,c)$ then $b \in B$, $c \in C$ and $\exists d\ (f(b)=d \wedge d=g(c))$, so
$f(b)=g(c)$, so $\exists a\from A\ (b=p(a) \wedge q(a)=c)$ by the pullback
condition, so $(\overline p \circ \overline q\inv)(b,c)$.

$\underline{\overline p \circ \overline q\inv \subseteq \overline f \inv \circ
\overline g}$. For any $b$ and $c$, if $(\overline p \circ \overline
q\inv)(b,c)$ then there exists $a\from A$ such that $b=p(a) \wedge q(a)=c$, so
$f(b)=f(p(a))=g(q(a))=g(c)$, so $(\overline f\inv \circ \overline g)(b,c)$.

$\underline{id_A \subseteq \overline p\inv \circ \overline p \ \cap\ \overline
q\inv \circ \overline q}$. This follows from $id_A \subseteq \overline p\inv
\circ \overline p$ and $id_A \subseteq \overline q\inv \circ \overline q$, which
come from theorem~2(ii).

$\underline{\overline p\inv \circ \overline p \ \cap\ \overline q\inv \circ
\overline q \subseteq id_A}$. For any $a,a'$, if $(\overline p\inv \circ
\overline p \ \cap\ \overline q\inv \circ \overline q)(a,a')$ then $a,a' \in A$
and $\exists b\from B\ (p(a)=b \wedge b=p(a'))$ and $\exists c\from C\ (q(a)=c
\wedge c=q(a'))$, hence $f(b)=f(p(a))=g(q(a))=g(c)$, so by the pullback condition
there exists only one $x\from A$ such that $p(x)=b$ and $q(x)=c$, so $a=a'$, as
required.

($\Leftarrow$) Suppose $\overline f \inv \circ \overline g = \overline p \circ
\overline q\inv$ and $\overline p\inv \circ \overline p \ \cap\ \overline q\inv
\circ \overline q = id_A$. I shall verify the conditions for a pullback.

$\underline{f \circ p = g \circ q}$. For any $a\from A$, $(\overline p \circ
\overline q\inv)(p(a),q(a))$ holds, so by the equation $\overline f \inv \circ
\overline g = \overline p \circ \overline q\inv$ we have $(\overline f \inv
\circ \overline g)(p(a),q(a))$, which means that $f(p(a)) = g(q(a))$, as
required.

$\underline{\forall b\from B\ \forall c\from C\ (f(b)=g(c) \Rightarrow \exists
a\from A\ (p(a)=b \wedge q(a)=c))}$. Consider any $b\from B$ and $c\from C$ such
that $f(b)=g(c)$. Then $(\overline f\inv \circ \overline g)(b,c)$ holds, so by
the equation $\overline f \inv \circ \overline g = \overline p \circ \overline
q\inv$ we have $(\overline p \circ \overline q\inv)(b,c)$, which means that
there exists $a\from A$ such that $b=p(a)$ and $q(a)=c$ as required.

$\underline{\forall b\from B\ \forall c\from C\ (f(b)=g(c) \Rightarrow
\exists^{\le 1} a\from A\ (p(a)=b \wedge q(a)=c))}$. Consider any $b\from B$ and
$c\from C$ such that $f(b)=g(c)$. Suppose there exist $a,a'\from A$ such that
$p(a)=b=p(a')$ and $q(a)=c=q(a')$. Then $(\overline p\inv \circ \overline p \
\cap\ \overline q\inv \circ \overline q)(a,a')$, so by $\overline p\inv \circ
\overline p \ \cap\ \overline q\inv \circ \overline q = id_A$ we have $a=a'$, as
required. \qed

\theorem 7. For any sets $A,B,C$, and any functions $p:A\to C$ and $q:B\to C$,
$A \buildrel p \over \rightarrow C \buildrel q \over \leftarrow B$ is a sum
diagram in the category of sets iff
$$ \overline p \circ \overline p\inv \ \cup\ \overline q \circ \overline q\inv
= id_C, \quad
\overline p\inv \circ \overline p = id_A, \quad
\overline q\inv \circ \overline q = id_B, \quad
\overline p\inv \circ \overline q = \bot, \quad
\overline q\inv \circ \overline p = \bot. $$

\proof ($\Rightarrow$) Assume $A \buildrel p \over \rightarrow C \buildrel q
\over \leftarrow B$ is a sum diagram.

$\underline{\overline p \circ \overline p\inv \ \cup\ \overline q \circ
\overline q\inv = id_C}$. Theorem~2(i) gives $\overline p \circ \overline p\inv
\subseteq id_C$ and $\overline q \circ \overline q\inv \subseteq id_C$; so
$\overline p \circ \overline p\inv \ \cup \ \overline q \circ \overline q\inv
\subseteq id_C$. To show that this inclusion is an equality, choose a set $X$
with more than one element and any functions $f:A \to X$ and $g:B \to X$. Since
$A \buildrel p \over \rightarrow C \buildrel q \over \leftarrow B$ is a sum
diagram, there exists a unique function $i:C \to X$ such that $i\circ p =f$ and
$i\circ q = g$. If $\overline p \circ \overline p\inv \ \cup \ \overline q \circ
\overline q\inv \subset id_C$ then choose $c\from C$ such that $(\overline p
\circ \overline p\inv \ \cup \ \overline q \circ \overline q\inv)(c,c)$ does not
hold. Define $j:C \to X$ as equal to $i$ except at $c$. Then, for all $a\from
A$, $(\overline p\circ \overline p\inv)(p(a),p(a))$ holds, so $p(a) \ne c$, so
$j(p(a))=i(p(a))=f(a)$. Thus $j \circ p = f$. A similar argument shows that $j
\circ q = g$. This contradicts the uniqueness of $i$. The contradiction
establishes that $\overline p \circ \overline p\inv \ \cup \ \overline q \circ
\overline q\inv = id_C$.

$\underline{\overline p\inv \circ \overline p = id_A}$. Theorem 2(ii) gives
$id_A \subseteq \overline p\inv \circ \overline p$. For the converse, choose a
set $X=A$, a function $f:A\to X$ equal to the identity function on $A$, and an
arbitrary function $g:B\to X$ (ignoring the case $A = \emptyset$, for which
$\overline p\inv \circ \overline p = id_A$ is trivially true). Then by the sum
property there exists a unique function $i:C\to X$ such that $i \circ p = f$ and
$i\circ q = g$; thus $i:C \to A$ and $\overline i\circ \overline p = id_A$. Then
$id_A \circ \overline p\inv \subseteq \overline i \circ id_C$ by theorem~2(iii),
so $\overline p\inv \subseteq \overline i$, so $\overline p\inv \circ \overline
p \subseteq \overline i \circ \overline p = id_A$, as required.

$\underline{\overline q\inv \circ \overline q = id_B}$. A similar argument
applies.

$\underline{\overline p\inv \circ \overline q = \bot}$. Choose a set $X$ with
more than one element, and choose $f:A\to X$ and $g:B\to X$ with disjoint
images, so that $\overline f\inv \circ \overline g = \bot$. By the sum property,
there exists a unique function $i:C\to X$ such that $i \circ p = f$ and $i \circ
q = g$. Then
$$ \bot = \overline f\inv \circ \overline g
= (\overline i \circ \overline p)\inv \circ \overline i \circ \overline q
= \overline p\inv \circ \overline i\inv \circ \overline i \circ \overline q
\supseteq \overline p\inv \circ id_C \circ \overline q
= \overline p\inv \circ \overline q $$
so $\bot = \overline p\inv \circ \overline q$, as required.

$\underline{\overline q\inv \circ \overline p = \bot}$. This follows by
inverting $\overline p\inv \circ \overline q = \bot$.

($\Leftarrow$) Assume the five equations; I shall show $A \buildrel p \over
\rightarrow C \buildrel q \over \leftarrow B$ is a sum diagram. Given any set
$X$ and functions $f:A\to X$ and $g:B\to X$, define a relation $R = \overline f
\circ \overline p\inv \ \cup \ \overline g \circ \overline q\inv$. First note
that
$$\eqalign{
R \circ \overline p
&= \overline f \circ \overline p\inv \circ \overline p \ \cup \
\overline g \circ \overline q\inv \circ \overline p
= \overline f \circ id_A \ \cup \ \overline g \circ \bot
= \overline f, \cr
R \circ \overline q
&= \overline f \circ \overline p\inv \circ \overline q \ \cup \
\overline g \circ \overline q\inv \circ \overline q
= \overline f \circ \bot \ \cup \ \overline g \circ id_B
= \overline g.
}$$
Then
$$ R \circ R\inv
= R \circ
(\overline p \circ \overline f\inv \ \cup \ \overline q \circ \overline g\inv)
= R \circ \overline p \circ \overline f\inv \ \cup\ R \circ \overline q \circ
\overline g\inv
= \overline f \circ \overline f\inv \ \cup\
\overline g \circ \overline g\inv
\subseteq id_X $$
by theorem~2(i), and
$$\eqalign{
R\inv \circ R
&= (\overline p \circ \overline f\inv \ \cup \
\overline q \circ \overline g\inv) \circ
(\overline f \circ \overline p\inv \ \cup \
\overline g \circ \overline q\inv)
\supseteq \overline p \circ \overline f\inv \circ \overline f \circ \overline
p\inv \ \cup \
\overline q \circ \overline g\inv \circ \overline g \circ \overline q\inv
\cr&
\supseteq \overline p \circ id_A \circ \overline p\inv \ \cup \
\overline q \circ id_B \circ \overline q\inv
= \overline p \circ \overline p\inv \ \cup \
\overline q \circ \overline q\inv
= id_C
}$$
using theorem~2(ii). By theorem~5, $R=\overline i$, for some function $i:C\to
X$. The equations $R \circ \overline p = \overline f$ and $R \circ \overline q =
\overline g$ then imply $i \circ p = f$ and $i \circ q = g$.

To show the uniqueness of $i$, consider any function $j:C\to X$ satisfying $j
\circ p = f$ and $j \circ q = g$. Then $\overline j \circ \overline p =
\overline f$ and $\overline j \circ \overline q = \overline g$, so by
theorem~2(iii) $\overline f \circ \overline p\inv \subseteq \overline j \circ
id_C = \overline j$ and $\overline g \circ \overline q\inv \subseteq \overline j
\circ id_C = \overline j$, so $\overline i = R = \overline f \circ \overline
p\inv \ \cup\ \overline g \circ \overline q\inv \subseteq \overline j$. Since
$i$ and $j$ are both functions from $C$ to $X$, this is sufficient to imply
$i=j$, as required. \qed

\subhead{2.3 Acyclic and connected relations}

\defn A relation $R$ is \i{finite} iff there are finitely many pairs $(a,b)$
such that $R(a,b)$ holds.

\defn The \ic{not-equal-to} relation $NE$ is defined by $NE(a,b) \iff a \ne b$.

\theorem 8. For any relation $R$,

\item{(i)} $\dom(R \ \cap\ NE \circ R) = \comp{a}{\exists^{>1}b\ R(b,a)}$,

\item{(ii)} $\dom(R \setdiff NE \circ R) = \comp{a}{\exists!b\ R(b,a)}$,

\item{(iii)} $\dom(R \ \cap\ NE \circ R) \ \cap \ \dom(R \setdiff NE \circ R)
= \emptyset$,

\item{(iv)} $\dom(R \ \cap\ NE \circ R) \ \cup \ \dom(R \setdiff NE \circ R)
= \dom(R)$,

\item{(v)} $\ran(R \ \cap\ R \circ NE) = \comp{b}{\exists^{>1}a\ R(b,a)}$,

\item{(vi)} $\ran(R \setdiff R \circ NE) = \comp{b}{\exists!a\ R(b,a)}$,

\item{(vii)} $\ran(R \ \cap\ R \circ NE) \ \cap \ \ran(R \setdiff R \circ NE)
= \emptyset$,

\item{(viii)} $\ran(R \ \cap\ R \circ NE) \ \cup \ \ran(R \setdiff R \circ NE)
= \ran(R)$.

\def\iff{\text{\quad iff\quad }}

\proof (i) For any $a$,
$$\eqalign{
a \in \dom(R \ \cap\ NE \circ R)
&\iff \exists b\ (R \ \cap\ NE \circ R)(b,a)
\iff \exists b\ R(b,a) \ \wedge\ \exists b'\ (b\ne b' \wedge R(b',a))
\cr&
\iff \exists b,b'\ (b\ne b' \wedge R(b,a) \wedge R(b',a))
\iff \exists^{>1}b\ R(b,a).
}$$

(ii) For any $a$,
$$\eqalign{
a \in \dom(R \setdiff NE \circ R)
&\iff \exists b\ (R \setdiff NE \circ R)(b,a)
\iff \exists b\ R(b,a) \ \wedge\ \neg\exists b'\ (b\ne b' \wedge R(b',a))
\cr&
\iff \exists!b\ R(b,a).
}$$

(iii) and (iv) follow from (i) and (ii).

(v)--(viii) follow from (i)--(iv) respectively by substituting $R\inv$ for $R$.
\qed

\theorem 9. For any relations $R,S,T$,
$$ \dom(R \cap T) \ \cap\ \dom(S \setdiff NE \circ T) \subseteq \dom(R \cap S).
$$

\proof For any $a \in \dom(R \cap T) \ \cap\ \dom(S \setdiff NE \circ T)$,
there exists $b$ such that $R(b,a)$ and $T(b,a)$ and there exists $c$ such that
$S(c,a)$ but not $(NE \circ T)(c,a)$. The last of these means that there is no
$d$ not equal to $c$ such that $T(d,a)$; hence $b=c$. Thus we have $R(b,a)$ and
$S(b,a)$, so $a \in \dom(R \cap S)$. \qed

\defn A relation $R$ is \i{acyclic} iff
$$ \NOT\, \exists R^*\ (\bot \ne R^* \subseteq R \, \and\, R^* \subseteq (R^*
\circ NE \, \cap\, NE \circ R^*)). $$

\def\mapleft#1{\,\smash{\mathop{\leftarrow}\limits^{#1}}}
\def\mapright#1{\smash{\mathop{\rightarrow}\limits^{#1}}\,}

\medskip\f
(Informally, $R$ is acyclic iff every non-empty subrelation $R^*$ has an element
of valency 1, i.e., an element related to just one element by $R^*$ or to just
one element by ${R^*}\!\inv$. This is equivalent to the non-existence of a
finite cyclic sequence $x_1,\ldots x_n,x_1$, with $n$ even and $n>2$, where the terms
are all different and and related by $x_1 \mapright R x_2 \mapleft R x_3
\mapright R x_4 \mapleft R x_5 \mapright R \cdots \mapright R x_n \mapleft R
x_1$. However, we shall not need this
characterisation in the theory that follows.)

\theorem 10. If a relation $R$ is acyclic and $R' \subseteq R$ then $R'$ is
also acyclic.

\proof This is immediate from the definition. \qed

\theorem 11.

\item{(i)} If $f:X\to Y$, $R$ is a relation on $X$, and $S$ is a relation on
$Y$, such that
$$ S = \overline f \circ R \circ \overline f\inv, \qquad
\overline f\inv \circ \overline f \ \cap R\inv \circ R \subseteq id_X, \qquad
R \subseteq R \circ NE $$
then $S \subseteq S \circ NE$.

\item{(ii)} If $f:X\to Y$, $R$ is a relation on $X$, and $S$ is a relation on
$Y$, such that
$$ S = \overline f \circ R \circ \overline f\inv, \qquad
\overline f\inv \circ \overline f \ \cap R \circ R\inv \subseteq id_X, \qquad
R \subseteq NE \circ R$$
then $S \subseteq NE \circ S$.

\proof (i) Define the universal relations $U_X$ on $X$ and $U_Y$ on $Y$ by
$$ \forall a,b \quad (U_X(a,b) \iff a \in X \wedge b \in X, \quad
U_Y(a,b) \iff a \in Y \wedge b \in Y). $$
Then $U_Y \subseteq id_Y \cup NE$, so
$$\eqalign{
U_X
&= \overline f\inv \circ U_Y \circ \overline f
\subseteq \overline f\inv \circ (id_Y \cup NE) \circ \overline f
= \overline f\inv \circ id_Y \circ \overline f \ \cup\
\overline f\inv \circ NE \circ \overline f
\cr&
= \overline f\inv \circ \overline f \ \cup\
\overline f\inv \circ NE \circ \overline f
}$$
so
$$ U_X \setdiff \overline f\inv \circ \overline f
\subseteq \overline f\inv \circ NE \circ \overline f. \eqno(1)$$
Also, $R\inv \circ R \subseteq U_X$, since $R$ is on $X$, and
$$ \overline f\inv \circ \overline f \ \cap\ R\inv \circ R \ \cap\ NE
\subseteq id_X \cap NE = \bot $$
so
$$\eqqalignno\quad{
R\inv \circ R \ \cap\ NE
&\subseteq U_X\setdiff \overline f\inv \circ \overline f
&\cr
&\subseteq \overline f\inv \circ NE \circ \overline f
&\text{by (1)}\cr
}{(2)}$$
so
$$\eqqalign\quad{
S &= \overline f \circ R \circ \overline f\inv
&\cr
&= \overline f \circ (R \cap R) \circ \overline f\inv
&\cr
&\subseteq \overline f \circ (R \ \cap\ R \circ NE) \circ \overline f\inv
&\text{since $R \subseteq R \circ NE$}\cr
&\subseteq \overline f \circ R \circ (R\inv \circ R \ \cap\ NE) \circ
\overline f\inv
&\text{by theorem 4(ii)}\cr
&\subseteq \overline f \circ R \circ \overline f\inv \circ NE \circ
\overline f \circ \overline f\inv
&\text{by (2)}\cr
&= S \circ NE \circ \overline f \circ \overline f\inv
&\text{since $S = \overline f \circ R \circ \overline f\inv$}\cr
&\subseteq S \circ NE \circ id_Y
&\text{by theorem~2(i)}\cr
&\subseteq S \circ NE
&\cr
}$$
as required.

(ii) Inverting the hypotheses $S = \overline f \circ R \circ \overline f\inv$
and $R \subseteq NE \circ R$ gives $S\inv = \overline f \circ R\inv \circ
\overline f\inv$ and $R\inv \subseteq R\inv \circ NE$. Applying part (i) of the
theorem, with $R\inv$ and $S\inv$ substituted for $R$ and $S$, gives $S\inv
\subseteq S\inv \circ NE$, which can be inverted to $S \subseteq NE \circ S$.
\qed

\theorem 12. If $f:X\to Y$, $R$ is a relation on $X$, and $S$ is a relation
on $Y$, such that
$$ \overline f \circ R \subseteq S \circ \overline f, \qquad
\overline f\inv \circ \overline f \ \cap\ R\inv \circ R \subseteq id_X, \qquad
\overline f\inv \circ \overline f \ \cap\ R \circ R\inv \subseteq id_X $$
then $R$ is acyclic if $S$ is.

\proof Assuming $S$ is acyclic, we shall infer that $R$ is. Consider any
relation $R^*$ such that $\bot \ne R^* \subseteq R$; we must show $R^*
\not\subseteq R^* \circ NE \ \cap\ NE \circ R^*$. Define a relation $S^* =
\overline f \circ R^* \circ \overline f\inv$ on $Y$. Then $S^* \ne \bot$ (choose
any $x,x'$ such that $R^*(x,x')$; then $S^*(f(x),f(x'))$). Also, $\overline f
\circ R^* \subseteq \overline f \circ R \subseteq S \circ \overline f$, so $S^*
= \overline f \circ R^* \circ \overline f\inv \subseteq S \circ id_Y = S$ by
theorem~2(iii). Since $S$ is acyclic we conclude that $S^* \not\subseteq S^*
\circ NE \ \cap\ NE \circ S^*$.

Now, if $R^* \subseteq R^* \circ NE \ \cap\ NE \circ R^*$ then $R^* \subseteq
R^* \circ NE$ and $R^* \subseteq NE \circ R^*$. Also,
$$ \overline f\inv \circ \overline f \ \cap\ {R^*}\inv \circ R^* \subseteq
\overline f\inv \circ \overline f \ \cap\ R\inv \circ R \subseteq id_X $$
and
$$ \overline f\inv \circ \overline f \ \cap\ R^* \circ {R^*}\inv \subseteq
\overline f\inv \circ \overline f \ \cap\ R \circ R\inv \subseteq id_X $$
so, by theorem~11, $S^* \subseteq S^* \circ NE$ and $S^* \subseteq NE \circ
S^*$. This gives $S^* \subseteq S^* \circ NE \ \cap \ NE \circ S^*$, which is
not true.

This contradiction establishes that $R^* \not\subseteq R^* \circ NE \ \cap\ NE
\circ R^*$, as required. \qed

\defn If $f:X\to Y$ and $R$ is a relation on $X$ then $R$ is \i{connected}
relative to $f$ iff, for any set $Z$ and function $g:X\to Z$ such that
$\overline g \circ R \subseteq \overline g$, there exists a function $i:f(X)\to
Z$ such that $i \circ f = g$.

\medskip\f
(Informally, $R$ is connected relative to $f$ iff, for any $x,x'\from X$ such
that $f(x)=f(x')$, there exists a finite sequence $x=x_0,x_1,\ldots x_n=x'$ such
that, for each $i\from\{1,\ldots n\}$, $R(x_{i-1},x_i)$ or $R(x_i,x_{i-1})$
holds.)

\theorem 13. Given sets $N,\Sigma$, a function $P:N\to\Sigma$, and a finite
relation $G$ on $N$ such that

\item{(a)} $G \circ G = \bot$,

\item{(b)} $G$ is acyclic,

\item{(c)} $\overline P \circ G \subseteq \overline P$,

\f
then

\item{(i)} $\forall X \subseteq\Sigma\ |P\pre X| - |G \circ id_{P\pre X}| \ge
0$,

\item{(ii)} for any $X \subseteq\Sigma$, if $|P\pre X| - |G \circ id_{P\pre
X}|=0$ then $P\pre X = \emptyset$,

\item{(iii)} if $\forall X \subseteq\Sigma\ |P\pre X| - |G \circ id_{P\pre X}|
\le |X|$ then $G$ is connected relative to $P$.

\proof The proof is by induction on $|G|$. For the induction basis, suppose
$|G|=0$; then we can verify (i), (ii) and (iii) directly, as follows.

(i) For any $X\subseteq \Sigma$, $|P\pre X| - |G \circ id_{P\pre X}| = |P\pre X|
\ge 0$.

(ii) For any $X\subseteq \Sigma$ such that $|P\pre X| - |G \circ id_{P\pre
X}|=0$, we have $|P\pre X|=0$ and hence $P\pre X=\emptyset$, as required.

(iii) If $\forall X \subseteq\Sigma\ |P\pre X| - |G \circ id_{P\pre X}| \le |X|$
then
$$ \forall\sigma\from\Sigma\quad |P\preo\sigma| \le 1 $$
which means that $P$ is injective. In that case, given any $Z$ and $Q:N\to Z$,
the unique function $i:P(N)\to Z$ such that $i\circ P = Q$ is defined by
$\forall n\from N\ i(P(n)) = Q(n)$.

\medskip

For the induction step, suppose that $|G| > 0$, and define
$$\eqalign{
G' &= G \ \cap\ G \circ NE \ \cap\ NE \circ G \cr
S_1 &= \ran(G\setdiff G\circ NE) \cr
S_2 &= \dom((G \ \cap\ G\circ NE)\setdiff NE \circ G) \cr
S &= S_1 \cup S_2 \cr
N' &= N \setdiff S \cr
P' &= P|_{N'}.
}$$
These have the following properties.

\bigskip

\item{$(\alpha)$} $G' \subset G$.

Proof. This follows since $G$ is acyclic and not equal to $\bot$.

\bigskip

\item{$(\beta)$} $G'$ is a finite relation on $N'$.

Proof. $G'$ is finite since $G' \subset G$ and $G$ is finite. To show that $G'$
is on $N'$,
$$\eqqalign\quad{
\dom(G') \cap S_1
&\subseteq \dom(G) \cap \ran(G) = \emptyset
&\text{since $G \circ G = \bot$}\cr
\dom(G') \cap S_2
&\subseteq \dom(G \cap NE \circ G) \cap \dom(G \setdiff NE \circ G) =
\emptyset
&\text{by theorem~8(iii)} \cr
\ran(G') \cap S_1
&\subseteq \ran(G \cap G \circ NE) \cap \ran(G \setdiff G \circ NE) =
\emptyset
&\text{by theorem~8(vii)} \cr
\ran(G') \cap S_2
&\subseteq \ran(G) \cap \dom(G) = \emptyset
&\text{since $G \circ G = \bot$} \cr
}$$
thus $\dom(G') \subseteq N\setdiff S = N'$ and $\ran(G') \subseteq N\setdiff S =
N'$, as required.

\bigskip

\item{$(\gamma)$} For every $x \from S$, there exists a unique $y$ such that
$(G\setdiff G')(x,y)$ or $(G\setdiff G')(y,x)$ (these two cases being mutually
exclusive).

Proof. $(G\setdiff G')(x,y)$ and $(G\setdiff G')(y,x)$ are mutually exclusive by
$(G\setdiff G') \circ (G\setdiff G') \subseteq G \circ G = \bot$. We have $G
\setdiff G \circ NE \subseteq G \setdiff G'$, so
$$ S_1 \subseteq \ran(G\setdiff G'), \eqno(1) $$
and
$$ S_1 \, \cap\ \ran\bigl((G\setdiff G') \cap (G\setdiff G')\circ NE\bigr)
\subseteq S_1 \, \cap\ \ran(G \cap G\circ NE)
= \emptyset \eqno(2) $$
by theorem~8(vii), so from (1), (2) and theorem~8(viii)
$$ S_1
\subseteq \ran\bigl((G\setdiff G')\setdiff(G\setdiff G') \circ NE\bigr). $$
Using theorem~8(vi), this can be written as
$$ \forall x\from S_1 \, \exists!y \ (G\setdiff G')(x,y). \eqno(3) $$
Similarly, $(G \cap G \circ NE)\setdiff NE \circ G \subseteq G\setdiff G'$, so
$$ S_2 \subseteq \dom(G\setdiff G'), \eqno(4) $$
and
$$ S_2 \ \cap\ \dom\bigl((G\setdiff G') \cap NE \circ (G\setdiff G')\bigr)
\subseteq \dom(G\setdiff NE \circ G) \ \cap\ \dom(G \cap NE \circ G)
= \emptyset \eqno(5) $$
by theorem~8(iii), so from (4), (5) and theorem~8(iv)
$$ S_2
\subseteq \dom\bigl((G\setdiff G')\setdiff NE \circ (G\setdiff G')\bigr). $$
Using theorem~8(ii) this can be written as
$$ \forall x\from S_2 \, \exists!y\ (G\setdiff G')(y,x). \eqno(6) $$
Consequently, from (3), (6), and $(G\setdiff G') \circ (G\setdiff G') = \bot$,
$$ \forall x\from S\ \exists!y\ ((G\setdiff G')(x,y) \vee
(G\setdiff G')(y,x)) $$
as required.

\bigskip

\item{$(\delta)$} $\forall x,y\ (G(x,y) \Rightarrow x \in N' \vee y \in N')$.

Proof. First,
$$ \ran(G \cap G \circ NE) \ \cap\ S_1 = \ran(G \cap G \circ NE) \ \cap\
\ran(G \setdiff G \circ NE) = \emptyset \eqno(7) $$
by theorem~8(vii). Secondly,
$$ \ran(G \cap G \circ NE) \ \cap\ S_2
= \ran(G \cap G \circ NE) \ \cap\ \dom((G \ \cap\ G\circ NE)\setdiff NE \circ
G)
\subseteq \ran(G) \ \cap\ \dom(G)
= \emptyset. \eqno(8) $$
Combining (7) and (8) gives
$$ \ran(G \cap G \circ NE) \ \cap\ S = \emptyset. \eqno(9) $$
Next,
$$ \dom(G\setdiff G \circ NE) \ \cap\ S_1
= \dom(G\setdiff G \circ NE) \ \cap\ \ran(G\setdiff G\circ NE)
\subseteq \dom(G) \ \cap\ \ran(G)
= \emptyset. \eqno(10)$$
Also, applying theorem~9, with $R = G\setdiff G \circ NE$, $S = G \cap G \circ
NE$, and $T = G$, gives
$$ \dom(G\setdiff G \circ NE) \ \cap\ \dom((G \cap G \circ NE) \setdiff NE
\circ G)
\subseteq \dom((G\setdiff G \circ NE) \ \cap\ (G \cap G \circ NE)). $$The
right-hand side is $\dom(\bot)$, so this simplifies to
$$ \dom(G\setdiff G \circ NE) \ \cap\ S_2 = \emptyset. \eqno(11) $$
Combining (10) and (11) gives
$$ \dom(G\setdiff G \circ NE) \ \cap\ S = \emptyset. \eqno(12) $$
Finally, given any $x,y$ such that $G(x,y)$ holds, either $(G \circ NE)(x,y)$
holds, in which case $x \notin S$ by (9), or $(G \circ NE)(x,y)$ does not hold,
in which case $y \notin S$ by (12). Thus $x \in N'$ or $y \in N'$.

\bigskip

\item{$(\epsilon)$} For every $x,y$ such that $(G\setdiff G')(x,y)$ holds,
either $x \in S$ or $y \in S$.

Proof. Using the definition $G' = G \ \cap\ G \circ NE \ \cap\ NE \circ G$,
$$ G\setdiff G'
= (G \setdiff G \circ NE) \ \cup\ ((G \cap G \circ NE) \setdiff NE \circ G)
$$
so if $(G\setdiff G')(x,y)$ then $x \in \ran(G \setdiff G \circ NE) = S_1$ or $y
\in \dom((G \cap G \circ NE) \setdiff NE \circ G) = S_2$; thus $x \in S$ or $y
\in S$.

By $(\delta)$, we cannot have both $x \in S$ and $y \in S$.

\bigskip

\item{$(\zeta)$} $\forall x\from S\ \exists y \from N'\ (G(x,y) \vee G(y,x))$.

Proof. Given $x\from S$, the existence of $y$ satisfying $G(x,y) \vee G(y,x)$ is
assured by $(\gamma)$, and it must be in $N'$ because of $(\delta)$.

\bigskip

\item{$(\eta)$} $\forall x,y\from N\ (G(x,y) \Rightarrow P(x)=P(y))$.

Proof. The hypothesis $\overline P \circ G \subseteq \overline P$ means
$$ \forall \sigma,y\ ((\overline P \circ G)(\sigma,y) \Rightarrow \overline
P(\sigma,y)) $$
which may be expanded to
$$ \forall \sigma,y\ (\exists x\ (\sigma=P(x) \wedge G(x,y)) \Rightarrow
\sigma=P(y)) $$
which is logically equivalent to
$$ \forall x,y\from N\ (G(x,y) \Rightarrow P(x)=P(y)) $$
since $\dom(P)=N$ and $G$ is on $N$.

\bigskip

\item{$(\theta)$} $\forall X \subseteq \Sigma\ |(G\setdiff G') \circ
id_{P\pre X}| = |S \cap P\pre X|$.

Proof. By $(\gamma)$ and $(\epsilon)$, there is a bijection $\omega$ between
pairs $(x,y)$ such that $(G\setdiff G')(x,y)$ holds and elements of $S$:
$$ \omega(x,y) = x \text{ or } y \text{, whichever one is in } S. $$
This gives $|G\setdiff G'| = |S|$. Moreover, for any $X \subseteq \Sigma$, and
any $x,y$ satisfying $(G\setdiff G')(x,y)$, $((G\setdiff G') \circ id_{P\pre
X})(x,y)$ iff $y \in P\pre X$ iff $x \in P\pre X$ (this is because $P(x)=P(y)$,
from $(\eta)$), so this in turn is equivalent to $\omega(x,y) \in P\pre X$. Thus
$\omega$ maps the pairs $(x,y)$ satisfying $((G\setdiff G') \circ id_{P\pre
X})(x,y)$ onto $S \cap P\pre X$. The conclusion follows.

\bigskip

\item{$(\iota)$} $G' \circ G' = \bot$.

Proof. This follows since $G' \subset G$ and $G \circ G = \bot$.

\bigskip

\item{$(\kappa)$} $G'$ is acyclic.

Proof. This follows from $G' \subset G$ by theorem~10.

\bigskip

\item{$(\lambda)$} $\overline{P'} \circ G' \subseteq \overline{P'}$.

Proof. We have $G' = G' \circ id_{N'}$, $\overline{P'} = \overline P \circ
id_{N'} \subseteq \overline P$, $G' \subset G$, and $\overline P \circ G
\subseteq \overline P$, so
$$ \overline{P'} \circ G'
= \overline{P'} \circ G' \circ id_{N'}
\subseteq \overline P \circ G \circ id_{N'}
\subseteq \overline P \circ id_{N'}
= \overline{P'}. $$

\bigskip

\item{$(\mu)$} $|G'| < |G|$.

Proof. This follows from $G' \subset G$.

\bigskip

\item{$(\nu)$} $\forall X\subseteq\Sigma\ |P'{}\pre X| - |G' \circ id_{P'{}\pre
X}| = |P\pre X| - |G \circ id_{P\pre X}|$.

Proof. We have $P'{}\pre X = P\pre X \cap N' = P\pre X \setdiff S$ and hence
$$ |P'{}\pre X| = |P\pre X| - |S \cap P\pre X|. $$
Also, $G' \circ id_{P'{}\pre X} = G' \circ id_{N'} \circ id_{P\pre X} = G' \circ
id_{P\pre X}$, since $G'$ is on $N'$, so
$$ |G' \circ id_{P'{}\pre X}|
= |G' \circ id_{P\pre X}|
= |G \circ id_{P\pre X}| - |(G\setdiff G') \circ id_{P\pre X}|
= |G \circ id_{P\pre X}| - |S \cap P\pre X|
$$
by $(\theta)$. Hence
$$ |P'{}\pre X| - |G' \circ id_{P'{}\pre X}|
= |P\pre X| - |G \circ id_{P\pre X}|. $$

\bigskip

\item{$(\xi)$} $P\pre X = \emptyset$ if $P'{}\pre X = \emptyset$.

Proof. I shall prove the contrapositive. If $P\pre X \ne \emptyset$ then there
exists $x \from N$ such that $P(x) \in X$. If $x \in N'$ then $x \in P'{}\pre
X$, whereas if $x \notin N'$ then $x \in S$, so by $(\zeta)$ there exists
$y\from N'$ such that $G(x,y)$ or $G(y,x)$. By $(\eta)$, $P(y)=P(x)\in X$, so $y
\in P'{}\pre X$. In either case, $P'{}\pre X \ne \emptyset$.

\bigskip

\item{$(\omicron)$} $P'(N') = P(N)$.

Proof. Recall that $P' = P|_{N'}$, so $P'(N') = P(N')$. By $(\zeta)$, for every
$x \from S$ there exists $y\from N'$ such that $G(x,y)$ or $G(y,x)$; by
$(\eta)$, this implies $P(x)=P(y)$. This shows that $P(S) \subseteq P(N')$.
Since $N = S \cup N'$, this gives $P(N) = P(S) \cup P(N') = P(N')$. Hence
$P'(N') = P(N)$.

\bigskip

\item{$(\pi)$} $G$ is connected relative to $P$ if $G'$ is connected
relative to $P'$.

Proof. Consider any set $Z$ and any function $Q:N \to Z$ such that $\overline Q
\circ G \subseteq \overline Q$. Define $Q'=Q|_{N'}:N'\to Z$, and note that
$$ \overline{Q'} \circ G'
= \overline{Q'} \circ G' \circ id_{N'}
\subseteq \overline Q \circ G \circ id_{N'}
\subseteq \overline Q \circ id_{N'}
= \overline{Q'}. $$
Assuming $G'$ is connected relative to $P'$, there exists a function
$i:P'(N')\to Z$ such that $i \circ P' = Q'$; this means that $i \circ P$ agrees
with $Q$ on $N'$. By $(\omicron)$, we have $i:P(N)\to Z$. Moreover I claim that
$i \circ P = Q$. For any $x \in S$, by $(\zeta)$ there exists $y\from N'$ such
that $G(x,y)$ or $G(y,x)$. Then $(\eta)$ gives $P(x)=P(y)$, and by similar
reasoning the hypothesis $\overline Q \circ G \subseteq \overline Q$ gives
$Q(x)=Q(y)$. Then
$$ i(P(x)) = i(P(y)) = Q(y) = Q(x). $$
So $i \circ P = Q$ holds on $S$ as well as on $N'$, i.e., it holds on the whole
of $N$. Thus we conclude that $i:P(N)\to Z$ and $i \circ P = Q$, as required.

\bigskip\f
Now we are ready to apply the induction step of the theorem. By $(\beta)$,
$(\iota)$--$(\mu)$, we can apply the inductive hypothesis to $N',P',G'$, and
thereby verify (i), (ii) and (iii) for $N,P,G$:

(i) for any $X \subseteq\Sigma$, applying $(\nu)$, $|P\pre X| - |G \circ
id_{P\pre X}| = |P'{}\pre X| - |G' \circ id_{P'{}\pre X}| \ge 0$ by inductive
hypothesis;

(ii) for any $X \subseteq\Sigma$, if $|P\pre X| - |G \circ id_{P\pre X}|=0$ then
$|P'{}\pre X| - |G' \circ id_{P'{}\pre X}|=0$ by $(\nu)$, so $P'{}\pre X =
\emptyset$ by inductive hypothesis, so $P\pre X = \emptyset$ by $(\xi)$;

(iii) if $\forall X \subseteq\Sigma\ |P\pre X| - |G \circ id_{P\pre X}| \le |X|$
then $\forall X \subseteq\Sigma\ |P'{}\pre X| - |G' \circ id_{P'{}\pre X}| \le
|X|$ by $(\nu)$, so $G'$ is connected relative to $P'$ by inductive hypothesis,
so $G$ is connected relative to $P$ by $(\pi)$.\qed

\subhead{2.4 Minimal relations relative to a function}

\defn If $f:X\to Y$ and $R$ is a relation on $X$ then $R$ is \i{minimal}
relative to $f$ iff
$$ \forall R^*\subseteq R\ \ (\overline f \circ R^* = \overline f \circ R
\Rightarrow R^* = R). $$

\medskip\f
(Informally, $R$ is minimal relative to $f$ iff, for any $x\from X$ and $y\from
Y$, there exists at most one $x'\from X$ such that $f(x')=y$ and $R(x',x)$.)

\theorem 14. If $f:X\to Y$ and $R$ is a relation on $X$ then $R$ is minimal
relative to $f$ iff
$$ \overline f\inv \circ \overline f \ \cap\ R \circ R\inv \subseteq id_X. $$

\proof $(\Rightarrow)$ Suppose $R$ is minimal relative to $f$. For any $x,x'$
such that $(\overline f\inv \circ \overline f \cap R \circ R\inv)(x,x')$, we
have $x,x'\in X$, $f(x)=f(x')$, and there exists $z$ such that $R(x,z)$ and
$R(x',z)$. Now suppose $x \ne x'$. Define a relation $R^*$ equal to $R$ except
that $R^*(x,z)$ does not hold. Thus $R^* \subset R$, but $\overline f \circ R^*
= \overline f \circ R$, since $(\overline f \circ R^*)(f(x),z)$ still holds (via
$x'$) and $\overline f \circ R^*$ is identical to $\overline f \circ R$ in all
other respects. The existence of $R^*$ contradicts the minimality of $R$. This
contradiction demonstrates that $x=x'$, as required.

$(\Leftarrow)$ Suppose $\overline f\inv \circ \overline f \cap R \circ R\inv
\subseteq id_X$. Consider any $R^*\subseteq R$ such that $\overline f \circ R^*
= \overline f \circ R$. Then
$$\eqqalign\quad{
R &= id_X \circ R \ \cap\ R
&\cr
&\subseteq \overline f\inv \circ \overline f \circ R \ \cap\ R
&\text{by theorem~2(ii)} \cr
&= \overline f\inv \circ \overline f \circ R^* \ \cap\ R
&\text{since $\overline f \circ R^* = \overline f \circ R$} \cr
&\subseteq (\overline f\inv \circ \overline f \ \cap\ R \circ {R^*}\inv) \circ
R^*
&\text{by theorem~4(i)} \cr
&\subseteq (\overline f\inv \circ \overline f \ \cap\ R \circ R\inv) \circ R^*
&\text{since $R^* \subseteq R$} \cr
&\subseteq id_X \circ R^*
&\text{since $\overline f\inv \circ \overline f \cap R \circ R\inv \subseteq
id_X$} \cr
&= R^*
&\cr
}$$
so $R^*=R$, as required. \qed

\vfill\supereject 
\input supp3
\vfill\supereject 
\def\Flex{\hbox{\i{Flex}}}

\runninghead{4. Embeddings and the definite match function}

\head{4. Embeddings and the Definite Match Function}

\subhead{4.1 Introduction}
The account of the recognition problem given in the previous sections has one
very obvious deficiency: it does not say what relation should hold between the
pattern and the image to make the pattern a good interpretation of the image.
Indeed, it does not make any use of the image at all, nor does it involve any
geometry.

In this section this deficiency will be rectified. Each symbol (and node) in the
pattern must be embedded in the image plane using an affine transformation; the
collection of all these affine transformations is called an \i{embedding token}.
The grammar imposes constraints on the embedding token, stipulating that if two
symbols are grammatically related then their embedding transformations must be
geometrically related; the collection of all these constraints is called an
\i{embedding type}. Embedding types make use of the concept of a \i{fleximap},
introduced in (2004, \S5).

The aim of recognition is to construct a definite pattern and embedding token
that \i{match}, or satisfy the constraints of, the image, the grammar and
embedding type. The degree of match is expressed by the \i{definite match
function} $DM$.

This section defines embedding tokens and types (slightly modifying the
definitions in (2004, \S6.4)), and the $DM$ function. It also refines the use 
of templates (introduced in (2004, \S4)), defines a symmetry of the grammar, and
demonstrates the affine invariance of the whole framework.

\subhead{4.2 Embedding tokens and types}
As in (2004), $\G$ is the group of affine transformations on the plane, a
six-dimensional Lie group. The composition or product of two affine 
transformations is written as $g \cdot g'$. Composition of two higher-level 
functions such as homomorphisms, embedding tokens or embedding types will be 
written using the \ic{$\circ$} symbol.

\defn An \i{embedding token} for a network $\network{}$ is a function
$u:\Sigma\cup N\to\G$ such that
$$ \forall n,n^* \from N\ (G(n,n^*) \Rightarrow u(n)=u(n^*)). $$

\medskip\f
The product $u_1 \cdot u_2$ of embedding tokens $u_1$ and $u_2$ is defined as in
(2004, \S6.4): 
$$ \forall x\from\Sigma\cup N\ (u_1 \cdot u_2)(x) = u_1(x)\cdot
u_2(x). $$
It follows immediately that $u_1 \cdot u_2$ is an embedding
token. As before we can also define the induced embedding token $u \circ f$ on
$\N'$, where $u$ is an embedding token on $\N$ and $f:\N'\to\N$ is a
homomorphism. However, we must check that $u \circ f$ satisfies the definition
of an embedding token, as follows.

\theorem 25. If $u$ is an embedding token for $\N$ and $f:\N'\to\N$ is a
homomorphism then $u \circ f$ is an embedding token for $\N'$.

\proof We shall use the notation $\N'=\network{'}$, $\N=\network{}$ and $u'=u
\circ f$. Clearly $u':\Sigma'\cup N' \to \G$. Consider any $n,n^* \from N'$ such
that $G'(n,n^*)$. We have $\overline f \circ G' = G \circ \overline f$, and
hence $G'(n,n^*)$ implies $(\overline f \circ G')(f(n),n^*)$, which implies $(G
\circ \overline f)(f(n),n^*)$, i.e., $G(f(n),f(n^*))$. Since $u$ is an embedding
token for $\N$ this implies $u(f(n))=u(f(n^*))$, i.e., $u'(n)=u'(n^*)$. Thus
$u'$ is an embedding token for $\N'$. \qed

\defn An \i{embedding type} for a network $\network{}$ is a sextuple
$(sub,\allowbreak con,\allowbreak rel,\allowbreak symm,\allowbreak tem,
\allowbreak in)$, in which $sub:\comp{(\sigma,\sigma^*) \from
\Sigma\times\Sigma}{G(\sigma,\sigma^*)} \to \Flex$, $con:N\to\Flex$,
$rel:E\to\Flex$, $symm:\Sigma\to Sub(\G)$, $tem:\Sigma\to Tem$, and
$in:\Sigma\to\Flex$ where $\Flex$ is the set of all fleximaps, $Sub(\G)$ is the
set of all subgroups of $\G$, and $Tem$ is the set of all templates; moreover,
for every $\sigma\in\Sigma$, the fleximap $in(\sigma)$ must have nominal part
equal to the identity transformation.

\medskip\f
This definition of embedding type is just as in (2004, \S6.4), except for the
presence of $sub$. The meaning of $sub$ is that if $\sigma^*$ is a subsymbol of
$\sigma$ then $sub(\sigma,\sigma^*)$ is a fleximap describing the relationship
between the embeddings of $\sigma^*$ and $\sigma$.

Embedding tokens are constrained by a symmetry condition. If $u$ is an embedding
token for $\N$ and $v$ is an embedding type for $\N$, where $\N=\network{}$, the
\i{symmetry condition} for $\N,u,v$ is
$$ \forall n\from N \quad u(P(n))\inv \cdot u(n) \in symm(P(n)). $$
This states that each node $n$ is embedded in the image plane in the same way as
the part $P(n)$, up to a symmetry of $P(n)$.

Given an embedding type $v=(sub_1,con_1,rel_1,symm_1,tem_1,in_1)$ and an
embedding token $u$ for a network $\network{}$, we can define an embedding type
$v \cdot u$ for the same network by $v \cdot u =
(sub_2,con_2,rel_2,symm_1,tem_2,in_2)$, where
$$\eqalign{
\forall \sigma,\sigma^* \from \Sigma \quad (G(\sigma,\sigma^*) \ \Rightarrow\
sub_2(\sigma,\sigma^*)
&= u(\sigma)\inv \cdot sub_1(\sigma,\sigma^*) \cdot u(\sigma^*)) \cr
\forall n\from N \quad con_2(n) &= u(W(n))\inv \cdot con_1(n) \cdot u(n) \cr
\forall e\from E \quad rel_2(e) &= u(A(S(e)))\inv \cdot rel_1(e) \cdot
u(A(F(e))) \cr
\forall \sigma\from\Sigma \quad tem_2(\sigma) &= tem_1(\sigma) \circ u(\sigma)
\cr
\forall \sigma\from\Sigma \quad
in_2(\sigma) &= u(\sigma)\inv \cdot in_1(\sigma) \cdot u(\sigma)
}$$

Given an embedding type $v=(sub,con,rel,symm,tem,in)$ for a network $\N$ and a
homomorphism $f:\N'\to\N$, there is an induced embedding type $v \circ f$ for
$\N'$ defined by
$$ v \circ f
= (sub',con \circ f,rel \circ f,symm \circ f,tem \circ f,in \circ f). $$
where
$$ \forall \sigma,\sigma^*\from\Sigma \quad (G(\sigma,\sigma^*) \ \Rightarrow\
sub'(\sigma,\sigma^*) = sub(f(\sigma),f(\sigma^*))). $$

\theorem 26. (Lemma~1 of (2004, \S6.4)) If $f:\N'\to\N$ is a
homomorphism, $v$ is an embedding type for $\N$, and $u$ is an embedding token
for $\N$, then
$$ (v \cdot u) \circ f = (v \circ f) \cdot (u \circ f). $$

\proof The proof is a slightly adapted version of the one in (2004, \S6.4).
Let $\N'=\network{'}$, $\N=\network{}$ and $v = (sub_1,\allowbreak con_1,
\allowbreak rel_1, \allowbreak symm_1, \allowbreak tem_1, \allowbreak in_1)$.
Then $v \cdot u = (sub_2, con_2, rel_2, symm_1, tem_2, in_2)$, where
$$\eqalign{
\forall \sigma,\sigma^* \from \Sigma \quad (G(\sigma,\sigma^*) \ \Rightarrow\
sub_2(\sigma,\sigma^*)
&= u(\sigma)\inv \cdot sub_1(\sigma,\sigma^*) \cdot u(\sigma^*))
\cr
\forall n\from N \quad con_2(n) &= u(W(n))\inv \cdot con_1(n) \cdot u(n)
\cr
\forall e\from E \quad rel_2(e) &= u(A(S(e)))\inv \cdot rel_1(e) \cdot
u(A(F(e))) \cr
\forall \sigma\from\Sigma \quad tem_2(\sigma) &= tem_1(\sigma) \circ
u(\sigma)
\cr
\forall \sigma\from\Sigma \quad in_2(\sigma)
&= u(\sigma)\inv \cdot in_1(\sigma) \cdot u(\sigma)
}$$
and hence
$$ (v \cdot u) \circ f =
(sub', con_2\circ f, rel_2\circ f, symm_1\circ f, tem_2\circ f, in_2\circ f) $$
where
$$ \forall \sigma,\sigma^*\from\Sigma' \quad (G'(\sigma,\sigma^*) \ \Rightarrow\
sub'(\sigma,\sigma^*) = sub_2(f(\sigma),f(\sigma^*))). $$

We also have $v\circ f = (sub'', con_1\circ f, rel_1\circ f, symm_1\circ f,
tem_1\circ f, in_1\circ f)$, where
$$ \forall \sigma,\sigma^*\from\Sigma' \quad (G'(\sigma,\sigma^*) \ \Rightarrow\
sub''(\sigma,\sigma^*) = sub_1(f(\sigma),f(\sigma^*))). $$
Hence $(v\circ f) \cdot (u\circ f) = (sub_3, con_3, rel_3, symm_1\circ f, tem_3,
in_3)$, where
$$\eqalign{
\forall \sigma,\sigma^*\from\Sigma' \quad (G'(\sigma,\sigma^*) \ \Rightarrow \
sub_3(\sigma,\sigma^*)
&= (u \circ f)(\sigma)\inv \cdot sub''(\sigma,\sigma^*) \cdot
(u \circ f)(\sigma^*) \cr
&= u(f(\sigma))\inv \cdot sub_1(f(\sigma),f(\sigma^*)) \cdot
u(f(\sigma^*)) \cr
&= sub_2(f(\sigma), f(\sigma^*))
= sub'(\sigma,\sigma^*))
\cr
\forall n\from N' \quad con_3(n)
&= (u\circ f)(W'(n))\inv \cdot (con_1\circ f)(n) \cdot (u\circ f)(n) \cr
&= u(f(W'(n)))\inv \cdot con_1(f(n)) \cdot u(f(n)) \cr
&= u(W(f(n)))\inv \cdot con_1(f(n)) \cdot u(f(n)) \cr
&= con_2(f(n)) = (con_2 \circ f)(n) \cr
\forall e\from E' \quad
rel_3(e) &=
(u\circ f)(A'(S'(e)))\inv \cdot (rel_1\circ f)(e) \cdot (u\circ f)(A'(F'(e)))
\cr
&= u(f(A'(S'(e))))\inv \cdot rel_1(f(e)) \cdot u(f(A'(F'(e)))) \cr
&= u(A(S(f(e))))\inv \cdot rel_1(f(e)) \cdot u(A(F(f(e)))) \cr
&= rel_2(f(e)) = (rel_2 \circ f)(e) \cr
\forall \sigma\from\Sigma' \quad
tem_3(\sigma) &= (tem_1\circ f)(\sigma) \circ (u\circ f)(\sigma) \cr
&= tem_1(f(\sigma)) \circ u(f(\sigma)) \cr
&= tem_2(f(\sigma)) = (tem_2 \circ f)(\sigma) \cr
\forall \sigma\from\Sigma' \quad
in_3(\sigma)
&= (u\circ f)(\sigma)\inv \cdot (in_1\circ f)(\sigma) \cdot (u\circ f)(\sigma)
\cr
&= u(f(\sigma))\inv \cdot in_1(f(\sigma)) \cdot u(f(\sigma)) \cr
&= in_2(f(\sigma)) = (in_2 \circ f)(\sigma)
}$$
which shows that $(v \cdot u) \circ f= (v\circ f) \cdot (u\circ f)$. \qed

\defn If $\N'=\network{'}$ is a subnetwork of $\N$, with 
inclusion homomorphism $f:\N'\to\N$,

\item{(i)} the \i{restriction} of $u$, an embedding token for $\N$, to $\N'$,
denoted $u|_{\N'}$, is defined as $u \circ f = u|_{\Sigma'\cup N'}$; this
is an embedding token for $\N'$ by theorem~25;

\item{(ii)} the \i{restriction} of $v$, an embedding type for $\N$, to $\N'$,
denoted $v|_{\N'}$, is defined as $v \circ f$, an embedding type for $\N'$.

\subhead{4.3 Symmetries}

\defn A \i{symmetry} of a network $\N=\network{}$, with respect to the embedding
type $v=(sub,con,rel,symm,tem,in)$, is a pair $(a,s)$, where $a:\N\to\N$ is an
automorphism of $\N$ and $s$ is an embedding token for $\N$, such that

\blob $\forall \sigma\from\Sigma \ s(\sigma) \in symm(\sigma)$,

\blob $\forall n\from N \ s(n) \in symm(P(n))$,

\blob $v \cdot s = v \circ a$.

\medskip\f
This is just as in (2004, \S7.5). However, the operation of global application
of a symmetry of the grammar to the pattern, in lemma~2, needs to be
generalised to \i{local} symmetries, in which different symmetries are applied
to different symbols of the pattern

\defn Given networks $\N_1=\network{_1}$ and $\N_0=\network{_0}$, a homomorphism
$p:\N_1\to\N_0$, and an embedding token $v$ on $\N_0$, define $\Cal S_0$ as the
group of symmetries of $\N_0$ with respect to $v$. A \i{local symmetry} of
$\N_1$ with respect to $\N_0,p,v$ is a function $\pi:\Sigma_1 \to \Cal S_0$ such
that

\blob $\forall \sigma,\sigma^*\from\Sigma_1\ (G_1(\sigma,\sigma^*) \Rightarrow
\pi(\sigma)=\pi(\sigma^*))$,

\blob $\forall e\from E_1\ \pi(W_1(A_1(F_1(e)))) = \pi(W_1(A_1(S_1(e))))$,

\blob $\forall n \from N_1\ a(P_1(n))(p(P_1(n))) = a(W_1(n))(p(P_1(n)))$,

\medskip\f
where $\pi$ is decomposed into components by $\forall\sigma\from\Sigma_1\
\pi(\sigma) = (a(\sigma),s(\sigma))$, for functions $a,s$.

\medskip\f
Given a local symmetry $\pi$ and an embedding token $u$ for $\N_1$, the
\i{application of $\pi$ to $p,u$} produces a new homomorphism $p':\N_1\to\N_0$,
defined by
$$\eqalign{
&\forall \sigma\from\Sigma_1 \cr
&\forall n\from N_1 \cr
&\forall h\from H_1 \cr
&\forall e\from E_1 \cr
&\forall k\from K_1 \cr
}\ \ \eqalign{
p'(\sigma) &= a(\sigma)(p(\sigma)) \cr
p'(n) &= a(W_1(n))(p(n)) \cr
p'(h) &= a(W_1(A_1(h)))(p(h)) \cr
p'(e) &= a(W_1(A_1(F_1(e))))(p(e)) \cr
p'(k) &= a(W_1(A_1(F_1(C_1(k)))))(p(k)), \cr
}$$
and a new embedding token $u'=u \cdot s'$ for $\N_1$, where the embedding token
$s'$ is defined by
$$\eqalign{
&\forall \sigma\from\Sigma_1 \cr
&\forall n\from N_1
}\ \ \eqalign{
s'(\sigma) &= s(\sigma)(p(\sigma)) \cr
s'(n) &= s(W_1(n))(p(n)).
}$$

\theorem 27. In the above definition, $p':\N_1\to\N_0$ is a homomorphism and
$s',u'$ are embedding tokens for $\N_1$, as claimed.

\proof We shall continue to use the above notation.

First we verify that $p':\N_1\to\N_0$ is a homomorphism. The conditions
$$ p'(\Sigma_1) \subseteq \Sigma_0, \quad p'(N_1) \subseteq N_0, \quad
p'(H_1) \subseteq H_0, \quad p'(E_1) \subseteq E_0, \quad p'(K_1) \subseteq
K_0 $$
are immediate.

Next we check $W_0 \circ p' = p' \circ W_1$:
$$\eqqalign\quad{
\forall n\from N_1\quad W_0(p'(n))
&= W_0\bigl(a(W_1(n))(p(n))\bigr)
&\cr
&= a(W_1(n))\bigl(W_0(p(n))\bigr)
&\text{since $a(W_1(n))$ is an automorphism}\cr
&= a(W_1(n))\bigl(p(W_1(n))\bigr)
&\text{since $p$ is an homomorphism}\cr
&= p'(W_1(n)),
&\cr
}$$
$$ \forall \sigma\from\Sigma_1\quad W_0(p'(\sigma))
= p'(\sigma)
= p'(W_1(\sigma)). \kern150pt $$
Next we check $P_0 \circ p' = p' \circ P_1$:
$$\eqqalign\quad{
\forall n\from N_1 \quad P_0(p'(n))
&= P_0\bigl(a(W_1(n))(p(n))\bigr)
&\cr
&= a(W_1(n))\bigl(P_0(p(n))\bigr)
&\text{since $a(W_1(n))$ is an automorphism}\cr
&= a(W_1(n))\bigl(p(P_1(n))\bigr)
&\text{since $p$ is an homomorphism}\cr
&= a(P_1(n))\bigl(p(P_1(n))\bigr)
&\text{since $\pi$ is a local symmetry}\cr
&= p'(P_1(n)).
&\cr
}$$
Next we check $F_0 \circ p' = p' \circ F_1$:
$$\eqqalign\quad{
\forall e\from E_1 \quad F_0(p'(e))
&= F_0\bigl(a(W_1(A_1(F_1(e))))(p(e))\bigr)
&\cr
&= a(W_1(A_1(F_1(e))))\bigl(F_0(p(e))\bigr)
&\text{since $a(W_1(A_1(F_1(e))))$ is an automorphism}\cr
&= a(W_1(A_1(F_1(e))))\bigl(p(F_1(e))\bigr)
&\text{since $p$ is a homomorphism}\cr
&= p'(F_1(e)).
&\cr
}$$
Next we check $S_0 \circ p' = p' \circ S_1$:
$$\eqqalign\quad{
\forall e\from E_1 \quad S_0(p'(e))
&= S_0\bigl(a(W_1(A_1(F_1(e))))(p(e))\bigr)
&\cr
&= a(W_1(A_1(F_1(e))))\bigl(S_0(p(e))\bigr)
&\text{since $a(W_1(A_1(F_1(e))))$ is an automorphism}\cr
&= a(W_1(A_1(F_1(e))))\bigl(p(S_1(e))\bigr)
&\text{since $p$ is a homomorphism}\cr
&= a(W_1(A_1(S_1(e))))\bigl(p(S_1(e))\bigr)
&\text{since $\pi$ is a local symmetry}\cr
&= p'(S_1(e)).
&\cr
}$$
Next we check that $\rectangleA{N_0\cup\Sigma_0}{N_1\cup\Sigma_1}{H_0}{H_1}
{p'|_{N_1\cup\Sigma_1}}{A_0}{A_1}{p'|_{H_1}}$ is a pullback in the category of
sets. The equation $A_0 \circ p'|_{H_1} = p'|_{N_1\cup\Sigma_1} \circ A_1$
follows by
$$\eqqalign\quad{
\forall h\from H_1\quad A_0(p'(h))
&= A_0\bigl(a(W_1(A_1(h)))(p(h))\bigr)
&\cr
&= a(W_1(A_1(h)))\bigl(A_0(p(h))\bigr)
&\text{since $a(W_1(A_1(h)))$ is an automorphism}\cr
&= a(W_1(A_1(h)))\bigl(p(A_1(h))\bigr)
&\text{since $p$ is an homomorphism}\cr
&= p'(A_1(h)).
&\cr
}$$
The other half of the pullback condition is
$$ \forall h_0\from H_0\ \forall x_1\from N_1\cup\Sigma_1 \quad
(A_0(h_0) = p'(x_1) \ \Rightarrow\ \exists!h_1\from H_1\ (A_1(h_1)=x_1 \wedge
p'(h_1)=h_0)). \eqno (1) $$
To prove this, consider any $h_0\from H_0$ and any $x_1\from N_1\cup\Sigma_1$.
Define $a^*=a(W_1(x_1))$, an automorphism of $\N_0$. By theorem~15, $a^* \circ
p:\N_1\to\N_0$ is a homomorphism, so the pullback
$\longrectangleA{N_0\cup\Sigma_0}{N_1\cup\Sigma_1}{H_0}{H_1} {(a^*\circ
p)|_{N_1\cup\Sigma_1}}{A_0}{A_1}{(a^*\circ p)|_{H_1}}$ implies
$$ A_0(h_0) = a^*(p(x_1)) \ \Rightarrow\
\exists!h_1\from H_1\ (A_1(h_1)=x_1 \wedge a^*(p(h_1))=h_0). \eqno (2) $$
Now, $p'(x_1) = a^*(p(x_1))$; and, for any $h_1\from H_1$, if $A_1(h_1)=x_1$
then $p'(h_1) = a(W_1(A_1(h_1)))(p(h_1)) = a^*(p(h_1))$. Thus (2) may be
rewritten, and quantifiers over $h_0$ and $x_1$ added, to give (1). This
completes the proof of the pullback.

The pullback $\rectangleA{E_0}{E_1}{K_0}{K_1}{p'|_{E_1}}{C_0}{C_1}{p'|_{K_1}}$
is verified similarly.

Next we check that $G_0 \circ \overline{p'} = \overline{p'} \circ G_1$ and $G_1$
is minimal relative to $p'$. Let us restrict our attention to nodes in the first
instance. In view of theorem~14, we have to show
$$\eqalign{
&\forall n_0\from N_0\ \forall n_1^*\from N_1\ \ 
(G_0(n_0,p'(n_1^*)) \ \Leftrightarrow\
\exists n_1\from N_1\ (n_0 = p'(n_1) \wedge G_1(n_1,n_1^*))); \cr
&\forall n_0\from N_0\ \forall n_1^*\from N_1\ \ 
\exists^{\le1} n_1\from N_1\ (n_0 = p'(n_1) \wedge G_1(n_1,n_1^*)).}
\eqno(3) $$
To prove these, consider any $n_0\from N_0$ and any $n_1^*\from N_1$. Define
$a^*=a(W_1(n_1^*))$, an automorphism of $\N_0$. By theorem~15, $a^* \circ
p:\N_1\to\N_0$ is a homomorphism, so
$$\eqalign{
&G_0(n_0,a^*(p(n_1^*))) \ \Leftrightarrow\
\exists n_1\from N_1\ (n_0 = a^*(p(n_1)) \wedge G_1(n_1,n_1^*)); \cr
&\exists^{\le1} n_1\from N_1\ (n_0 = a^*(p(n_1)) \wedge G_1(n_1,n_1^*)).}
\eqno(4) $$
Now, the condition $G_0(n_0,a^*(p(n_1^*)))$ is equivalent to
$G_0(n_0,p'(n_1^*))$, since $a^*(p(n_1^*)) = p'(n_1^*)$. Moreover, for any
$n_1\from N_1$, if $G_1(n_1,n_1^*)$ then $G_1(W_1(n_1),W_1(n_1^*))$, by
$\overline{W_1} \circ G_1 \subseteq G_1 \circ \overline{W_1}$, so
$\pi(W_1(n_1))=\pi(W_1(n_1^*))$, so $a(W_1(n_1))=a(W_1(n_1^*))=a^*$, so $p'(n_1)
= a(W_1(n_1))(p(n_1)) = a^*(p(n_1))$. Thus the condition $n_0 = a^*(p(n_1))
\wedge G_1(n_1,n_1^*)$ is equivalent to $n_0 = p'(n_1) \wedge G_1(n_1,n_1^*)$.
Hence (4) may be rewritten (quantifying over $n_0$ and $n_1^*$) as (3), as
required. This deals with the node case. Statements similar to (3) for symbols,
hooks, edges and facets can be proved in the same way, completing the proof that
$G_0 \circ \overline{p'} = \overline{p'} \circ G_1$ and $G_1$ is minimal
relative to $p'$.

This completes the proof that $p':\N_1\to\N_0$ is a homomorphism.

Next we verify that $s'$ is an embedding token for $\N_1$. Consider any
$n,n^*\from N_1$ such that $G_1(n,n^*)$ holds. We must show that
$s'(n)=s'(n^*)$.

First, $\pi(W_1(n))$ is a symmetry of $\N_0$, so $s(W_1(n))$ is an embedding
token for $\N_0$; moreover, $G_0(p(n),p(n^*))$ holds; so $s(W_1(n))(p(n)) =
s(W_1(n))(p(n^*))$.

Secondly, we have $G_1(W_1(n),W_1(n^*))$, so $\pi(W_1(n))=\pi(W_1(n^*))$, so
$s(W_1(n))=s(W_1(n^*))$.

Putting these two observations together,
$$ s'(n) = s(W_1(n))(p(n)) = s(W_1(n))(p(n^*)) = s(W_1(n^*))(p(n^*)) = s'(n^*)
$$
as required. It follows now that $u' = u \cdot s'$ is an embedding token for
$\N_1$. \qed

\subhead{4.4 Templates and saturation}
The concepts of an image, a template, and the correlation function $\rho_{I,T}$
are carried over from (2004, \S 4), with two modifications.

The first modification is intended to prevent two identical symbol tokens from
forming at the same place in the image, or more generally to prevent two or
more symbol tokens from claiming credit for the same patch of the image. If two
or more symbol tokens' templates overlap in the image plane, i.e., if there are
points $x$ in the image plane where $tem(\sigma)(u(\sigma)\inv(x)) > 0$ for two
or more symbol tokens $\sigma$, then the point $x$ should become \i{saturated}
and the contribution it makes to the correlation function should be reduced.
For this it is necessary to calculate the saturation $sat(x)$ of each point
$x$, which is roughly the sum of $tem(\sigma)(u(\sigma)\inv(x))$ over each
symbol token $\sigma$. (However, this needs modification for subsymbols to
avoid double-counting.) The formal definition of saturation follows.

Suppose we are given a definite network $\N=\network{}$, an embedding token $u$ for $\N$,
and a function $tem:\Sigma\to Tem$. The \i{(definite) saturation function}, 
$sat:\R^2\to\R$, is defined by
$$ \forall x\from\R^2\quad
sat(x) = \sum_{\sigma\in\Sigma} (1-g_\sigma) \, tem(\sigma)(u(\sigma)\inv(x)) $$
where $g_\sigma = \bigl|\comp{\sigma^*\from\Sigma}{G(\sigma^*,\sigma)}\bigr|$.
We call $sat(x)$ the \i{saturation at} $x$.

The correlation function $\rho_{I,T}$, between an image $I$ and a template $T$,
was defined in (2004, \S4.2) by
$$ \rho_{I,T}(g) = |det(\rep g)| \int T(u) \, (I(g(u))-I_0) \d^2u =
\int T(g\inv(x)) \, (I(x)-I_0) \d^2x $$
for any affine transformation $g$, where $\rep g$ is the matrix representation
of $g$ and $I_0$ is a positive real constant associated with $T$. This must now
be modified to take account of saturation:
$$ \rho_{I,T,sat}(g)
= |det(\rep g)| \int w(sat(g(u))) \, T(u) \, (I(g(u))-I_0) \d^2u
= \int w(sat(x)) \, T(g\inv(x)) \, (I(x)-I_0) \d^2x $$
where $w$ is a weighting function that suppresses the integrand at points $x$
where $sat(x)$ is above 1. A suitable definition of $w$ is
$$ \forall s\from\R\quad w(s) =
\cases{
1 & if $s \le 1$, \cr
(1.6-s)/0.6 & if $1 < s < 1.6$, \cr
0 & if $1.6 \le s$.
}$$

The second modification is to give the factor of $|\det(\rep g)|$ that
occurs in the formula for $\rho_{I,T,sat}(g)$ an adjustable exponent:
$$\eqalign{
\rho_{I,T,sat}(g)
&= |det(\rep g)|^{1-k} \int w(sat(g(u))) \, T(u) \, (I(g(u))-I_0) \d^2u \cr
&= |\det(\rep g)|^{-k} \int w(sat(x)) \, T(g\inv(x)) \, (I(x)-I_0) \d^2x
}$$
where $k$ is a constant characteristic of the template, with $0 \le k \le 1$
normally. 

\def\I{\Bbb I}
\def\intx#1{\int w(sat(x)) \, #1 \d^2x}
\def\intu#1{\int w(sat(g(u))) \, #1 \d^2u}

The calculation of template force in (2004, \S4.3) is affected by these two
changes as follows. For any $g\from\G$ and $A\from\A$,
$$\eqalign{
\rho_{I,T,sat}(g \cdot \exp A) 
&= |\det(\rep{g\cdot\exp A})|^{-k} \intx{T((g\cdot \exp A)\inv(x))(I(x)-I_0)}
\cr
&= |\det(\rep g\cdot\exp\rep A)|^{-k} \intx{\rep T((\rep g \exp\rep A)\inv\rep x)(I(x)-I_0)}
\cr
&= |\det(\rep g)|^{-k} e^{-k\tr(\rep A)} \intx{\rep T(\exp(-\rep A)\rep g\inv\rep x)(I(x)-I_0)}
\cr
&= |\det(\rep g)|^{-k} (\I-k\tr(\rep A) + o(A)) \kern-2pt \intx{\rep T((\I-\rep A+o(A))\rep g\inv\rep x)(I(x)-I_0)}
\cr
&= |\det(\rep g)|^{-k} (\I-k\tr(\rep A) + o(A)) \cdot
\cr&
\hskip63pt \intx{\bigl(\rep T(\rep g\inv\rep x) - (\rep\nabla T(g\inv x))\rep
A\rep g\inv\rep x + o(A)\bigr)(I(x)-I_0)}
\cr
&= \rho_{I,T,sat}(g) - k\tr(\rep A)\rho_{I,T,sat}(g)
\cr&\kern59pt 
- |\det(\rep g)|^{-k} \intx{\bigl((\rep\nabla T(g\inv x))\rep A\rep g\inv\rep
x\bigr)(I(x)-I_0)} + o(A)
}$$
where $\I$ is the $6\times6$ identity matrix.
Hence the derivative $\rho_{I,T,sat*}:\G \to (\A \to \R)$ is defined by
$$\eqalign{
\forall g\from\G\ \forall A\from\A\ \ \rho_{I,T,sat*}(g)(A) 
=& - k\tr(\rep A)\rho_{I,T,sat}(g)
\cr
& - |\det(\rep g)|^{-k} \intx{\bigl((\rep\nabla T(g\inv x))\rep A\rep g\inv\rep
x\bigr)(I(x)-I_0)} 
\cr
=& - k\tr(\rep A)\rho_{I,T,sat}(g)
\cr
& - |\det(\rep g)|^{1-k} \intu{\bigl((\rep\nabla T(u))\rep A\rep
u\bigr)(I(g(u))-I_0)}. 
}$$
This gives a matrix representation for the force,
$$\eqalign{
\forall g\from\G\ \ \rep{\rho_{I,T,sat*}(g)} 
=& 
- k\rho_{I,T,sat}(g)\I
- |\det(\rep g)|^{-k} \intx{\bigl(\rep g\inv \rep x(\rep\nabla
T(g\inv(x)))\bigr)(I(x)-I_0)}
\cr
=& 
- k\rho_{I,T,sat}(g)\I
- |\det(\rep g)|^{1-k} \intu{\bigl(\rep u(\rep\nabla T(u))\bigr)(I(g(u))-I_0)}.
}$$

\subhead{4.5 The definite match function}
The \i{definite match function} $DM$ measures how well a definite network
$\N=\network{}$ matches an image $I$, given an embedding token $u$ for $\N$, and
an embedding type $v=(sub,con,rel,symm,tem,in)$ for $\N$. It is defined by
$$\eqalign{
DM(I, \N, u, v)
=& \sum_{\sigma\in\Sigma} \rho_{I,tem(\sigma),sat}(u(\sigma))
\ - \ \theta |\Sigma\setdiff P(N)|
\ - \sum_{(\sigma,\sigma^*)\mid G(\sigma,\sigma^*)} \kern-15pt
E_{sub(\sigma,\sigma^*)}\bigl(u(\sigma)\inv \cdot u(\sigma^*)\bigr)
\cr&
\ - \ \sum_{n\in N} E_{con(n)}\bigl(u(W(n))\inv \cdot u(n)\bigr)
\ - \ \sum_{e\in E} E_{rel(e)}\bigl(u(A(S(e)))\inv \cdot u(A(F(e)))\bigr)
}$$
where $\theta$ is a positive real constant and $sat$ is the definite saturation
function, as defined in the previous section. 

The first term on the right-hand side is a sum over all symbols; $tem(\sigma)$
is the template for $\sigma$, and $\rho_{I,tem(\sigma),sat}(u(\sigma))$
measures the correlation between the template (embedded in the image using
$u(\sigma)$) and the image $I$.

The second term on the right-hand side applies a fixed penalty of $\theta$ for
each \ic{bare} symbol, i.e., each symbol that is not a part of another symbol.
This term encourages the symbols to connect themselves together rather than
remaining separate.

The third term measures how well each subsymbol matches its supersymbol
geometrically. The summation is over all pairs $(\sigma,\sigma^*)$ such that
$\sigma$ is a supersymbol of $\sigma^*$; $sub(\sigma,\sigma^*)$ is a fleximap
that defines what the geometric relationship between $\sigma^*$ and $\sigma$
should be; $u(\sigma)\inv \cdot u(\sigma^*)$ is the actual relationship between
them; the quadratic penalty function $E_\tau(G)$ calculates the penalty for the
deviation between an affine transformation $G$ and a fleximap $\tau$, as
defined in (2004, \S5.3).

The fourth term measures how well each part matches its whole geometrically. The summation
is over all nodes $n$; $P(n)$ is the part symbol and $W(n)$ is the whole
symbol. The node $n$ has its own embedding $u(n)$, which equals $u(P(n))$ up
to a symmetry; $u(W(n))\inv \cdot u(n)$ is the actual geometric relationship
between the part (or rather the node) and the whole; $con(n)$ is a fleximap
specifying what the relationship should be.

The final term measures how well each pair of siblings match geometrically.
The sum is over every edge $e$, representing a sibling relationship between two
nodes $A(F(e))$ and $A(S(e))$; $u(A(S(e)))\inv \cdot u(A(F(e)))$ is the actual
relationship and $rel(e)$ is the fleximap specifying what the relationship
should be.

All these fleximaps are provided by the embedding type $v$; the final
component $in$ of $v$ is not used yet.

The way $DM$ will be used in the statement of the recognition problem is as
follows. An embedding type $v$ for the grammar $\N_0$ is given at the outset.
The parsing homomorphism $p:\N_1\to\N_0$ induces an embedding type $v\circ p$
for $\N_1$. An embedding token $u$ for $\N_1$ is constructed by the parser,
satisfying the symmetry condition for $\N_1,u,v\circ p$. At the end of recognition,
when $\N_1$ is definite, we measure how well $u$ matches $v \circ p$ by
calculating $DM(I,\N_1,u,v\circ p)$.

\subhead{4.6 Invariance theorems}
Lemmas~1 and 2 from (2004, \S7) hold for the definite match function $DM$;
I shall restate them here, but with lemma~2 generalised from global symmetries
to local symmetries. I shall also add two new theorems on the affine invariance
of the $\rho$ and match functions.

\theorem 28. (Lemma~1 of (2004, \S7.3): invariance under affine transformation
of the symbols' internal frames of reference.) For any image $I$, definite
network $\N$,
embedding tokens $u,u'$ for $\N$, and embedding type $v$ for $\N$, then
$$ DM(I, \N, u\cdot u', v\cdot u') = DM(I, \N, u, v); $$

\proof The proof is very similar to the one in (2004), but I shall restate it in
full. Let $v=(sub_1, con_1, \allowbreak rel_1, \allowbreak symm_1, tem_1,in_1)$;
then $v\cdot u'=(sub_2, con_2,rel_2,symm_1,tem_2,in_2)$, where
$$\eqalign{
\forall \sigma,\sigma^* \from \Sigma \quad (G(\sigma,\sigma^*) \ \Rightarrow\
sub_2(\sigma,\sigma^*)
&= u'(\sigma)\inv \cdot sub_1(\sigma,\sigma^*) \cdot u'(\sigma^*))
\cr
\forall n\from N \quad con_2(n) &= u'(W(n))\inv \cdot con_1(n) \cdot u'(n)
\cr
\forall e\from E \quad rel_2(e) &= u'(A(S(e)))\inv \cdot rel_1(e) \cdot
u'(A(F(e))) \cr
\forall \sigma\from\Sigma \quad tem_2(\sigma) &= tem_1(\sigma) \circ
u'(\sigma)
\cr
\forall \sigma\from\Sigma \quad
in_2(\sigma) &= u'(\sigma)\inv \cdot in_1(\sigma) \cdot u'(\sigma)
}$$
Now, first, for any $\sigma\from\Sigma$,
$$ \rho_{I,tem_2(\sigma),sat}((u\cdot u')(\sigma))
= \rho_{I,tem_1(\sigma)\circ u'(\sigma),sat}(u(\sigma)\cdot u'(\sigma))
= \rho_{I,tem_1(\sigma),sat}(u(\sigma)) $$
using lemma~1 of (2004, \S4.2). Note that the saturation function $sat$ is
unchanged by the application of $u'$. This is because
$$ \forall \sigma\from\Sigma\ \forall x\from\R^2\quad\!\!
tem_2(\sigma)((u\cdot u')(\sigma)\inv(x))
= (tem_1(\sigma) \circ u'(\sigma))(u'(\sigma)\inv(u(\sigma)\inv(x)))
= tem_1(\sigma)(u(\sigma)\inv(x)) $$
and so the calculation of $sat(x)$ is unaffected.

Secondly, for any $\sigma,\sigma^* \from \Sigma$ such that $G(\sigma,\sigma^*)$,
$$\eqalign{
E_{sub_2(\sigma,\sigma^*)}((u\cdot u')(\sigma)\inv \cdot (u\cdot u')(\sigma^*))
&=
E_{u'(\sigma)\inv \cdot sub_1(\sigma,\sigma^*) \cdot u'(\sigma^*)}
(u'(\sigma)\inv \cdot u(\sigma)\inv \cdot u(\sigma^*) \cdot u'(\sigma^*))
\cr&
= E_{sub_1(\sigma,\sigma^*)}(u(\sigma)\inv \cdot u(\sigma^*))
}$$
by lemma~1 of (2004, \S5.3).

Thirdly, for any $n\from N$,
$$\eqalign{
E_{con_2(n)}((u\cdot u')&(W(n))\inv \cdot (u\cdot u')(n))
\cr&
= E_{u'(W(n))\inv \cdot con_1(n) \cdot u'(n)}
(u'(W(n))\inv \cdot u(W(n))\inv \cdot u(n) \cdot u'(n))
\cr&
= E_{con_1(n)}(u(W(n))\inv \cdot u(n))
}$$
by lemma~1 of (2004, \S5.3).

Fourthly, for any $e\from E$, using the abbreviations $n_1=A(F(e))$ and
$n_2=A(S(e))$,
$$\eqalign{
E_{rel_2(e)}((u\cdot u')(n_2)\inv \cdot (u\cdot u')(n_1))
&=E_{u'(n_2)\inv \cdot rel_1(e) \cdot u'(n_1)}
(u'(n_2)\inv \cdot u(n_2)\inv \cdot u(n_1) \cdot u'(n_1))
\cr&
= E_{rel_1(e)}(u(n_2)\inv \cdot u(n_1))
}$$
and, using the abbreviations $\sigma_1=W(A(F(e)))$ and $\sigma_2=W(A(S(e)))$,
$$\eqalign{
E_{in_2(\sigma_1)}((u\cdot u')(\sigma_2)\inv \cdot (u\cdot u')(\sigma_1))
&= E_{u'(\sigma_1)\inv \cdot in_1(\sigma_1) \cdot u'(\sigma_1)}
(u'(\sigma_2)\inv \cdot u(\sigma_2)\inv \cdot
u(\sigma_1) \cdot u'(\sigma_1))
\cr&
= E_{in_1(\sigma_1)}(u(\sigma_2)\inv \cdot u(\sigma_1))
}$$
by lemma~1 of (2004, \S5.3) again, using the assumption that $u'(\sigma_1) =
u'(\sigma_2)$ (which holds under the conditions of (i) or (ii)).

Thus each term of $DM(I, \N, u\cdot u', v\cdot u')$ equals the corresponding
term of $DM(I, \N, u, v)$. \qed

\theorem 29. (Invariance of $DM$ under a local symmetry.) Given
an image $I$, a semi-definite network $\N_0$, a definite network $\N_1$, 
a homomorphism
$p:\N_1\to\N_0$, an embedding token $u$ for $\N_1$, an embedding type $v$ for
$\N_0$, and a local symmetry $\pi$ of $\N_1$ with respect to $\N_0,p,v$, the
application of $\pi$ to $p,u$ produces a homomorphism $p':\N_1\to\N_0$ and an
embedding token $u'$ for $\N_1$.

Then 

(i) $DM(I, \N_1, u', v\circ p') = DM(I, \N_1, u, v\circ p)$,

(ii) The symmetry condition holds for $\N_1,u',v \circ p'$ iff it holds for
$\N_1,u,v \circ p$.

\proof We begin by recapitulating the relevant definitions and notation. Define
functions $a,s$ by $\forall\sigma\from\Sigma_1\
\pi(\sigma)=(a(\sigma),s(\sigma))$. Then $p'$ is given by
$$\eqalign{
&\forall \sigma\from\Sigma_1 \cr
&\forall n\from N_1 \cr
&\forall h\from H_1 \cr
&\forall e\from E_1 \cr
&\forall k\from K_1 \cr
}\ \ \eqalign{
p'(\sigma) &= a(\sigma)(p(\sigma)) \cr
p'(n) &= a(W_1(n))(p(n)) \cr
p'(h) &= a(W_1(A_1(h)))(p(h)) \cr
p'(e) &= a(W_1(A_1(F_1(e))))(p(e)) \cr
p'(k) &= a(W_1(A_1(F_1(C_1(k)))))(p(k)) \cr
} \eqno (1) $$
and $u' = u \cdot s'$, where $s'$ is an embedding token for $\N_1$ defined by
$$\eqalign{
\forall \sigma\from\Sigma_1 \cr
\forall n\from N_1
}\ \ \eqalign{
s'(\sigma) &= s(\sigma)(p(\sigma)) \cr
s'(n) &= s(W_1(n))(p(n)).
} \eqno (2) $$
Also, $v=(sub,con,rel,symm,tem,in)$, and, for any $\sigma^\dagger\from\Sigma_1$,
$(a(\sigma^\dagger),s(\sigma^\dagger))$ is a symmetry of $\N_0$ with respect to
$v$, so $v \circ a(\sigma^\dagger) = v \cdot s(\sigma^\dagger)$; in terms of
components this means
$$\eqalign{
&(sub^\ddagger, con \circ a(\sigma^\dagger),
rel \circ a(\sigma^\dagger), symm \circ a(\sigma^\dagger),
tem \circ a(\sigma^\dagger), in \circ a(\sigma^\dagger))
= v \circ a(\sigma^\dagger)
\cr
& = v \cdot s(\sigma^\dagger) =
(sub^\dagger,con^\dagger,rel^\dagger,symm,tem^\dagger,in^\dagger)
}\eqno (3) $$
where $sub^\ddagger,sub^\dagger,con^\dagger,rel^\dagger,tem^\dagger,in^\dagger$
are defined by
$$\eqalign{
\forall \sigma,\sigma^* \from \Sigma_0 \quad (G_0(\sigma,\sigma^*) \ \Rightarrow\
sub^\ddagger(\sigma,\sigma^*) &=
sub(a(\sigma^\dagger)(\sigma),a(\sigma^\dagger)(\sigma^*))) \cr
\forall \sigma,\sigma^* \from \Sigma_0 \quad (G_0(\sigma,\sigma^*) \ \Rightarrow\
sub^\dagger(\sigma,\sigma^*)
&= (s(\sigma^\dagger)(\sigma))\inv \cdot sub(\sigma,\sigma^*) \cdot
s(\sigma^\dagger)(\sigma^*)) \cr
\forall n\from N_0 \quad con^\dagger(n)
&= (s(\sigma^\dagger)(W_0(n)))\inv \cdot con(n) \cdot s(\sigma^\dagger)(n) \cr
\forall e\from E_0 \quad rel^\dagger(e)
&= (s(\sigma^\dagger)(A_0(S_0(e))))\inv \cdot rel(e) \cdot
s(\sigma^\dagger)(A_0(F_0(e))) \cr
\forall \sigma\from\Sigma_0 \quad tem^\dagger(\sigma)
&= tem(\sigma) \circ s(\sigma^\dagger)(\sigma) \cr
\forall \sigma\from\Sigma_0 \quad
in^\dagger(\sigma)
&= (s(\sigma^\dagger)(\sigma))\inv \cdot in(\sigma) \cdot
s(\sigma^\dagger)(\sigma).
} \eqno (4) $$
I claim that $v \circ p' = (v \circ p) \cdot s'$. To verify the claim we may
write the left-hand side as
$$ v \circ p'
= (sub', con \circ p', rel \circ p', symm \circ p', tem \circ p',
in \circ p') $$
where
$$ \forall\sigma,\sigma^*\from \Sigma_1 \quad (G_1(\sigma,\sigma^*) \Rightarrow
sub'(\sigma,\sigma^*) = sub(p'(\sigma),p'(\sigma^*))) \eqno (5) $$
and the right-hand side as
$$ (v \circ p) \cdot s' =
(sub'',con'',rel'',symm \circ p,tem'',in'') $$
where
$$\eqalign{
\forall \sigma,\sigma^* \from \Sigma_1 \quad 
(G_1(\sigma,\sigma^*) \ \Rightarrow\
sub''(\sigma,\sigma^*)
&= s'(\sigma)\inv \cdot sub(p(\sigma),p(\sigma^*)) \cdot s'(\sigma^*)) \cr
\forall n\from N_1 \quad con''(n) &= s'(W_1(n))\inv \cdot con(p(n)) \cdot
s'(n) \cr
\forall e\from E_1 \quad rel''(e) &= s'(A_1(S_1(e)))\inv \cdot rel(p(e))
\cdot s'(A_1(F_1(e))) \cr
\forall \sigma\from\Sigma_1 \quad tem''(\sigma) &= tem(p(\sigma)) \circ
s'(\sigma)
\cr
\forall \sigma\from\Sigma_1 \quad
in''(\sigma) &= s'(\sigma)\inv \cdot in(p(\sigma)) \cdot s'(\sigma).
} \eqno (6) $$
Now we can verify the claim by comparing the six components of $v \circ p'$ and
$(v \circ p) \cdot s'$.
$$\eqqalign{\ \ }{
\forall \sigma,\sigma^*\from\Sigma_1\ \ (G_1(\sigma,\sigma^*) \Rightarrow
\kern-30pt &
&\cr
sub'(\sigma,\sigma^*)
&= sub(p'(\sigma),p'(\sigma^*))
&\text{by (5)}\cr
&= sub\bigl(a(\sigma)(p(\sigma)),a(\sigma^*)(p(\sigma^*))\bigr)
&\text{by (1)}\cr
&= sub\bigl(a(\sigma)(p(\sigma)),a(\sigma)(p(\sigma^*))\bigr)
&\text{since $\pi$ is a local symmetry}\cr
&= sub^\ddagger(p(\sigma),p(\sigma^*))
&\text{by (4) with $\sigma^\dagger=\sigma$}\cr
&= sub^\dagger(p(\sigma),p(\sigma^*))
&\text{by (3)}\cr
&= \bigl(s(\sigma)(p(\sigma))\bigr)\inv \cdot sub(p(\sigma),p(\sigma^*)) \cdot
s(\sigma)(p(\sigma^*))
&\text{by (4)}\cr
&= \bigl(s(\sigma)(p(\sigma))\bigr)\inv \cdot sub(p(\sigma),p(\sigma^*)) \cdot
s(\sigma^*)(p(\sigma^*))
&\text{since $\pi$ is a local symmetry}\cr
&= s'(\sigma)\inv \cdot sub(p(\sigma),p(\sigma^*)) \cdot s'(\sigma^*)
&\text{by (2)}\cr
&= sub''(\sigma,\sigma^*))
&\text{by (6)}\cr
}$$

$$\eqqalign{\kern-5pt}{
\forall n \from N_1 \ \
(con \circ p')(n)
&= con(p'(n))
= con(a(W_1(n))(p(n)))
&\text{by (1)}\cr
&= con^\dagger(p(n))
&\text{by (3) with $\sigma^\dagger = W_1(n)$}\cr
&=\bigl(s(W_1(n))(W_0(p(n)))\bigr)\inv \!\cdot con(p(n)) \cdot s(W_1(n))(p(n))
&\kern5pt\text{by (4)}\cr
&=\bigl(s(W_1(n))(p(W_1(n)))\bigr)\inv \!\cdot con(p(n)) \cdot s(W_1(n))(p(n))
&\kern5pt\text{since $W_0 \circ p = p \circ W_1$}\cr
&=s'(W_1(n))\inv \cdot con(p(n)) \cdot s'(n)
&\text{by (2)}\cr
&= con''(n)
&\text{by (6)}\cr
}$$

$$\eqqalign{\kern-46pt}{
\forall e\from E_1 \ \ &(rel \circ p')(e)
= rel(p'(e))
= rel\bigl(a(W_1(A_1(F_1(e))))(p(e))\bigr)
&\text{by (1)}\cr
&= rel^\dagger(p(e))
&\text{by (3) with $\sigma^\dagger=W_1(A_1(F_1(e)))$}\cr
&= \bigl(s(\sigma^\dagger)(A_0(S_0(p(e))))\bigr)\inv \cdot rel(p(e))
\cdot s(\sigma^\dagger)(A_0(F_0(p(e))))
&\text{by (4)}\cr
&= \bigl(s(\sigma^\dagger)(p(A_1(S_1(e))))\bigr)\inv \cdot rel(p(e))
\cdot s(\sigma^\dagger)(p(A_1(F_1(e))))
&\text{since $p$ is a homomorphism}\cr
&= \bigl(s(W_1(A_1(S_1(e))))(p(A_1(S_1(e))))\bigr)\inv \cdot rel(p(e))
\cdot s(\sigma^\dagger)(p(A_1(F_1(e))))
&\cr&
&\text{since $\pi$ is a local symmetry}\cr
&= s'(A_1(S_1(e)))\inv \cdot rel(p(e)) \cdot s'(A_1(F_1(e)))
&\text{by (2)}\cr
&= rel''(e)
&\text{by (6)}\cr
}$$

$$\eqqalign\quad{
\forall\sigma\from\Sigma_1 \quad
(symm \circ p')(\sigma)
&= symm(p'(\sigma))
= symm(a(\sigma)(p(\sigma)))
&\text{by (1)}\cr
&= symm(p(\sigma))
&\text{by (3), with $\sigma^\dagger=\sigma$}\cr
&= (symm \circ p)(\sigma)
&\cr
}$$

$$\eqqalign\quad{
\forall\sigma\from\Sigma_1 \quad
(tem \circ p')(\sigma)
&= tem(p'(\sigma))
= tem(a(\sigma)(p(\sigma)))
&\text{by (1)}\cr
&= tem^\dagger(p(\sigma))
&\text{by (3) with $\sigma^\dagger=\sigma$}\cr
&= tem(p(\sigma)) \circ s(\sigma)(p(\sigma))
&\text{by (4)}\cr
&= tem(p(\sigma)) \circ s'(\sigma)
&\text{by (2)}\cr
&= tem''(\sigma)
&\text{by (6)}\cr
}$$

$$\eqqalign\quad{
\forall\sigma\from\Sigma_1 \quad
(in \circ p')(\sigma)
&= in(p'(\sigma))
= in(a(\sigma)(p(\sigma)))
&\text{by (1)}\cr
&= in^\dagger(p(\sigma))
&\text{by (3) with $\sigma^\dagger=\sigma$}\cr
&= (s(\sigma)(p(\sigma)))\inv \cdot in(p(\sigma)) \cdot
s(\sigma)(p(\sigma))
&\text{by (4)}\cr
&= s'(\sigma)\inv \cdot in(p(\sigma)) \cdot s'(\sigma)
&\text{by (2)}\cr
&= in''(\sigma)
&\text{by (6).}\cr
}$$
This completes the verification of the claim that $v \circ p' = (v \circ p)
\cdot s'$.

Now we are in a position to prove part (i) of the theorem:
$$\eqqalign\quad{
DM(I,\N_1,u',v \circ p')
&= DM(I,\N_1,u \cdot s', v \circ p')
&\cr
&= DM(I,\N_1,u \cdot s', (v \circ p) \cdot s')
&\text{by the claim}\cr
&= DM(I,\N_1,u,v \circ p)
&\text{by theorem~28(i).}\cr
}$$

For part (ii), consider any $n\from N_1$. Recall that, for any
$\sigma^\dagger\from\Sigma_1$, $symm \circ a(\sigma^\dagger) = symm$, by (3),
so, taking $\sigma^\dagger=P_1(n)$, $symm(a(P_1(n))(p(P_1(n)))) =
symm(p(P_1(n)))$ and hence
$$ symm(p'(P_1(n))) = symm(p(P_1(n))). \eqno(7) $$

Secondly, since $(a(P_1(n)),s(P_1(n)))$ is a symmetry of $\N_0$ with respect to
$v$,
$$ s(P_1(n))(p(P_1(n))) \in symm(p(P_1(n))) \eqno(8) $$
and, since $(a(W_1(n)),s(W_1(n)))$ is a symmetry of $\N_0$ with respect to $v$,
$$ s(W_1(n))(p(n)) \in symm(P_0(p(n))) = symm(p(P_1(n))). \eqno(9) $$

Now, suppose that the symmetry condition holds for $\N_1,u,v\circ p$. Then, for
any $n\from N_1$, $u(P_1(n))\inv \cdot u(n) \in symm(p(P_1(n)))$, so
$$\eqqalign\quad{
u'(P_1(n))\inv \cdot u'(n)
&= \bigl(s(P_1(n))(p(P_1(n)))\bigr)\inv \cdot u(P_1(n))\inv \cdot u(n) \cdot
s(W_1(n))(p(n))
&\cr
&\in symm(p(P_1(n)))
&\text{by (8) and (9)}\cr
&= symm(p'(P_1(n)))
&\text{by (7)}\cr
}$$
so the symmetry condition for $\N_1,u',v\circ p'$ holds. Conversely, suppose
that the symmetry condition for $\N_1,u',v\circ p'$ holds. Then, for any $n\from
N_1$, $u'(P_1(n))\inv \cdot u'(n) \in symm(p'(P_1(n))) = symm(p(P_1(n)))$, by
(7), so from
$$ u'(P_1(n))\inv \cdot u'(n)
= \bigl(s(P_1(n))(p(P_1(n)))\bigr)\inv \cdot u(P_1(n))\inv \cdot u(n) \cdot
s(W_1(n))(p(n)) $$
we have
$$\eqqalign\quad{
u(P_1(n))\inv \cdot u(n)
&= s(P_1(n))(p(P_1(n))) \cdot u'(P_1(n))\inv \cdot u'(n) \cdot
\bigl(s(W_1(n))(p(n))\bigr)\inv
&\cr
&\in symm(p(P_1(n)))
&\text{by (8) and (9)}\cr
}$$
so the symmetry condition for $\N_1,u,v\circ p$ holds. \qed

\theorem 30. (Affine invariance of the $\rho$ function.) For any template $T$,
any image $I$, and any affine transformations $g,g'$,
$$ \rho_{I\circ g\inv,T,sat\circ g\inv}(g\cdot g')
= |\det(\rep g)|^{1-k} \, \rho_{I,T,sat}(g').
$$

\medskip\f
(Recall that $\overline g$ is the matrix representation of $g$.)

\proof Recall the definition
$$ \rho_{I,T,sat}(g)
= |det(\rep g)|^{1-k} \int w(sat(g(u))) \, T(u) \, (I(g(u))-I_0) \d^2u. $$
Now,
$$\eqalign{
\rho_{I\circ g\inv,T,sat\circ g\inv}(g\cdot g')
&= |det(\rep{g\cdot g'})|^{1-k} \kern-3pt \int w((sat\circ g\inv)((g\cdot g')(u))) \, T(u) \,
((I\circ g\inv)((g\cdot g')(u))-I_0) \d^2u \cr
&= |det(\rep g)|^{1-k} \, |det(\rep{g'})|^{1-k} \kern-3pt \int w(sat(g'(u))) \, T(u) \,
(I(g'(u))-I_0) \d^2u \cr
&= |det(\rep g)|^{1-k} \, \rho_{I,T,sat}(g').
}\kern-5pt$$
\qed

\theorem 31. (Affine invariance of $DM$.) For any affine $g$
such that $|det(\overline g)|=1$, any image $I$, any definite network $\N=\network{}$,
any embedding token $u$ for $\N$, and any embedding type $v$ for $\N$, define a
new, affine-transformed image $I' = I \circ g\inv$, and a new,
affine-transformed embedding token $u'$ for $\N$ by $\forall x\from\Sigma\cup N\
u'(x) = g \cdot u(x)$. Then
$$ DM(I', \N, u', v) = DM(I, \N, u, v). $$

\proof Let $sat$ be the definite saturation function calculated using the 
embedding token $u$. Then the saturation function calculated using $u'$ is 
$sat'= sat \circ g\inv$, by the definition of $sat$ in \S4.4. By theorem~30
$$ \forall \sigma\from\Sigma \quad
\rho_{I',tem(\sigma),sat'}(u'(\sigma)) = \rho_{I,tem(\sigma),sat}(u(\sigma)). $$
Also,
$$ \forall \sigma,\sigma^*\from\Sigma \quad u'(\sigma)\inv \cdot u'(\sigma^*)
= u(\sigma)\inv \cdot g\inv \cdot g \cdot u(\sigma^*)
= u(\sigma)\inv \cdot u(\sigma^*) $$
and similarly
$$\eqalign{
\forall n\in N \quad u'(W(n))\inv \cdot u'(n)
&= u(W(n))\inv \cdot u(n)
\cr
\forall e\in E \quad u'(A(S(e)))\inv \cdot u'(A(F(e)))
&= u(A(S(e)))\inv \cdot u(A(F(e)))
\cr
\forall e\in E \quad u'(W(A(S(e))))\inv \cdot u'(W(A(F(e))))
&= u(W(A(S(e))))\inv \cdot u(W(A(F(e))))
}$$
Thus the each term of $DM(I', \N, u', v)$ equals the corresponding term of
$DM(I, \N, u, v)$. \qed

\subhead{4.7 The recognition problem -- definitive statement}
With the help of the theory developed so far we can now give a definitive
statement of the recognition problem, taking account of embeddings.

Given a semi-definite network $\N_0$ (representing a grammar), an embedding type
$v$ for $\N_0$, and an image $I$, the recognition problem is to construct a
definite network $\N_1$ (representing a pattern), a homomorphism
$p:\N_1\to\N_0$, and an embedding token $u$ for $\N_1$, maximising $DM(I, \N_1,
u, v\circ p)$, subject to the symmetry condition for $\N_1,u,v\circ p$.

\vfill\supereject
\runninghead{5. Inclusion functions}

\head{5. Inclusion Functions}

\subhead{5.1 Introduction}
During recognition, when many competing grammatical possibilities are being
considered in parallel in the same pattern, some possibilities are evaluated as better than others.
That is, each symbol token $\sigma$ in the pattern has associated with it a real
number $i(\sigma) \from [0,1]$ (called an \i{inclusion value}) indicating the
algorithm's degree of confidence that $\sigma$ should be present in the final
pattern. If $i(\sigma)=1$ then the algorithm
has decided definitely to include it in the final pattern; if $i(\sigma)=0$ the
algorithm has decided definitely to prune it (but hasn't yet done so); 
intermediate values indicate
uncertainty about whether to keep it. Similarly each node token $n$ and edge token
$e$ has
an inclusion value $i(n)$ or $i(e)$ indicating the algorithm's degree of
confidence
that it should be included in the final pattern. (Hooks and facets do not need
their own inclusion values as they stand or fall with the symbol, node or edge
they belong to.)

The function $i$ is called an \i{inclusion function} and is accompanied by a
second inclusion function $j$, defined below.

By the end of the recognition process, each inclusion value have been driven to
the extremes, $0$ or $1$, and the symbols, nodes and edges with inclusion value
$0$ have all been pruned.

\subhead{5.2 Definition of inclusion functions}

\defn A pair of \i{inclusion functions} on a network $\N=\network{}$ is defined
as $(i,j)$, where $i:\Sigma\cup N \cup E \to [0,1]$ and $j:\Sigma\cup N\cup H
\cup (K\setdiff dom(G)) \to [0,1]$, such that
$$\eqalignno{
\forall \sigma\from\Sigma \quad i(\sigma)
&= j(\sigma) \ + \sum_{n\in P\preo\sigma} \hskip-3mm (1-g_n)i(n),
\qquad\text{where $g_n = \bigl|\comp{n^*\from N}{G(n^*,n)}\bigr|$} \qquad & (1)
\cr
\forall n \from N \quad i(W(n)) &= j(n) + i(n) & (2)
\cr
\forall h\from H \quad i(A(h)) &= j(h) \ + \sum_{e\in F\preo h} \hskip-3mm i(e)
\ + \sum_{e\in S\preo h} \hskip-3mm i(e) & (3)
\cr
\forall k \from K\setdiff dom(G) \quad
i(C(k)) &= j(k) + \sum_{k^* \mid G(k,k^*)} i(C(k^*)). & (4)
}$$
(This is a slightly modified version of the definition in (2004, \S7.2), taking
account of subsymbols. The summation notation in (4) means a sum
over all $k^*$ such that $G(k,k^*)$.)

This definition may be interpreted informally as follows. (In the following
explanation I shall use the future tense to state conditions that will hold 
at the end of recognition when the pattern is definite, and the present tense
for what holds during recognition when the pattern is indefinite.)

Line (1). At the end of recognition each symbol $\sigma$ will be either a \ic{bare} symbol (with $P\preo\sigma
=\emptyset$) or a part of one larger symbol (with $|P\preo\sigma| = 1$). 
Hence the nodes presently in $P\preo\sigma$ are in competition with one
another; at most one will survive to the end. $i(\sigma)$ is
interpreted as the degree of confidence in $\sigma$, $j(\sigma)$ is the degree
of confidence that $\sigma$ will be a bare symbol, and $i(n)$
is the degree of confidence in $n$. An exception to this competition is that if
$n$ is a subnode of $n^*$ (i.e., $G(n^*,n)$) then they may both be correct; 
the $1-g_n$ factor allows for this co-existence.

Line (2). $i(W(n))$ is the degree of confidence in $W(n)$, $j(n)$ is the
degree of confidence that $W(n)$ will survive to the end but $n$ will not, and
$i(n)$ is the degree of confidence in $n$.

Line (3) expresses the fact that each hook $h$ will have a single edge incident
to it (i.e., $|F\preo h| + |S\preo h| = 1$); hence the edges presently in
$F\preo h \cup S\preo h$ are in competition with one another. Thus $i(A(h))$
is the degree of confidence in the node or symbol $A(h)$, $i(e)$ is the degree
of confidence in $e$, and $j(h)$ is the degree of confidence that $A(h)$ will
survive to the end but that none of its present edges will (i.e., the correct
edge has yet to be created).

Line (4) expresses the fact that each facet $k$ that is not itself a sub-facet
will be glued to a single sub-facet. Hence if $k$ is presently glued to several
sub-facets then they are in competition with one another; $i(C(k^*))$ is the
degree of confidence in the edge $C(k^*)$, $j(k)$ is the degree of confidence
that $C(k)$ is correct but that none of $k$'s present sub-facets is.

\theorem 32. If $\N=\network{}$ is a definite network and $(i,j)$ is a pair of
inclusion functions on $\N$ satisfying $\forall x\from\Sigma\cup N \cup E\ i(x)
= 1$, then
$$ \forall\sigma\from\Sigma\ j(\sigma) =
\cases{0 & if $\sigma \in P(N)$\cr
1 & otherwise}, \quad
\forall n\from N\ j(n) = 0, \quad
\forall h\from H\ j(h) = 0, \quad
\forall k\from K\setdiff\dom(G)\ j(k) = 0. $$

\proof For any $\sigma\from\Sigma$,
$$ i(\sigma) = j(\sigma) \ + \sum_{n\in P\preo\sigma} \hskip-3mm (1-g_n)i(n) $$
where $g_n = \bigl|\comp{n^*\from N}{G(n^*,n)}\bigr|$, so
$$ 1 = j(\sigma) + |P\preo\sigma| - |G_N \circ id_{P\preo\sigma}|. $$
This implies $j(\sigma) \in \Z$, and since also $j(\sigma) \in [0,1]$ we
have $j(\sigma) \in \{0,1\}$. Now, for any $\sigma\in\Sigma$, if $\sigma\notin
P(N)$ then $P\preo\sigma=\emptyset$, which immediately gives $|P\preo\sigma| -
|G_N \circ id_{P\preo\sigma}| = 0$ and so $j(\sigma)=1$. Conversely, if
$j(\sigma) = 1$ then $|P\preo\sigma| - |G_N \circ id_{P\preo\sigma}| = 0$, so by
theorem~13(ii) (applied to $N,\Sigma,P,G_N$) $P\preo\sigma = \emptyset$, so
$\sigma\notin P(N)$. This shows that $j(\sigma) = 1$ if $\sigma \notin P(N)$ and
$j(\sigma) = 0$ if $\sigma \in P(N)$.

For any $n\from N$,
$$ i(\sigma) = j(n) + i(n) $$
and hence $j(n) = 0$.

For any $h\from H$,
$$ i(A(h)) = j(h) \ + \sum_{e\in F\preo h} \hskip-3mm i(e)
\ + \sum_{e\in S\preo h} \hskip-3mm i(e) $$
and, thanks to the sum diagram $E \buildrel F \over \rightarrow H \buildrel S
\over \leftarrow E$, there is a unique $e\from E$ such that either $F(e) = h$ or
$S(e) = h$; so $j(h) = 0$.

For any $k\from K\setdiff\dom(G)$,
$$ i(C(k)) = j(k) + \sum_{k^* \mid G(k,k^*)} i(C(k^*)). $$
By the definiteness condition $id_K = G_K \circ G_K\inv \cup G_K\inv \circ G_K$,
there exists $k^*\from K$ such that $G(k,k^*)$ (otherwise $(G_K \circ G_K\inv
\cup G_K\inv \circ G_K)(k,k)$ would not hold); moreover, this $k^*$ is unique
(for if there were a second, $k^{**}$, then $(G_K \circ G_K\inv \cup G_K\inv
\circ G_K)(k^*,k^{**})$ would hold). Thus $j(k) = 0$. \qed

\subhead{5.3 The recognition process}
With the help of the theory developed so far we can give an initial
description of the recognition process. It constructs a pattern $\N_1$, a homomorphism
$p:\N_1\to\N_0$ (where $\N_0$ is the grammar), and a pair of inclusion functions
$(i,j)$ on $\N_1$, by a sequence of structural operations on the pattern.

The recognition process must ensure that, at the end, the following conditions
hold.

\blob $\forall x\from \Sigma_1\cup N_1\cup E_1\ i(x) = 1$,

\blob $\N_1$ is definite.

\vfill\supereject
\def\Flex{\hbox{\i{Flex}}}

\runninghead{6. The indefinite match function}

\head{6. The Indefinite Match Function}

\subhead{6.1 Introduction}
In section 4 we constructed the definite match function $DM$, which measures how
well a definite pattern (with an embedding token) matches the image, the grammar
and embedding type. Now we shall generalise it to the \i{indefinite match
function} $IM$, which applies to patterns that are not necessarily definite,
with inclusion functions. The affine invariance theorems of \S4.6 are generalised
to $IM$.

The recognition process attempts to maximise the value of $IM$ during
recognition, so that the final, definite pattern will maximise $DM$.

\subhead{6.2 Template matching}
The template matching function of \S4.4 is generalised as follows.

Suppose we are given a network $\N=\network{}$, an embedding token $u$ for $\N$,
a function $tem:\Sigma\to Tem$, and a pair $(i,j)$ of inclusion functions on
$\N$. The \i{(indefinite) saturation function}, $sat:\R^2\to\R$, is defined by
$$ \forall x\from\R^2\quad
sat(x) = \sum_{\sigma\in\Sigma} (1-g_\sigma) \, i(\sigma) \,
tem(\sigma)(u(\sigma)\inv(x)) $$
where $g_\sigma = \bigl|\comp{\sigma^*\from\Sigma}{G(\sigma^*,\sigma)}\bigr|$.

In the special case where the inclusion functions satisfy $\forall
\sigma\from\Sigma\ i(\sigma) = 1$, as at the end of recognition, the definition
of $sat$ reduces to the definite saturation function defined in \S4.4.

The correlation function $\rho_{I,T,sat}$ between an image $I$ and a 
template $T$ is as in \S4.4, except for using the indefinite saturation 
function,
$$\eqalign{
\rho_{I,T,sat}(g)
&= |det(\rep g)|^{1-k} \int w(sat(g(u))) \, T(u) \, (I(g(u))-I_0) \d^2u \cr
&= |\det(\rep g)|^{-k} \int w(sat(x)) \, T(g\inv(x)) \, (I(x)-I_0) \d^2x
}$$

\subhead{6.3 The indefinite match function}
The \i{indefinite match} function $IM$ measures how well a (not necessarily
definite) network $\N=\network{}$ matches an image $I$, given an embedding token
$u$ for $\N$, an embedding type $v=(sub,con,rel,\allowbreak symm, \allowbreak
tem,in)$ for $\N$, a pair of inclusion functions $(i,j)$ on $\N$, and a function
$B:\Sigma\cup H\cup (K\setdiff\dom(G))\to\closeopen{0,\infty}$. It is defined by
$$\eqalign{
& \kern-10pt IM(I, \N, u, v, i, j, B) = \cr
& \sum_{\sigma\in\Sigma}
\bigl( i(\sigma) \rho_{I,tem(\sigma),sat}(u(\sigma)) - j(\sigma) B(\sigma)
\bigr)
-\sum_{(\sigma,\sigma^*)\mid G(\sigma,\sigma^*)} \kern-15pt i(\sigma^*)
E_{sub(\sigma,\sigma^*)}(u(\sigma)\inv \cdot u(\sigma^*))
\cr&
- \sum_{n\in N} i(n) E_{con(n)}(u(W(n))\inv \cdot u(n))
- \sum_{h \in H} j(h) B(h)
- \sum_{k \in K\setdiff\dom(G)} \kern-12pt j(k) B(k)
\cr&
- \sum_{e\in E} i(e)
\bigl( E_{rel(e)}(u(A(S(e)))\inv \cdot u(A(F(e)))) +
E_{in(W(A(F(e))))}(u(W(A(S(e))))\inv \cdot u(W(A(F(e))))) \bigr)
}$$
where $sat$ is the indefinite saturation function. Observe that the $B$
function imposes a penalty for each \ic{bare} symbol, hook and facet, i.e.,
each symbol that is not a part of any other symbol ($j(\sigma)=1$), each hook
with no incident edges ($j(h)=1$), and each facet that should be glued to a
sub-facet but is not ($j(k)=1$). A function $B:\Sigma\cup H\cup
(K\setdiff\dom(G))\to\closeopen{0,\infty}$ is called a \i{bareness function}
for $\N$. The final term, $E_{in(W(A(F(e))))}(\cdots)$, has no counterpart in
$DM$; it is to penalise edges between two nodes belonging to different wholes
(see \S9.6).

The following theorem shows that $DM$ is a special case of $IM$.

\theorem 33. If

\item{(a)} $\N$ is definite,

\item{(b)} $\forall x\from\Sigma\cup N \cup E\ i(x) = 1$,

\item{(c)} $\forall\sigma\from\Sigma\setdiff P(N)\ B(\sigma)=\theta$,

\smallskip\f
then $IM(I,\N,u,v,i,j,B) = DM(I,\N,u,v)$.

\proof By theorem~32,
$$\forall\sigma\from\Sigma\ j(\sigma) =
\cases{0 & if $\sigma \in P(N)$\cr
1 & otherwise},\quad
\forall n\from N\ j(n) = 0, \quad
\forall h\from H\ j(h) = 0, \quad
\forall k\from K\setdiff\dom(G)\ j(k) = 0. $$
It follows that each term of $IM(I,\N,u,v,i,j,B)$ simplifies to the
corresponding term of $DM(I,\allowbreak\N,\allowbreak u,\allowbreak v)$ or
vanishes; in particular, for each $e\from E$, the term
$$ E_{in(W(A(F(e))))}(u(W(A(S(e))))\inv \cdot u(W(A(F(e))))) $$
vanishes since $W(A(S(e))) = W(A(F(e)))$ by the definiteness conditions. \qed

\medbreak

In the recognition process an embedding token $u$ for $\N_1$ is constructed,
along with $\N_1$ and $p$. An embedding type $v\circ p$ is induced using $p$ from
the given embedding type $v$ for $\N_0$. Throughout recognition we measure how
well $u$ matches $v\circ p$ by calculating $IM(I,\N_1,u,v\circ p,i,j,B)$, and we
seek to maximise this by continually adjusting $u$, subject to the symmetry
condition for $\N_1,u,v\circ p$.

\subhead{6.4 Invariance theorems}
I shall generalise the invariance theorems of \S4.6 from $DM$ to $IM$.

\theorem 34. (Lemma~1 of (2004, \S7.3): invariance under affine transformation
of the symbols' internal frames of reference.) For any image $I$, network $\N$,
embedding tokens $u,u'$ for $\N$, embedding type $v$ for $\N$, inclusion
functions $i,j$ on $\N$, and bareness function $B$ for $\N$,
$$ IM(I, \N, u\cdot u', v\cdot u', i, j, B) = IM(I, \N, u, v, i, j, B), $$
provided $u' \circ W \circ A \circ F = u' \circ W \circ A \circ S$.

\proof As in theorem~28, each term of $IM(I, \N, u\cdot u', v\cdot u', i,
j, B)$ equals the corresponding term of $IM(I, \N, u, v, i, j, B)$. \qed

\theorem 35. (Invariance of the match functions under a local symmetry.) Given
an image $I$, a semi-definite network $\N_0$, a network $\N_1$, a homomorphism
$p:\N_1\to\N_0$, an embedding token $u$ for $\N_1$, an embedding type $v$ for
$\N_0$, and a local symmetry $\pi$ of $\N_1$ with respect to $\N_0,p,v$, the
application of $\pi$ to $p,u$ produces a homomorphism $p':\N_1\to\N_0$ and an
embedding token $u'$ for $\N_1$.

(i) For any inclusion functions $i,j$ and bareness function $B$ for $\N_1$,
$IM(I, \N_1, u', v\circ p', i, j, B) \allowbreak = IM(I, \N_1, u, v\circ p, i,
j, B)$.

(ii) The symmetry condition holds for $\N_1,u',v \circ p'$ iff it holds for
$\N_1,u,v \circ p$.

\proof The argument of theorem~29 generalises:
$$\eqqalign\quad{
IM(I,\N_1,u',v \circ p',i,j,B)
&= IM(I,\N_1,u \cdot s', (v \circ p) \cdot s',i,j,B)
&\text{since $v \circ p' = (v \circ p) \cdot s'$}\cr
&= IM(I,\N_1,u,v \circ p,i,j,B)
&\text{by theorem~34.}\cr
}$$
To justify this use of theorem~34 we must check that $s' \circ W_1 \circ A_1
\circ F_1 = s' \circ W_1 \circ A_1 \circ S_1$. For any $e\from E_1$,
$$\eqqalign\quad{
s'(W_1(A_1(F_1(e))))
&= s(W_1(A_1(F_1(e))))(p(W_1(A_1(F_1(e)))))
&\cr
&= s(W_1(A_1(F_1(e))))(W_0(A_0(F_0(p(e)))))
&\text{since $p$ is a homomorphism}\cr
&= s(W_1(A_1(F_1(e))))(W_0(A_0(S_0(p(e)))))
&\text{since $\N_0$ is semi-definite}\cr
&= s(W_1(A_1(S_1(e))))(W_0(A_0(S_0(p(e)))))
&\text{since $\pi$ is a local symmetry}\cr
&= s(W_1(A_1(S_1(e))))(p(W_1(A_1(S_1(e)))))
&\text{since $p$ is a homomorphism}\cr
&= s'(W_1(A_1(S_1(e))))
&\cr
}$$
as required.

For part (ii), the proof in theorem~29 applies (it does not require $\N_1$ to be
definite). \qed

\theorem 36. (Affine invariance of the $\rho$ function.) For any template $T$,
any image $I$, and any affine transformations $g,g'$,
$$ \rho_{I\circ g\inv,T,sat\circ g\inv}(g\cdot g')
= |\det(\rep g)|^{1-k} \, \rho_{I,T,sat}(g').
$$

\medskip\f
(Recall that $\overline g$ is the matrix representation of $g$.)

\proof This is identical to theorem~30, except using the indefinite saturation
function. The same proof applies. \qed

\theorem 37. (Affine invariance of $IM$.) For any affine $g$ such that
$|det(\overline g)|=1$, any image $I$, any network $\N=\network{}$, any
embedding token $u$ for $\N$, and any embedding type $v$ for $\N$, define a new,
affine-transformed image $I' = I \circ g\inv$, and a new, affine-transformed
embedding token $u'$ for $\N$ by $\forall x\from\Sigma\cup N\ u'(x) = g \cdot
u(x)$.

For any inclusion functions $i,j$ and bareness function $B$ for $\N$,
$$ IM(I', \N, u', v, i, j, B) = IM(I, \N, u, v, i, j, B). $$
(The condition $|det(\overline g)|=1$ may be dropped if $k=1$.)

\proof Let $sat$ be the indefinite saturation function calculated using the
embedding token $u$.

As in the proof of theorem~31, each term of $IM(I', \N, u', v, i, j, B)$ equals
the corresponding term of $IM(I, \N, u, v, \allowbreak i, \allowbreak j,
\allowbreak B)$. \qed

\subhead{6.5 Adjustment of the embedding token}
During recognition the embeddings of all the symbols and nodes are continually
adjusted to maximise $IM(I, \N_1, u, v\circ p, i, j, B)$ (subject to the
symmetry condition). This is done by a process of gradient ascent, as defined in
(2004, \S\S7.6--7.8), but with the calculation of the derivative of the match
function in \S7.6 augmented to allow for the new terms in the match function. To
be precise, theorem~3 of \S7.6 is amended as follows. We make a small
change in the embedding token from $u$ to $u \cdot \Delta u$, where
$$\eqalign{
\forall\sigma\from\Sigma\ \ \Delta u(\sigma) &= \exp(\epsilon V_\sigma) \cr
\forall n\from N\ \ \Delta u(n) &= \exp(\epsilon V_n) \cr
}$$
where the increments $V_\sigma,V_n \in \A$ are linked by the symmetry
condition; then the value of $IM$ changes to
$$ IM(I, \N, u \cdot \Delta u, v, i, j, B) =
IM(I, \N, u, v, i, j, B) +
\epsilon \sum_{\sigma\in\Sigma} F_\sigma(V_\sigma) + o(\epsilon) $$
where, for each $\sigma\from\Sigma$,
$$\eqalign{
&F_\sigma = F^0_\sigma + F^1_\sigma + F^2_\sigma + F^3_\sigma + F^4_\sigma \cr
&F^0_\sigma, F^1_\sigma, F^2_\sigma, F^3_\sigma \text{ are as before} \cr
&F^4_\sigma = -\sum_{\sigma^*|G(\sigma,\sigma^*)}
Ad(Sub_{\sigma,\sigma^*}\inv)\adj(F_{\sigma,\sigma^*}) +
\sum_{\sigma^*|G(\sigma^*,\sigma)} F_{\sigma^*,\sigma}
}$$
and, for each $\sigma,\sigma^*\from\Sigma$ such that $G(\sigma,\sigma^*)$,
$$\eqalign{
F_{\sigma,\sigma^*} &= -i(\sigma^*)
E_{sub(\sigma,\sigma^*)*}(Sub_{\sigma,\sigma^*}) \cr
Sub_{\sigma,\sigma^*} &= u(\sigma)\inv \cdot u(\sigma^*).
}$$
The theorem is proved by the same methods as before.

\subhead{6.6 The recognition process}
During the recognition process $IM(I, \N_1, u, v\circ p, i, j, B)$ is 
maximised, and at the end the conditions of theorem~33
are satisfied, so $DM(I, \N_1, u, v\circ p)$ is maximised.

\vfill\supereject
\runninghead{7. How the inclusion functions are determined}

\head{7. How the Inclusion Functions are Determined}

\subhead{7.1 Introduction}
This section refines the account of the recognition process by describing how
the inclusion functions $i$ and $j$ are determined during recognition. The
inclusion functions are determined by a simulated annealing process, governed
by a \i{temperature} parameter that varies across the pattern and with time.
Where the structure of the pattern is changing, the temperature is high, and
this makes the inclusion functions take on mid-range values, so several
alternative interpretations can co-exist in parallel; when structural changes
stop, the temperature declines and the inclusion functions are pushed towards
$0$ or $1$, and so a choice is forced between alternatives and the pattern
becomes definite. The temperature varies across the pattern, as some parts of
the pattern may be very active while other parts have settled down.

\subhead{7.2 The inclusion vector, $\bold i$}
Our first step is to reformulate $i,j$ and the constraints on them in a vector
notation in order to emphasise their linear nature (this vector notation is for
use only in this section). Given a pair of inclusion functions $(i,j)$ on a
network $\N=\network{}$, we shall convert $(i,j)$ into the \i{inclusion vector}
$\bold i$ on $\N$, with components $\bold i_x$, for all $x \in X$, where
$$ X = \Sigma \times \set{0,1} \ \cup\ N \times \set{0,1} \ \cup\ H \ \cup\ E
\ \cup\ K\setdiff dom(G). $$
Each component of $\bold i$ represents one value of $i$ or $j$, as follows.
$$\eqalign{
\forall\sigma\from\Sigma \quad \bold i_{(\sigma,0)} &= i(\sigma), \quad
\bold i_{(\sigma,1)} = j(\sigma) \cr
\forall n \from N \quad \bold i_{(n,0)} &= i(n), \quad \bold i_{(n,1)} = j(n) \cr
\forall h \from H \quad \bold i_h &= j(h) \cr
\forall e \from E \quad \bold i_e &= i(e) \cr
\forall k \from K\setdiff dom(G) \quad \bold i_k &= j(k) \cr
}$$
The constraints on $i$ and $j$ can be expressed as a set of linear conditions on
$\bold i$ of the form
$$ \forall y \from Y \quad \bold c^y \cdot \bold i
= \sum_{x\in X} \bold c^y_x \bold i_x = 0 $$
using a set of vectors $\bold c^y$, for all $y\from Y$, where
$$ Y = \Sigma \,\cup\, N \,\cup\, H \,\cup\, K\setdiff dom(G) $$
and $\bold c^y$ has components $\bold c^y_x$ for $x\from X$, specified as
follows. For each $\sigma\from\Sigma$, the constraint $i(\sigma) = j(\sigma) +
\sum_{n\in P\preo\sigma} (1-g_n) i(n)$ is expressed as $\bold c^\sigma \cdot
\bold i = 0$, where
$$ \bold c^\sigma_x = \cases{
1 & if $x=(\sigma,0)$ \cr
-1 & if $x=(\sigma,1)$ \cr
g_n-1 & if $x=(n,0)$ for some $n\from P\preo\sigma$ \cr
0 & otherwise} $$
For each $n\from N$, the condition $i(W(n)) = j(n) + i(n)$ is expressed as
$\bold c^n \cdot \bold i = 0$, where
$$ \bold c^n_x = \cases{
1 & if $x=(W(n),0)$ \cr
-1 & if $x=(n,1)$ or $x=(n,0)$ \cr
0 & otherwise} $$
For each $h\from H$, the condition $i(A(h)) = j(h) + \sum_{e \in F\preo h} i(e)
+ \sum_{e \in S\preo h} i(e)$ is expressed as $\bold c^h \cdot \bold i = 0$,
where
$$ \bold c^h_x = \cases{
1 & if $x=(A(h),0)$ \cr
-1 & if $x=h$ or $x\in F\preo h$ or $x\in S\preo h$ \cr
0 & otherwise.} $$
(Note that this assumes that $F(e) \ne S(e)$ for each edge $e$.) For each $k
\from K \setdiff dom(G)$, the constraint $i(C(k)) = j(k) + \sum_{k^* \mid
G(k,k^*)} i(C(k^*))$ is expressed as $\bold c^k \cdot \bold i = 0$, where
$$ \bold c^k_x = \cases{
1 & if $x = C(k)$ \cr
-1 & if $x = k$ \cr
-1 & if $x = C(k^*)$, for some $k^*$ such that $G(k,k^*)$ \cr
0 & otherwise.} $$
This completes the specification of the $\bold c^y$ vectors.

Note that, using this vector notation, the $IM$ function is linear in $\bold i$
(if we disregard the dependence of the saturation function on $\bold i$):
$$\eqalign{
& \kern-10pt IM(I, \N, u, v, i, j, B) \cr
& = \sum_{\sigma\in\Sigma}
\bigl( i(\sigma) \rho_{I',tem(\sigma),sat}(u(\sigma)) - j(\sigma)B(\sigma)
\bigr)
-\sum_{(\sigma,\sigma^*)\mid G(\sigma,\sigma^*)} \kern-15pt i(\sigma^*)
E_{sub(\sigma,\sigma^*)}(u(\sigma)\inv \cdot u(\sigma^*))
\cr&\phantom{=}
- \sum_{n\in N} i(n) E_{con(n)}(u(W(n))\inv \cdot u(n))
- \sum_{h \in H} j(h) B(h)
- \sum_{k \in K\setdiff \dom(G)} \kern-12pt j(k) B(k)
\cr&\phantom{=}
- \sum_{e\in E} i(e)
\bigl( E_{rel(e)}(u(A(S(e)))\inv \cdot u(A(F(e)))) +
E_{in(W(A(F(e))))}(u(W(A(S(e))))\inv \cdot u(W(A(F(e))))) \bigr)
\cr
&= \bold i \cdot \bold m
}$$
where $\bold m$ is a vector whose components $\bold m_x$ are given by
$$\eqalign{
&\forall\sigma\from\Sigma\quad
\bold m_{(\sigma,0)}
= \rho_{I',tem(\sigma),sat}(u(\sigma))
- \sum_{\sigma^*\mid G(\sigma^*,\sigma)} \kern-5pt
E_{sub(\sigma^*,\sigma)}(u(\sigma^*)\inv \cdot u(\sigma)),
\qquad
\bold m_{(\sigma,1)} = -B(\sigma) \cr
&\forall n\from N\quad
\bold m_{(n,0)} = -E_{con(n)}(u(W(n))\inv \cdot u(n)), \qquad
\bold m_{(n,1)} = 0 \cr
&\forall h\from H \quad \bold m_h = -B(h) \cr
&\forall e\from E \quad \bold m_e
= -E_{rel(e)}(u(A(S(e)))\inv \cdot u(A(F(e))))
-E_{in(W(A(F(e))))}(u(W(A(S(e))))\inv \cdot u(W(A(F(e))))) \cr
&\forall k\from K\setdiff dom(G) \quad \bold m_k = -B(k)
}$$

\subhead{7.3 How $\bold i$ is determined}
Recall that recognition is governed by the expression $IM(I, \N_1, u, v\circ p,
i, j, B)$. As shown above, this can be expressed in the form $IM(I, \N_1, u,
v\circ p, i, j, B) = \bold i \cdot \bold m$, for a suitable vector $\bold m$. 
The inclusion vector $\bold i$ is determined by maximising the expression $$ E
= \sum_{x\in X} \frac{\bold i_x \bold m_x}{T_x} -\sum_{x\in X} \bigl( \bold i_x
\ln \bold i_x + (1-\bold i_x) \ln (1-\bold i_x) \bigr) $$ subject to the
constraints $\forall y\from Y \ \bold c^y \cdot \bold i = 0$, where each $T_x$
is a positive number, known as the \i{temperature} of $x$. To be precise, every
symbol, node, hook, edge and facet has a temperature, and we define
$T_{(\sigma,0)} = T_{(\sigma,1)} = T_\sigma$ and $T_{(n,0)} = T_{(n,1)} = T_n$.
(If $\bold i_x=0$ we treat $\bold i_x \ln \bold i_x$ as $0$, and if $\bold
i_x=1$ we treat $(1-\bold i_x) \ln (1-\bold i_x)$ as $0$.)

Using the method of Lagrange multipliers, we have to maximise the Lagrangian
$$ L
= \sum_{x\in X} \frac{\bold i_x \bold m_x}{T_x}
-\sum_{x\in X}
\bigl( \bold i_x \ln \bold i_x + (1-\bold i_x) \ln (1-\bold i_x) \bigr)
+ \sum_{y\in Y} \lambda_y \bold c^y \cdot \bold i
$$
where $\lambda_y$ is a Lagrange multiplier, for each $y\from Y$. This gives
$$ \forall x\from X\quad
0 = \frac{\partial L}{\partial \bold i_x}
= \frac{\bold m_x}{T_x} - \ln \Bigl( \frac{\bold i_x}{1-\bold i_x} \Bigr)
+ \sum_{y\in Y} \lambda_y \bold c^y_x.
$$
This has the solution
$$ \bold i_x
= \sigmoid\Bigl(
\frac{\bold m_x}{T_x} + \sum_{y\in Y} \lambda_y \bold c^y_x
\Bigr)
$$
where the sigmoid function $\sigmoid:\R \to (0,1)$ is defined by
$\forall u\from\R\ \sigmoid(u) = \frac1{1+e^{-u}}$.
By examining the second derivatives it can be determined that this solution is a
local maximum. Note that this solution satisfies $\forall x\from X\ \bold i_x
\in (0,1)$, and so $i$ and $j$ map into $[0,1]$, as required.

If all the temperatures are high, all $\bold i_x$ tend to take mid-range values. If all temperatures are at the minimum allowed value
$T_{min}$, the $\frac{\bold m_x}{T_x}$ terms will become large, and all $\bold
i_x$ are likely to become very close to $0$ or $1$, in which case we will round
them to $0$ or $1$, giving
$$ E = \frac{\sum_{x\in X} \bold i_x \bold m_x}{T_{min}}
= \frac{IM(I, \N, u, v, i, j, B)}{T_{min}}. $$

\subhead{7.4 Algorithm for finding $\bold i$}
The inclusion vector $\bold i$ is determined above by
$$ \forall x\from X \quad
\bold i_x
= \sigmoid
\Bigl( \frac{\bold m_x}{T_x} + \sum_{y\in Y} \lambda_y \bold c^y_x \Bigr)
$$
subject to the constraints $\forall y\from Y\ \bold c^y \cdot \bold i = 0$,
where the $\lambda_y$ parameters are unknown. We can split each $\bold c^y$
vector into two vectors $\bold c^{y+}$ and $\bold c^{y-}$
by separating positive and negative components:
$$ \forall y\from Y\ \forall x\from X\quad \bold c^{y+}_x = \max(\bold c^y_x,0),
\quad \bold c^{y-}_x = \max(-\bold c^y_x,0), $$
so that the constraints may be written as $\forall y\from Y\ 
\bold c^{y+} \cdot \bold i = \bold c^{y-} \cdot \bold i$. (Note that $\forall
y\from Y\ \bold c^{y+}, \bold c^{y-} \ne \bold 0$.)
Also define
$$ \forall y\from Y\quad C^{y+} = \max_{x\in X} \bold c^{y+}_x, \quad
C^{y-} = \max_{x\in X} \bold c^{y-}_x, \quad
C^y = C^{y+} + C^{y-}. $$
The following iterative
algorithm seeks values of $\lambda_y$ satisfying the constraints.

\bigskip

\indent For each $y\from Y$, initialise $\lambda_y$ to its final value last time
this algorithm was run;

\smallbreak

\indent repeat

\smallbreak

\indent\indent for each $x\from X$, do
$\bold i_x \assign \sigmoid\bigl( \bold m_x/T_x + \sum_{y\in Y} \lambda_y \bold
c^y_x \bigr)$ $\mid$

\smallbreak

\indent\indent for each $y \from Y$, do $\displaystyle\lambda_y \assign
\lambda_y + \frac1{C^y}
\ln\Bigl(\frac{\bold c^{y-}\cdot \bold i}{\bold c^{y+}\cdot \bold i}\Bigr)$

\smallbreak

\indent until equilibrium;

\smallbreak

\indent for each $x\from X$, if $\bold i_x$ is very close to $0$ or $1$,
then round it to $0$ or $1$.

\bigbreak\f
In this algorithm the semicolon means sequential composition, the \ic{$\mid$} symbol
means parallel composition, and the \ic{for each} loops are
parallel loops. This means that all the assignment statements in the
\ic{repeat} loop body
may be executed concurrently in any fair order. Note that this loop is by far
the most computationally expensive part of the entire recognition process, so the
high degree of parallelism is relevant from the point of view of time
complexity.

The \ic{for each $y\from Y$} loop may be expressed more explicitly as

\smallbreak

\indent\indent for each $\sigma\from\Sigma$, do
$\displaystyle\lambda_\sigma \assign \lambda_\sigma +
\frac1C\ln\Bigl(\frac{j(\sigma)+\sum_{n\in
P\preo\sigma}(1-g_n)i(n)}{i(\sigma)}\Bigr)$ $\mid$

\smallbreak

\indent\indent (where $C = \max(2,\max\comp{g_n}{n \in P\preo\sigma})$) $\mid$

\smallbreak

\indent\indent for each $n\from N$, do
$\displaystyle\lambda_n \assign \lambda_n +
\tfrac12\ln\Bigl(\frac{i(n)+j(n)}{i(W(n))}\Bigr)$ $\mid$

\smallbreak

\indent\indent for each $h\from H$, do
$\displaystyle\lambda_h \assign \lambda_h +
\tfrac12\ln\Bigl(\frac{j(h)+\sum_{e\in F\preo h}i(e) + \sum_{e\in S\preo
h}i(e)}{i(A(h))}\Bigr)$ $\mid$

\smallbreak

\indent\indent for each $k\from K\setdiff dom(G)$, do
$\displaystyle\lambda_k \assign \lambda_k + \tfrac12\ln\Bigl( \frac{j(k) +
\sum_{k^* \mid G(k,k^*)} i(C(k^*))}{i(C(k))}\Bigr)$.

\bigskip\f
The rationale for this algorithm is as follows. We begin with a lemma.

\def\lemma{\medskip\f{\bf Lemma. }}

\lemma (a) For any $l\from\R$ and any $\delta>0$,
$$ 1 < \frac{\sigmoid(l+\delta)}{\sigmoid(l)} < e^\delta. $$
(b) For any $l\from\R$ and any $\delta<0$,
$$ 1 > \frac{\sigmoid(l+\delta)}{\sigmoid(l)} > e^\delta . $$

\proof (a) Since $\delta>0$,
and $\sigmoid$ and the exponential function are strictly increasing,
$$ 1
< \frac{\sigmoid(l+\delta)}{\sigmoid(l)}
= \frac{1 + e^{-l}}{1 + e^{-l-\delta}}
= \frac{e^l + 1}{e^{l+\delta} + 1} e^\delta < e^\delta. $$

(b) Similarly, for $\delta<0$,
$$ 1
> \frac{\sigmoid(l+\delta)}{\sigmoid(l)}
= \frac{1 + e^{-l}}{1 + e^{-l-\delta}}
= \frac{e^l + 1}{e^{l+\delta} + 1} e^\delta > e^\delta. \qed $$

\medbreak\f
Now, consider the effect of applying one of the update rules,
$$ \lambda_y \assign
\lambda_y + \delta, \quad\text{where } \delta =
\frac1{C^y}
\ln\Bigl(\frac{\bold c^{y-}\cdot \bold i}{\bold c^{y+}\cdot \bold i}\Bigr), $$
on the constraint $\bold c^{y+} \cdot \bold i = \bold c^{y-} \cdot \bold i$.

We have $\bold i_x = \sigmoid(l_x)$, where $l_x = \bold m_x/T_x + \sum_{y\in Y}
\lambda_y \bold c^y_x$, for each $x\from X$.
The update rule $\lambda_y := \lambda_y + \delta$ causes $\bold i_x$ to be
updated to $\bold i_x' = \sigmoid(l_x+\delta\bold c^y_x)$, for each $x\from
X$.

\case1{$\bold c^{y+} \cdot \bold i < \bold c^{y-} \cdot \bold i$}
Then $\delta>0$.

For each $x \from X$ such that $\bold c^y_x > 0$, part~(a) of the lemma gives
$$ 1 < \frac{\sigmoid(l_x + \delta\bold c^y_x)}{\sigmoid(l_x)} <
e^{\delta\bold c^y_x} \le
e^{\delta C^{y+}} $$
i.e., $1 < \bold i_x'/\bold i_x < e^{\delta C^{y+}}$.
Hence, taking a weighted sum over all such $x$,
$$ 1 < \frac{\bold c^{y+} \cdot \bold i'}{\bold c^{y+} \cdot \bold i}
< e^{\delta C^{y+}}. $$
For each $x \from X$ such that $\bold c^y_x < 0$, part~(b) of the lemma gives
$$ 1 > \frac{\sigmoid(l_x + \delta\bold c^y_x)}{\sigmoid(l_x)} > e^{\delta\bold c^y_x}
\ge e^{-\delta C^{y-}} $$
i.e., $1 > \bold i_x'/\bold i_x > e^{-\delta C^{y-}}$.
Hence, taking a weighted sum over all such $x$,
$$ 1 > \frac{\bold c^{y-} \cdot \bold i'}{\bold c^{y-} \cdot \bold i}
> e^{-\delta C^{y-}}. $$
Dividing the inequalities gives
$$ 1 <
\frac{\bold c^{y+} \cdot \bold i'/\bold c^{y-} \cdot \bold i'}
{\bold c^{y+} \cdot \bold i/\bold c^{y-} \cdot \bold i}
< e^{\delta C^y}
= \frac{\bold c^{y-} \cdot \bold i}{\bold c^{y+} \cdot \bold i}. $$
Hence
$$ \frac{\bold c^{y+} \cdot \bold i}{\bold c^{y-} \cdot \bold i}
< \frac{\bold c^{y+} \cdot \bold i'}{\bold c^{y-} \cdot \bold i'}
< 1. $$
This shows that, after the update, the constraint $\bold c^{y+} \cdot \bold i 
= \bold c^{y-} \cdot \bold i$ is closer to being satisfied than it was
before.

\medbreak

\case2{$\bold c^{y+} \cdot \bold i > \bold c^{y-} \cdot \bold i$}
Then $\delta<0$.

For each $x \from X$ such that $\bold c^y_x > 0$, part~(b) of the lemma gives
$$ 1 > \frac{\sigmoid(l_x + \delta\bold c^y_x)}{\sigmoid(l_x)} 
> e^{\delta\bold c^y_x} \ge e^{\delta C^{y+}} $$
i.e., $1 > \bold i_x'/\bold i_x > e^{\delta C^{y+}}$.
Hence, taking a weighted sum over all such $x$,
$$ 1 > \frac{\bold c^{y+} \cdot \bold i'}{\bold c^{y+} \cdot \bold i}
> e^{\delta C^{y+}}. $$
For each $x \from X$ such that $\bold c^y_x < 0$, part~(a) of the lemma gives
$$ 1 < \frac{\sigmoid(l_x + \delta\bold c^y_x)}{\sigmoid(l_x)} < e^{\delta\bold c^y_x}
\le e^{-\delta C^{y-}} $$
i.e., $1 < \bold i_x'/\bold i_x < e^{-\delta C^{y-}}$.
Hence, taking a weighted sum over all such $x$,
$$ 1 < \frac{\bold c^{y-} \cdot \bold i'}{\bold c^{y-} \cdot \bold i}
< e^{-\delta C^{y-}}. $$
Dividing the inequalities gives
$$ 1 > 
\frac{\bold c^{y+} \cdot \bold i'/\bold c^{y-} \cdot \bold i'}
{\bold c^{y+} \cdot \bold i/\bold c^{y-} \cdot \bold i}
> e^{\delta C^y}
= \frac{\bold c^{y-} \cdot \bold i}{\bold c^{y+} \cdot \bold i}. $$
Hence
$$ \frac{\bold c^{y+} \cdot \bold i}{\bold c^{y-} \cdot \bold i}
> \frac{\bold c^{y+} \cdot \bold i'}{\bold c^{y-} \cdot \bold i'}
> 1. $$
This shows that, after the update, the constraint $\bold c^{y+} \cdot \bold i 
= \bold c^{y-} \cdot \bold i$ is closer to being satisfied than it was
before.

\case3{$\bold c^{y+} \cdot \bold i = \bold c^{y-} \cdot \bold i$}
Then $\delta=0$ and no change is made.

\medbreak
Thus, for each constraint
$\bold c^{y+} \cdot \bold i = \bold c^{y-} \cdot \bold i$, the update rule for
$\lambda_y$ moves $\bold i$
closer to satisfying the constraint. This does not imply that $\bold i$ moves
closer to satisfying \i{all} the constraints, still less does it prove
convergence to an $\bold i$ satisfying all the constraints, but it does provide
some motivation for the update rules used.

\subhead{7.5 The recognition process}
We can now refine further the account of the recognition process. During recognition
$\bold i$, and hence $(i,j)$, is determined by maximising
$$ E = \sum_{x\in X} \frac{\bold i_x \bold m_x}{T_x}
-\sum_{x\in X} \bigl(
\bold i_x \ln \bold i_x + (1-\bold i_x) \ln (1-\bold i_x)
\bigr) $$
subject to the constraints $\forall y\from Y \ \bold c^y \cdot \bold i = 0$,
given temperatures $T_x$ for each $x\from X$. (Here, $\bold i$ is the inclusion
vector corresponding to the pair of inclusion functions $(i,j)$ on the pattern
$\N_1$, and $\bold m$ is calculated using the image $I$, the embedding token $u$
on $\N_1$, and the embedding type $v \circ p$ on $\N_1$.)

In the final stages of recognition, all the temperatures will converge to the
minimum allowed temperature $T_{min}>0$ and so each $\bold i_x$ is likely to
approach $0$ or $1$, and is then rounded to $0$ or $1$, giving
$$ E = \frac{IM(I, \N_1, u, v\circ p, i, j, B)}{T_{min}}. $$
Hence maximising $E$ reduces to maximising $IM(I, \N_1, u, v\circ p, i, j, B)$.
As pointed out in \S6.6, this maximises $DM(I,\N_1,u,v\circ p)$ for the final
pattern.

\vfill\supereject
\runninghead{8. The structural operations}

\head{8. The Structural Operations}

\subhead{8.1 Introduction}
In this section I shall define the \i{structural operations} by which the pattern
is incrementally grown during recognition. There are four kinds:

\blob pruning operations,

\blob extension operations,

\blob merging two symbol tokens,

\blob partitioning a symbol token into two.

\subhead{8.2 Pruning operations}

\defn Given a network $\N=\network{}$ and a pair $(i,j)$ of inclusion
functions on $\N$, a \i{pruning operation} is a transformation from $\N$ to a
subnetwork $\N'=\network{'}$ such that
$$ \forall \sigma\from\Sigma\setdiff\Sigma'\ i(\sigma) = 0, \quad
\forall n\from N\setdiff N'\ i(n) = 0, \quad \forall e\from E\setdiff E'\ i(e)
= 0. $$
A pruning operation is \i{trivial} iff $\N'=\N$.

\theorem 38. For any pruning operation from $\N$ to $\N'$, given a
pair $(i,j)$ of inclusion functions on $\N$,

\item{(i)} $\forall \sigma\from\Sigma\setdiff\Sigma' \ j(\sigma) = 0, \quad
\forall h\from H\setdiff H'\ j(h) = 0, \quad
\forall k\from (K\setdiff\dom(G))\setdiff (K'\setdiff\dom(G'))\ j(k) = 0$,

\item{(ii)} $(i|_{\Sigma'\cup N'\cup E'}, j|_{\Sigma'\cup N'\cup H'\cup
(K'\setdiff\dom(G'))})$ is a pair of inclusion functions on $\N'$ (called the
\i{restriction of $(i,j)$ to $\N'$}).

\proof (i) For any $\sigma\from\Sigma\setdiff\Sigma'$,
$$ i(\sigma) = j(\sigma) \ + \sum_{n\in P\preo\sigma} \hskip-3mm (1-g_n)i(n) $$
where $i(\sigma)=0$; moreover, the condition $P(N') \subseteq \Sigma'$ implies
that each $n\from P\preo\sigma$ is in $N\setdiff N'$ and so $i(n)=0$. Hence
$j(\sigma)=0$.

For any $h\from H\setdiff H'$, we have $h \notin H'=A\pre{N'\cup\Sigma'}$, so
$A(h) \notin N'\cup\Sigma'$, which means $A(h) \in N\setdiff N' \ \cup\
\Sigma\setdiff\Sigma'$, so $i(A(h)) = 0$. By the condition
$$ i(A(h)) = j(h) \ + \sum_{e\in F\preo h} \hskip-3mm i(e) \ +
\sum_{e\in S\preo h} \hskip-3mm i(e) $$
this implies $j(h) = 0$.

For any $k\from (K\setdiff\dom(G))\setdiff (K'\setdiff\dom(G'))$, since
$\dom(G') \subseteq \dom(G)$ we have $k \notin K'=C\pre{E'}$, so $C(k) \in
E\setdiff E'$, so $i(C(k)) = 0$. By the condition
$$ i(C(k)) = j(k) + \sum_{k^* \mid G(k,k^*)} i(C(k^*)) $$
this implies $j(k) = 0$.

(ii) Define $i'=i|_{\Sigma'\cup N'\cup E'}$, $j'=j|_{\Sigma'\cup N'\cup H'\cup
(K'\setdiff\dom(G'))}$, and $I = id_{\Sigma'\cup N'\cup H' \cup E' \cup K'}$.
The condition
$$\forall \sigma\from\Sigma \quad i(\sigma)
= j(\sigma) \ + \sum_{n\in P\preo\sigma} \hskip-3mm (1-g_n)i(n) $$
implies the same condition for $(i',j')$ on $\N'$. We need to check that the
value of $g_n$ is the same in both cases, i.e., $\bigl|\comp{n^*\from
N'}{G'(n^*,n)}\bigr|=\bigl|\comp{n^*\from N}{G(n^*,n)}\bigr|$ for every $n\from
N'$. In fact, for any $n\from N'$, using $G' = G \circ I$,
$$ \bigl|\comp{n^*\from N'}{G'(n^*,n)}\bigr| = |G' \circ id_{\{n\}}|
= |G \circ I \circ id_{\{n\}}|
= |G \circ id_{\{n\}}|
= \bigl|\comp{n^*\from N}{G(n^*,n)}\bigr| $$
as required. Moreover, $\sum_{n\in P\preo\sigma} (1-g_n)i(n) = \sum_{n\in
P'{}\preo\sigma} (1-g_n)i'(n)$, since the right-hand side merely omits terms
$(1-g_n)i(n)$ for which $i(n)=0$.

Secondly, the condition
$$ \forall n \from N \quad i(W(n)) = j(n) + i(n) $$
implies the same condition for $(i',j')$ on $\N'$.

Thirdly, the condition
$$ \forall h\from H \quad i(A(h)) = j(h) \ +
\sum_{e\in F\preo h} \hskip-3mm i(e)
\ + \sum_{e\in S\preo h} \hskip-3mm i(e) $$
implies the same condition for $(i',j')$ on $\N'$. We have $\sum_{e\in F\preo h}
i(e) = \sum_{e\in F'{}\preo h} i'(e)$, since the right-hand side merely omits
terms $i(e)$ that are equal to $0$; and similarly $\sum_{e\in S\preo h} i(e) =
\sum_{e\in S'{}\preo h} i'(e)$.

Fourthly, the condition
$$ \forall k \from K\setdiff dom(G) \quad
i(C(k)) = j(k) + \sum_{k^* \mid G(k,k^*)} i(C(k^*)) $$
implies the same condition for $(i',j')$ on $\N'$. For any $k\from
K'\setdiff\dom(G')$, we have $k \in K\setdiff dom(G)$ by theorem~24(iii), so
$i(C(k)) = j(k) + \sum_{k^* \mid G(k,k^*)} i(C(k^*))$. Also,
$$ \comp{k^*}{G'(k,k^*)} = \comp{k^*}{G(k,k^*) \wedge k^* \in K'}
= \comp{k^*}{G(k,k^*) \wedge C(k^*) \in E'} $$
by $G' = G \circ I$. Thus $\comp{k^*}{G'(k,k^*)} \subseteq
\comp{k^*}{G(k,k^*)}$, and any $k^*$ in the latter set but not in the former has
$C(k^*) \notin E'$ and so $i(C(k^*))=0$. This shows that $\sum_{k^* \mid
G'(k,k^*)} i'(C'(k^*)) = \sum_{k^* \mid G(k,k^*)} i(C(k^*))$.

This completes the verification that $(i',j')$ is a pair of inclusion functions
on $\N'$. \qed

\medskip\f
In practice we may confine ourselves to elementary pruning operations,
involving removal of a single symbol, node or edge.

\defn Given a network $\N=\network{}$ and a pair of inclusion functions $(i,j)$
on $\N$, an \i{elementary pruning operation} is one of the following operations.

\medskip

\item{(i)} \i{Pruning a symbol $\sigma\from\Sigma$} transforms $\N$ to
$\N'=\network{'}$, where

$\Sigma' = \Sigma \setdiff \bigl( \{\sigma\} \cup
\comp{\sigma^*}{G(\sigma,\sigma^*)} \bigr)$, \quad $N' = W\pre{\Sigma'} \cap
P\pre{\Sigma'}$, \quad $H' = A\pre{N' \cup \Sigma'}$,

$E' = F\pre{H'} \cap S\pre{H'}$, \quad $K' = C\pre{E'}$,

$W' = W|_{N'\cup\Sigma'}$, \quad $P' = P|_{N'}$, \quad $A' = A|_{H'}$, \quad $F'
= F|_{E'}$, \quad $S' = S|_{E'}$, \quad $C' = C|_{K'}$,

$G' = id_{\Sigma'\cup N'\cup H'\cup E'\cup K'} \circ G \circ id_{\Sigma'\cup
N'\cup H'\cup E'\cup K'}$.

\item{} This operation is permitted provided
$\forall\sigma^*\from\Sigma\setdiff\Sigma'\ i(\sigma^*)=0$ and $\forall n\from
P\pre{\Sigma\setdiff\Sigma'}\ i(n)=0$.

\medskip

\item{(ii)} \i{Pruning a node $n\from N$} transforms $\N$ to $\N'=\network{'}$,
where

$\Sigma' = \Sigma$, \quad $N' = N \setdiff \bigl( \{n\} \cup
\comp{n^*}{G(n,n^*)} \bigr)$, \quad $H' = A\pre{N' \cup \Sigma'}$,

$E' = F\pre{H'} \cap S\pre{H'}$, \quad $K' = C\pre{E'}$,

$W' = W|_{N'\cup\Sigma'}$, \quad $P' = P|_{N'}$, \quad $A' = A|_{H'}$, \quad $F'
= F|_{E'}$, \quad $S' = S|_{E'}$, \quad $C' = C|_{K'}$,

$G' = id_{\Sigma'\cup N'\cup H'\cup E'\cup K'} \circ G \circ id_{\Sigma'\cup
N'\cup H'\cup E'\cup K'}$.

\item{} This operation is permitted provided $\forall n^*\from N\setdiff N'\
i(n^*)=0$.

\medskip

\item{(iii)} \i{Pruning an edge $e\from E$} transforms $\N$ to
$\N'=\network{'}$, where

$\Sigma' = \Sigma$, \quad $N' = N$, \quad $H' = H$, \quad $E' = E \setdiff
\bigl( \{e\} \cup \comp{e^*}{G(e,e^*)} \bigr)$, \quad $K' = C\pre{E'}$,

$W' = W$, \quad $P' = P$, \quad $A' = A$, \quad $F' = F|_{E'}$, \quad $S' =
S|_{E'}$, \quad $C' = C|_{K'}$,

$G' = id_{\Sigma'\cup N'\cup H'\cup E'\cup K'} \circ G \circ id_{\Sigma'\cup
N'\cup H'\cup E'\cup K'}$.

\item{} This operation is permitted provided $\forall e^*\from E\setdiff E'\
i(e^*)=0$.

\theorem 39. All elementary pruning operations are pruning operations.

\proof Let the network be $\N=\network{}$ and the inclusion functions be $i,j$.

(i) Consider pruning a symbol $\sigma\from\Sigma$, producing $\N'=\network{'}$.
We must show that $\N'$ is a subnetwork of $\N$. The only condition that is not
obvious is $G \circ id_{\Sigma'\cup N'\cup H'\cup E'\cup K'} \subseteq
id_{\Sigma'\cup N'\cup H'\cup E'\cup K'} \circ G$. This is proved in five parts.

First, $G \circ id_{\Sigma'} \subseteq id_{\Sigma'} \circ G$ is verified as
follows. For any $\sigma_1,\sigma_2\from\Sigma$, if $(G \circ
id_{\Sigma'})(\sigma_1,\sigma_2)$ then $G(\sigma_1,\sigma_2)$ and $\sigma_2 \in
\Sigma'$, so $\sigma_2 \ne \sigma$ and $G(\sigma,\sigma_2)$ does not hold. This
implies that $\sigma_1 \ne \sigma$ and $G(\sigma,\sigma_1)$ does not hold (by $G
\circ G = \bot$). This gives $\sigma_1 \in \Sigma'$, and hence $(id_{\Sigma'}
\circ G)(\sigma_1,\sigma_2)$, as required.

The condition $G \circ id_{N'} \subseteq id_{N'} \circ G$ is verified as
follows.
$$\eqqalign\quad{
G \circ id_{N'}
&= G \circ id_N \circ id_{N'}
= id_N \circ G \circ id_{N'}
\subseteq id_{N\cup\Sigma} \circ G \circ id_{N'} \kern-80pt
&\cr
&\subseteq \overline W\inv \circ G \circ \overline W \circ id_{N'}
&\text{from $\overline W \circ G \subseteq G \circ \overline W$ by
theorem~2(iv)}\cr
&\subseteq \overline W\inv \circ G \circ id_{\Sigma'} \circ \overline W
&\text{since $N' \subseteq W\pre{\Sigma'}$}\cr
&\subseteq \overline W\inv \circ id_{\Sigma'} \circ G \circ \overline W
&\text{since $G \circ id_{\Sigma'} \subseteq id_{\Sigma'} \circ G$}\cr
&= id_{W\pre{\Sigma'}} \circ \overline W\inv \circ G \circ \overline W
&\cr
}$$
so by theorem~4(vi)
$$ G \circ id_{N'} \subseteq id_{W\pre{\Sigma'}} \circ G $$
and similarly
$$ G \circ id_{N'} \subseteq id_{P\pre{\Sigma'}} \circ G $$
so
$$\eqqalign\quad{
G \circ id_{N'}
&\subseteq id_{W\pre{\Sigma'}} \circ G \ \cap\ id_{P\pre{\Sigma'}} \circ G
&\cr
&= id_{W\pre{\Sigma'}} \circ (G \cap id_{P\pre{\Sigma'}} \circ G)
&\text{by theorem~4(iv)}\cr
&= id_{W\pre{\Sigma'}} \circ id_{P\pre{\Sigma'}} \circ (G \cap G)
&\text{by theorem~4(iv)}\cr
&= id_{N'} \circ G.
&\cr
}$$

The condition $G \circ id_{H'} \subseteq id_{H'} \circ G$ is verified as
follows.
$$\eqqalign\quad{
G \circ id_{H'}
&= G \circ id_H \circ id_{H'}
= id_H \circ G \circ id_{H'} \kern-40pt
&\cr
&\subseteq \overline A\inv \circ G \circ \overline A \circ id_{H'}
&\text{from $\overline A \circ G \subseteq G \circ \overline A$ by
theorem~2(iv)}\cr
&= \overline A\inv \circ G \circ id_{N'\cup\Sigma'} \circ \overline A
&\text{since $H' = A\pre{N'\cup\Sigma'}$}\cr
&\subseteq \overline A\inv \circ id_{N'\cup\Sigma'} \circ G \circ \overline A
&\text{since $G \circ id_{\Sigma'} \subseteq id_{\Sigma'} \circ G$ and
$G \circ id_{N'} \subseteq id_{N'} \circ G$}\cr
&= id_{H'} \circ \overline A\inv \circ G \circ \overline A
&\text{since $H' = A\pre{N'\cup\Sigma'}$}\cr
}$$
so by theorem~4(vi)
$$ G \circ id_{H'} \subseteq id_{H'} \circ G. $$

The condition $G \circ id_{E'} \subseteq id_{E'} \circ G$ is verified as
follows.
$$\eqqalign\quad{
G \circ id_{E'}
&= G \circ id_E \circ id_{E'}
= id_E \circ G \circ id_{E'} \kern-40pt
&\cr
&\subseteq \overline F\inv \circ G \circ \overline F \circ id_{E'}
&\text{from $\overline F \circ G \subseteq G \circ \overline F$ by
theorem~2(iv)}\cr
&\subseteq \overline F\inv \circ G \circ id_{H'} \circ \overline F
&\text{since $E' \subseteq F\pre{H'}$}\cr
&\subseteq \overline F\inv \circ id_{H'} \circ G \circ \overline F
&\text{since $G \circ id_{H'} \subseteq id_{H'} \circ G$}\cr
&= id_{F\pre{H'}} \circ \overline F\inv \circ G \circ \overline F
&\cr
}$$
so by theorem~4(vi)
$$ G \circ id_{E'} \subseteq id_{F\pre{H'}} \circ G $$
and similarly
$$ G \circ id_{E'} \subseteq id_{S\pre{H'}} \circ G $$
so
$$\eqqalign\quad{
G \circ id_{E'}
&\subseteq id_{F\pre{H'}} \circ G \ \cap\ id_{S\pre{H'}} \circ G
&\cr
&= id_{F\pre{H'}} \circ (G \cap id_{S\pre{H'}} \circ G)
&\text{by theorem~4(iv)}\cr
&= id_{F\pre{H'}} \circ id_{S\pre{H'}} \circ (G \cap G)
&\text{by theorem~4(iv)}\cr
&= id_{E'} \circ G.
&\cr
}$$

Finally, the condition $G \circ id_{K'} \subseteq id_{K'} \circ G$ is verified
as follows.
$$\eqqalign\quad{
G \circ id_{K'}
&= G \circ id_K \circ id_{K'}
= id_K \circ G \circ id_{K'} \kern-40pt
&\cr
&\subseteq \overline C\inv \circ G \circ \overline C \circ id_{K'}
&\text{from $\overline C \circ G \subseteq G \circ \overline C$ by
theorem~2(iv)}\cr
&= \overline C\inv \circ G \circ id_{E'} \circ \overline C
&\text{since $K' = C\pre{E'}$}\cr
&\subseteq \overline C\inv \circ id_{E'} \circ G \circ \overline C
&\text{since $G \circ id_{E'} \subseteq id_{E'} \circ G$}\cr
&= id_{K'} \circ \overline C\inv \circ G \circ \overline C
&\text{since $K' = C\pre{E'}$}\cr
}$$
so by theorem~4(vi)
$$ G \circ id_{K'} \subseteq id_{K'} \circ G. $$
It follows then that $G \circ id_{\Sigma'\cup N'\cup H'\cup E'\cup K'} \subseteq
id_{\Sigma'\cup N'\cup H'\cup E'\cup K'} \circ G$ and hence $\N'$ is a
subnetwork of $\N$.

We also need to verify the conditions on the inclusion functions for a pruning
operation.

The first condition, $\forall\sigma^*\from\Sigma\setdiff\Sigma'\ i(\sigma^*)=0$,
is given.

The second condition, $\forall n\from N\setdiff N'\ i(n)=0$, is verified as
follows. For any $n\from N\setdiff N'$, we have $n \notin W\pre{\Sigma'}$ or
$n\notin P\pre{\Sigma'}$. In the former case, $W(n) \in \Sigma\setdiff\Sigma'$,
so $i(W(n))=0$, so, by the constraint $i(W(n)) = j(n) + i(n)$, we have $i(n)=0$
as required. In the latter case, $n \in P\pre{\Sigma\setdiff\Sigma'}$, so we are
given that $i(n)=0$ as required.

The third condition, $\forall e\from E\setdiff E'\ i(e)=0$, is verified as
follows. For any $e\from E\setdiff E'$, we have $e \notin F\pre{H'}$ or $e
\notin S\pre{H'}$. In the former case, $F(e) \notin H'$, so $A(F(e)) \notin N'
\cup \Sigma'$, so $i(A(F(e)))=0$. Hence by the constraint $\forall h\from H\
i(A(h)) = j(h) \ + \sum_{e\in F\preo h} i(e) \ + \sum_{e\in S\preo h} i(e)$ it
follows that $i(e)=0$ as required. The latter case is similar.

This completes the proof that pruning $\sigma$ is a pruning operation.

(ii) Consider pruning a node $n\from N$, producing $\N'=\network{'}$. The
verification that $\N'$ is a subnetwork of $\N$ is similar to the one in part
(i), but simpler. We also need to verify the conditions on the inclusion
functions for a pruning operation.

The first condition, $\forall\sigma\from\Sigma\setdiff\Sigma'\ i(\sigma)=0$, is
vacuously true because $\Sigma'=\Sigma$.

The second condition, $\forall n^*\from N\setdiff N'\ i(n^*)=0$, is given.

The third condition, $\forall e\from E\setdiff E'\ i(e)=0$, is verified exactly
as in part (i).

(iii) Consider pruning an edge $e\from E$, producing $\N'=\network{'}$. The
verification that $\N'$ is a subnetwork of $\N$ is similar to the one in part
(i), but simpler. We also need to verify the conditions on the inclusion
functions for a pruning operation.

The first two conditions, $\forall\sigma\from\Sigma\setdiff\Sigma'\ i(\sigma)=0$
and $\forall n\from N\setdiff N'\ i(n)=0$, are vacuously true because
$\Sigma'=\Sigma$ and $N'=N$.

The third condition, $\forall e^*\from E\setdiff E'\ i(e^*)=0$, is given. \qed

\medskip\f
The following theorem shows why it is sufficient to restrict attention to
elementary pruning operations.

\theorem 40. If any non-trivial pruning operation is possible on a network
then an elementary pruning operation is possible on it.

\proof Consider a network $\N=\network{}$ with inclusion functions $i,j$ and
suppose that a non-trivial pruning operation is possible on it, producing a
proper subnetwork $\N'=\network{'}$. Then there exists
$\sigma\from\Sigma\setdiff\Sigma'$ or $n\from N\setdiff N'$ or $h\from H\setdiff
H'$ or $e\from E\setdiff E'$ or $k\from K\setdiff K'$. However, note that if
$h\from H\setdiff H'$ then $A(h) \in N\setdiff N' \cup \Sigma\setdiff\Sigma'$,
since $H'=A\pre{N'\cup\Sigma'}$; and if $k\in K\setdiff K'$ then $C(k) \in
E\setdiff E'$ since $K'=C\pre{E'}$. So we can infer that there exists
$\sigma\from\Sigma\setdiff\Sigma'$ or $n\from N\setdiff N'$ or $e\from E\setdiff
E'$.

Consider the case where there exists $\sigma\from\Sigma\setdiff\Sigma'$. Then
$\forall\sigma^*\from\Sigma\ (G(\sigma,\sigma^*) \Rightarrow \sigma^* \in
\Sigma\setdiff\Sigma')$, by the condition $G \circ id_{\Sigma'\cup N'\cup H'\cup
E'\cup K'} \subseteq id_{\Sigma'\cup N'\cup H'\cup E'\cup K'} \circ G$. Defining
a set $\Sigma_0=\{\sigma\} \cup \comp{\sigma^*}{G(\sigma,\sigma^*)}$, we then
have $\Sigma_0 \subseteq \Sigma\setdiff\Sigma'$, so
$\forall\sigma^*\from\Sigma_0\ i(\sigma^*)=0$; moreover the condition
$P(N')\subseteq \Sigma'$ implies $P\pre{\Sigma_0} \subseteq N\setdiff N'$ and
hence $\forall n\from P\pre{\Sigma_0}\ i(n)=0$. Hence we can perform on $\N$ the
elementary pruning operation of pruning $\sigma$, giving a subnetwork
$\N''=\network{''}$, with $\Sigma''=\Sigma\setdiff\Sigma_0$.

Next consider the case where there exists $n\from N\setdiff N'$. Then $\forall
n^*\from N\ (G(n,n^*) \Rightarrow n^* \in N\setdiff N')$, by the condition $G
\circ id_{\Sigma'\cup N'\cup H'\cup E'\cup K'} \subseteq id_{\Sigma'\cup N'\cup
H'\cup E'\cup K'} \circ G$. Defining a set $N_0=\{n\} \cup
\comp{n^*}{G(n,n^*)}$, we then have $N_0 \subseteq N\setdiff N'$, so $\forall
n^*\from N_0\ i(n^*)=0$. Hence we can perform on $\N$ the elementary pruning
operation of pruning $n$, giving a subnetwork $\N''=\network{''}$, with
$N''=N\setdiff N_0$.

Finally consider the case where there exists $e\from E\setdiff E'$. Then
$\forall e^*\from E\ (G(e,e^*) \Rightarrow e^* \in E\setdiff E')$, by the
condition $G \circ id_{\Sigma'\cup N'\cup H'\cup E'\cup K'} \subseteq
id_{\Sigma'\cup N'\cup H'\cup E'\cup K'} \circ G$. Defining a set $E_0=\{e\}
\cup \comp{e^*}{G(e,e^*)}$, we then have $E_0 \subseteq E\setdiff E'$, so
$\forall e^*\from E_0\ i(e^*)=0$. Hence we can perform on $\N$ the elementary
pruning operation of pruning $e$, giving a subnetwork $\N''=\network{''}$, with
$E''=E\setdiff E_0$.

Hence in all cases an elementary pruning operation is possible. \qed

\theorem 41. If a pruning operation is carried out on a network $\N$, given a
pair of inclusion functions $(i,j)$ on $\N$, resulting in a subnetwork $\N'$,
then, for any image $I$ and any embedding token $u$, embedding type $v$ and
bareness function $B$ for $\N$,
$$ IM(I, \N', u', v', i', j', B') = IM(I, \N, u, v, i, j, B) $$
where $u',v',i',j',B'$ are the restrictions of $u,v,i,j,B$ to $\N'$. Moreover,
the symmetry condition holds for $\N',u',v'$ if it holds for $\N,u,v$.

\proof We use the usual notation, $\N=\network{}$, $\N'=\network{'}$,
$v=(sub,\allowbreak con,\allowbreak rel,\allowbreak symm,\allowbreak tem,
\allowbreak in)$, $v'=(sub',\allowbreak con',\allowbreak rel',\allowbreak
symm',\allowbreak tem', \allowbreak in')$. By the definition of a pruning
operation and theorem~38(i),
$$\eqalign{
&\forall\sigma\from\Sigma\setdiff\Sigma'\ i(\sigma) = 0 = j(\sigma), \quad
\forall n\from N\setdiff N'\ i(n) = 0, \quad
\forall h\from H\setdiff H'\ j(h) = 0,
\cr&
\forall e\from E\setdiff E'\ i(e) = 0, \quad
\forall k\from (K\setdiff\dom(G))\setdiff (K'\setdiff\dom(G'))\ j(k) = 0.
}$$
This implies that the pruning operation makes no difference to the value of
$IM$. The only term for which this is not obvious is
$\sum_{(\sigma,\sigma^*)\mid G(\sigma,\sigma^*)} i(\sigma^*)
E_{sub(\sigma,\sigma^*)}(u(\sigma)\inv \cdot u(\sigma^*))$. Since $G'_\Sigma =
G_\Sigma \circ id_{\Sigma'}$ (by theorem~24(i)), the difference
$$ \sum_{(\sigma,\sigma^*)\mid G(\sigma,\sigma^*)} i(\sigma^*)
E_{sub(\sigma,\sigma^*)}(u(\sigma)\inv \cdot u(\sigma^*))
\ - \sum_{(\sigma,\sigma^*)\mid G'(\sigma,\sigma^*)} i'(\sigma^*)
E_{sub'(\sigma,\sigma^*)}(u'(\sigma)\inv \cdot u'(\sigma^*)) $$
is the sum of $i(\sigma^*) E_{sub(\sigma,\sigma^*)}(u(\sigma)\inv \cdot
u(\sigma^*))$ over pairs $(\sigma,\sigma^*)$ having $\sigma^* \in
\Sigma\setdiff\Sigma'$, and for such pairs the term vanishes since $i(\sigma^*)
= 0$.

The symmetry condition for $\N',u',v'$ immediately follows from the one for
$\N,u,v$.\qed

\medbreak\f
Pruning is used in the recognition process as follows. We have a pattern
$\N_1$, a parse $p:\N_1\to\N_0$, an embedding token $u$ for $\N_1$, and a pair
of inclusion functions $(i,j)$ on $\N_1$. We carry out an elementary pruning
operation on $\N_1$ to give a subnetwork $\N_1'$, with a new parse
$p|_{\N_1'}:\N_1'\to\N_0$ (\S3.7), a new embedding token $u|_{\N_1'}$ (\S4.2),
and a new pair of inclusion functions, the restriction of $(i,j)$ to $\N_1'$
(theorem~38(ii)).

\subhead{8.3 Unprunability and its consequences}

\defn A network $\N=\network{}$ is \i{unprunable}, given a pair of
inclusion functions $(i,j)$ on $\N$, iff there is no proper subnetwork
$\N'=\network{'}$ of $\N$ satisfying
$$ \forall \sigma\from\Sigma\setdiff\Sigma'\ i(\sigma) = 0, \quad
\forall n\from N\setdiff N'\ i(n) = 0, \quad
\forall e\from E\setdiff E'\ i(e) = 0. $$

\medskip\f
(In other words, a network is unprunable iff no non-trivial pruning operation is
possible on it, or, equivalently by theorem~40, iff no elementary pruning
operation is possible on it.)

\theorem 42. If

\item{(a)} $\N_1=\network{_1}$ is a network,

\item{(b)} $p:\N_1\to\N_0$ is a homomorphism, where $\N_0$ is a semi-definite
network,

\item{(c)} $(i,j)$ is a pair of inclusion functions on $\N_1$ satisfying
$\forall x\from \Sigma_1 \cup N_1 \cup E_1 \ i(x) \in \{0, 1\}$,

\item{(d)} $\N_1$ is unprunable, given $(i,j)$,

\smallskip\f
then $\forall e\from E_1\ i(e) = 1$.

\proof Consider the pruning operation that transforms $\N_1$ to
$\N_2=\network{_2}$, where

$\Sigma_2 = \Sigma_1, \quad N_2 = N_1, \quad H_2 = H_1, \quad E_2 = \comp{e\from
E_1}{i(e)=1}, \quad K_2 = C_1\pre{E_2},$

$W_2 = W_1, \quad P_2 = P_1, \quad A_2 = A_1, \quad F_2 = F_1|_{E_2}, \quad S_2
= S_1|_{E_2}, \quad C_2 = C_1|_{K_2},$

$G_2 = id_{\Sigma_2\cup N_2\cup H_2\cup E_2\cup K_2} \circ G_1 \circ
id_{\Sigma_2\cup N_2\cup H_2\cup E_2\cup K_2}$.

\smallskip\f
I shall show that this is indeed a pruning operation, and then since $\N_1$ is
assumed unprunable it will follow that $\N_2=\N_1$.

First we check that $\N_2$ is a subnetwork of $\N_1$. The conditions
$$ W_1(N_2) \subseteq \Sigma_2, \quad P_1(N_2) \subseteq \Sigma_2, \quad
H_2 = A_1\pre{N_2\cup\Sigma_2}, \quad F_1(E_2) \subseteq H_2, \quad
S_1(E_2) \subseteq H_2 $$
are immediate, since $\Sigma_2=\Sigma_1$, $N_2=N_1$ and $H_2=H_1$. The condition
$K_2 = C_1\pre{E_2}$ holds by definition.

The functions $W_2,P_2,A_2,F_2,S_2,C_2$ are as they ought to be for a
subnetwork.

To verify $G_1 \circ id_{\Sigma_2\cup N_2\cup H_2\cup E_2 \cup K_2} \subseteq
id_{\Sigma_2\cup N_2\cup H_2\cup E_2\cup K_2} \circ G_1$ we need the following
derivations.

For every $k,k^*\from K_1$ such that $G_1(k,k^*)$, we have $k \in \ran(G_1)$, so
$k \notin \dom(G_1)$, so
$$ i(C_1(k)) = j(k) + \sum_{k'|G_1(k,k')} i(C_1(k')) \ge i(C_1(k^*)); $$
thus if $k^* \in K_2$ then $C_1(k^*) \in E_2$, so $i(C_1(k^*))=1$, so
$i(C_1(k))=1$, so $C_1(k) \in E_2$, so $k \in K_2$. This shows
$$ G_{1K} \circ id_{K_2} \subseteq id_{K_2} \circ G_{1K}. \eqno (1) $$
Next,
$$\eqqalignno\quad{
G_{1E} \circ id_{E_2}
&= \overline{C_1} \circ G_{1K} \circ \overline{C_1}\inv \circ id_{E_2}
&\text{by theorem~20(iv)} \cr
&= \overline{C_1} \circ G_{1K} \circ id_{K_2} \circ \overline{C_1}\inv
&\text{since $K_2 = C_1\pre{E_2}$} \cr
&\subseteq \overline{C_1} \circ id_{K_2} \circ G_{1K} \circ \overline{C_1}\inv
&\text{by (1)} \cr
&= id_{E_2} \circ \overline{C_1} \circ G_{1K} \circ \overline{C_1}\inv
&\text{since $K_2 = C_1\pre{E_2}$} \cr
&= id_{E_2} \circ G_{1E}
&\text{by theorem~20(iv).} \cr
}{(2)} $$
Next,
$$ G_1 \circ id_{\Sigma_2\cup N_2\cup H_2}
= G_{1\Sigma} \cup G_{1N} \cup G_{1H}
= id_{\Sigma_2\cup N_2\cup H_2} \circ G_1 \eqno(3) $$
since $\Sigma_2=\Sigma_1$, $N_2=N_1$ and $H_2=H_1$. Combining (1), (2) and (3)
gives
$$ G_1 \circ id_{\Sigma_2\cup N_2\cup H_2\cup E_2\cup K_2}
\subseteq id_{\Sigma_2\cup N_2\cup H_2\cup E_2\cup K_2} \circ G_1 $$
as required. Thus $\N_2$ is indeed a subnetwork of $\N_1$. The remaining
conditions for a pruning operation,
$$ \forall \sigma\from\Sigma_1\setdiff\Sigma_2\ i(\sigma) = 0, \quad
\forall n\from N_1\setdiff N_2\ i(n) = 0, \quad
\forall e\from E_1\setdiff E_2\ i(e) = 0, $$
hold by definition of $\Sigma_2,N_2,E_2$.

Since $\N_1$ is assumed unprunable, given $(i,j)$, it follows that $\N_2=\N_1$.
This means that $E_2=E_1$ and so $\forall e\from E_1\ i(e)=1$. \qed

\theorem 43. If

\item{(a)} $\N_1=\network{_1}$ is a network,

\item{(b)} $p:\N_1\to\N_0$ is a homomorphism, where $\N_0$ is a semi-definite
network,

\item{(c)} $(i,j)$ is a pair of inclusion functions on $\N_1$ satisfying

$\forall x\from \Sigma_1 \cup N_1 \cup E_1 \ i(x) \in \{0, 1\}, \quad \forall
h\from H_1\ j(h)=0, \quad \forall k\from K_1\setdiff\dom(G_1)\ j(k)=0$,

\item{(d)} $\N_1$ is unprunable, given $(i,j)$,

\smallskip\f
then

\smallskip

\item{(i)} $\forall e\from E_1\ i(e) = 1$,

\item{(ii)} $\forall n\from N_1\ i(n) = 1$,

\item{(iii)} $E_1 \buildrel F_1 \over \rightarrow A_1\pre{N_1\cup Y} \buildrel
S_1 \over \leftarrow E_1$ is a sum diagram in the category of sets, where
$Y=\comp{\sigma\from\Sigma_1}{i(\sigma)=1}$,

\item{(iv)} $\exists f:K_1\setdiff\dom(G_1) \to K_1 \ G_{1K}\inv = \overline
f$,

\item{(v)} $\forall n\from N_1\ i(W_1(n)) = 1 = i(P_1(n))$,

\item{(vi)} $\forall X \subseteq\Sigma_1\ |P_1\pre X| - |G_{1N} \circ
id_{P_1\pre X}| \le |X|$.

\proof (i) is given by theorem~42.

(ii) Consider the pruning operation that transforms $\N_1$ to
$\N_2=\network{_2}$, where

$\Sigma_2 = \Sigma_1, \quad N_2 = \comp{n\from N_1}{i(n)=1}, \quad H_2 =
A_1\pre{N_2\cup\Sigma_2}, \quad E_2 = E_1, \quad K_2 = K_1,$

$W_2 = W_1|_{N_2\cup\Sigma_2}, \quad P_2 = P_1|_{N_2}, \quad A_2 = A_1|_{H_2},
\quad F_2 = F_1, \quad S_2 = S_1, \quad C_2 = C_1,$

$G_2 = id_{\Sigma_2\cup N_2\cup H_2\cup E_2\cup K_2} \circ G_1 \circ
id_{\Sigma_2\cup N_2\cup H_2\cup E_2\cup K_2}$.

\smallskip\f
I shall show that this is indeed a pruning operation, and then since $\N_1$ is
assumed unprunable it will follow that $\N_2=\N_1$.

First we check that $\N_2$ is a subnetwork of $\N_1$. The conditions $W_1(N_2)
\subseteq \Sigma_2$ and $P_1(N_2) \subseteq \Sigma_2$, are immediate, since
$\Sigma_2=\Sigma_1$.

Define $Y=\comp{\sigma\from\Sigma_1}{i(\sigma)=1}$ (as in part (iii) in the
statement of the theorem). For any $h\from H_1$, we have the condition
$$ i(A_1(h)) = j(h) \ + \sum_{e\in F_1\preo h} \hskip-3mm i(e)
\ + \sum_{e\in S_1\preo h} \hskip-3mm i(e) $$
where $j(h)=0$; so $h \in A_1\pre{N_2 \cup Y}$ iff $i(A_1(h))=1$ iff there
exists $e\from F_1\preo h$ or $e\from S_1\preo h$ (where such an $e$ is unique
and belongs to just one of the two sets). This means that
$$ E_1 \buildrel F_1 \over \rightarrow A_1\pre{N_2\cup Y} \buildrel
S_1 \over \leftarrow E_1 \text{ is a sum diagram.} \eqno (1) $$
This implies $F_1(E_1) \subseteq A_1\pre{N_2\cup Y} \subseteq H_2$ and $S_1(E_1)
\subseteq A_1\pre{N_2\cup Y} \subseteq H_2$, as required.

The functions $W_2,P_2,A_2,F_2,S_2,C_2$ are as required for a subnetwork.

To verify $G_1 \circ id_{\Sigma_2\cup N_2\cup H_2\cup E_2 \cup K_2} \subseteq
id_{\Sigma_2\cup N_2\cup H_2\cup E_2\cup K_2} \circ G_1$ we need the following
derivations.

Since $\Sigma_2=\Sigma_1$, $E_2=E_1$ and $K_2=K_1$,
$$\eqalign{
G_1 \circ id_{\Sigma_2} &= G_{1\Sigma} = id_{\Sigma_2} \circ G_1, \cr
G_1 \circ id_{E_2} &= G_{1E} = id_{E_2} \circ G_1, \cr
G_1 \circ id_{K_2} &= G_{1K} = id_{K_2} \circ G_1.
} \eqno(2) $$
Next,
$$\eqqalignno{\kern3pt}{
G_{1H} \circ id_{A_1\pre{N_2}}
&\subseteq G_{1H} \circ id_{A_1\pre{N_2\cup Y}}
&\cr
&= G_{1H} \circ \bigl( \overline{F_1} \circ \overline{F_1}\inv \ \cup \
\overline{S_1} \circ \overline{S_1}\inv \bigr)
&\text{by theorem~7 and (1)} \cr
&= G_{1H} \circ \overline{F_1} \circ \overline{F_1}\inv \ \cup \
G_{1H} \circ \overline{S_1} \circ \overline{S_1}\inv
& \cr
&= G_1 \circ \overline{F_1} \circ \overline{F_1}\inv \ \cup \
G_1 \circ \overline{S_1} \circ \overline{S_1}\inv
& \cr
&= \overline{F_1} \circ G_1 \circ \overline{F_1}\inv \ \cup \
\overline{S_1} \circ G_1 \circ \overline{S_1}\inv
&\text{by theorem~20(ii)} \cr
&= \overline{F_1} \circ id_{E_1} \circ G_1 \circ \overline{F_1}\inv \ \cup \
\overline{S_1} \circ id_{E_1} \circ G_1 \circ \overline{S_1}\inv
& \cr
&\subseteq id_{H_2} \circ \overline{F_1} \circ G_1 \circ \overline{F_1}\inv \
\cup \ id_{H_2} \circ \overline{S_1} \circ G_1 \circ \overline{S_1}\inv
&\text{since $F_1(E_1) \subseteq H_2$} \cr
&= id_{H_2} \circ G_1 \circ \overline{F_1} \circ \overline{F_1}\inv
\ \cup \ id_{H_2} \circ G_1 \circ \overline{S_1} \circ \overline{S_1}\inv
&\text{by theorem~20(ii)} \cr
&\subseteq id_{H_2} \circ G_1 \circ id_{H_1} \ \cup \
id_{H_2} \circ G_1 \circ id_{H_1}
&\text{by theorem~2(i)} \cr
&= id_{H_2} \circ G_{1H}.
&\cr
}{\kern-30pt(3)}$$
Next, from $\overline{A_1} \circ G_1 \subseteq G_1 \circ \overline{A_1}$ we have
$$\eqqalign\quad{
G_{1H} \circ id_{A_1\pre{\Sigma_2}}
&\subseteq \overline{A_1}\inv \circ G_1 \circ \overline{A_1} \circ
id_{A_1\pre{\Sigma_2}}
&\text{by theorem~2(iv)}\cr
&= \overline{A_1}\inv \circ G_1 \circ id_{\Sigma_2} \circ \overline{A_1}
&\cr
&= \overline{A_1}\inv \circ id_{\Sigma_2} \circ G_1 \circ \overline{A_1}
&\text{by (2)}\cr
&\subseteq id_{H_2} \circ \overline{A_1}\inv \circ G_1 \circ \overline{A_1}
&\text{since $A_1\pre{\Sigma_2} \subseteq H_2$}\cr
}$$
so by theorem~4(vi)
$$ G_{1H} \circ id_{A_1\pre{\Sigma_2}} \subseteq id_{H_2} \circ G_{1H}. \eqno(4)
$$
Hence,
$$\eqqalignno\quad{
G_{1H} \circ id_{H_2}
&= G_{1H} \circ id_{A_1\pre{N_2 \cup \Sigma_2}}
&\cr
&= G_{1H} \circ id_{A_1\pre{N_2}} \ \cup\ G_{1H} \circ id_{A_1\pre{\Sigma_2}}
&\cr
&\subseteq id_{H_2} \circ G_{1H}
&\text{by (3) and (4).}\cr
}{(5)}$$
Next,
$$\eqqalignno\quad{
G_{1N} \circ id_{N_2}
&= id_{N_1} \circ \overline{A_1} \circ G_{1H} \circ \overline{A_1}\inv \circ
id_{N_2}
&\text{by theorem~20(iii)} \cr
&\subseteq id_{N_1} \circ \overline{A_1} \circ G_{1H} \circ id_{H_2} \circ
\overline{A_1}\inv
&\text{since $A_1\pre{N_2} \subseteq H_2$} \cr
&\subseteq id_{N_1} \circ \overline{A_1} \circ id_{H_2} \circ G_{1H} \circ
\overline{A_1}\inv
&\text{by (5)} \cr
&= id_{N_1} \circ id_{N_2\cup\Sigma_2} \circ \overline{A_1} \circ G_{1H} \circ
\overline{A_1}\inv
&\text{since $H_2 = A_1\pre{N_2\cup\Sigma_2}$} \cr
&= id_{N_2} \circ id_{N_1} \circ \overline{A_1} \circ G_{1H} \circ
\overline{A_1}\inv
& \cr
&= id_{N_2} \circ G_{1N}
&\text{by theorem~20(iii).} \cr
}{(6)}$$
From (2), (5) and (6),
$$ G_1 \circ id_{\Sigma_2\cup N_2\cup H_2\cup E_2\cup K_2} \subseteq
id_{\Sigma_2\cup N_2\cup H_2\cup E_2\cup K_2} \circ G_1. $$
Thus $\N_2$ is indeed a subnetwork of $\N_1$. The remaining conditions for a
pruning operation,
$$ \forall \sigma\from\Sigma_1\setdiff\Sigma_2\ i(\sigma) = 0, \quad
\forall n\from N_1\setdiff N_2\ i(n) = 0, \quad
\forall e\from E_1\setdiff E_2\ i(e) = 0, $$
hold by definition of $\Sigma_2,N_2,E_2$.

Since $\N_1$ is assumed unprunable, given $(i,j)$, it follows that $\N_2=\N_1$.
This means that $N_2=N_1$ and so $\forall n\from N_1\ i(n)=1$.

(iii) follows from (1), bearing in mind that $N_2=N_1$.

(iv) For any $k \from K_1 \setdiff \dom(G_1)$,
$$ i(C_1(k)) = j(k) + \sum_{k^*\mid G_1(k,k^*)} i(C_1(k^*)) $$
where $i(C_1(k)) = 1$, $j(k) = 0$, and each $i(C_1(k^*)) = 1$, by part (i) and
hypothesis~(c), so there exists a unique $k^*$ such that $G_1(k,k^*)$. Define
$f:K_1\setdiff\dom(G_1) \to K_1$ mapping $k$ to this $k^*$. On the other hand,
for any $k \from K_1 \wedge \dom(G_1)$, we have $k \notin \ran(G_1)$, so there
exists no $k^*$ such that $G_1(k,k^*)$. Thus $G_{1K}\inv = \overline f$.

(v) $\forall n\from N_1\ i(W_1(n)) = 1$ holds since, for any $n\from N_1$,
$$ i(W_1(n)) = j(n) + i(n) $$
where $i(n) = 1$ by part (ii), so $i(W_1(n)) = 1$.

The other equation, $\forall n\from N_1\ i(P_1(n)) = 1$, is proved using
theorem~21 and theorem~13. The hypotheses of theorem~21 hold, by parts (iii) and
(iv) just proved. Theorem~21 then tells us that $G_{1N}$ is acyclic. The next
step is to apply theorem~13 to the sets $N_1,\Sigma_1$, the function
$P_1:N_1\to\Sigma_1$ and the finite relation $G_{1N}$ on $N_1$. Let us check the
hypotheses of theorem~13.

Hypothesis (a): $G_{1N} \circ G_{1N} \subseteq G_1 \circ G_1 = \bot$ (since
$\N_1$ is a network).

Hypothesis (b): $G_{1N}$ is acyclic (as just shown).

Hypothesis (c): $\overline{P_1} \circ G_{1N} = \overline{P_1} \circ G_1
\subseteq \overline{P_1}$ (since $\N_1$ is a network).

\smallskip\f
Now, for any $\sigma\from\Sigma_1$ such that $i(\sigma)=0$, taking $X =
\{\sigma\}$ in theorem~13(i) gives
$$ |P_1\preo\sigma| - |G_{1N} \circ id_{P_1\preo\sigma}| \ge 0. $$
Moreover, (recalling the notation $g_n = \bigl|\comp{n^*\from
N_1}{G_1(n^*,n)}\bigr|$)
$$\eqalign{
0 = i(\sigma)
&= j(\sigma) \ + \sum_{n\in P_1\preo\sigma} \hskip-3mm (1-g_n)i(n)
= j(\sigma) \ + \sum_{n\in P_1\preo\sigma} \hskip-3mm (1-g_n)
\cr&
= j(\sigma) + |P_1\preo\sigma| -
|\comp{(n^*,n)\from N_1\times P_1\preo\sigma}{G_1(n^*,n)}|
\cr&
= j(\sigma) + |P_1\preo\sigma| - |G_{1N} \circ id_{P_1\preo\sigma}|
}$$
so $j(\sigma)=0$ and $|P_1\preo\sigma| - |G_{1N} \circ id_{P_1\preo\sigma}| =
0$. Then by theorem~13(ii) $P_1\preo\sigma = \emptyset$. The contrapositive of
this result is that if $P_1\preo\sigma \ne \emptyset$ then $i(\sigma)=1$. Thus
$\forall n\from N_1\ i(P_1(n)) = 1$, as required.

(vi) For any $\sigma\from\Sigma_1$,
$$\eqalign{
i(\sigma)
&= j(\sigma) \ + \sum_{n\in P_1\preo\sigma} \hskip-3mm (1-g_n)i(n)
= j(\sigma) + |P_1\preo\sigma| - |G_{1N} \circ id_{P_1\preo\sigma}|
}$$
as in part (v), where $i(\sigma) \in \{0,1\}$ and $j(\sigma) \in [0,1]$, so
$$ |P_1\preo\sigma| - |G_{1N} \circ id_{P_1\preo\sigma}| \le 1. $$
For any $X \subseteq\Sigma_1$, summing this inequality over all $\sigma\from X$
gives
$$ |P_1\pre X| - |G_{1N} \circ id_{P_1\pre X}| \le |X| $$
as required. \qed

\theorem 44. If

\item{(a)} $\N_1=\network{_1}$ is a network,

\item{(b)} $p:\N_1\to\N_0$ is a homomorphism, where $\N_0$ is a semi-definite
network,

\item{(c)} $(i,j)$ is a pair of inclusion functions on $\N_1$ satisfying

\smallskip

$\forall x\from \Sigma_1 \cup N_1 \cup E_1 \ i(x) \in \{0, 1\}$,\quad $\forall
h\from H_1 \ j(h) = 0$,\quad $\forall k\from K_1 \setdiff \dom(G_1)\ j(k) = 0$,

\smallskip

\item{(d)} $\N_1$ is unprunable, given $(i,j)$,

\item{(e)} $E_1 \doublearrow{A_1 \circ F_1}{A_1 \circ S_1} N_1\cup\Sigma_1
\buildrel W_1 \over \rightarrow \Sigma_1$ is a coequaliser diagram in the
category of sets,

\smallskip\f
then

\smallskip

\item{(i)} $\forall x\from \Sigma_1\cup N_1\cup E_1\ i(x) = 1$,

\item{(ii)} $\N_1$ is definite.

\proof The hypotheses of this theorem include those of theorem~43, so we can
apply theorem~43.

(i) From theorem~43(i),(ii) we already have $\forall e\from E_1\ i(e) = 1$ and
$\forall n\from N_1\ i(n) = 1$. Consider the pruning operation that transforms
$\N_1$ to $\N_2=\network{_2}$, where

$\Sigma_2 = \comp{\sigma\from\Sigma_1}{i(\sigma)=1}, \quad N_2 = N_1, \quad H_2=
A_1\pre{N_2\cup\Sigma_2}, \quad E_2 = E_1, \quad K_2 = K_1,$

$W_2 = W_1|_{N_2\cup\Sigma_2}, \quad P_2 = P_1, \quad A_2 = A_1|_{H_2}, \quad
F_2 = F_1, \quad S_2 = S_1, \quad C_2 = C_1,$

$G_2 = id_{\Sigma_2\cup N_2\cup H_2\cup E_2\cup K_2} \circ G_1 \circ
id_{\Sigma_2\cup N_2\cup H_2\cup E_2\cup K_2}$.

\smallskip\f
I shall show that this is indeed a pruning operation, and then since $\N_1$ is
assumed unprunable it will follow that $\N_2=\N_1$.

First we check that $\N_2$ is a subnetwork. The first two conditions, $W_1(N_2)
\subseteq \Sigma_2$ and $P_1(N_2) \subseteq \Sigma_2$ follow from
theorem~43(v).

Theorem~43(iii) tells us that
$$ E_1 \buildrel F_1 \over \rightarrow H_2 \buildrel
S_1 \over \leftarrow E_1 \text{ is a sum diagram} \eqno (1) $$
since $H_2 = A_1\pre{N_2\cup\Sigma_2} = A_1\pre{N_1\cup Y}$. This implies
$F_1(E_2) \subseteq H_2$ and $S_1(E_2) \subseteq H_2$, as required.

The functions $W_2,P_2,A_2,F_2,S_2,C_2$ are as required for a subnetwork.

Next we verify the condition $G_1 \circ id_{\Sigma_2\cup N_2\cup H_2\cup E_2\cup
K_2} \subseteq id_{\Sigma_2\cup N_2\cup H_2\cup E_2\cup K_2} \circ G_1$.

The hypotheses of theorem~22 are satisfied (with $Y=\Sigma_2$). Theorem~22(iii)
gives
$$ G_1 \circ id_{\Sigma_2} \subseteq id_{\Sigma_2} \circ G_1. \eqno(2) $$
The conditions
$$\eqalignno{
G_1 \circ id_{N_2} &= id_{N_2} \circ G_1 &(3)\cr
G_1 \circ id_{E_2} &= id_{E_2} \circ G_1 &(4)\cr
G_1 \circ id_{K_2} &= id_{K_2} \circ G_1 &(5)
}$$
hold trivially, since $N_2=N_1$, $E_2=E_1$ and $K_2=K_1$. Also,
$$\eqqalign\quad{
G_1 \circ id_{H_2}
&= id_{H_1} \circ G_1 \circ id_{H_2}
&\text{since $H_2 \subseteq H_1$}\cr
&\subseteq \overline{A_1}\inv \circ G_1 \circ \overline{A_1} \circ id_{H_2}
&\text{from $\overline{A_1} \circ G_1 \subseteq G_1 \circ \overline{A_1}$ by
theorem~2(iv)}\cr
&= \overline{A_1}\inv \circ G_1 \circ id_{N_2\cup \Sigma_2} \circ
\overline{A_1}
&\text{since $H_2 = A_1\pre{N_2\cup\Sigma_2}$}\cr
&\subseteq \overline{A_1}\inv \circ id_{N_2\cup \Sigma_2} \circ G_1 \circ
\overline{A_1}
&\text{by (3) and (2)}\cr
&= id_{H_2} \circ \overline{A_1}\inv \circ G_1 \circ \overline{A_1}
&\text{since $H_2 = A_1\pre{N_2\cup\Sigma_2}$}\cr
}$$
and hence by theorem~4(vi)
$$ G_1 \circ id_{H_2} \subseteq id_{H_2} \circ G_1. \eqno(6) $$
From (2), (3), (4), (5) and (6) we derive $G_1 \circ id_{\Sigma_2\cup N_2\cup
H_2\cup E_2\cup K_2} \subseteq id_{\Sigma_2\cup N_2\cup H_2\cup E_2\cup K_2}
\circ G_1$. Hence $\N_2$ is indeed a subnetwork of $\N_1$.

The conditions
$$\forall \sigma\from\Sigma_1\setdiff\Sigma_2\ i(\sigma) = 0, \quad
\forall n\from N_1\setdiff N_2\ i(n) = 0, \quad
\forall e\from E_1\setdiff E_2\ i(e) = 0 $$
follow immediately from the definitions of $\Sigma_2,N_2,E_2$. This completes
the verification that we have a pruning operation.

Since $\N_1$ is assumed to be unprunable, given $(i,j)$, the pruning operation
must be the trivial one, with $\N_2=\N_1$. This means that $\Sigma_2=\Sigma_1$
and so $\forall\sigma\from\Sigma_1\ i(\sigma)=1$, as required.

(ii) We shall apply theorem~23; let us check its hypotheses.

Hypothesis (a) holds by theorem~43(vi).

Hypothesis (b), that $E_1 \buildrel F_1 \over \rightarrow H_1 \buildrel S_1
\over \leftarrow E_1$ is a sum diagram, follows from (1) and the fact that
$\N_2=\N_1$.

Hypothesis (c) holds by theorem~27(iv).

Hypothesis (d) holds by hypothesis (e) of this theorem.

Thus it follows by theorem~23 that $\N_1$ is definite. \qed

\subhead{8.4 Extension operations}
Given a grammar $\N_0$, a pattern $\N_1$, a homomorphism $p:\N_1\to\N_0$, and an
embedding token $u$ for $\N_1$, an \i{extension} of $(\N_1,p,u)$ is a triple
$(\N_1',p',u')$ where $\N_1$ is a subnetwork of $\N_1'$, $p':\N_1'\to\N_0$ is a
homomorphism such that $p = p'|_{\N_1}$, and $u'$ is an embedding token for
$\N_1'$ such that $u = u'|_{\N_1}$.

$(\N_1',p',u')$ is a \i{minimal} extension of $(\N_1,p,u)$ satisfying a
condition $P$ iff

\smallskip

\item{(i)} $(\N_1',p',u')$ is an extension of $(\N_1,p,u)$ satisfying $P$;

\item{(ii)} for any extension $(\N_1'',p'',u'')$ of $(\N_1,p,u)$ satisfying $P$,
$|\N_1'| \le |\N_1''|$,

\smallskip\f
where the cardinality $|\N|$ of a network $\N$ is defined by $|\network{}| =
|\Sigma| + |N| + |H| + |E| + |K|$.

An extension is \i{trivial} iff $\N_1'=\N_1$.

\medbreak\f
Using these notions we can define the extension operations used in the
algorithm. The notation is as usual: we have a grammar $\N_0=\network{_0}$
and an embedding type $v = (sub,\allowbreak
con,\allowbreak rel,\allowbreak symm,\allowbreak tem, \allowbreak in)$ on
$\N_0$, a pattern $\N_1=\network{_1}$ with a parse $p:\N_1\to\N_0$, an embedding
token $u$, a pair of inclusion functions $(i,j)$, and a bareness function
$B$ for $\N_1$; we shall produce an extended network $\N_1'=\network{_1'}$
with a new parse $p':\N_1'\to\N_0$ and embedding token $u'$. The
threshold $\theta$ is the positive constant used in the $DM$ function (see
\S4.5); the thresholds $\theta_0,\theta_1,\theta_2,\theta_3,\theta_4$ are 
used only in the extension operations and may be made dependent on parameters
such as temperature.

In the extension operations the following additional conditions, referred to
collectively as \i{the extension conditions}, will be imposed.

\blob $\forall\sigma\from\Sigma_1\ ({P_1'}\preo\sigma \not\subseteq N_1 \imp 
j(\sigma) > \theta_0 \and B(\sigma) < \theta)$,

\blob $\forall h\from H_1\ ({F_1'}\preo h \cup {S_1'}\preo h
\not\subseteq E_1 \imp j(h) > \theta_0)$,

\blob $\forall e\from E_1'\ (A_1'(F_1'(e)) \notin N_1 \OR
A_1'(S_1'(e)) \notin N_1 \imp W_1'(A_1'(F_1'(e))) = W_1'(A_1'(S_1'(e))))$,

\blob $\forall n \in N_1'\setdiff N_1 \ \
E_{con(p'(n))}(u'(W_1'(n))\inv \cdot u'(n)) < \theta_1$,

\blob the symmetry condition for $\N_1',u',v \circ p'$.

\medskip\f
The \i{extension operations} are as follows (see figure~1 below). For each one,
the extension conditions are checked at the end and the operation is cancelled
if they do not hold. (Note that no consistent pair of inclusion functions
$(i',j')$ can be specified for the extended pattern $\N_1'$, so we recalculate 
them as in \S7.4, using the old inclusion functions $(i,j)$ as a starting 
point.)

\medskip\f
(a) (Joining two symbols.) Given symbols $\sigma_1,\sigma_2 \from \Sigma_1$, an
edge $e_0 \from E_0$, and affine transformations $s_1 \from symm(p(\sigma_1))$
and $s_2 \from symm(p(\sigma_2))$ such that

\blob $P_0(A_0(F_0(e_0))) = p(\sigma_1)$ and $P_0(A_0(S_0(e_0))) = p(\sigma_2)$,

\blob $E_{rel(e_0)}(s_2\inv \cdot u(\sigma_2)\inv \cdot u(\sigma_1) \cdot s_1)
< \theta_2$,

\medskip\f
construct a minimal extension $(\N_1',p',u')$ of $(\N_1,p,u)$ (if one exists)
such that $\N_1'$ contains nodes $n_1,n_2$ and an edge $e$ for which

\blob $p'(e)=e_0$, $A_1'(F_1'(e))=n_1$, $A_1'(S_1'(e)) = n_2$,
$P_1'(n_1) = \sigma_1$ and $P_1'(n_2) = \sigma_2$,

\blob $u'(n_1) = u(\sigma_1) \cdot s_1$ and $u'(n_2) = u(\sigma_2) \cdot s_2$.

\medskip\f
(b) (Joining three symbols.) Given symbols
$\sigma_1,\sigma_2,\sigma_3\from\Sigma_1$, edges $e_{01},e_{02}\from E_0$,
$s_1\from symm(p(\sigma_1))$, $s_2\from symm(p(\sigma_2))$ and $s_3\from
symm(p(\sigma_3))$ such that

\blob $A_0(S_0(e_{01}))=A_0(F_0(e_{02}))$, $P_0(A_0(F_0(e_{01})))=p(\sigma_1)$,
$P_0(A_0(S_0(e_{01})))=p(\sigma_2)$ and
$P_0(A_0(S_0(e_{02})))\allowbreak=p(\sigma_3)$,

\blob $E_{rel(e_{01})}(s_2\inv \cdot u(\sigma_2)\inv\cdot u(\sigma_1) \cdot s_1)
+ E_{rel(e_{02})}(s_3\inv \cdot u(\sigma_3)\inv \cdot u(\sigma_2) \cdot s_2) <
\theta_3$,

\medskip\f
construct a minimal extension $(\N_1',p',u')$ of $(\N_1,p,u)$ (if one exists)
such that $\N_1'$ contains nodes $n_1,n_2,n_3$ and edges $e_1,e_2$ for which

\blob $p'(e_1)=e_{01}$, $p'(e_2)=e_{02}$, $A_1'(F_1'(e_1)) = n_1$,
$A_1'(S_1'(e_1))=n_2=A_1'(F_1'(e_2))$, $A_1'(S_1'(e_2))=n_3$,
$P_1'(n_1)=\sigma_1$, $P_1'(n_2)=\sigma_2$ and $P_1'(n_3)=\sigma_3$,

\blob $u'(n_1)=u(\sigma_1)\cdot s_1$, $u'(n_2)=u(\sigma_2)\cdot s_2$ and
$u'(n_3)=u(\sigma_3)\cdot s_3$.

\medskip\f
(There are also variations of operation~(b), in which the directions of $e_{01}$
and $e_1$ are reversed, or the directions of $e_{02}$ and $e_2$ are reversed.)

\medskip\f
(c) (Extending from a hook.) Given a hook $h\from H_1$, construct a minimal
extension $(\N_1',p',u')$ of $(\N_1,p,u)$ such that

\blob $p'({F_1'}\inv(\{h\})) = F_0\inv(p(\{h\}))$ and $p'({S'_1}\inv(\{h\})) =
S_0\inv(p(\{h\}))$,

\blob $\forall e\from E_1'\setdiff E_1\ \ E_{rel(p'(e))}(u'(A_1'(S_1'(e)))\inv
\cdot u'(A_1'(F_1'(e)))) = 0$.

\medskip\f
(d) (Extending from a facet.) Given a facet $k\from K_1$ such that

\blob $W_1(A_1(F_1(C_1(k))))=W_1(A_1(S_1(C_1(k))))$

\blob $j(k) > \theta_0$,

\medskip\f
construct a minimal extension $(\N_1',p',u')$ of $(\N_1,p,u)$ such that

\blob $\overline{p'} \circ {G_1'}\inv \circ id_{\{k\}} = G_0\inv \circ
\overline p \circ id_{\{k\}}$.

\medskip\f
(e) (Extending from a part to a whole.) Given a symbol $\sigma\from\Sigma_1$,
construct a minimal extension $(\N_1',p',u')$ of $(\N_1,p,u)$ such that

\blob $p'({P_1'}\pre{\{\sigma\}}) = P_0\pre{p(\{\sigma\})}$,

\blob $\forall n\from N_1'\setdiff N_1\ E_{con(p'(n))}(u'(W_1'(n))\inv \cdot
u'(n)) = 0$.

\medskip\f
(f) (Filling in a missing part between two parts.) Given nodes $n_1,n_3\from
N_1$, hooks $h_1,h_3\from H_1$, edges $e_{01},e_{02}\from E_0$ and an affine
transformation $f$ such that

\blob $W_1(n_1)=W_1(n_3)$, $A_1(h_1)=n_1$, $A_1(h_3)=n_3$,
$A_0(S_0(e_{01}))=A_0(F_0(e_{02}))$, $F_0(e_{01})=p(h_1)$ and
$S_0(e_{02})=p(h_3)$,

\blob $E_{rel(e_{01})}(f\inv \cdot u(n_1)) + E_{rel(e_{02})}(u(n_3)\inv \cdot f)
< \theta_4$,

\medskip\f
construct a minimal extension $(\N_1',p',u')$ of $(\N_1,p,u)$ (if one exists)
such that $\N_1'$ contains edges $e_1,e_2$ and a node $n_2$ for which

\blob $p'(e_1) = e_{01}$, $p'(e_2) = e_{02}$, $F'_1(e_1) = h_1$,
$A'_1(S'_1(e_1))=n_2=A'_1(F'_1(e_2))$ and $S'_1(e_2) = h_3$,

\blob if $n_2\notin N_1$ then $u'(n_2)=f$.

\medskip\f
(There are also variations of operation~(f), in which the directions of $e_{01}$
and $e_1$ are reversed, or the directions of $e_{02}$ and $e_2$ are reversed.)

\medskip\f
(g) (Filling in a symbol between part and whole.) Given symbols
$\sigma_1,\sigma_3\from\Sigma_1$, symbols \newline
$\sigma_{01},\sigma_{02},\sigma_{03}\from\Sigma_0$, nodes $n_{01},n_{02}\from
N_0$, $s\from symm(\sigma_{03})$, and an affine transformation $f$ such that

\blob $p(\sigma_1)=\sigma_{01}$, $p(\sigma_3)=\sigma_{03}$,
$W_0(n_{01})=\sigma_{01}$, $P_0(n_{01})=\sigma_{02}=W_0(n_{02})$ and
$P_0(n_{02})=\sigma_{03}$,

\blob $E_{con(n_{01})}(u(\sigma_1)\inv \cdot f) +
E_{con(n_{02})}(f\inv \cdot u(\sigma_3) \cdot s) < \theta_4$,

\smallskip\f
construct a minimal extension $(\N_1',p',u')$ of $(\N_1,p,u)$ such that $\N_1'$
contains a symbol $\sigma_2$ and nodes $n_1,n_2$ for which

\blob $p'(n_1)=n_{01}$, $p'(n_2)=n_{02}$, $W_1'(n_1)=\sigma_1$,
$P_1'(n_1)=\sigma_2=W_1(n_2)$ and $P_1'(n_2)=\sigma_3$,

\blob if $n_1 \notin N_1$ then $u'(n_1)=u'(\sigma_2)=f$,

\blob if $n_2 \notin N_1$ then $u'(n_2)=u(\sigma_3)\cdot s$.

\medskip\f
These extension operations are applied concurrently, in a fair order, controlled
by probabilities; the probability is low in cases where new symbols would be
created (particularly operations~(a) and (e)), to avoid the creation of too many
new symbols.

These operations are depicted in figure~1. In this figure rectangles
represent symbols, circles represent nodes, small filled discs represent hooks, lines
with arrowheads halfway along represent edges, and small crosses represent
facets (shown only for operation~(e)); the $W$ and $P$ functions, which map each
node to the whole and part symbols, are represented by lines with arrowheads at
the end. For each operation solid lines are used for the symbols, nodes, etc.,
assumed to be present in the pattern before the extension operation; dashed
lines are used for the symbols, nodes, etc., added by the extension operation
(if they are not already present in $\N_1$). Thus, for example, operation~(g)
adds one symbol and two nodes (and their associated hooks), unless a suitable
symbol or suitable nodes already exist in $\N_1$. Note, however, that whenever
an edge is added the appropriate number of superedges must also be added, in
order that $p'$ satisfy the conditions for a homomorphism; and the same applies
to symbols, nodes, etc.; these are not shown in the figure.

\def\twofigures#1#2#3#4#5{\centerline{\percentsize{#1}\epsfbox{#2}{\hskip #3}
\percentsize{#4}\epsfbox{#5}}\epsfxsize=\hsize}

\def\threefigures#1#2#3#4#5#6#7#8{\centerline{\percentsize{#1}\epsfbox{#2}
{\hskip #3}\percentsize{#4}\epsfbox{#5}{\hskip #6}
\percentsize{#7}\epsfbox{#8}}\epsfxsize=\hsize}

\bigskip

\goodbreak

\twofigures{30}{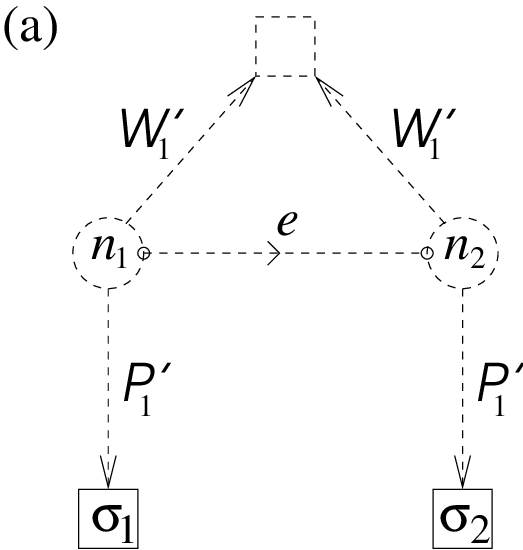}{50pt}{50}{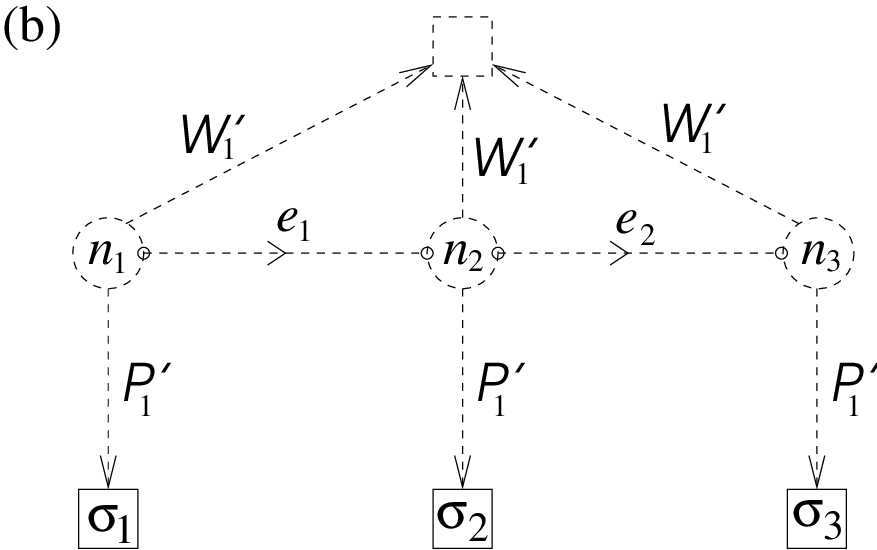}

\bigskip\null\bigskip\null\bigskip

\twofigures{35}{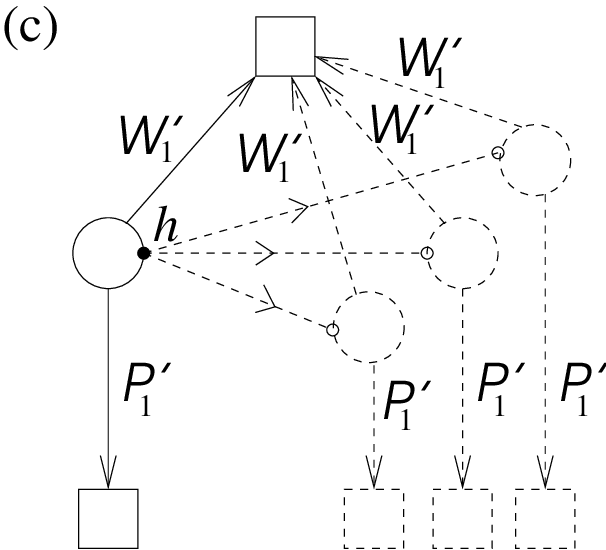}{50pt}{40}{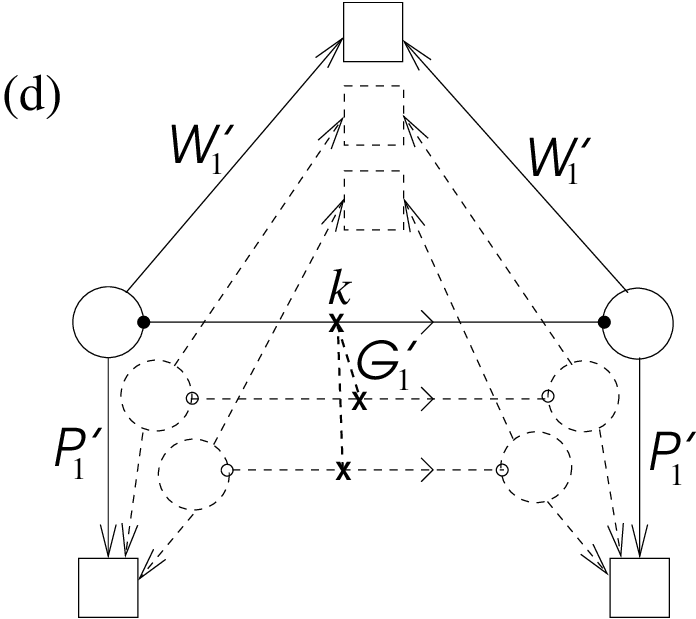}

\bigskip\null\bigskip\null\bigskip

{\nobreak

\threefigures{26}{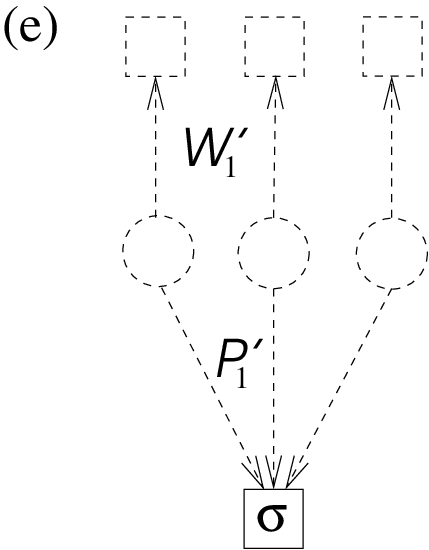}{35pt}{50}{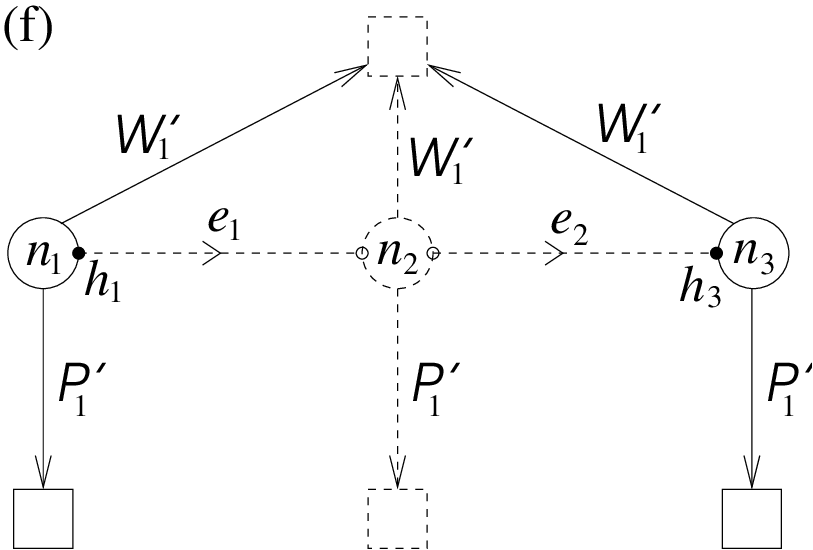}{15pt}{14}{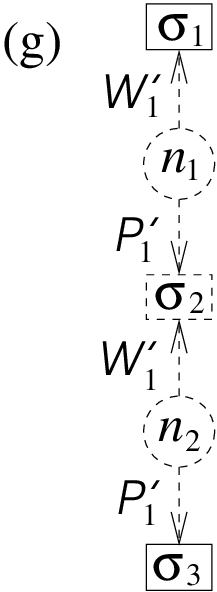}

\bigskip

\longcaption{Figure 1. The extension operations. The figure shows the relevant
parts of the pattern $\N_1'$ after each extension operation. Solid lines depict
what must be present before the operation; dashed lines depict what is added if
not already present.}

}

\subhead{8.5 Inextendability and its consequences}

\defn $(\N_1,p,u)$ is \i{inextendable}, given $i,j,v,B$, iff none of the
extension operations can be applied to it, other than ones giving a trivial
extension.

\theorem 45. If

\item{(a)} $\N_1=\network{_1}$ is a network with an embedding token $u$ and a
bareness function $B$,

\item{(b)} $p:\N_1\to\N_0$ is a homomorphism, where $\N_0$ is a semi-definite
network with an embedding type $v$,

\item{(c)} $(i,j)$ is a pair of inclusion functions on $\N_1$ satisfying
$\forall x\from \Sigma_1 \cup N_1\ i(x) \in \{0, 1\}$ and $\forall e\from E_1\
i(e) = 1$,

\item{(d)} $(\N_1,p,u)$ is inextendable, given $i,j,v,B$,

\item{(e)} $W_1 \circ A_1 \circ F_1 = W_1 \circ A_1 \circ S_1$,

\smallskip\f
then $\forall h\from H_1\ j(h)=0$ and $\forall k\from K_1\setdiff\dom(G_1)\
j(k)=0$.

\proof For any $h\from H_1$, we have
$$ i(A(h)) = j(h) \ + \sum_{e\in F_1\preo h} \hskip-3mm i(e)
\ + \sum_{e\in S_1\preo h} \hskip-3mm i(e). \eqno(1) $$
This implies that $j(h)$ is an integer, and hence must be $0$ or $1$. Suppose
$j(h)=1$. Then the operation of extending from $h$ (extension operation~(c)) is
possible, giving an extension $(\N_1',p',u')$ such that $p'({F_1'}\inv(\{h\})) =
F_0\inv(p(\{h\}))$ and $p'({S'_1}\inv(\{h\})) = S_0\inv(p(\{h\}))$. However, we
are assuming $(\N_1,p,u)$ is inextendable, so $(\N_1',p',u')=(\N_1,p,u)$. Thus
$p(F_1\inv(\{h\})) = F_0\inv(p(\{h\}))$ and $p(S_1\inv(\{h\})) =
S_0\inv(p(\{h\}))$.

Now, $\N_0=\network{_0}$ is semi-definite and so satisfies $F_0(E_0) \cup
S_0(E_0) = H_0$. This means that $F_0\inv(p(\{h\})) \ne \emptyset$ or
$S_0\inv(p(\{h\})) \ne \emptyset$. Hence $p(F_1\inv(\{h\})) \ne \emptyset$ or
$p(S_1\inv(\{h\})) \ne \emptyset$. Hence $F_1\inv(\{h\}) \ne \emptyset$ or
$S_1\inv(\{h\}) \ne \emptyset$. Any edge $e$ in these sets has $i(e)=1$, by
hypothesis (c), so by (1) $i(A(h)) \ge 2$, which is impossible. This
contradiction establishes that $j(h)=0$ as required.

For any $k\from K_1 \setdiff \dom(G_1)$, we have
$$ i(C(k)) = j(k) + \sum_{k^* \mid G_1(k,k^*)} i(C(k^*)). $$
This implies that $j(k)$ is an integer, and hence must be $0$ or $1$. Suppose
$j(k)=1$. Then $\sum_{k^* \mid G_1(k,k^*)} i(C(k^*))=0$, and hence by
hypothesis~(c) there are no $k^*$ such that $G_1(k,k^*)$ holds. This can be
expressed as
$$ G_1\inv \circ id_{\{k\}} = \bot. \eqno(2) $$
Also, since $k\notin \dom(G_1)$ we have
$$ G_1 \circ id_{\{k\}} = \bot. \eqno (3) $$
Now, by hypothesis~(e) and since $j(k)=1$, the operation of extending from $k$
(extension operation~(d)) is possible, giving an extension $(\N_1',p',u')$ such
that $\overline{p'} \circ {G_1'}\inv \circ id_{\{k\}} = G_0\inv \circ \overline
p \circ id_{\{k\}}$. However, we are assuming $(\N_1,p,u)$ is inextendable,
hence $(\N_1',p',u')=(\N_1,p,u)$. Thus
$$ \overline p \circ G_1\inv \circ id_{\{k\}} = G_0\inv \circ \overline p \circ
id_{\{k\}}. \eqno(4) $$
Since $\N_0$ is semi-definite, $G_0$ is minimal relative to $\N_0$ and hence
$id_{K_0} \subseteq G_{0K} \circ G_{0K}\inv \cup G_{0K}\inv \circ G_{0K}$. Then
$$\eqqalign{\kern-9pt}{
\overline p \circ id_{\{k\}}
&\subseteq G_{0K} \circ G_{0K}\inv \circ \overline p \circ id_{\{k\}}\ \cup\
G_{0K}\inv \circ G_{0K} \circ \overline p \circ id_{\{k\}}
&\cr
&\subseteq G_0 \circ G_0\inv \circ \overline p \circ id_{\{k\}}\ \cup\
G_0\inv \circ G_0 \circ \overline p \circ id_{\{k\}}
&\cr
&= G_0 \circ \overline p \circ G_1\inv \circ id_{\{k\}} \ \cup\
G_0\inv \circ \overline p \circ G_1 \circ id_{\{k\}}
&\text{by (4) and since $p$ is a homomorphism}\cr
&= \bot \ \cup \bot = \bot
&\text{by (2) and (3).}\cr
}$$
But this is absurd, since $(\overline p \circ id_{\{k\}})(p(k),k)$ holds. This
contradiction establishes that $j(k)=0$, as required. \qed

\subhead{8.6 Merging two symbol tokens}
We may merge two symbol tokens of the same type that have similar embedding
transformations (up to a symmetry transformation). Two symbol tokens
$\sigma_1,\sigma_2\from\Sigma_1$ of type $\sigma_0\from\Sigma_0$ are considered
to have similar embeddings up to a symmetry transformation iff there exists
$s\in symm(\sigma_0)$ such that $E_{in(\sigma_0)}(s\inv \cdot u(\sigma_2)\inv
\cdot u(\sigma_1))$ is below a threshold. If this condition holds then the
symmetry $s$ is applied to $\sigma_2$ (this is a local symmetry operation; the
other symbols are unchanged); $\sigma_1$ and $\sigma_2$ are replaced by a single
symbol; and the nodes and edges of $\sigma_1$ and $\sigma_2$ are pooled.
Local symmetry operations have already been defined in \S4.3. The merging
itself is formally defined as follows.

\defn Given a network $\N_1=\network{_1}$, and a homomorphism $p:\N_1\to\N_0$,
and two symbols $\sigma_1,\sigma_2\from\Sigma_1$ such that
$p(\sigma_1)=p(\sigma_2)$, 
the operation of \i{merging $\sigma_1$ and $\sigma_2$} produces a new network
$\N_1'=\network{_1'}$ and a homomorphism $\mu:\N_1\to\N_1'$ defined as follows.
First note that there are bijections $p|_{A_1\preo{\sigma_1}}:
A_1\preo{\sigma_1} \to A_0\preo{p(\sigma_1)}$ and
and
$p|_{A_1\preo{\sigma_2}}:
A_1\preo{\sigma_2} \to A_0\preo{p(\sigma_1)}$
and hence a bijection
$\gamma = p|_{A_1\preo{\sigma_1}}\inv \circ p|_{A_1\preo{\sigma_2}}:
A_1\preo{\sigma_2} \to A_1\preo{\sigma_1}$. Now define

$\Sigma_1' = \Sigma_1 \setminus \set{\sigma_2}$,
$N_1' = N_1$,
$H_1' = H_1 \setminus A_1\preo{\sigma_2}$,
$E_1' = E_1$,
$K_1' = K_1$,

\smallskip

$\forall\sigma\from\Sigma_1\ \mu(\sigma) = \cases{
\sigma_1 & if $\sigma=\sigma_2$ \cr
\sigma & otherwise
}$,
$\forall h\from H_1\ \mu(h) = \cases{
\gamma(h) & if $A_1(h) = \sigma_2$ \cr
h & otherwise}$,

\smallskip

$\forall x\from N_1\cup E_1\cup K_1\ \mu(x) = x$

$\forall\sigma\from\Sigma_1'\ W_1'(\sigma) = \sigma$,
$\forall n\from N_1'\ W_1'(n) = \mu(W_1(n))$,

$P_1' = \mu \circ P_1$,
$A_1' = A_1|_{H_1'}$,
$F_1' = \mu \circ F_1$,
$S_1' = \mu \circ S_1$,
$C_1' = C_1$,

$G_1' = \overline\mu \circ G_1 \circ \overline\mu\inv$.

\medbreak\f
This gives the network $\N_1'$ and homomorphism $\mu:\N_1\to\N_1'$. 

Note that $\mu$ is surjective and satisfies 
$\forall x,y\from\Sigma_1\cup N_1\cup H_1\cup
E_1\cup K_1\ (\mu(x)=\mu(y) \imp p(x)=p(y))$, so there exists a unique
function $p'$ such that $p'\circ\mu = p$; this $p'$ is a homomorphism from
$\N_1'$ to $\N_0$. This is the new parse.

If $u$ is the old embedding token on $\N_1$, we can define a new embedding
token $u'$ on $\N_1'$ by
$$ \forall\sigma\from\Sigma_1'\ u'(\sigma) = \cases{
G & if $\sigma=\sigma_1$ \cr
u(\sigma) & otherwise},
\quad
\forall n\from N_1'\ u'(n) = u(n) $$
where $G$ is an affine transformation intermediate between $u(\sigma_1)$ and
$u(\sigma_2) \cdot s$. This is calculated as follows. Find $A\from\A$ such that 
$u(\sigma_2) \cdot s \cdot u(\sigma_1)\inv = \exp(A)$; then choose $G
= \exp(A/2) \cdot u(\sigma_1) = \exp(-A/2) \cdot u(\sigma_2) \cdot s$.

No consistent pair of inclusion functions
$(i',j')$ can be specified for the new network $\N_1'$, so we recalculate 
them as in \S7.4, using the restriction of the old inclusion functions $(i,j)$
to $\N_1'$ as a starting point.

\subhead{8.7 Partitioning a symbol token into two}
Consider any pattern $\N_1=\network{_1}$.
For any $\sigma_0\from\Sigma_1$, if the nodes
and symbol in $W_1\preo{\sigma_0}$ can be partitioned into two disjoint non-empty
subsets $T_1,T_2$, such that there is no edge between any element $T_1$ and
any element of $T_2$, then $\sigma_0$ may be replaced by two symbols, 
$(\sigma_0,1)$ and
$(\sigma_0,2)$, with $(\sigma_0,1)$ getting the nodes of $T_1$ and
$(\sigma_0,2)$ getting the nodes of $T_2$. The subsymbols of $\sigma_0$ are
glued to $(\sigma_0,1)$ or $(\sigma_0,2)$ as appropriate (or duplicated if
necessary). The nodes above $\sigma_0$
must be duplicated; i.e., $n$ is replaced by $(n,i)$ and $(n,j)$, for
two indices $i,j$, and
likewise for their hooks, edges and facets.
This operation is called
\i{partitioning $\sigma_0$}. It is roughly the inverse of the merging operation.

\defn In a network $\network{}$, a symbol $\sigma_0\from\Sigma$ is 
\i{partitionable} iff there exist sets $T_1,T_2$ such that 
$T_1 \cup T_2 = W\preo{\sigma_0}$ and $T_1 \cap T_2 = \emptyset$ and
$T_1,T_2 \ne \emptyset$
and 
$F\pre{A\pre{T_1}} \cap S\pre{A\pre{T_2}} = \emptyset$ and 
$S\pre{A\pre{T_1}} \cap F\pre{A\pre{T_2}} = \emptyset$.

The network $\network{}$ is \i{partitionable} iff at least one symbol in
$\Sigma$ is partitionable; otherwise it is \i{unpartitionable}.

\defn If a symbol $\sigma_0$ is partitionable in $\N=\network{}$, with sets
$T_1,T_2$, then \i{partitioning $\sigma_0$} is the construction of a new
network $\N'$ as follows.

First define a function $I$ on $\Sigma\cup N\cup E$ by

\blob $I(\sigma_0) = \set{1,2}$,

\blob $\forall n\from N \cap T_1\ (I(n) = \set 1 \times I(P(n)) \and \forall n^*\ (G(n,n^*)
\imp I(n^*) = I(n)))$

\blob $\forall n\from N \cap T_2\ (I(n) = \set 2  \times I(P(n))\and \forall n^*\ (G(n,n^*)
\imp I(n^*) = I(n)))$

\blob $\forall \sigma^*\ (G(\sigma_0,\sigma^*) \imp I(\sigma^*) =
\bigcup_{n\in N \cap W\preo{\sigma^*}} proj_1(I(n)))$

\blob for all other $\sigma\from\Sigma$, $I(\sigma) = \set 0$,

\blob for all other $n\from N$, $I(n) = I(W(n)) \times I(P(n))$,

\blob $\forall e\from E\ I(e) = I(A(F(e))) \times I(A(S(e)))$,

\medskip\f where the function $proj_1$ is defined by $\forall(i,j)\
proj_1(i,j) = i$.

Define the new network $\N'=\network{'}$, by

\blob $\Sigma' = \comp{(\sigma,i)}{\sigma\from\Sigma \and i \in I(\sigma)}$,
$N' = \comp{(n,i)}{n\from N \and i \in I(n)}$,

\blob $H' = \comp{(h,i)}{h\from H \and i \in I(A(h))}$,
$E' = \comp{(e,i)}{e\from E \and i \in I(e)}$,

\blob $K' = \comp{(k,i)}{k\from K \and i \in I(C(k))}$,

\blob $\forall(\sigma,i)\from\Sigma'\ W'(\sigma,i) = (\sigma,i)$,
$\forall(n,(i,j))\from N'\ W'(n,(i,j)) = (W(n),i)$,

\blob $\forall(n,(i,j))\from N'\ P'(n,(i,j)) = (P(n),j)$,
$\forall(h,i)\from H'\ A'(h,i) = (A(h),i)$,

\blob $\forall(e,(i,j))\from E'\ F'(e,(i,j)) = (F(e),i)$,
$\forall(e,(i,j))\from E'\ S'(e,(i,j)) = (S(e),j)$,

\blob $\forall(k,i)\from K'\ C'(k,i) = (C(k),i)$,

\blob $\forall(\sigma,i),(\sigma^*,j)\from \Sigma'\ (G'((\sigma,i),(\sigma^*,j))
\iff G(\sigma,\sigma^*) \and c(i,j))$,

\blob $\forall(n,i),(n^*,j)\from N'\ (G'((n,i),(n^*,j)) 
\iff G(n,n^*) \and c_2(i,j))$,

\blob $\forall(h,i),(h^*,j)\from H'\ (G'((h,i),(h^*,j)) 
\iff G(h,h^*) \and c_2(i,j))$,

\blob $\forall(e,i),(e^*,j)\from E'\ (G'((e,i),(e^*,j)) 
\iff G(e,e^*) \and c_4(i,j))$,

\blob $\forall(k,i),(k^*,j)\from K'\ (G'((k,i),(k^*,j)) 
\iff G(k,k^*) \and c_4(i,j))$,

\medskip\f
where 
$$\eqalign{
c(i,j) \ &\iff\  i=j \OR i=0 \cr
c_2((i,j),(k,l)) \ &\iff\  c(i,k) \and c(j,l) \cr
c_4((i,j),(k,l)) \ &\iff\  c_2(i,k) \and c_2(j,l). \cr
}$$
\medskip\f
Define a homomorphism $\pi:\N'\to\N$ by
$\forall(x,i)\from \Sigma'\cup N' \cup H' \cup E' \cup K'\
\pi(x,i) = x$.

\medbreak

During the recognition process any partitionable symbol in the pattern $\N_1$
may be partitioned, producing a new network $\N_1'$, with a homomorphism
$\pi:\N_1'\to\N_1$. The parse $p:\N_1\to\N_0$ becomes $p\circ\pi:\N_1'\to\N_0$
and the embedding token $u$ becomes $u \circ \pi$.
The new pair of inclusion functions is $(i\circ\pi,j\circ\pi)$.

\ignore{
In a network $\N=\network{}$, with an embedding token $u$, if a symbol
$\sigma\from\Sigma$ is partitionable then the operation of \i{partitioning
$\sigma$} produces a network $\N'=\network{'}$ and an embedding token $u'$
defined as follows.

$\Sigma' = (\Sigma_1\setminus\{\sigma\}) \cup \set{(\sigma,1),(\sigma,2)}$, 

$N' = (N \setminus N^*) \ \cup\ \comp{(n,1),(n,2)}{n \in N^*}$, 
where $N^* = P\preo\sigma$

$H' = (N \setminus H^*) \ \cup\ \comp{(h,1),(h,2)}{h \in H^*}$, 
where $H^* = A\pre{N^*}$.

$E' = (E \setminus E^*)
\ \cup\ \comp{(e,1),(e,2)}{e \in E^*}$,
where $E^* = F\pre{H^*} \cup S\pre{H^*}$

$K' = (K \setminus K^*)
\ \cup\ \comp{(k,1),(k,2)}{k \in K^*}$,
where $K^* = C\pre{E^*}$

Define $W':N'\cup\Sigma'\to\Sigma'$ by
$$\eqalign{
\forall n\from N\ W_1'(n) &= \cases{
(\sigma,1) & if $n \in N_1$ \cr
(\sigma,2) & if $n \in N_2$ \cr
\sigma & if $n \notin W\preo\sigma$
} \cr
\forall \sigma\from\Sigma'\ W'(\sigma) &= \sigma
}$$

Define $P':N'\to\Sigma'$ by

Again.

Define an index-generating function $I:\Sigma\cup N\cup E \to 
{\Cal P}({\Bbb N})$ by
$$\eqalign{
\forall \sigma^* \from \Sigma\ I(\sigma^*) &= \cases{
\set{1,2} & if $\sigma^*=\sigma$ \cr
\set{0} & if $\sigma^*\ne\sigma$
} \cr
\forall n\from N\ I(n) &= \cases{
\set{1,2} & if $n\in N^*$, where $N^* = P\preo\sigma$ \cr
\set{1} & if $n\in N_1$ \cr
\set{2} & if $n\in N_2$ \cr
\set{0} & otherwise
} \cr
\forall e\from E\ I(e) &= \cases{
\set{1,2} & if $e\in E^*$, where $E^* = F\pre{H^*} \cup S\pre{H^*}$ \cr
\set{0} & if $e \notin E^*$
}
}$$
Then define
$$\eqalign{
\Sigma' &= \comp{(\sigma^*,i)}{\sigma^* \in \Sigma \and i \in
I(\sigma^*)} \cr
N' &= \comp{(n,i)}{n \in N \and i \in I(n)} \cr
H' &= \comp{(h,i)}{h \in H \and i \in I(A(h))} \cr
E' &= \comp{(e,i,j)}{e \in E \and i \in I(A(F(e))) \and j \in I(A(S(e)))} \cr
K' &= \comp{(k,i,j)}{k \in K \and (C(k),i,j) \in E'}
}$$
Define $W':N'\cup\Sigma'\to\Sigma'$ by 
$$ \forall (n,i)\from N'\cup\Sigma'\ W'(n,i) = (W(n),i). $$
Define $P':N'\to\Sigma'$ by *** WRONG
$$ \forall (n,i)\from\Sigma'\ P'(n,i) = (P(n),i). $$
Define $A':H'\to N'\cup\Sigma'$ by
$$ \forall (h,i)\from H'\ A'(h,i) = (A(h),i). $$ 
Define $F':E'\to H'$ by
$$ \forall (e,i,j)\from E'\ F'(e,i,j) = (F(e),i). $$ 
Define $S':E'\to H'$ by
$$ \forall (e,i,j)\from E'\ S'(e,i,j) = (S(e),j). $$ 
Define $C':K'\to E'$ by
$$ \forall (k,i)\from K'\ C'(k,i) = (C(k),i). $$ 

DON'T FORGET G!

Define the new embedding token $u':N'\cup\Sigma'\to\G$ by 
$$\eqalign{
\forall (n,i) \from N'\ u'(n,i) &= u(n) \cr
\forall (\sigma,i) \from \Sigma'\ u'(\sigma,i) &= u(\sigma).
}$$

ignore}

\theorem 46. If $\N=\network{}$ is an unpartitionable network satisfying the
condition $W \circ A \circ F = W \circ A \circ S$ then
$E \doublearrow{A \circ F}{A \circ S}
N\cup\Sigma \buildrel W \over \rightarrow \Sigma$ is a coequaliser
diagram in the category of sets.

\proof Consider any set $X$ and function $\alpha:N\cup\Sigma\to X$ such that
$\alpha \circ A \circ F = \alpha \circ A \circ S$. We must show that
there exists a unique function $\mu:\Sigma\to X$ such that $\alpha = 
\mu \circ W$.

Define $\mu = \alpha|_\Sigma$. 
Consider any symbol $\sigma\from\Sigma$. 

Define $T_1 = \comp{x\from
W\preo\sigma}{\alpha(x)=\alpha(\sigma)}$ and $T_2 = \comp{x\from
W\preo\sigma}{\alpha(x)\ne\alpha(\sigma)}$. Then $T_1 \cup T_2 = 
W\preo\sigma$ and $T_1 \cap T_2 = \emptyset$.
Note also that $\sigma \in T_1$, so $T_1 \ne \emptyset$.

Since $W \circ A \circ F = W \circ A \circ S$ and
$\alpha \circ A \circ F = \alpha \circ A \circ S$ we have, for any
$e\from E$,
$$\eqalign{
e \in F\pre{A\pre{T_1}} \ &\iff\ A(F(e)) \in T_1 
\ \iff\ W(A(F(e))) = \sigma \and \alpha(A(F(e))) = \alpha(\sigma)
\cr
\ &\iff\ W(A(S(e))) = \sigma \and \alpha(A(S(e))) = \alpha(\sigma)
\ \iff\ A(S(e)) \in T_1
\cr
\ &\iff\ e \in S\pre{A\pre{T_1}}  
}$$
so $F\pre{A\pre{T_1}} = S\pre{A\pre{T_1}}$, and similarly
$F\pre{A\pre{T_2}} = S\pre{A\pre{T_2}}$.
Then
$$\eqalign{
F\pre{A\pre{T_1}} \cap S\pre{A\pre{T_2}}
&= F\pre{A\pre{T_1}} \cap F\pre{A\pre{T_2}}
= F\pre{A\pre{T_1 \cap T_2}}
\cr&
= F\pre{A\pre{\emptyset}}
= \emptyset 
}$$
and similarly $S\pre{A\pre{T_1}} \cap F\pre{A\pre{T_2}} = \emptyset$.

So all the conditions for $\sigma$ to be partitionable have been verified,
except $T_2 \ne \emptyset$. But $\sigma$ is not partitionable, by hypothesis,
so $T_2 = \emptyset$. This means that
$\forall n\from W\preo\sigma\ \alpha(n)=\alpha(\sigma) = \mu(W(n))$.

Since we have shown this for arbitrary $\sigma\from\Sigma$ we have
$\forall n\from N \cup \Sigma\ \alpha(n) = \mu(W(n))$, i.e.,
$\alpha = \mu \circ W$, as required.

Conversely, consider any function $\mu:\Sigma\to X$ such that 
$\alpha = \mu \circ W$. Then $\forall\sigma\from\Sigma\ \alpha(\sigma) =
\mu(W(\sigma)) = \mu(\sigma)$, so $\mu = \alpha|_{\Sigma}$. This shows
that $\mu$ is unique. 

This completes the verification of the coequaliser condition. \qed

\subhead{8.8 The outcome of the recognition process}
The recognition process must ensure that, at the end, the pattern $\N_1$,
the homomorphism $p:\N_1\to\N_0$, the inclusion functions $i,j$, and the
embedding token $u$ satisfy the conditions

\blob $\forall x\from \Sigma_1 \cup N_1 \cup E_1 \ i(x) \in \{0, 1\}$,

\blob $\N_1$ is unprunable, given $(i,j)$,

\blob $(\N_1,p,u)$ is inextendable, given $i,j,v,B$,

\blob $\N_1$ is unpartitionable,

\blob $W_1 \circ A_1 \circ F_1 = W_1 \circ A_1 \circ S_1$,

\blob $\forall\sigma\from\Sigma_1\setdiff P_1(N_1)\ B(\sigma) = \theta$.

\medskip\f
It will be shown in \S9.6 that these conditions imply that $\forall
x\from\Sigma_1\cup N_1\cup E_1\ i(x) = 1$ and $\N_1$ is definite; hence the
recognition process is finished.

\vfill\supereject
\runninghead{9. The whole recognition process}

\head{9. The Whole Recognition Process}

\subhead{9.1 Introduction}
This section completes the account of recognition by filling in some missing
details: the line operations, the determination of
temperature, the determination of the bareness function, and the halting
condition.

At the end of recognition the pattern should be definite and all the symbols',
nodes' and edges' inclusion values should be $1$. Previous sections have stated
various sufficient conditions for this to be the case. Now I shall show that
(under some mild assumptions) these conditions are indeed satisfied at the end
of recognition, and that the definite match function $DM$ is maximised.

\subhead{9.2 Line operations}
I shall assume the grammar contains a symbol type
called \i{line}; symbol tokens of this type are called lines. Geometrically
they are infinitely thin line segments, and their embeddings are always
similarities. Parsing starts with a set of randomly arranged lines, symbols of
other types being built up from there. There is no necessary reason to start
with lines, but it is convenient for a wide range of examples, so I shall
provide some special operations for dealing with lines.

\item{(a)} Create a line. A line symbol token $\sigma$ is created; its
initial embedding $u(\sigma)$ is chosen by a random search aiming to maximise
$\rho_{I,T,sat}(u(\sigma))$. This operation is applied throughout recognition
(though mostly at the start when most of the image is not covered by symbol
tokens).

\item{(b)} Randomise a line. If a line's inclusion value falls too low, and
it is bare (not part of another symbol token), a new random embedding transformation is
chosen for it by the same method as in (a).

\item{(c)} Remove a bare line. If a line is not part of another symbol and
its temperature falls below a threshold, it has a small probability of being
removed. The purpose of this is to tidy up the pattern by removing lines that
have not been incorporated into higher-level symbols.

\item{(d)} Glue two lines together, end to end. If two lines are nearly
collinear, with an end of one line close to an end of the other, as measured by
a fleximap, the two lines are replaced by a single large line. Their bars are
connected together, end to end.

\ignore{

\itemitem{(e)} Split a line. A line is divided into two lines. This occurs if
its template value $\rho_{I',tem(\sigma),sat}(u(\sigma))$ would be improved by
doing so and it is not part of another symbol.

}

\def\spread{\mathrel{\mapstochar\Rightarrow}}
\def\sspread{\mathrel{\Leftarrow\kern-3pt\mapstochar\kern-2pt\Rightarrow}}

\subhead{9.3 How temperature is determined}
Every symbol token, node token, hook token, edge token and facet token has a
temperature. These change continually by the following three processes. (There 
are two parameters controlling the spread of temperature across the network,
$\beta=0.3$ and $\gamma=0.2$. The notation $X \spread
Y$ means the assignment statement $Y \assign \max(X,Y)$, and $X \sspread Y$
means $X \spread Y$ and $Y \spread X$.)

\medskip

\item{1.} Every symbol, node, hook, edge or facet token created by a line
operation or an extension operation is given a high initial temperature.

\medskip

\item{2.} Temperature is spread through the pattern by applying the following
operations periodically.

\blob For every hook $h\from H_1$, do $T_{A_1(h)} \spread T_h$; $\beta T_h \spread
T_{A_1(h)}$.

\blob For every edge $e\from E_1$, do $T_{F_1(e)} \sspread T_e$; $T_{S_1(e)}
\sspread T_e$.

\blob For every node $n\from N_1$, do

\indent\indent $T_{P_1(n)} \spread T_n$; $\gamma T_n \spread T_{W_1(n)}$;

\indent\indent if $n\in\dom(G_1)$ then
$\gamma T_{W_1(n)} \spread T_n$ else $\gamma T_n \spread T_{P_1(n)}$.

\blob For every pair $k,k^*\from K_1$ such that $G_1(k,k^*)$, do $T_k \sspread
T_{k^*}$.

\blob For each $k\from K_1$, do $T_{C_1(k)} \sspread T_k$.

\medskip

\item{3.} Periodically each temperature $T$ declines by the formula
$$ T \assign a + \eta T $$
where the constant $\eta$ is slightly below $1$ and the constant $a$ is small
and positive. In the absence of other temperature changes all temperatures will
converge to $T_{min}=a/(1-\eta)$. The value of $a$ is chosen so as to give a 
desired minimum temperature, $T_{min}$.

\medskip\f
The temperatures perform a simulated annealing function. Wherever the structure
of the pattern changes, temperature is increased, by process~1\ignore{; wherever
the geometry changes, temperature is increased, by process 2}. These increases
in temperatures are spread to neighbouring parts of the pattern, by process~2.
In the absence of changes in the structure the temperature will decline, by
process~3. The general effect of this is that rapidly changing areas of the
pattern will be hot, and areas that have settled down will become cold.

Where the pattern is hot the inclusion values will take mid-range values; this
allows rival grammatical possibilities to co-exist. Where the pattern is cold
the inclusion values tend to be driven towards $0$ or $1$, and this forces a
choice to be made between the rival grammatical possibilities, leading to a
definite pattern.

As recognition finishes, structural and geometric changes cease and the temperature
declines to $T_{min}$ throughout the pattern. All the inclusion values are
likely to approach $0$ or $1$. However, this is not guaranteed; it is possible
to construct a network in which there is no consistent final assignment of $0$
or $1$ inclusion values, except for the trivial solution in which all inclusion
values are $0$ (consider, for example, the case of an edge that is connected to
the same hook at both ends where the hook has no other incident edges).
Nevertheless, in realistic cases the inclusion values do go to $0$ or $1$, and
this will be assumed in what follows.

\subhead{9.4 How the bareness function $B$ is determined}
For each $h\from H_1$, $B(h)$ is initially $0$ and increases by a fixed amount
every time an extension operation is applied that adds edges to $F_1\preo h \cup
S_1\preo h$.

For each $k\from K_1$, $B(k)$ is initially $0$ and increases by a fixed amount
every time an extension operation is applied that adds facets to $\comp{k^*\from
K_1}{G_1(k,k^*)}$.

For each $\sigma\from\Sigma_1$, if $P_0\pre{p(\{\sigma\})} = \emptyset$ then
$B(\sigma)$ is initially set to $\theta$ (where $\theta$ is the constant used in
the $DM$ function), and never changes thereafter. If $P_0\pre{p(\{\sigma\})} \ne
\emptyset$ then $B(\sigma)$ is initially set to a positive value $\theta_0 <
\theta$; $B(\sigma)$ is increased by a fixed amount every time extension
operation (a), (b), (e) or (g) is applied that adds nodes to $P_1\preo\sigma$.
The increment is chosen so that $\theta-\theta_0$ is a multiple of the
increment.

The purpose of all this is to prevent the recognition algorithm from getting stuck
in an infinite loop by trying the same thing over and over again. Suppose a hook
$h$ is bare, and then edges are added to it by the operation of extending from
$h$, then the edges are removed by a pruning operation; and this is repeated
indefinitely. The value of $B(h)$ will increase each time edges are added,
making the algorithm more and more unwilling to remove all the edges and leave
the hook bare. Eventually the algorithm will either keep an edge or remove the
node $A(h)$ altogether; either way, the infinite loop is averted. Likewise, the
monotonic increase in $B(k)$ prevents the algorithm from repeatedly adding and
removing sub-facets to $k$ forever.

The monotonic increase in $B(\sigma)$ prevents the algorithm from making any
further attempts to add nodes above $\sigma$ using extension operations (a),
(b), (e) or (g), once $B(\sigma)$ has increased to $\theta$. It follows that
$B(\sigma)$ can never increase above $\theta$. Throughout recognition we have 
$$ \forall\sigma\from\Sigma_1\ B(\sigma) \le \theta, \text{ with equality if }
P_0\pre{p(\{\sigma\})} = \emptyset. \eqno(1) $$
At the end of recognition all the $B(\sigma)$ values for bare symbol tokens
$\sigma$ should equal $\theta$. This is ensured by the following theorem.

\theorem 47. If

\item{(a)} $\N_1=\network{_1}$ is a definite network satisfying
$W_1 \circ A_1 \circ F_1 = W_1 \circ A_1 \circ S_1$,

\item{(b)} $p:\N_1\to\N_0$ is a homomorphism, where $\N_0=\network{_0}$ is a
semi-definite network,

\item{(c)} $(i,j)$ is a pair of inclusion functions on $\N_1$ satisfying
$\forall x\from \Sigma_1\cup N_1\cup E_1\ i(x) = 1$,

\item{(d)} $u$ is an embedding token for $\N_1$ and $v$ is an embedding type
for $\N_0$,

\item{(e)} $B$ is a bareness function for $\N_1$ satisfying
$\forall\sigma\from\Sigma_1\ B(\sigma) \le \theta, \text{ with equality if }
P_0\pre{p(\{\sigma\})} = \emptyset$,

\item{(f)} $(\N_1,p,u)$ is inextendable, given $i,j,v,B$,

\smallskip\f
then

\smallskip

\item{} $\forall\sigma\from\Sigma_1\setdiff P_1(N_1)\ B(\sigma) = \theta$.

\proof Consider any $\sigma\from\Sigma_1\setdiff P_1(N_1)$. In view of
hypotheses (a) and (c), and the fact that $\sigma\notin P_1(N_1)$, theorem~32 tells
us that $j(\sigma)=1$. Now, if $P_0\pre{p(\{\sigma\})} = \emptyset$ then
$B(\sigma)=\theta$ by hypothesis~(e). Suppose, on the other hand,
$P_0\pre{p(\{\sigma\})} \ne \emptyset$. Then hypothesis~(e) gives
$B(\sigma)\le\theta$. Suppose that $B(\sigma) < \theta$. Then, since
$j(\sigma)=1$, extension operation~(e) is possible, giving an extension
$(\N_1',p',u')$ of $(\N_1,p,u)$ such that $p'({P_1'}\pre{\{\sigma\}}) =
P_0\pre{p(\{\sigma\})}$. However hypothesis~(f) tells us that this is a
trivial extension, so 
$(\N_1',p',u')=(\N_1,p,u)$. This means $p(P_1\pre{\{\sigma\}}) =
P_0\pre{p(\{\sigma\})}$. But this is impossible: the left-hand side is empty,
since $\sigma\notin P_1(N_1)$, but the right-hand side is non-empty. This
contradiction establishes that $B(\sigma)=\theta$, as required. \qed

\subhead{9.5 Summary of the entire recognition process}
The input to the parser is an image $I$, a semi-definite network $\N_0$
(representing a grammar), and an embedding type $v$ for $\N_0$. During 
recognition, a network $\N_1$ (representing a pattern), a homomorphism $p:\N_1\to\N_0$, a
pair of inclusion functions $(i,j)$, an embedding token $u$, and a bareness
function $B$ for $\N_1$ are constructed.

The recognition process is a sequence of steps, called \i{cycles}. In each
cycle,

\blob $i$ and $j$ are recalculated (\S7.4);

\blob $u$ is adjusted (subject to the symmetry condition) to increase
$IM(I, \N_1, u, v\circ p, i, j, B)$ (\S6.5);

\blob all temperatures spread and decline a little (\S9.3);

\blob structural operations are applied to $\N_1$ if the conditions are
satisfied (elementary pruning
operations, extension operations, merging two symbol tokens, and partitioning
a symbol token into two); every new symbol, node, hook, edge or facet is given
a high temperature (\S9.3), and some bareness values are increased
after an extension operation (\S9.4);

\blob line operations are applied to $\N_1$ (\S9.2).

\medskip\f
The algorithm halts when

\blob no further structural operations are possible (except for trivial
extensions);

\blob the temperatures have declined very close to the minimum $T_{min}$.

\subhead{9.6 The outcome of recognition}
At the end of recognition, condition (1) will hold (since it holds throughout
recognition); also, the pattern $\N_1=\network{_1}$ and the inclusion functions
$i,j$ are likely to satisfy the condition
$$ \forall x\from \Sigma_1 \cup N_1 \cup E_1 \ i(x) \in \{0, 1\}. \eqno(2) $$
This is likely because the lowering of temperature at the end of recognition pushes
all inclusion values to $0$ or $1$.

Also, the condition
$$ W_1 \circ A_1 \circ F_1 = W_1 \circ A_1 \circ S_1. \eqno(3) $$
is likely to hold. This is because the term
$E_{in(p(W_1(A_1(F_1(e)))))}(u(W_1(A_1(S_1(e))))\inv \cdot u(W_1(A_1(F_1(e)))))$
in $IM(I, \N_1, u, v\circ p, i, j, B)$ penalises any edge $e\from E_1$ for which
$W_1(A_1(F_1(e))) \ne W_1(A_1(S_1(e)))$. The penalty is large and increases in
effect as temperature falls. This term generates a force that pulls the two
symbols $W_1(A_1(F_1(e)))$ and $W_1(A_1(S_1(e)))$ closer together; eventually,
either they will merge or $i(e)$ will fall so low that $e$ is pruned.

Conditions (2) and (3) are not guaranteed to hold, but they can be expected to
hold in practice. Assuming they do hold we can apply the following theorem.

\theorem 48. If

\item{(a)} $\N_1=\network{_1}$ is a network satisfying
$W_1 \circ A_1 \circ F_1 = W_1 \circ A_1 \circ S_1$,

\item{(b)} $p:\N_1\to\N_0$ is a homomorphism, where $\N_0=\network{_0}$ is a
semi-definite network,

\item{(c)} $(i,j)$ is a pair of inclusion functions on $\N_1$ satisfying
$\forall x\from \Sigma_1 \cup N_1 \cup E_1 \ i(x) \in \{0, 1\}$,

\item{(d)} $u$ is an embedding token for $\N_1$ and $v$ is an embedding type
for $\N_0$,

\item{(e)} $B$ is a bareness function for $\N_1$ satisfying
$\forall\sigma\from\Sigma_1\ B(\sigma) \le \theta, \text{ with equality if }
P_0\pre{p(\{\sigma\})} = \emptyset$,

\item{(f)} $\N_1$ is unprunable, given $(i,j)$,

\item{(g)} $(\N_1,p,u)$ is inextendable, given $i,j,v,B$,

\item{(h)} $\N_1$ is unpartitionable,

\smallskip\f
then

\smallskip

\item{(1)} $\N_1$ is definite,

\item{(2)} $\forall x\from \Sigma_1\cup N_1\cup E_1\ i(x) = 1$,

\item{(3)} $IM(I,\N,u,v,i,j,B) = DM(I,\N,u,v)$.

\proof Theorem~46, using hypotheses~(a,h), tells us that

\item{(i)} $E_1 \doublearrow{A_1 \circ F_1}{A_1 \circ S_1}
N_1\cup\Sigma_1 \buildrel W_1 \over \rightarrow \Sigma_1$ is a coequaliser
diagram in the category of sets. 

\smallskip\f
Theorem~42, using hypotheses~(c,f), gives 

\item{(j)} $\forall e\from E_1\ i(e)=1$. 

\smallskip\f
So theorem~45, using hypotheses~(a,c,g) and (j), gives

\item{(k)}
$\forall h\from H_1\ j(h)=0$ and $\forall k\from K_1\setdiff\dom(G_1)\ j(k)=0$.

\smallskip\f
Then theorem~44, using hypotheses~(c,f) and (i,k), gives conclusions~(1,2).

\smallskip\f
Theorem~47, using hypotheses~(a,e,g) and (1,2), then gives

\item{(l)} $\forall\sigma\from\Sigma_1\setdiff P_1(N_1)\ B(\sigma) = \theta$.

\smallskip\f
Conclusion~(3) then follows by theorem~33, using (l) and (1,2). \qed

\medskip\f
As explained in \S6.6 and \S7.5, the algorithm has attempted throughout to
choose $i,j$ to maximise $E$ and to choose $u$ to maximise $IM(I,\N_1,u,v\circ
p,i,j,B)$; as recognition ends this amounts to choosing $i,j,u$ to maximise
$IM(I,\N_1,u,v\circ p,i,j,B)$, and this amounts to
maximising $DM(I,\N_1,u,v\circ p)$ at the end of recognition. Thus the recognition
problem is solved.

It should be noted that there is a number of ways in which recognition can fail.
The core of the theory is provably correct, but the more peripheral parts of
the algorithm are supported only by heuristic arguments (which I have
indicated throughout by use of the word \ic{likely}).

\item{(i)} The algorithm for determining the inclusion functions (\S7.4) is not
guaranteed to halt. It finds only a local maximum of $E$, not a global
maximum.

\item{(ii)} Even for low temperature, maximising $E$ is not precisely the
same as maximising $IM(I, \N_1, \allowbreak u, \allowbreak v\circ p, 
\allowbreak i, \allowbreak j, B)$.

\item{(iii)} The monotonic raising of the bareness function may cut off possible
structural extensions prematurely.

\item{(iv)} Symbol tokens may be merged or not merged, or partitioned or not
partitioned, wrongly. (Errors in merging can be corrected by partitioning and
vice versa.)

\item{(v)} The whole algorithm is not guaranteed to halt.

\item{(vi)} It is not guaranteed that very low temperature will force all
inclusion values to $0$ or $1$.

\item{(vii)} Incoherent edges may survive to the end.

\item{(viii)} Some portions of the image may have been overlooked. 

\medbreak\f
In practice it is only (iii), (iv), (v) and (viii) that matter.

\vfill\supereject

\def\ee #1 - #2\par{\smallbreak\f #1 -- #2\par}
\def\eee #1 - #2 - #3\par{\smallbreak\f #1 -- #2 -- #3\par}

\runninghead{Summary of notation and terminology}

\head{Summary of Notation and Terminology}

\subhead{Logical notation used}

\ee $\wedge$, $\vee$, $\Rightarrow$, $\iff$, $\neg$, $\forall$, $\exists$ -
\ic{and}, \ic{or}, \ic{implies}, \ic{iff}, \ic{not}, \ic{for all} and \ic{there
exists} (note that $\forall$, $\exists$ and $\NOT$ have highest precedence, followed by $\and$
and $\OR$, followed by $\Rightarrow$ and $\iff$)

\subhead{Concepts from category theory presupposed}

\ee the category of sets - its objects are sets and its morphisms are functions

\ee sum, pullback, coequaliser - limits and colimits in the category of sets

\subhead{\S2. Functions and Relations}

\ee function - \S2.2

\eee $\dom(f)$, $\ran(f)$ - the domain and range of function $f$ - \S2.2

\eee $f(A)$, $f\inv(B)$ - the image and preimage of a set under a function -
\S2.2

\eee $f|_A$ - the restriction of a function $f$ to a set $A$ - \S2.2

\eee $f \circ g$ - the composition of functions $f$ and $g$ - \S2.2

\ee (binary) relation - \S2.2

\eee $\dom(R)$, $\ran(R)$ - the domain and range of a relation $R$ - \S2.2

\eee $id_A$ - the identity relation on a set $A$ - \S2.2

\eee $\bot$ - the empty relation - \S2.2

\eee $R \subseteq S$ - $R$ is a sub-relation of $S$ (the same symbol is used 
for the subset relation) - \S2.2

\eee $R \subset S$ - $R$ is a proper sub-relation of $S$ (the same symbol is 
used for the proper subset relation) - \S2.2

\eee $R \cap S$, $R \cup S$, $R \setdiff S$ - the intersection, union and
difference of two relations (or sets) - \S2.2

\eee $R \circ S$ - the composition of two relations - \S2.2

\eee $R\inv$ - the inverse of a relation $R$ - \S2.2

\eee $\overline f$ - the graph of a function $f$ - \S2.2

\eee finite relation - a relation satisfied by finitely many pairs - \S2.3

\eee $NE$ - a relation such that $NE(x,y) \iff x \ne y$ - \S2.3

\ee acyclic relation - \S2.3

\ee connected relation relative to a function - \S2.3

\ee minimal relation relative to a function - \S2.4

\subhead{\S3. Networks and Homomorphisms}

\ee network (symbols, nodes, hooks, edges, facets, gluing relation,
subsymbol, subnode, subhook, subedge, subfacet, supersymbol, supernode,
superhook, superedge, superfacet) - \S3.2

\ee homomorphism (from a network to another) - \S3.2

\eee $f\inv$ - inverse homomorphism of $f$ - \S3.2

\eee isomorphism - an invertible homomorphism - \S3.2

\eee automorphism - an isomorphism from a network to itself - \S3.2

\ee minimal relation relative to a network - \S3.3

\eee semi-definite network - the grammar is a semi-definite network - \S3.4

\eee definite network - the pattern is definite at the end of recognition - \S3.4

\ee subnetwork (and proper subnetwork) - \S3.7

\ee the inclusion homomorphism (from a subnetwork to the whole network) - \S3.7

\eee $p|_{\N'}$ - the restriction of a homomorphism $p$ to a subnetwork $\N'$ - \S3.7

\subhead{\S4. Embeddings and the Definite Match Function}

\eee $\G$ - the group of all affine transformations on the plane - (2004, \S3)

\eee $g \cdot g'$ - the composition of two affine transformations - (2004,
\S3)

\eee $E_\tau$ - the \ic{energy} or penalty function for a fleximap $\tau$ - 
(2004, \S5.3)

\eee $u$ - an embedding token - \S4.2

\eee $u_1 \cdot u_2$ - the product of two embedding tokens - \S4.2

\eee $u \circ f$ - the embedding token induced by a homomorphism $f$ from
an embedding token $u$ - \S4.2

\eee $v$ - an embedding type - \S4.2

\ee the symmetry condition for a network, an embedding token, and an embedding 
type - \S4.2

\eee $v \cdot u$ - an embedding token defined by an embedding type $v$ and
an embedding token $u$ - \S4.2

\eee $v \circ f$ - the embedding type induced by a homomorphism $f$ from an
embedding type $v$ - \S4.2

\eee $u|_{\N'}$ - the restriction of an embedding token $u$ to a subnetwork $\N'$ -
\S4.2

\eee $v|_{\N'}$ - the restriction of an embedding type $v$ to a subnetwork $\N'$ -
\S4.2

\eee $(a,s)$ - a symmetry of a network $\N$ with respect to $v$ - \S4.3

\eee $\pi$ - a local symmetry of a network $\N_1$ with respect $\N_0,p,v$ -
\S4.3

\ee the application of a local symmetry to $p,u$ - \S4.3

\eee $T$ - a template - (2004, \S4)

\eee $I$ - an image, $I:\R^2\to\R$ - (2004, \S4)

\eee $sat(x)$ - (definite) saturation at a point $x$ (used in $\rho_{I,T,sat}$) - \S4.4

\eee $w$ - the weighting function (used in $\rho_{I,T,sat}$) - \S4.4

\eee $\rho_{I,T,sat}$ - the correlation function for an image $I$ and a template
$T$ - \S4.4

\eee $k$ - a constant in the definition of $\rho_{I,T,sat}$ - \S4.4

\eee $DM$ - the definite match function - \S4.5

\eee $\theta$ - the penalty for a bare symbol (a positive real constant)
- \S4.5

\ee the recognition problem (final statement) - \S4.7

\subhead{\S5. Inclusion Functions}

\eee $i$ and $j$ - inclusion functions - \S5.2

\subhead{\S6. The Indefinite Match Functions}

\eee $sat(x)$ - (indefinite) saturation at a point $x$ - \S6.2 

\eee $IM$ - the indefinite match function - \S6.3

\eee $B$ - the bareness function - \S6.3

\subhead{\S7. How the Inclusion Functions are Determined}

\eee $\bold i$ - the inclusion vector, with typical component $\bold i_x$
(for $x\from X$) - \S7.2

\eee $X$ - the index set for the components of $\bold i$ - \S7.2

\eee $Y$ - the index set for the constraints on $\bold i$ - \S7.2

\eee $\bold c^y$ - one constraint vector (for one $y\from Y$), with typical
component $\bold c^y_x$ (for $x\from X$) - \S7.2

\eee $\bold m$ - the vector of coefficients in $IM$, with typical component
$\bold m_x$ (for $x\from X$) - \S7.2

\eee $T_x$ - the temperature of $x$ (for $x\from X$) - \S7.3

\eee $E$ - an expression that is maximised to determine $\bold i$ - \S7.3

\eee $T_{min}$ - the minimum allowed temperature - \S7.3

\subhead{\S8. The Extension Operations}

\eee pruning operation (and trivial pruning operation) - transforming a network
into a subnetwork, given a pair of inclusion functions - \S8.2

\ee the restriction of $(i,j)$ to a subnetwork, $\N'$ - \S8.2

\eee elementary pruning operation - pruning a symbol, a node or an edge - \S8.2

\eee unprunable network - i.e., no non-trivial pruning operation is possible on
it - \S8.3

\ee extension of a triple $(\N_1,p,u)$ - \S8.4

\ee minimal and trivial extensions - \S8.4

\ee the extension conditions - \S8.4

\ee the extension operations - \S8.4

\eee $\theta_0,\theta_1,\theta_2,\theta_3,\theta_4$ - constant thresholds used in the
extension operations - \S8.2

\ee inextendable triple $(\N_1,p,u)$ - \S8.5

\ee merging two symbols - \S8.6

\ee partitioning a symbol token - \S8.7

\ee partitionable and unpartitionable symbols and networks - \S8.7

\subhead{\S9. The Whole Recognition Process}

\ee line operations - \S9.2

\ee the recognition process (full summary) - \S9.5

\ee the outcome of recognition - \S9.6

\vfill\supereject

\bye
