# Supplementary material for: A New Graph Grammar Formalism for Robust Syntactic Pattern Recognition
Source: arXiv:2504.15975 source file (2025-04-24)
Supplement: Supplementary file 2 [file supp1.tex]

\runninghead{1. Introduction}

\head{1. Introduction}

\bigskip\f
The purpose of this project is to develop a new graph grammar formalism for
error-tolerant syntactic pattern recognition.  This paper provides the
mathematical theory in full. It should be read in conjunction with the paper
\i{A New Graph Grammar Formalism for Robust Syntactic Pattern Recognition},
available at https://doi.org/10.48550/arXiv.2504.15975,
which provides a broader account of the context, purpose and application of 
this project, with example grammars and runs.

This paper develops further the mathematical framework in my 2004 technical
report, \i{Mathematical Theory of Recursive Symbol Systems} (Technical Report
GEN-0401, Keele University, Computer Science Department, available at
https://eprints.keele.ac.uk/id/eprint/63/), which I shall cite here simply as
\ic{(2004)}.  Sections 1--5 of (2004) are still valid, but section 6 (Networks
and Homomorphisms) and section 7 (The Recognition Problem) are inadequate and
this report supersedes them.  In particular, I have extended the concept of
network, mainly by the addition of \i{subsymbols}, and developed the
mathematical theory to define the pattern recognition process fully.

The contents of this report are as follows.

Section 2 develops the general theory of functions and relations that will be
needed in the subsequent sections.

Section 3 gives new definitions of \i{network}, \i{homomorphism} and
\i{definite} and \i{semi-definite} networks, superseding those in (2004, \S6).

Section 4 extends the theory of embeddings, introduced in (2004, \S6.4). The
$Match$ function, which was introduced in (2004, \S7.3), is treated more
satisfactorily here as two functions, a \i{definite match function} $DM$ and an
\i{indefinite match function} $IM$ (defined in \S6). 
The subject of symmetries is treated more
thoroughly and several theorems are proved on the affine invariance of the
grammatical framework. The theory of templates (introduced in (2004, \S4)) is
extended here by introducing the concept of \i{saturation}, which expresses the
notion that when several templates overlap in the image plane they interfere
with one another. The recognition problem can now be formally stated.

Section 5 develops the theory of inclusion functions, which were introduced in
(2004, \S7.2).

Section 6 defines the \i{indefinite match function} $IM$, which applies to
networks that are not necessarily definite, with inclusion functions.
The invariance theorems of \S4 are generalised to $IM$. The calculation of the
adjustment of the embeddings by gradient ascent in (2004) is adapted to $IM$.

Section 7 states the mechanism by which the inclusion functions are determined
during recognition.

Section 8 defines the \i{structural operations} by which the pattern grows during
recognition.

Section 9 states the entire recognition algorithm.

The whole theory is built up by a process of stepwise refinement. The first
four sections establish the underlying framework and specify the recognition
problem. Sections~5--9 develop the algorithm for solving it incrementally,
starting with an abstract account of the recognition process and refining it
step by step with each chapter. Stepwise refinement is a valuable method for
managing the complexity of the mathematical theory and the algorithm: it allows
for a separation of concerns, particularly between the structural and geometric
aspects of the theory, and enables the theory to be built up one layer at a
time, with the whole recognition process in view at each stage, at
ever-increasing levels of detail.

At each stage of the theory I shall make explicit the correctness conditions
the recognition algorithm must satisfy to solve the recognition problem,
culminating in theorem~48. The earlier, more fundamental stages (\S\S2--6) are
clean, rigorous and provably correct; the subsequent stages are progressively
messier, with arbitrary parameters and algorithms not guaranteed to converge to
the optimum solution. I distinguish clearly between those properties of the
recognition process that are guaranteed to hold, those that are likely to hold,
and those that one merely hopes will hold.
