# Supplementary material for: A New Graph Grammar Formalism for Robust Syntactic Pattern Recognition
Source: arXiv:2504.15975 source file (2025-04-24)
Supplement: Supplementary file 3 [file supp2.tex]

\runninghead{2. Functions and relations}

\head{2. Functions and Relations}

\subhead{2.1 Introduction}
This section introduces some concepts involving functions and relations that
will be needed in the theory of networks to follow, especially the concept of an
\i{acyclic} relation, a \i{connected} relation relative to a function, and a
\i{minimal} relation relative to a function. Relations will be used in the
following section to express the way in which subsymbols are glued to
supersymbols.

\subhead{2.2 Basic definitions and theorems}
A \i{function} $f:X\to Y$ maps every element of the set $X$ to a unique element
of the set $Y$. $X$ is called the \i{domain} of $f$, $\dom(f)$.

\defn For any function $f:X\to Y$ and any sets $A,B$,
$$ f(A) = \comp{f(x)}{x \in X \cap A}, \qquad
f\pre B = \comp{x \in X}{f(x) \in B}. $$
The \i{range} of $f$, $\ran(f)$, is defined as $f(X)$.

\defn For any function $f:X\to Y$ and any set $A \subseteq X$, the
\i{restriction} of $f$ to $A$, $f|_A:A \to Y$, is defined by
$$ \forall x\from A\ f|_A(x) = f(x). $$

\defn For any functions $f:A\to B$ and $g:C\to D$, the \i{composition} of $f$
and $g$, $f \circ g:C \cap g\pre A \to B$, is defined by
$$ \forall x\from C \cap g\pre A \quad (f\circ g)(x) = f(g(x)). $$

\medskip\f
The term \i{relation} will be understood to mean a binary relation applicable to
all objects: for any relation $R$ and every pair of objects $a,b$, either
$R(a,b)$ holds or it does not.

\defn The \i{domain} $\dom(R)$ and \i{range} $\ran(R)$ of a relation $R$ are
defined by
$$ \dom(R) = \comp{a}{\exists b\ R(b,a)}, \qquad
\ran(R) = \comp{b}{\exists a\ R(b,a)}. $$

\defn A relation $R$ is said to be \i{on} a set $A$ iff $\dom(R) \subseteq A$
and $\ran(R) \subseteq A$.

\defn For any set $A$, the \i{identity} relation $id_A$ is defined by
$$ \forall a,b\quad (id_A(a,b) \ \iff \ a=b\in A). $$

\defn The empty relation $\bot$ is defined by $\forall a,b \ \neg\, \bot(a,b)$.

\defn For any relations $R$ and $S$,
$$\eqalign{
R = S \ &\iff \ \forall a,b\ (R(a,b) \iff S(a,b)) \cr
R \subseteq S \ &\iff \ \forall a,b\ (R(a,b) \Rightarrow S(a,b)) \cr 
R \subset S \ &\iff \ R \subseteq S \and R \ne S.
}$$

\defn For any relations $R$ and $S$, the relations $R \cap S$, $R \cup S$ and
$R\setdiff S$ are defined by
$$\forall a,b\ \ \left\lbrace\eqalign{
(R \cap S)(a,b) &\iff R(a,b) \wedge S(a,b), \cr
(R \cup S)(a,b) &\iff R(a,b) \vee S(a,b), \cr
(R \setdiff S)(a,b) &\iff R(a,b) \wedge \neg S(a,b).
}\right.$$

\defn For any relations $R$ and $S$, the \i{composed} relation $R \circ S$ is
defined by
$$ \forall a,c\ \ 
((R \circ S)(a,c) \ \iff \ \exists b\ (R(a,b) \wedge S(b,c))).
$$
(In all expressions, the composition operator $\circ$ has higher syntactic
precedence than $\cap$, $\cup$ and $\setdiff$.)

\defn For any relation $R$, the \i{inverse} relation $R\inv$ is defined
by
$$ \forall a,b\ \ (R\inv (b,a) \ \iff \ R(a,b)). $$

\defn The \i{graph} of a function $f$ is the relation $\overline f$ defined by
$$ \forall a,b\ \ (\overline f(b,a) \ \iff \ a \in \dom(f) \wedge b=f(a)). $$

\theorem 1. (Obvious properties of relations.) For any relations $R,S,T$,
any functions $f,g$, and any sets $A,X,Y$,

\item{(i)} $\overline{f \circ g} = \overline f \circ \overline g$,
$\dom(\overline f) = \dom(f)$, and $\ran(\overline f) = \ran(f)$

\item{(ii)} if $f:X \to Y$ then $\overline f \circ id_X = \overline f = id_Y
\circ \overline f$,

\item{(iii)} if $f,g:X\to Y$ and $\overline f \subseteq \overline g$ then
$f=g$,

\item{(iv)} $\overline{f|_A} = \overline f \circ id_A$,

\item{(v)} $id_A \circ \overline f = \overline f \circ id_{f\pre A}$,

\item{(vi)} $id_A \circ R \subseteq R$ and $R \circ id_A \subseteq R$, with
equality if $R$ is on $A$,

\item{(vii)} $id_X \circ id_Y = id_{X \cap Y} = id_X \cap id_Y$ and $id_{X \cup
Y} = id_X \cup id_Y$,

\item{(viii)} $\bot \circ R = \bot = R \circ \bot$,

\item{(ix)} $T \subseteq R \cap S$ iff $T \subseteq R$ and $T \subseteq S$
(in particular, $R \cap S \subseteq R$ and $R \cap S \subseteq S$),

\item{(x)} $R \cup S \subseteq T$ iff $R \subseteq T$ and $S \subseteq T$
(in particular, $R \subseteq R \cup S$ and $S \subseteq R \cup S$),

\item{(xi)} $(R \circ S)\inv = S\inv \circ R\inv$, $(R \cap S)\inv = R\inv
\cap S\inv$, $(R \cup S)\inv = R\inv \cup S\inv$,

\item{(xii)} if $R \subseteq S$ then $R\inv \subseteq S\inv$, $R \circ T
\subseteq S \circ T$ and $T \circ R \subseteq T \circ S$,

\item{(xiii)} if $R \subseteq S$ then $\dom(R) \subseteq \dom(S)$ and $\ran(R)
\subseteq \ran(S)$,

\item{(xiv)} if $R \circ S = \bot$ then $\dom(R) \cap \ran(S) = \emptyset$,

\item{(xv)} $\ran(R) = \dom(R\inv)$,

\item{(xvi)} $id_{\dom(R)} \subseteq R\inv \circ R$ and $id_{\ran(R)} \subseteq
R \circ R\inv$,

\item{(xvii)} $\dom(R \circ id_A) = \dom(R) \cap A$ and $\ran(id_A \circ R) = A
\cap \ran(R)$.

\theorem 2. If $f:X\to Y$, and $R$ and $S$ are relations, then

\item{(i)} $\overline f \circ \overline f\inv \subseteq id_Y$,

\item{(ii)} $id_X \subseteq \overline f\inv \circ \overline f$,

\item{(iii)} if $R \subseteq S \circ \overline f$ then $R \circ \overline f\inv
\subseteq S \circ id_Y$,

\item{(iv)} if $\overline f \circ R \subseteq S$ then $id_X \circ R \subseteq
\overline f\inv \circ S$.

\proof (i) For any $y,y'$ such that $(\overline f \circ \overline f\inv)(y,y')$,
we have $y,y' \in Y$ and $\exists x \from X\ (y = f(x) \wedge f(x) = y')$, which
implies that $y=y'$, and hence $id_Y(y,y')$.

(ii) For any $x\from X$, there exists $y$ (namely $f(x)$) such that $f(x) = y$
and $y = f(x)$, and hence $(\overline f\inv \circ \overline f)(x,x)$.

(iii) If $R \subseteq S \circ \overline f$ then $R \circ \overline f\inv
\subseteq S \circ \overline f \circ \overline f\inv \subseteq S \circ id_Y$, by
part (i).

(iv) If $\overline f \circ R \subseteq S$ then $id_X \circ R \subseteq \overline
f\inv \circ \overline f \circ R \subseteq \overline f\inv \circ S$, by part
(ii). \qed

\theorem 3. For any relations $R,S,T$ and any function $f$,

\item{(i)} $(R \cup S) \circ T = R \circ T \ \cup\ S \circ T$,

\item{(ii)} $T \circ (R \cup S) = T \circ R \ \cup\ T \circ S$,

\item{(iii)} $(R \cap S) \circ T \subseteq R \circ T \ \cap\ S \circ T$,

\item{(iv)} $T \circ (R \cap S) \subseteq T \circ R \ \cap\ T \circ S$,

\item{(v)} $(R \cap S) \circ \overline f = R \circ \overline f \ \cap\ S \circ
\overline f$,

\item{(vi)} $\overline f\inv \circ (R \cap S) = \overline f\inv \circ R \ \cap\
\overline f\inv \circ S$.

\proof (i) For any $a,c$,
$$\eqalign{
((R \cup S) \circ T)(a,c)
&\text{ iff } \exists b\ ((R \cup S)(a,b) \wedge T(b,c)) \cr
&\text{ iff } \exists b\ ((R(a,b) \vee S(a,b)) \wedge T(b,c)) \cr
&\text{ iff } \exists b\ (R(a,b) \wedge T(b,c)) \vee
\exists b\ (S(a,b) \wedge T(b,c)) \cr
&\text{ iff } (R \circ T \ \cup\ S \circ T)(a,c).
}$$

(ii) For any $a,c$,
$$\eqalign{
(T \circ (R \cup S))(a,c)
&\text{ iff } \exists b\ (T(a,b) \wedge (R \cup S)(b,c)) \cr
&\text{ iff } \exists b\ (T(a,b) \wedge (R(b,c) \vee S(b,c))) \cr
&\text{ iff } \exists b\ (T(a,b) \wedge R(b,c)) \vee \exists b\ (T(a,b) \wedge
S(b,c)) \cr
&\text{ iff } (T \circ R \ \cup\ T \circ S)(a,c).
}$$

(iii) From $R \cap S \subseteq R$ and $R \cap S \subseteq S$ we infer $(R \cap
S) \circ T \subseteq R \circ T$ and $(R \cap S) \circ T \subseteq S \circ T$,
and hence $(R \cap S) \circ T \subseteq R \circ T \ \cap\ S \circ T$.

(iv) From $R \cap S \subseteq R$ and $R \cap S \subseteq S$ we infer $T \circ (R
\cap S) \subseteq T \circ R$ and $T \circ (R \cap S) \subseteq T \circ S$, and
hence $T \circ (R \cap S) \subseteq T \circ R \ \cap\ T \circ S$.

(v) For any $a,c$,
$$\eqalign{
((R \cap S) \circ \overline f)(a,c)
&\text{ iff } \exists b\ ((R \cap S)(a,b) \wedge c \in \dom(f) \wedge b=f(c)) \cr
&\text{ iff } c \in \dom(f) \wedge (R \cap S)(a,f(c)) \cr
&\text{ iff } c \in \dom(f) \wedge R(a,f(c)) \wedge S(a,f(c)) \cr
&\text{ iff } \exists b\ (R(a,b) \wedge c \in \dom(f) \wedge b=f(c)) \ \wedge\ 
\exists b'\ (S(a,b') \wedge c \in \dom(f) \wedge b'=f(c)) \cr
&\text{ iff } (R \circ \overline f)(a,c) \ \wedge\ (S \circ \overline f)(a,c)
\cr
&\text{ iff } (R \circ \overline f \ \cap\ S \circ \overline f)(a,c).
}$$

(vi) Part (v) gives $(R\inv \cap S\inv) \circ \overline f = R\inv \circ
\overline f \ \cap\ S\inv \circ \overline f$, and taking the inverse gives
$\overline f\inv \circ (R \cap S) = \overline f\inv \circ R \ \cap\ \overline
f\inv \circ S$. \qed

\theorem 4. For any relations $R,S,T$, and any sets $A,B$,

\item{(i)} $R \circ S \ \cap\ T \subseteq (R \ \cap\ T \circ S\inv) \circ S$,

\item{(ii)} $R \circ S \ \cap\ T \subseteq R \circ (S \ \cap\ R\inv \circ T)$,

\item{(iii)} $R \circ id_A \ \cap\ S = (R \cap S) \circ id_A$,

\item{(iv)} $id_A \circ R \ \cap\ S = id_A \circ (R \cap S)$,

\item{(v)} if $id_A \circ R \subseteq S \circ id_B$ then $id_A \circ R
\subseteq R \circ id_B$,

\item{(vi)} if $R \circ id_A \subseteq id_B \circ S$ then $R \circ id_A
\subseteq id_B \circ R$.

\proof (i) For any $x,z$,
$$\eqalign{
(R \circ S \ \cap\ T)(x,z)
&\text{ iff } \exists y\ (R(x,y) \wedge S(y,z) \wedge T(x,z)) \cr
&\text{ implies } \exists y,z'\ (R(x,y) \wedge T(x,z') \wedge S(y,z') \wedge
S(y,z))
\quad\text{by taking $z'=z$} \cr
&\text{ iff } \exists y\ (R(x,y) \wedge (T \circ S\inv)(x,y) \wedge S(y,z)) \cr
&\text{ iff } ((R \ \cap\ T \circ S\inv) \circ S)(x,z).
}$$

(ii) Applying part (i), with $S\inv$ substituted for $R$, $R\inv$ substituted
for $S$, and $T\inv$ substituted for $T$,
$$ S\inv \circ R\inv \ \cap\ T\inv
\subseteq (S\inv \ \cap\ T\inv \circ R) \circ R\inv $$
and then inverting this gives
$$ R \circ S \ \cap\ T \subseteq R \circ (S \ \cap\ R\inv \circ T). $$

(iii) Using part (i), $R \circ id_A \ \cap\ S \subseteq (R \cap S \circ id_A)
\circ id_A \subseteq (R \cap S) \circ id_A$. Conversely, using theorem~3(iii),
$(R \cap S) \circ id_A \subseteq R \circ id_A \ \cap\ S \circ id_A \subseteq R
\circ id_A \ \cap\ S$.

(iv) Applying part (iii) with $R\inv$ substituted for $R$ and $S\inv$
substituted for $S$ gives $R\inv \circ id_A \ \cap\ S\inv = (R\inv \cap S\inv)
\circ id_A$, and inverting this gives $id_A \circ R \ \cap\ S = id_A \circ (R
\cap S)$.

(v) If $id_A \circ R \subseteq S \circ id_B$ then, combining this with $id_A
\circ R \subseteq R$ gives
$$\eqqalign\quad{
id_A \circ R &\subseteq S \circ id_B \ \cap\ R
&\cr
&= (S \cap R) \circ id_B
&\text{by part (iii)}\cr
&\subseteq R \circ id_B
&\text{since $S \cap R \subseteq R$.}\cr
}$$

(vi) If $R \circ id_A \subseteq id_B \circ S$ then, combining this with $R \circ
id_A \subseteq R$ gives
$$\eqqalign\quad{
R \circ id_A &\subseteq id_B \circ S \ \cap\ R
&\cr
&= id_B \circ (S \cap R)
&\text{by part (iv)}\cr
&\subseteq id_B \circ R
&\text{since $S \cap R \subseteq R$.}\cr
}$$
\qed

\theorem 5. For any relation $R$, $R=\overline f$ for some function $f:X\to
Y$ iff $R \circ R\inv \subseteq id_Y$ and $id_X \subseteq R\inv \circ R$.

\proof ($\Rightarrow$) If $R = \overline f$ then $R \circ R\inv \subseteq
id_Y$ and $id_X \subseteq R\inv \circ R$ by theorem~2(i),(ii).

($\Leftarrow$) Suppose $R \circ R\inv \subseteq id_Y$ and $id_X \subseteq R\inv
\circ R$. For any $x\from X$, $id_X(x,x)$ holds, so $(R\inv \circ R)(x,x)$
holds, so there exists $y$ such that $R(y,x)$.

For any $x\from X$ and any $y$, if $R(y,x)$ then $(R\circ R\inv)(y,y)$, so
$id_Y(y,y)$, so $y\from Y$.

For any $x\from X$ and $y,y'\from Y$, if $R(y,x)$ and $R(y',x)$ then $(R\circ
R\inv)(y,y')$, so $id_Y(y,y')$, so $y=y'$.

These facts show that $R = \overline f$ for a function $f:X\to Y$. \qed

\theorem 6. A rectangle of functions $\displaystyle\rectangleA DCBAgfqp$ is a
pullback in the category of sets iff
$$ \overline f \inv \circ \overline g = \overline p \circ \overline q\inv
\quad\text{and}\quad
\overline p\inv \circ \overline p \ \cap\ \overline q\inv \circ \overline q
= id_A. $$

\proof I shall use the standard characterisation of a pullback in the category
of sets, namely $f \circ p = g \circ q$ and $\forall b\from B\ \forall c\from
C\ (f(b)=g(c) \Rightarrow \exists!a\from A\ (p(a)=b \wedge q(a)=c))$.

($\Rightarrow$) Suppose the rectangle is a pullback. I shall verify the two
equations.

$\underline{\overline f \inv \circ \overline g \subseteq \overline p \circ
\overline q\inv}$. For any $b$ and $c$, if $(\overline f \inv \circ \overline
g)(b,c)$ then $b \in B$, $c \in C$ and $\exists d\ (f(b)=d \wedge d=g(c))$, so
$f(b)=g(c)$, so $\exists a\from A\ (b=p(a) \wedge q(a)=c)$ by the pullback
condition, so $(\overline p \circ \overline q\inv)(b,c)$.

$\underline{\overline p \circ \overline q\inv \subseteq \overline f \inv \circ
\overline g}$. For any $b$ and $c$, if $(\overline p \circ \overline
q\inv)(b,c)$ then there exists $a\from A$ such that $b=p(a) \wedge q(a)=c$, so
$f(b)=f(p(a))=g(q(a))=g(c)$, so $(\overline f\inv \circ \overline g)(b,c)$.

$\underline{id_A \subseteq \overline p\inv \circ \overline p \ \cap\ \overline
q\inv \circ \overline q}$. This follows from $id_A \subseteq \overline p\inv
\circ \overline p$ and $id_A \subseteq \overline q\inv \circ \overline q$, which
come from theorem~2(ii).

$\underline{\overline p\inv \circ \overline p \ \cap\ \overline q\inv \circ
\overline q \subseteq id_A}$. For any $a,a'$, if $(\overline p\inv \circ
\overline p \ \cap\ \overline q\inv \circ \overline q)(a,a')$ then $a,a' \in A$
and $\exists b\from B\ (p(a)=b \wedge b=p(a'))$ and $\exists c\from C\ (q(a)=c
\wedge c=q(a'))$, hence $f(b)=f(p(a))=g(q(a))=g(c)$, so by the pullback condition
there exists only one $x\from A$ such that $p(x)=b$ and $q(x)=c$, so $a=a'$, as
required.

($\Leftarrow$) Suppose $\overline f \inv \circ \overline g = \overline p \circ
\overline q\inv$ and $\overline p\inv \circ \overline p \ \cap\ \overline q\inv
\circ \overline q = id_A$. I shall verify the conditions for a pullback.

$\underline{f \circ p = g \circ q}$. For any $a\from A$, $(\overline p \circ
\overline q\inv)(p(a),q(a))$ holds, so by the equation $\overline f \inv \circ
\overline g = \overline p \circ \overline q\inv$ we have $(\overline f \inv
\circ \overline g)(p(a),q(a))$, which means that $f(p(a)) = g(q(a))$, as
required.

$\underline{\forall b\from B\ \forall c\from C\ (f(b)=g(c) \Rightarrow \exists
a\from A\ (p(a)=b \wedge q(a)=c))}$. Consider any $b\from B$ and $c\from C$ such
that $f(b)=g(c)$. Then $(\overline f\inv \circ \overline g)(b,c)$ holds, so by
the equation $\overline f \inv \circ \overline g = \overline p \circ \overline
q\inv$ we have $(\overline p \circ \overline q\inv)(b,c)$, which means that
there exists $a\from A$ such that $b=p(a)$ and $q(a)=c$ as required.

$\underline{\forall b\from B\ \forall c\from C\ (f(b)=g(c) \Rightarrow
\exists^{\le 1} a\from A\ (p(a)=b \wedge q(a)=c))}$. Consider any $b\from B$ and
$c\from C$ such that $f(b)=g(c)$. Suppose there exist $a,a'\from A$ such that
$p(a)=b=p(a')$ and $q(a)=c=q(a')$. Then $(\overline p\inv \circ \overline p \
\cap\ \overline q\inv \circ \overline q)(a,a')$, so by $\overline p\inv \circ
\overline p \ \cap\ \overline q\inv \circ \overline q = id_A$ we have $a=a'$, as
required. \qed

\theorem 7. For any sets $A,B,C$, and any functions $p:A\to C$ and $q:B\to C$,
$A \buildrel p \over \rightarrow C \buildrel q \over \leftarrow B$ is a sum
diagram in the category of sets iff
$$ \overline p \circ \overline p\inv \ \cup\ \overline q \circ \overline q\inv
= id_C, \quad
\overline p\inv \circ \overline p = id_A, \quad
\overline q\inv \circ \overline q = id_B, \quad
\overline p\inv \circ \overline q = \bot, \quad
\overline q\inv \circ \overline p = \bot. $$

\proof ($\Rightarrow$) Assume $A \buildrel p \over \rightarrow C \buildrel q
\over \leftarrow B$ is a sum diagram.

$\underline{\overline p \circ \overline p\inv \ \cup\ \overline q \circ
\overline q\inv = id_C}$. Theorem~2(i) gives $\overline p \circ \overline p\inv
\subseteq id_C$ and $\overline q \circ \overline q\inv \subseteq id_C$; so
$\overline p \circ \overline p\inv \ \cup \ \overline q \circ \overline q\inv
\subseteq id_C$. To show that this inclusion is an equality, choose a set $X$
with more than one element and any functions $f:A \to X$ and $g:B \to X$. Since
$A \buildrel p \over \rightarrow C \buildrel q \over \leftarrow B$ is a sum
diagram, there exists a unique function $i:C \to X$ such that $i\circ p =f$ and
$i\circ q = g$. If $\overline p \circ \overline p\inv \ \cup \ \overline q \circ
\overline q\inv \subset id_C$ then choose $c\from C$ such that $(\overline p
\circ \overline p\inv \ \cup \ \overline q \circ \overline q\inv)(c,c)$ does not
hold. Define $j:C \to X$ as equal to $i$ except at $c$. Then, for all $a\from
A$, $(\overline p\circ \overline p\inv)(p(a),p(a))$ holds, so $p(a) \ne c$, so
$j(p(a))=i(p(a))=f(a)$. Thus $j \circ p = f$. A similar argument shows that $j
\circ q = g$. This contradicts the uniqueness of $i$. The contradiction
establishes that $\overline p \circ \overline p\inv \ \cup \ \overline q \circ
\overline q\inv = id_C$.

$\underline{\overline p\inv \circ \overline p = id_A}$. Theorem 2(ii) gives
$id_A \subseteq \overline p\inv \circ \overline p$. For the converse, choose a
set $X=A$, a function $f:A\to X$ equal to the identity function on $A$, and an
arbitrary function $g:B\to X$ (ignoring the case $A = \emptyset$, for which
$\overline p\inv \circ \overline p = id_A$ is trivially true). Then by the sum
property there exists a unique function $i:C\to X$ such that $i \circ p = f$ and
$i\circ q = g$; thus $i:C \to A$ and $\overline i\circ \overline p = id_A$. Then
$id_A \circ \overline p\inv \subseteq \overline i \circ id_C$ by theorem~2(iii),
so $\overline p\inv \subseteq \overline i$, so $\overline p\inv \circ \overline
p \subseteq \overline i \circ \overline p = id_A$, as required.

$\underline{\overline q\inv \circ \overline q = id_B}$. A similar argument
applies.

$\underline{\overline p\inv \circ \overline q = \bot}$. Choose a set $X$ with
more than one element, and choose $f:A\to X$ and $g:B\to X$ with disjoint
images, so that $\overline f\inv \circ \overline g = \bot$. By the sum property,
there exists a unique function $i:C\to X$ such that $i \circ p = f$ and $i \circ
q = g$. Then
$$ \bot = \overline f\inv \circ \overline g
= (\overline i \circ \overline p)\inv \circ \overline i \circ \overline q
= \overline p\inv \circ \overline i\inv \circ \overline i \circ \overline q
\supseteq \overline p\inv \circ id_C \circ \overline q
= \overline p\inv \circ \overline q $$
so $\bot = \overline p\inv \circ \overline q$, as required.

$\underline{\overline q\inv \circ \overline p = \bot}$. This follows by
inverting $\overline p\inv \circ \overline q = \bot$.

($\Leftarrow$) Assume the five equations; I shall show $A \buildrel p \over
\rightarrow C \buildrel q \over \leftarrow B$ is a sum diagram. Given any set
$X$ and functions $f:A\to X$ and $g:B\to X$, define a relation $R = \overline f
\circ \overline p\inv \ \cup \ \overline g \circ \overline q\inv$. First note
that
$$\eqalign{
R \circ \overline p
&= \overline f \circ \overline p\inv \circ \overline p \ \cup \
\overline g \circ \overline q\inv \circ \overline p
= \overline f \circ id_A \ \cup \ \overline g \circ \bot
= \overline f, \cr
R \circ \overline q
&= \overline f \circ \overline p\inv \circ \overline q \ \cup \
\overline g \circ \overline q\inv \circ \overline q
= \overline f \circ \bot \ \cup \ \overline g \circ id_B
= \overline g.
}$$
Then
$$ R \circ R\inv
= R \circ
(\overline p \circ \overline f\inv \ \cup \ \overline q \circ \overline g\inv)
= R \circ \overline p \circ \overline f\inv \ \cup\ R \circ \overline q \circ
\overline g\inv
= \overline f \circ \overline f\inv \ \cup\
\overline g \circ \overline g\inv
\subseteq id_X $$
by theorem~2(i), and
$$\eqalign{
R\inv \circ R
&= (\overline p \circ \overline f\inv \ \cup \
\overline q \circ \overline g\inv) \circ
(\overline f \circ \overline p\inv \ \cup \
\overline g \circ \overline q\inv)
\supseteq \overline p \circ \overline f\inv \circ \overline f \circ \overline
p\inv \ \cup \
\overline q \circ \overline g\inv \circ \overline g \circ \overline q\inv
\cr&
\supseteq \overline p \circ id_A \circ \overline p\inv \ \cup \
\overline q \circ id_B \circ \overline q\inv
= \overline p \circ \overline p\inv \ \cup \
\overline q \circ \overline q\inv
= id_C
}$$
using theorem~2(ii). By theorem~5, $R=\overline i$, for some function $i:C\to
X$. The equations $R \circ \overline p = \overline f$ and $R \circ \overline q =
\overline g$ then imply $i \circ p = f$ and $i \circ q = g$.

To show the uniqueness of $i$, consider any function $j:C\to X$ satisfying $j
\circ p = f$ and $j \circ q = g$. Then $\overline j \circ \overline p =
\overline f$ and $\overline j \circ \overline q = \overline g$, so by
theorem~2(iii) $\overline f \circ \overline p\inv \subseteq \overline j \circ
id_C = \overline j$ and $\overline g \circ \overline q\inv \subseteq \overline j
\circ id_C = \overline j$, so $\overline i = R = \overline f \circ \overline
p\inv \ \cup\ \overline g \circ \overline q\inv \subseteq \overline j$. Since
$i$ and $j$ are both functions from $C$ to $X$, this is sufficient to imply
$i=j$, as required. \qed

\subhead{2.3 Acyclic and connected relations}

\defn A relation $R$ is \i{finite} iff there are finitely many pairs $(a,b)$
such that $R(a,b)$ holds.

\defn The \ic{not-equal-to} relation $NE$ is defined by $NE(a,b) \iff a \ne b$.

\theorem 8. For any relation $R$,

\item{(i)} $\dom(R \ \cap\ NE \circ R) = \comp{a}{\exists^{>1}b\ R(b,a)}$,

\item{(ii)} $\dom(R \setdiff NE \circ R) = \comp{a}{\exists!b\ R(b,a)}$,

\item{(iii)} $\dom(R \ \cap\ NE \circ R) \ \cap \ \dom(R \setdiff NE \circ R)
= \emptyset$,

\item{(iv)} $\dom(R \ \cap\ NE \circ R) \ \cup \ \dom(R \setdiff NE \circ R)
= \dom(R)$,

\item{(v)} $\ran(R \ \cap\ R \circ NE) = \comp{b}{\exists^{>1}a\ R(b,a)}$,

\item{(vi)} $\ran(R \setdiff R \circ NE) = \comp{b}{\exists!a\ R(b,a)}$,

\item{(vii)} $\ran(R \ \cap\ R \circ NE) \ \cap \ \ran(R \setdiff R \circ NE)
= \emptyset$,

\item{(viii)} $\ran(R \ \cap\ R \circ NE) \ \cup \ \ran(R \setdiff R \circ NE)
= \ran(R)$.

\def\iff{\text{\quad iff\quad }}

\proof (i) For any $a$,
$$\eqalign{
a \in \dom(R \ \cap\ NE \circ R)
&\iff \exists b\ (R \ \cap\ NE \circ R)(b,a)
\iff \exists b\ R(b,a) \ \wedge\ \exists b'\ (b\ne b' \wedge R(b',a))
\cr&
\iff \exists b,b'\ (b\ne b' \wedge R(b,a) \wedge R(b',a))
\iff \exists^{>1}b\ R(b,a).
}$$

(ii) For any $a$,
$$\eqalign{
a \in \dom(R \setdiff NE \circ R)
&\iff \exists b\ (R \setdiff NE \circ R)(b,a)
\iff \exists b\ R(b,a) \ \wedge\ \neg\exists b'\ (b\ne b' \wedge R(b',a))
\cr&
\iff \exists!b\ R(b,a).
}$$

(iii) and (iv) follow from (i) and (ii).

(v)--(viii) follow from (i)--(iv) respectively by substituting $R\inv$ for $R$.
\qed

\theorem 9. For any relations $R,S,T$,
$$ \dom(R \cap T) \ \cap\ \dom(S \setdiff NE \circ T) \subseteq \dom(R \cap S).
$$

\proof For any $a \in \dom(R \cap T) \ \cap\ \dom(S \setdiff NE \circ T)$,
there exists $b$ such that $R(b,a)$ and $T(b,a)$ and there exists $c$ such that
$S(c,a)$ but not $(NE \circ T)(c,a)$. The last of these means that there is no
$d$ not equal to $c$ such that $T(d,a)$; hence $b=c$. Thus we have $R(b,a)$ and
$S(b,a)$, so $a \in \dom(R \cap S)$. \qed

\defn A relation $R$ is \i{acyclic} iff
$$ \NOT\, \exists R^*\ (\bot \ne R^* \subseteq R \, \and\, R^* \subseteq (R^*
\circ NE \, \cap\, NE \circ R^*)). $$

\def\mapleft#1{\,\smash{\mathop{\leftarrow}\limits^{#1}}}
\def\mapright#1{\smash{\mathop{\rightarrow}\limits^{#1}}\,}

\medskip\f
(Informally, $R$ is acyclic iff every non-empty subrelation $R^*$ has an element
of valency 1, i.e., an element related to just one element by $R^*$ or to just
one element by ${R^*}\!\inv$. This is equivalent to the non-existence of a
finite cyclic sequence $x_1,\ldots x_n,x_1$, with $n$ even and $n>2$, where the terms
are all different and and related by $x_1 \mapright R x_2 \mapleft R x_3
\mapright R x_4 \mapleft R x_5 \mapright R \cdots \mapright R x_n \mapleft R
x_1$. However, we shall not need this
characterisation in the theory that follows.)

\theorem 10. If a relation $R$ is acyclic and $R' \subseteq R$ then $R'$ is
also acyclic.

\proof This is immediate from the definition. \qed

\theorem 11.

\item{(i)} If $f:X\to Y$, $R$ is a relation on $X$, and $S$ is a relation on
$Y$, such that
$$ S = \overline f \circ R \circ \overline f\inv, \qquad
\overline f\inv \circ \overline f \ \cap R\inv \circ R \subseteq id_X, \qquad
R \subseteq R \circ NE $$
then $S \subseteq S \circ NE$.

\item{(ii)} If $f:X\to Y$, $R$ is a relation on $X$, and $S$ is a relation on
$Y$, such that
$$ S = \overline f \circ R \circ \overline f\inv, \qquad
\overline f\inv \circ \overline f \ \cap R \circ R\inv \subseteq id_X, \qquad
R \subseteq NE \circ R$$
then $S \subseteq NE \circ S$.

\proof (i) Define the universal relations $U_X$ on $X$ and $U_Y$ on $Y$ by
$$ \forall a,b \quad (U_X(a,b) \iff a \in X \wedge b \in X, \quad
U_Y(a,b) \iff a \in Y \wedge b \in Y). $$
Then $U_Y \subseteq id_Y \cup NE$, so
$$\eqalign{
U_X
&= \overline f\inv \circ U_Y \circ \overline f
\subseteq \overline f\inv \circ (id_Y \cup NE) \circ \overline f
= \overline f\inv \circ id_Y \circ \overline f \ \cup\
\overline f\inv \circ NE \circ \overline f
\cr&
= \overline f\inv \circ \overline f \ \cup\
\overline f\inv \circ NE \circ \overline f
}$$
so
$$ U_X \setdiff \overline f\inv \circ \overline f
\subseteq \overline f\inv \circ NE \circ \overline f. \eqno(1)$$
Also, $R\inv \circ R \subseteq U_X$, since $R$ is on $X$, and
$$ \overline f\inv \circ \overline f \ \cap\ R\inv \circ R \ \cap\ NE
\subseteq id_X \cap NE = \bot $$
so
$$\eqqalignno\quad{
R\inv \circ R \ \cap\ NE
&\subseteq U_X\setdiff \overline f\inv \circ \overline f
&\cr
&\subseteq \overline f\inv \circ NE \circ \overline f
&\text{by (1)}\cr
}{(2)}$$
so
$$\eqqalign\quad{
S &= \overline f \circ R \circ \overline f\inv
&\cr
&= \overline f \circ (R \cap R) \circ \overline f\inv
&\cr
&\subseteq \overline f \circ (R \ \cap\ R \circ NE) \circ \overline f\inv
&\text{since $R \subseteq R \circ NE$}\cr
&\subseteq \overline f \circ R \circ (R\inv \circ R \ \cap\ NE) \circ
\overline f\inv
&\text{by theorem 4(ii)}\cr
&\subseteq \overline f \circ R \circ \overline f\inv \circ NE \circ
\overline f \circ \overline f\inv
&\text{by (2)}\cr
&= S \circ NE \circ \overline f \circ \overline f\inv
&\text{since $S = \overline f \circ R \circ \overline f\inv$}\cr
&\subseteq S \circ NE \circ id_Y
&\text{by theorem~2(i)}\cr
&\subseteq S \circ NE
&\cr
}$$
as required.

(ii) Inverting the hypotheses $S = \overline f \circ R \circ \overline f\inv$
and $R \subseteq NE \circ R$ gives $S\inv = \overline f \circ R\inv \circ
\overline f\inv$ and $R\inv \subseteq R\inv \circ NE$. Applying part (i) of the
theorem, with $R\inv$ and $S\inv$ substituted for $R$ and $S$, gives $S\inv
\subseteq S\inv \circ NE$, which can be inverted to $S \subseteq NE \circ S$.
\qed

\theorem 12. If $f:X\to Y$, $R$ is a relation on $X$, and $S$ is a relation
on $Y$, such that
$$ \overline f \circ R \subseteq S \circ \overline f, \qquad
\overline f\inv \circ \overline f \ \cap\ R\inv \circ R \subseteq id_X, \qquad
\overline f\inv \circ \overline f \ \cap\ R \circ R\inv \subseteq id_X $$
then $R$ is acyclic if $S$ is.

\proof Assuming $S$ is acyclic, we shall infer that $R$ is. Consider any
relation $R^*$ such that $\bot \ne R^* \subseteq R$; we must show $R^*
\not\subseteq R^* \circ NE \ \cap\ NE \circ R^*$. Define a relation $S^* =
\overline f \circ R^* \circ \overline f\inv$ on $Y$. Then $S^* \ne \bot$ (choose
any $x,x'$ such that $R^*(x,x')$; then $S^*(f(x),f(x'))$). Also, $\overline f
\circ R^* \subseteq \overline f \circ R \subseteq S \circ \overline f$, so $S^*
= \overline f \circ R^* \circ \overline f\inv \subseteq S \circ id_Y = S$ by
theorem~2(iii). Since $S$ is acyclic we conclude that $S^* \not\subseteq S^*
\circ NE \ \cap\ NE \circ S^*$.

Now, if $R^* \subseteq R^* \circ NE \ \cap\ NE \circ R^*$ then $R^* \subseteq
R^* \circ NE$ and $R^* \subseteq NE \circ R^*$. Also,
$$ \overline f\inv \circ \overline f \ \cap\ {R^*}\inv \circ R^* \subseteq
\overline f\inv \circ \overline f \ \cap\ R\inv \circ R \subseteq id_X $$
and
$$ \overline f\inv \circ \overline f \ \cap\ R^* \circ {R^*}\inv \subseteq
\overline f\inv \circ \overline f \ \cap\ R \circ R\inv \subseteq id_X $$
so, by theorem~11, $S^* \subseteq S^* \circ NE$ and $S^* \subseteq NE \circ
S^*$. This gives $S^* \subseteq S^* \circ NE \ \cap \ NE \circ S^*$, which is
not true.

This contradiction establishes that $R^* \not\subseteq R^* \circ NE \ \cap\ NE
\circ R^*$, as required. \qed

\defn If $f:X\to Y$ and $R$ is a relation on $X$ then $R$ is \i{connected}
relative to $f$ iff, for any set $Z$ and function $g:X\to Z$ such that
$\overline g \circ R \subseteq \overline g$, there exists a function $i:f(X)\to
Z$ such that $i \circ f = g$.

\medskip\f
(Informally, $R$ is connected relative to $f$ iff, for any $x,x'\from X$ such
that $f(x)=f(x')$, there exists a finite sequence $x=x_0,x_1,\ldots x_n=x'$ such
that, for each $i\from\{1,\ldots n\}$, $R(x_{i-1},x_i)$ or $R(x_i,x_{i-1})$
holds.)

\theorem 13. Given sets $N,\Sigma$, a function $P:N\to\Sigma$, and a finite
relation $G$ on $N$ such that

\item{(a)} $G \circ G = \bot$,

\item{(b)} $G$ is acyclic,

\item{(c)} $\overline P \circ G \subseteq \overline P$,

\f
then

\item{(i)} $\forall X \subseteq\Sigma\ |P\pre X| - |G \circ id_{P\pre X}| \ge
0$,

\item{(ii)} for any $X \subseteq\Sigma$, if $|P\pre X| - |G \circ id_{P\pre
X}|=0$ then $P\pre X = \emptyset$,

\item{(iii)} if $\forall X \subseteq\Sigma\ |P\pre X| - |G \circ id_{P\pre X}|
\le |X|$ then $G$ is connected relative to $P$.

\proof The proof is by induction on $|G|$. For the induction basis, suppose
$|G|=0$; then we can verify (i), (ii) and (iii) directly, as follows.

(i) For any $X\subseteq \Sigma$, $|P\pre X| - |G \circ id_{P\pre X}| = |P\pre X|
\ge 0$.

(ii) For any $X\subseteq \Sigma$ such that $|P\pre X| - |G \circ id_{P\pre
X}|=0$, we have $|P\pre X|=0$ and hence $P\pre X=\emptyset$, as required.

(iii) If $\forall X \subseteq\Sigma\ |P\pre X| - |G \circ id_{P\pre X}| \le |X|$
then
$$ \forall\sigma\from\Sigma\quad |P\preo\sigma| \le 1 $$
which means that $P$ is injective. In that case, given any $Z$ and $Q:N\to Z$,
the unique function $i:P(N)\to Z$ such that $i\circ P = Q$ is defined by
$\forall n\from N\ i(P(n)) = Q(n)$.

\medskip

For the induction step, suppose that $|G| > 0$, and define
$$\eqalign{
G' &= G \ \cap\ G \circ NE \ \cap\ NE \circ G \cr
S_1 &= \ran(G\setdiff G\circ NE) \cr
S_2 &= \dom((G \ \cap\ G\circ NE)\setdiff NE \circ G) \cr
S &= S_1 \cup S_2 \cr
N' &= N \setdiff S \cr
P' &= P|_{N'}.
}$$
These have the following properties.

\bigskip

\item{$(\alpha)$} $G' \subset G$.

Proof. This follows since $G$ is acyclic and not equal to $\bot$.

\bigskip

\item{$(\beta)$} $G'$ is a finite relation on $N'$.

Proof. $G'$ is finite since $G' \subset G$ and $G$ is finite. To show that $G'$
is on $N'$,
$$\eqqalign\quad{
\dom(G') \cap S_1
&\subseteq \dom(G) \cap \ran(G) = \emptyset
&\text{since $G \circ G = \bot$}\cr
\dom(G') \cap S_2
&\subseteq \dom(G \cap NE \circ G) \cap \dom(G \setdiff NE \circ G) =
\emptyset
&\text{by theorem~8(iii)} \cr
\ran(G') \cap S_1
&\subseteq \ran(G \cap G \circ NE) \cap \ran(G \setdiff G \circ NE) =
\emptyset
&\text{by theorem~8(vii)} \cr
\ran(G') \cap S_2
&\subseteq \ran(G) \cap \dom(G) = \emptyset
&\text{since $G \circ G = \bot$} \cr
}$$
thus $\dom(G') \subseteq N\setdiff S = N'$ and $\ran(G') \subseteq N\setdiff S =
N'$, as required.

\bigskip

\item{$(\gamma)$} For every $x \from S$, there exists a unique $y$ such that
$(G\setdiff G')(x,y)$ or $(G\setdiff G')(y,x)$ (these two cases being mutually
exclusive).

Proof. $(G\setdiff G')(x,y)$ and $(G\setdiff G')(y,x)$ are mutually exclusive by
$(G\setdiff G') \circ (G\setdiff G') \subseteq G \circ G = \bot$. We have $G
\setdiff G \circ NE \subseteq G \setdiff G'$, so
$$ S_1 \subseteq \ran(G\setdiff G'), \eqno(1) $$
and
$$ S_1 \, \cap\ \ran\bigl((G\setdiff G') \cap (G\setdiff G')\circ NE\bigr)
\subseteq S_1 \, \cap\ \ran(G \cap G\circ NE)
= \emptyset \eqno(2) $$
by theorem~8(vii), so from (1), (2) and theorem~8(viii)
$$ S_1
\subseteq \ran\bigl((G\setdiff G')\setdiff(G\setdiff G') \circ NE\bigr). $$
Using theorem~8(vi), this can be written as
$$ \forall x\from S_1 \, \exists!y \ (G\setdiff G')(x,y). \eqno(3) $$
Similarly, $(G \cap G \circ NE)\setdiff NE \circ G \subseteq G\setdiff G'$, so
$$ S_2 \subseteq \dom(G\setdiff G'), \eqno(4) $$
and
$$ S_2 \ \cap\ \dom\bigl((G\setdiff G') \cap NE \circ (G\setdiff G')\bigr)
\subseteq \dom(G\setdiff NE \circ G) \ \cap\ \dom(G \cap NE \circ G)
= \emptyset \eqno(5) $$
by theorem~8(iii), so from (4), (5) and theorem~8(iv)
$$ S_2
\subseteq \dom\bigl((G\setdiff G')\setdiff NE \circ (G\setdiff G')\bigr). $$
Using theorem~8(ii) this can be written as
$$ \forall x\from S_2 \, \exists!y\ (G\setdiff G')(y,x). \eqno(6) $$
Consequently, from (3), (6), and $(G\setdiff G') \circ (G\setdiff G') = \bot$,
$$ \forall x\from S\ \exists!y\ ((G\setdiff G')(x,y) \vee
(G\setdiff G')(y,x)) $$
as required.

\bigskip

\item{$(\delta)$} $\forall x,y\ (G(x,y) \Rightarrow x \in N' \vee y \in N')$.

Proof. First,
$$ \ran(G \cap G \circ NE) \ \cap\ S_1 = \ran(G \cap G \circ NE) \ \cap\
\ran(G \setdiff G \circ NE) = \emptyset \eqno(7) $$
by theorem~8(vii). Secondly,
$$ \ran(G \cap G \circ NE) \ \cap\ S_2
= \ran(G \cap G \circ NE) \ \cap\ \dom((G \ \cap\ G\circ NE)\setdiff NE \circ
G)
\subseteq \ran(G) \ \cap\ \dom(G)
= \emptyset. \eqno(8) $$
Combining (7) and (8) gives
$$ \ran(G \cap G \circ NE) \ \cap\ S = \emptyset. \eqno(9) $$
Next,
$$ \dom(G\setdiff G \circ NE) \ \cap\ S_1
= \dom(G\setdiff G \circ NE) \ \cap\ \ran(G\setdiff G\circ NE)
\subseteq \dom(G) \ \cap\ \ran(G)
= \emptyset. \eqno(10)$$
Also, applying theorem~9, with $R = G\setdiff G \circ NE$, $S = G \cap G \circ
NE$, and $T = G$, gives
$$ \dom(G\setdiff G \circ NE) \ \cap\ \dom((G \cap G \circ NE) \setdiff NE
\circ G)
\subseteq \dom((G\setdiff G \circ NE) \ \cap\ (G \cap G \circ NE)). $$The
right-hand side is $\dom(\bot)$, so this simplifies to
$$ \dom(G\setdiff G \circ NE) \ \cap\ S_2 = \emptyset. \eqno(11) $$
Combining (10) and (11) gives
$$ \dom(G\setdiff G \circ NE) \ \cap\ S = \emptyset. \eqno(12) $$
Finally, given any $x,y$ such that $G(x,y)$ holds, either $(G \circ NE)(x,y)$
holds, in which case $x \notin S$ by (9), or $(G \circ NE)(x,y)$ does not hold,
in which case $y \notin S$ by (12). Thus $x \in N'$ or $y \in N'$.

\bigskip

\item{$(\epsilon)$} For every $x,y$ such that $(G\setdiff G')(x,y)$ holds,
either $x \in S$ or $y \in S$.

Proof. Using the definition $G' = G \ \cap\ G \circ NE \ \cap\ NE \circ G$,
$$ G\setdiff G'
= (G \setdiff G \circ NE) \ \cup\ ((G \cap G \circ NE) \setdiff NE \circ G)
$$
so if $(G\setdiff G')(x,y)$ then $x \in \ran(G \setdiff G \circ NE) = S_1$ or $y
\in \dom((G \cap G \circ NE) \setdiff NE \circ G) = S_2$; thus $x \in S$ or $y
\in S$.

By $(\delta)$, we cannot have both $x \in S$ and $y \in S$.

\bigskip

\item{$(\zeta)$} $\forall x\from S\ \exists y \from N'\ (G(x,y) \vee G(y,x))$.

Proof. Given $x\from S$, the existence of $y$ satisfying $G(x,y) \vee G(y,x)$ is
assured by $(\gamma)$, and it must be in $N'$ because of $(\delta)$.

\bigskip

\item{$(\eta)$} $\forall x,y\from N\ (G(x,y) \Rightarrow P(x)=P(y))$.

Proof. The hypothesis $\overline P \circ G \subseteq \overline P$ means
$$ \forall \sigma,y\ ((\overline P \circ G)(\sigma,y) \Rightarrow \overline
P(\sigma,y)) $$
which may be expanded to
$$ \forall \sigma,y\ (\exists x\ (\sigma=P(x) \wedge G(x,y)) \Rightarrow
\sigma=P(y)) $$
which is logically equivalent to
$$ \forall x,y\from N\ (G(x,y) \Rightarrow P(x)=P(y)) $$
since $\dom(P)=N$ and $G$ is on $N$.

\bigskip

\item{$(\theta)$} $\forall X \subseteq \Sigma\ |(G\setdiff G') \circ
id_{P\pre X}| = |S \cap P\pre X|$.

Proof. By $(\gamma)$ and $(\epsilon)$, there is a bijection $\omega$ between
pairs $(x,y)$ such that $(G\setdiff G')(x,y)$ holds and elements of $S$:
$$ \omega(x,y) = x \text{ or } y \text{, whichever one is in } S. $$
This gives $|G\setdiff G'| = |S|$. Moreover, for any $X \subseteq \Sigma$, and
any $x,y$ satisfying $(G\setdiff G')(x,y)$, $((G\setdiff G') \circ id_{P\pre
X})(x,y)$ iff $y \in P\pre X$ iff $x \in P\pre X$ (this is because $P(x)=P(y)$,
from $(\eta)$), so this in turn is equivalent to $\omega(x,y) \in P\pre X$. Thus
$\omega$ maps the pairs $(x,y)$ satisfying $((G\setdiff G') \circ id_{P\pre
X})(x,y)$ onto $S \cap P\pre X$. The conclusion follows.

\bigskip

\item{$(\iota)$} $G' \circ G' = \bot$.

Proof. This follows since $G' \subset G$ and $G \circ G = \bot$.

\bigskip

\item{$(\kappa)$} $G'$ is acyclic.

Proof. This follows from $G' \subset G$ by theorem~10.

\bigskip

\item{$(\lambda)$} $\overline{P'} \circ G' \subseteq \overline{P'}$.

Proof. We have $G' = G' \circ id_{N'}$, $\overline{P'} = \overline P \circ
id_{N'} \subseteq \overline P$, $G' \subset G$, and $\overline P \circ G
\subseteq \overline P$, so
$$ \overline{P'} \circ G'
= \overline{P'} \circ G' \circ id_{N'}
\subseteq \overline P \circ G \circ id_{N'}
\subseteq \overline P \circ id_{N'}
= \overline{P'}. $$

\bigskip

\item{$(\mu)$} $|G'| < |G|$.

Proof. This follows from $G' \subset G$.

\bigskip

\item{$(\nu)$} $\forall X\subseteq\Sigma\ |P'{}\pre X| - |G' \circ id_{P'{}\pre
X}| = |P\pre X| - |G \circ id_{P\pre X}|$.

Proof. We have $P'{}\pre X = P\pre X \cap N' = P\pre X \setdiff S$ and hence
$$ |P'{}\pre X| = |P\pre X| - |S \cap P\pre X|. $$
Also, $G' \circ id_{P'{}\pre X} = G' \circ id_{N'} \circ id_{P\pre X} = G' \circ
id_{P\pre X}$, since $G'$ is on $N'$, so
$$ |G' \circ id_{P'{}\pre X}|
= |G' \circ id_{P\pre X}|
= |G \circ id_{P\pre X}| - |(G\setdiff G') \circ id_{P\pre X}|
= |G \circ id_{P\pre X}| - |S \cap P\pre X|
$$
by $(\theta)$. Hence
$$ |P'{}\pre X| - |G' \circ id_{P'{}\pre X}|
= |P\pre X| - |G \circ id_{P\pre X}|. $$

\bigskip

\item{$(\xi)$} $P\pre X = \emptyset$ if $P'{}\pre X = \emptyset$.

Proof. I shall prove the contrapositive. If $P\pre X \ne \emptyset$ then there
exists $x \from N$ such that $P(x) \in X$. If $x \in N'$ then $x \in P'{}\pre
X$, whereas if $x \notin N'$ then $x \in S$, so by $(\zeta)$ there exists
$y\from N'$ such that $G(x,y)$ or $G(y,x)$. By $(\eta)$, $P(y)=P(x)\in X$, so $y
\in P'{}\pre X$. In either case, $P'{}\pre X \ne \emptyset$.

\bigskip

\item{$(\omicron)$} $P'(N') = P(N)$.

Proof. Recall that $P' = P|_{N'}$, so $P'(N') = P(N')$. By $(\zeta)$, for every
$x \from S$ there exists $y\from N'$ such that $G(x,y)$ or $G(y,x)$; by
$(\eta)$, this implies $P(x)=P(y)$. This shows that $P(S) \subseteq P(N')$.
Since $N = S \cup N'$, this gives $P(N) = P(S) \cup P(N') = P(N')$. Hence
$P'(N') = P(N)$.

\bigskip

\item{$(\pi)$} $G$ is connected relative to $P$ if $G'$ is connected
relative to $P'$.

Proof. Consider any set $Z$ and any function $Q:N \to Z$ such that $\overline Q
\circ G \subseteq \overline Q$. Define $Q'=Q|_{N'}:N'\to Z$, and note that
$$ \overline{Q'} \circ G'
= \overline{Q'} \circ G' \circ id_{N'}
\subseteq \overline Q \circ G \circ id_{N'}
\subseteq \overline Q \circ id_{N'}
= \overline{Q'}. $$
Assuming $G'$ is connected relative to $P'$, there exists a function
$i:P'(N')\to Z$ such that $i \circ P' = Q'$; this means that $i \circ P$ agrees
with $Q$ on $N'$. By $(\omicron)$, we have $i:P(N)\to Z$. Moreover I claim that
$i \circ P = Q$. For any $x \in S$, by $(\zeta)$ there exists $y\from N'$ such
that $G(x,y)$ or $G(y,x)$. Then $(\eta)$ gives $P(x)=P(y)$, and by similar
reasoning the hypothesis $\overline Q \circ G \subseteq \overline Q$ gives
$Q(x)=Q(y)$. Then
$$ i(P(x)) = i(P(y)) = Q(y) = Q(x). $$
So $i \circ P = Q$ holds on $S$ as well as on $N'$, i.e., it holds on the whole
of $N$. Thus we conclude that $i:P(N)\to Z$ and $i \circ P = Q$, as required.

\bigskip\f
Now we are ready to apply the induction step of the theorem. By $(\beta)$,
$(\iota)$--$(\mu)$, we can apply the inductive hypothesis to $N',P',G'$, and
thereby verify (i), (ii) and (iii) for $N,P,G$:

(i) for any $X \subseteq\Sigma$, applying $(\nu)$, $|P\pre X| - |G \circ
id_{P\pre X}| = |P'{}\pre X| - |G' \circ id_{P'{}\pre X}| \ge 0$ by inductive
hypothesis;

(ii) for any $X \subseteq\Sigma$, if $|P\pre X| - |G \circ id_{P\pre X}|=0$ then
$|P'{}\pre X| - |G' \circ id_{P'{}\pre X}|=0$ by $(\nu)$, so $P'{}\pre X =
\emptyset$ by inductive hypothesis, so $P\pre X = \emptyset$ by $(\xi)$;

(iii) if $\forall X \subseteq\Sigma\ |P\pre X| - |G \circ id_{P\pre X}| \le |X|$
then $\forall X \subseteq\Sigma\ |P'{}\pre X| - |G' \circ id_{P'{}\pre X}| \le
|X|$ by $(\nu)$, so $G'$ is connected relative to $P'$ by inductive hypothesis,
so $G$ is connected relative to $P$ by $(\pi)$.\qed

\subhead{2.4 Minimal relations relative to a function}

\defn If $f:X\to Y$ and $R$ is a relation on $X$ then $R$ is \i{minimal}
relative to $f$ iff
$$ \forall R^*\subseteq R\ \ (\overline f \circ R^* = \overline f \circ R
\Rightarrow R^* = R). $$

\medskip\f
(Informally, $R$ is minimal relative to $f$ iff, for any $x\from X$ and $y\from
Y$, there exists at most one $x'\from X$ such that $f(x')=y$ and $R(x',x)$.)

\theorem 14. If $f:X\to Y$ and $R$ is a relation on $X$ then $R$ is minimal
relative to $f$ iff
$$ \overline f\inv \circ \overline f \ \cap\ R \circ R\inv \subseteq id_X. $$

\proof $(\Rightarrow)$ Suppose $R$ is minimal relative to $f$. For any $x,x'$
such that $(\overline f\inv \circ \overline f \cap R \circ R\inv)(x,x')$, we
have $x,x'\in X$, $f(x)=f(x')$, and there exists $z$ such that $R(x,z)$ and
$R(x',z)$. Now suppose $x \ne x'$. Define a relation $R^*$ equal to $R$ except
that $R^*(x,z)$ does not hold. Thus $R^* \subset R$, but $\overline f \circ R^*
= \overline f \circ R$, since $(\overline f \circ R^*)(f(x),z)$ still holds (via
$x'$) and $\overline f \circ R^*$ is identical to $\overline f \circ R$ in all
other respects. The existence of $R^*$ contradicts the minimality of $R$. This
contradiction demonstrates that $x=x'$, as required.

$(\Leftarrow)$ Suppose $\overline f\inv \circ \overline f \cap R \circ R\inv
\subseteq id_X$. Consider any $R^*\subseteq R$ such that $\overline f \circ R^*
= \overline f \circ R$. Then
$$\eqqalign\quad{
R &= id_X \circ R \ \cap\ R
&\cr
&\subseteq \overline f\inv \circ \overline f \circ R \ \cap\ R
&\text{by theorem~2(ii)} \cr
&= \overline f\inv \circ \overline f \circ R^* \ \cap\ R
&\text{since $\overline f \circ R^* = \overline f \circ R$} \cr
&\subseteq (\overline f\inv \circ \overline f \ \cap\ R \circ {R^*}\inv) \circ
R^*
&\text{by theorem~4(i)} \cr
&\subseteq (\overline f\inv \circ \overline f \ \cap\ R \circ R\inv) \circ R^*
&\text{since $R^* \subseteq R$} \cr
&\subseteq id_X \circ R^*
&\text{since $\overline f\inv \circ \overline f \cap R \circ R\inv \subseteq
id_X$} \cr
&= R^*
&\cr
}$$
so $R^*=R$, as required. \qed
