# Supplementary material for: A New Graph Grammar Formalism for Robust Syntactic Pattern Recognition
Source: arXiv:2504.15975 source file (2025-04-24)
Supplement: Supplementary file 4 [file supp4.tex]

\def\Flex{\hbox{\i{Flex}}}

\runninghead{4. Embeddings and the definite match function}

\head{4. Embeddings and the Definite Match Function}

\subhead{4.1 Introduction}
The account of the recognition problem given in the previous sections has one
very obvious deficiency: it does not say what relation should hold between the
pattern and the image to make the pattern a good interpretation of the image.
Indeed, it does not make any use of the image at all, nor does it involve any
geometry.

In this section this deficiency will be rectified. Each symbol (and node) in the
pattern must be embedded in the image plane using an affine transformation; the
collection of all these affine transformations is called an \i{embedding token}.
The grammar imposes constraints on the embedding token, stipulating that if two
symbols are grammatically related then their embedding transformations must be
geometrically related; the collection of all these constraints is called an
\i{embedding type}. Embedding types make use of the concept of a \i{fleximap},
introduced in (2004, \S5).

The aim of recognition is to construct a definite pattern and embedding token
that \i{match}, or satisfy the constraints of, the image, the grammar and
embedding type. The degree of match is expressed by the \i{definite match
function} $DM$.

This section defines embedding tokens and types (slightly modifying the
definitions in (2004, \S6.4)), and the $DM$ function. It also refines the use 
of templates (introduced in (2004, \S4)), defines a symmetry of the grammar, and
demonstrates the affine invariance of the whole framework.

\subhead{4.2 Embedding tokens and types}
As in (2004), $\G$ is the group of affine transformations on the plane, a
six-dimensional Lie group. The composition or product of two affine 
transformations is written as $g \cdot g'$. Composition of two higher-level 
functions such as homomorphisms, embedding tokens or embedding types will be 
written using the \ic{$\circ$} symbol.

\defn An \i{embedding token} for a network $\network{}$ is a function
$u:\Sigma\cup N\to\G$ such that
$$ \forall n,n^* \from N\ (G(n,n^*) \Rightarrow u(n)=u(n^*)). $$

\medskip\f
The product $u_1 \cdot u_2$ of embedding tokens $u_1$ and $u_2$ is defined as in
(2004, \S6.4): 
$$ \forall x\from\Sigma\cup N\ (u_1 \cdot u_2)(x) = u_1(x)\cdot
u_2(x). $$
It follows immediately that $u_1 \cdot u_2$ is an embedding
token. As before we can also define the induced embedding token $u \circ f$ on
$\N'$, where $u$ is an embedding token on $\N$ and $f:\N'\to\N$ is a
homomorphism. However, we must check that $u \circ f$ satisfies the definition
of an embedding token, as follows.

\theorem 25. If $u$ is an embedding token for $\N$ and $f:\N'\to\N$ is a
homomorphism then $u \circ f$ is an embedding token for $\N'$.

\proof We shall use the notation $\N'=\network{'}$, $\N=\network{}$ and $u'=u
\circ f$. Clearly $u':\Sigma'\cup N' \to \G$. Consider any $n,n^* \from N'$ such
that $G'(n,n^*)$. We have $\overline f \circ G' = G \circ \overline f$, and
hence $G'(n,n^*)$ implies $(\overline f \circ G')(f(n),n^*)$, which implies $(G
\circ \overline f)(f(n),n^*)$, i.e., $G(f(n),f(n^*))$. Since $u$ is an embedding
token for $\N$ this implies $u(f(n))=u(f(n^*))$, i.e., $u'(n)=u'(n^*)$. Thus
$u'$ is an embedding token for $\N'$. \qed

\defn An \i{embedding type} for a network $\network{}$ is a sextuple
$(sub,\allowbreak con,\allowbreak rel,\allowbreak symm,\allowbreak tem,
\allowbreak in)$, in which $sub:\comp{(\sigma,\sigma^*) \from
\Sigma\times\Sigma}{G(\sigma,\sigma^*)} \to \Flex$, $con:N\to\Flex$,
$rel:E\to\Flex$, $symm:\Sigma\to Sub(\G)$, $tem:\Sigma\to Tem$, and
$in:\Sigma\to\Flex$ where $\Flex$ is the set of all fleximaps, $Sub(\G)$ is the
set of all subgroups of $\G$, and $Tem$ is the set of all templates; moreover,
for every $\sigma\in\Sigma$, the fleximap $in(\sigma)$ must have nominal part
equal to the identity transformation.

\medskip\f
This definition of embedding type is just as in (2004, \S6.4), except for the
presence of $sub$. The meaning of $sub$ is that if $\sigma^*$ is a subsymbol of
$\sigma$ then $sub(\sigma,\sigma^*)$ is a fleximap describing the relationship
between the embeddings of $\sigma^*$ and $\sigma$.

Embedding tokens are constrained by a symmetry condition. If $u$ is an embedding
token for $\N$ and $v$ is an embedding type for $\N$, where $\N=\network{}$, the
\i{symmetry condition} for $\N,u,v$ is
$$ \forall n\from N \quad u(P(n))\inv \cdot u(n) \in symm(P(n)). $$
This states that each node $n$ is embedded in the image plane in the same way as
the part $P(n)$, up to a symmetry of $P(n)$.

Given an embedding type $v=(sub_1,con_1,rel_1,symm_1,tem_1,in_1)$ and an
embedding token $u$ for a network $\network{}$, we can define an embedding type
$v \cdot u$ for the same network by $v \cdot u =
(sub_2,con_2,rel_2,symm_1,tem_2,in_2)$, where
$$\eqalign{
\forall \sigma,\sigma^* \from \Sigma \quad (G(\sigma,\sigma^*) \ \Rightarrow\
sub_2(\sigma,\sigma^*)
&= u(\sigma)\inv \cdot sub_1(\sigma,\sigma^*) \cdot u(\sigma^*)) \cr
\forall n\from N \quad con_2(n) &= u(W(n))\inv \cdot con_1(n) \cdot u(n) \cr
\forall e\from E \quad rel_2(e) &= u(A(S(e)))\inv \cdot rel_1(e) \cdot
u(A(F(e))) \cr
\forall \sigma\from\Sigma \quad tem_2(\sigma) &= tem_1(\sigma) \circ u(\sigma)
\cr
\forall \sigma\from\Sigma \quad
in_2(\sigma) &= u(\sigma)\inv \cdot in_1(\sigma) \cdot u(\sigma)
}$$

Given an embedding type $v=(sub,con,rel,symm,tem,in)$ for a network $\N$ and a
homomorphism $f:\N'\to\N$, there is an induced embedding type $v \circ f$ for
$\N'$ defined by
$$ v \circ f
= (sub',con \circ f,rel \circ f,symm \circ f,tem \circ f,in \circ f). $$
where
$$ \forall \sigma,\sigma^*\from\Sigma \quad (G(\sigma,\sigma^*) \ \Rightarrow\
sub'(\sigma,\sigma^*) = sub(f(\sigma),f(\sigma^*))). $$

\theorem 26. (Lemma~1 of (2004, \S6.4)) If $f:\N'\to\N$ is a
homomorphism, $v$ is an embedding type for $\N$, and $u$ is an embedding token
for $\N$, then
$$ (v \cdot u) \circ f = (v \circ f) \cdot (u \circ f). $$

\proof The proof is a slightly adapted version of the one in (2004, \S6.4).
Let $\N'=\network{'}$, $\N=\network{}$ and $v = (sub_1,\allowbreak con_1,
\allowbreak rel_1, \allowbreak symm_1, \allowbreak tem_1, \allowbreak in_1)$.
Then $v \cdot u = (sub_2, con_2, rel_2, symm_1, tem_2, in_2)$, where
$$\eqalign{
\forall \sigma,\sigma^* \from \Sigma \quad (G(\sigma,\sigma^*) \ \Rightarrow\
sub_2(\sigma,\sigma^*)
&= u(\sigma)\inv \cdot sub_1(\sigma,\sigma^*) \cdot u(\sigma^*))
\cr
\forall n\from N \quad con_2(n) &= u(W(n))\inv \cdot con_1(n) \cdot u(n)
\cr
\forall e\from E \quad rel_2(e) &= u(A(S(e)))\inv \cdot rel_1(e) \cdot
u(A(F(e))) \cr
\forall \sigma\from\Sigma \quad tem_2(\sigma) &= tem_1(\sigma) \circ
u(\sigma)
\cr
\forall \sigma\from\Sigma \quad in_2(\sigma)
&= u(\sigma)\inv \cdot in_1(\sigma) \cdot u(\sigma)
}$$
and hence
$$ (v \cdot u) \circ f =
(sub', con_2\circ f, rel_2\circ f, symm_1\circ f, tem_2\circ f, in_2\circ f) $$
where
$$ \forall \sigma,\sigma^*\from\Sigma' \quad (G'(\sigma,\sigma^*) \ \Rightarrow\
sub'(\sigma,\sigma^*) = sub_2(f(\sigma),f(\sigma^*))). $$

We also have $v\circ f = (sub'', con_1\circ f, rel_1\circ f, symm_1\circ f,
tem_1\circ f, in_1\circ f)$, where
$$ \forall \sigma,\sigma^*\from\Sigma' \quad (G'(\sigma,\sigma^*) \ \Rightarrow\
sub''(\sigma,\sigma^*) = sub_1(f(\sigma),f(\sigma^*))). $$
Hence $(v\circ f) \cdot (u\circ f) = (sub_3, con_3, rel_3, symm_1\circ f, tem_3,
in_3)$, where
$$\eqalign{
\forall \sigma,\sigma^*\from\Sigma' \quad (G'(\sigma,\sigma^*) \ \Rightarrow \
sub_3(\sigma,\sigma^*)
&= (u \circ f)(\sigma)\inv \cdot sub''(\sigma,\sigma^*) \cdot
(u \circ f)(\sigma^*) \cr
&= u(f(\sigma))\inv \cdot sub_1(f(\sigma),f(\sigma^*)) \cdot
u(f(\sigma^*)) \cr
&= sub_2(f(\sigma), f(\sigma^*))
= sub'(\sigma,\sigma^*))
\cr
\forall n\from N' \quad con_3(n)
&= (u\circ f)(W'(n))\inv \cdot (con_1\circ f)(n) \cdot (u\circ f)(n) \cr
&= u(f(W'(n)))\inv \cdot con_1(f(n)) \cdot u(f(n)) \cr
&= u(W(f(n)))\inv \cdot con_1(f(n)) \cdot u(f(n)) \cr
&= con_2(f(n)) = (con_2 \circ f)(n) \cr
\forall e\from E' \quad
rel_3(e) &=
(u\circ f)(A'(S'(e)))\inv \cdot (rel_1\circ f)(e) \cdot (u\circ f)(A'(F'(e)))
\cr
&= u(f(A'(S'(e))))\inv \cdot rel_1(f(e)) \cdot u(f(A'(F'(e)))) \cr
&= u(A(S(f(e))))\inv \cdot rel_1(f(e)) \cdot u(A(F(f(e)))) \cr
&= rel_2(f(e)) = (rel_2 \circ f)(e) \cr
\forall \sigma\from\Sigma' \quad
tem_3(\sigma) &= (tem_1\circ f)(\sigma) \circ (u\circ f)(\sigma) \cr
&= tem_1(f(\sigma)) \circ u(f(\sigma)) \cr
&= tem_2(f(\sigma)) = (tem_2 \circ f)(\sigma) \cr
\forall \sigma\from\Sigma' \quad
in_3(\sigma)
&= (u\circ f)(\sigma)\inv \cdot (in_1\circ f)(\sigma) \cdot (u\circ f)(\sigma)
\cr
&= u(f(\sigma))\inv \cdot in_1(f(\sigma)) \cdot u(f(\sigma)) \cr
&= in_2(f(\sigma)) = (in_2 \circ f)(\sigma)
}$$
which shows that $(v \cdot u) \circ f= (v\circ f) \cdot (u\circ f)$. \qed

\defn If $\N'=\network{'}$ is a subnetwork of $\N$, with 
inclusion homomorphism $f:\N'\to\N$,

\item{(i)} the \i{restriction} of $u$, an embedding token for $\N$, to $\N'$,
denoted $u|_{\N'}$, is defined as $u \circ f = u|_{\Sigma'\cup N'}$; this
is an embedding token for $\N'$ by theorem~25;

\item{(ii)} the \i{restriction} of $v$, an embedding type for $\N$, to $\N'$,
denoted $v|_{\N'}$, is defined as $v \circ f$, an embedding type for $\N'$.

\subhead{4.3 Symmetries}

\defn A \i{symmetry} of a network $\N=\network{}$, with respect to the embedding
type $v=(sub,con,rel,symm,tem,in)$, is a pair $(a,s)$, where $a:\N\to\N$ is an
automorphism of $\N$ and $s$ is an embedding token for $\N$, such that

\blob $\forall \sigma\from\Sigma \ s(\sigma) \in symm(\sigma)$,

\blob $\forall n\from N \ s(n) \in symm(P(n))$,

\blob $v \cdot s = v \circ a$.

\medskip\f
This is just as in (2004, \S7.5). However, the operation of global application
of a symmetry of the grammar to the pattern, in lemma~2, needs to be
generalised to \i{local} symmetries, in which different symmetries are applied
to different symbols of the pattern

\defn Given networks $\N_1=\network{_1}$ and $\N_0=\network{_0}$, a homomorphism
$p:\N_1\to\N_0$, and an embedding token $v$ on $\N_0$, define $\Cal S_0$ as the
group of symmetries of $\N_0$ with respect to $v$. A \i{local symmetry} of
$\N_1$ with respect to $\N_0,p,v$ is a function $\pi:\Sigma_1 \to \Cal S_0$ such
that

\blob $\forall \sigma,\sigma^*\from\Sigma_1\ (G_1(\sigma,\sigma^*) \Rightarrow
\pi(\sigma)=\pi(\sigma^*))$,

\blob $\forall e\from E_1\ \pi(W_1(A_1(F_1(e)))) = \pi(W_1(A_1(S_1(e))))$,

\blob $\forall n \from N_1\ a(P_1(n))(p(P_1(n))) = a(W_1(n))(p(P_1(n)))$,

\medskip\f
where $\pi$ is decomposed into components by $\forall\sigma\from\Sigma_1\
\pi(\sigma) = (a(\sigma),s(\sigma))$, for functions $a,s$.

\medskip\f
Given a local symmetry $\pi$ and an embedding token $u$ for $\N_1$, the
\i{application of $\pi$ to $p,u$} produces a new homomorphism $p':\N_1\to\N_0$,
defined by
$$\eqalign{
&\forall \sigma\from\Sigma_1 \cr
&\forall n\from N_1 \cr
&\forall h\from H_1 \cr
&\forall e\from E_1 \cr
&\forall k\from K_1 \cr
}\ \ \eqalign{
p'(\sigma) &= a(\sigma)(p(\sigma)) \cr
p'(n) &= a(W_1(n))(p(n)) \cr
p'(h) &= a(W_1(A_1(h)))(p(h)) \cr
p'(e) &= a(W_1(A_1(F_1(e))))(p(e)) \cr
p'(k) &= a(W_1(A_1(F_1(C_1(k)))))(p(k)), \cr
}$$
and a new embedding token $u'=u \cdot s'$ for $\N_1$, where the embedding token
$s'$ is defined by
$$\eqalign{
&\forall \sigma\from\Sigma_1 \cr
&\forall n\from N_1
}\ \ \eqalign{
s'(\sigma) &= s(\sigma)(p(\sigma)) \cr
s'(n) &= s(W_1(n))(p(n)).
}$$

\theorem 27. In the above definition, $p':\N_1\to\N_0$ is a homomorphism and
$s',u'$ are embedding tokens for $\N_1$, as claimed.

\proof We shall continue to use the above notation.

First we verify that $p':\N_1\to\N_0$ is a homomorphism. The conditions
$$ p'(\Sigma_1) \subseteq \Sigma_0, \quad p'(N_1) \subseteq N_0, \quad
p'(H_1) \subseteq H_0, \quad p'(E_1) \subseteq E_0, \quad p'(K_1) \subseteq
K_0 $$
are immediate.

Next we check $W_0 \circ p' = p' \circ W_1$:
$$\eqqalign\quad{
\forall n\from N_1\quad W_0(p'(n))
&= W_0\bigl(a(W_1(n))(p(n))\bigr)
&\cr
&= a(W_1(n))\bigl(W_0(p(n))\bigr)
&\text{since $a(W_1(n))$ is an automorphism}\cr
&= a(W_1(n))\bigl(p(W_1(n))\bigr)
&\text{since $p$ is an homomorphism}\cr
&= p'(W_1(n)),
&\cr
}$$
$$ \forall \sigma\from\Sigma_1\quad W_0(p'(\sigma))
= p'(\sigma)
= p'(W_1(\sigma)). \kern150pt $$
Next we check $P_0 \circ p' = p' \circ P_1$:
$$\eqqalign\quad{
\forall n\from N_1 \quad P_0(p'(n))
&= P_0\bigl(a(W_1(n))(p(n))\bigr)
&\cr
&= a(W_1(n))\bigl(P_0(p(n))\bigr)
&\text{since $a(W_1(n))$ is an automorphism}\cr
&= a(W_1(n))\bigl(p(P_1(n))\bigr)
&\text{since $p$ is an homomorphism}\cr
&= a(P_1(n))\bigl(p(P_1(n))\bigr)
&\text{since $\pi$ is a local symmetry}\cr
&= p'(P_1(n)).
&\cr
}$$
Next we check $F_0 \circ p' = p' \circ F_1$:
$$\eqqalign\quad{
\forall e\from E_1 \quad F_0(p'(e))
&= F_0\bigl(a(W_1(A_1(F_1(e))))(p(e))\bigr)
&\cr
&= a(W_1(A_1(F_1(e))))\bigl(F_0(p(e))\bigr)
&\text{since $a(W_1(A_1(F_1(e))))$ is an automorphism}\cr
&= a(W_1(A_1(F_1(e))))\bigl(p(F_1(e))\bigr)
&\text{since $p$ is a homomorphism}\cr
&= p'(F_1(e)).
&\cr
}$$
Next we check $S_0 \circ p' = p' \circ S_1$:
$$\eqqalign\quad{
\forall e\from E_1 \quad S_0(p'(e))
&= S_0\bigl(a(W_1(A_1(F_1(e))))(p(e))\bigr)
&\cr
&= a(W_1(A_1(F_1(e))))\bigl(S_0(p(e))\bigr)
&\text{since $a(W_1(A_1(F_1(e))))$ is an automorphism}\cr
&= a(W_1(A_1(F_1(e))))\bigl(p(S_1(e))\bigr)
&\text{since $p$ is a homomorphism}\cr
&= a(W_1(A_1(S_1(e))))\bigl(p(S_1(e))\bigr)
&\text{since $\pi$ is a local symmetry}\cr
&= p'(S_1(e)).
&\cr
}$$
Next we check that $\rectangleA{N_0\cup\Sigma_0}{N_1\cup\Sigma_1}{H_0}{H_1}
{p'|_{N_1\cup\Sigma_1}}{A_0}{A_1}{p'|_{H_1}}$ is a pullback in the category of
sets. The equation $A_0 \circ p'|_{H_1} = p'|_{N_1\cup\Sigma_1} \circ A_1$
follows by
$$\eqqalign\quad{
\forall h\from H_1\quad A_0(p'(h))
&= A_0\bigl(a(W_1(A_1(h)))(p(h))\bigr)
&\cr
&= a(W_1(A_1(h)))\bigl(A_0(p(h))\bigr)
&\text{since $a(W_1(A_1(h)))$ is an automorphism}\cr
&= a(W_1(A_1(h)))\bigl(p(A_1(h))\bigr)
&\text{since $p$ is an homomorphism}\cr
&= p'(A_1(h)).
&\cr
}$$
The other half of the pullback condition is
$$ \forall h_0\from H_0\ \forall x_1\from N_1\cup\Sigma_1 \quad
(A_0(h_0) = p'(x_1) \ \Rightarrow\ \exists!h_1\from H_1\ (A_1(h_1)=x_1 \wedge
p'(h_1)=h_0)). \eqno (1) $$
To prove this, consider any $h_0\from H_0$ and any $x_1\from N_1\cup\Sigma_1$.
Define $a^*=a(W_1(x_1))$, an automorphism of $\N_0$. By theorem~15, $a^* \circ
p:\N_1\to\N_0$ is a homomorphism, so the pullback
$\longrectangleA{N_0\cup\Sigma_0}{N_1\cup\Sigma_1}{H_0}{H_1} {(a^*\circ
p)|_{N_1\cup\Sigma_1}}{A_0}{A_1}{(a^*\circ p)|_{H_1}}$ implies
$$ A_0(h_0) = a^*(p(x_1)) \ \Rightarrow\
\exists!h_1\from H_1\ (A_1(h_1)=x_1 \wedge a^*(p(h_1))=h_0). \eqno (2) $$
Now, $p'(x_1) = a^*(p(x_1))$; and, for any $h_1\from H_1$, if $A_1(h_1)=x_1$
then $p'(h_1) = a(W_1(A_1(h_1)))(p(h_1)) = a^*(p(h_1))$. Thus (2) may be
rewritten, and quantifiers over $h_0$ and $x_1$ added, to give (1). This
completes the proof of the pullback.

The pullback $\rectangleA{E_0}{E_1}{K_0}{K_1}{p'|_{E_1}}{C_0}{C_1}{p'|_{K_1}}$
is verified similarly.

Next we check that $G_0 \circ \overline{p'} = \overline{p'} \circ G_1$ and $G_1$
is minimal relative to $p'$. Let us restrict our attention to nodes in the first
instance. In view of theorem~14, we have to show
$$\eqalign{
&\forall n_0\from N_0\ \forall n_1^*\from N_1\ \ 
(G_0(n_0,p'(n_1^*)) \ \Leftrightarrow\
\exists n_1\from N_1\ (n_0 = p'(n_1) \wedge G_1(n_1,n_1^*))); \cr
&\forall n_0\from N_0\ \forall n_1^*\from N_1\ \ 
\exists^{\le1} n_1\from N_1\ (n_0 = p'(n_1) \wedge G_1(n_1,n_1^*)).}
\eqno(3) $$
To prove these, consider any $n_0\from N_0$ and any $n_1^*\from N_1$. Define
$a^*=a(W_1(n_1^*))$, an automorphism of $\N_0$. By theorem~15, $a^* \circ
p:\N_1\to\N_0$ is a homomorphism, so
$$\eqalign{
&G_0(n_0,a^*(p(n_1^*))) \ \Leftrightarrow\
\exists n_1\from N_1\ (n_0 = a^*(p(n_1)) \wedge G_1(n_1,n_1^*)); \cr
&\exists^{\le1} n_1\from N_1\ (n_0 = a^*(p(n_1)) \wedge G_1(n_1,n_1^*)).}
\eqno(4) $$
Now, the condition $G_0(n_0,a^*(p(n_1^*)))$ is equivalent to
$G_0(n_0,p'(n_1^*))$, since $a^*(p(n_1^*)) = p'(n_1^*)$. Moreover, for any
$n_1\from N_1$, if $G_1(n_1,n_1^*)$ then $G_1(W_1(n_1),W_1(n_1^*))$, by
$\overline{W_1} \circ G_1 \subseteq G_1 \circ \overline{W_1}$, so
$\pi(W_1(n_1))=\pi(W_1(n_1^*))$, so $a(W_1(n_1))=a(W_1(n_1^*))=a^*$, so $p'(n_1)
= a(W_1(n_1))(p(n_1)) = a^*(p(n_1))$. Thus the condition $n_0 = a^*(p(n_1))
\wedge G_1(n_1,n_1^*)$ is equivalent to $n_0 = p'(n_1) \wedge G_1(n_1,n_1^*)$.
Hence (4) may be rewritten (quantifying over $n_0$ and $n_1^*$) as (3), as
required. This deals with the node case. Statements similar to (3) for symbols,
hooks, edges and facets can be proved in the same way, completing the proof that
$G_0 \circ \overline{p'} = \overline{p'} \circ G_1$ and $G_1$ is minimal
relative to $p'$.

This completes the proof that $p':\N_1\to\N_0$ is a homomorphism.

Next we verify that $s'$ is an embedding token for $\N_1$. Consider any
$n,n^*\from N_1$ such that $G_1(n,n^*)$ holds. We must show that
$s'(n)=s'(n^*)$.

First, $\pi(W_1(n))$ is a symmetry of $\N_0$, so $s(W_1(n))$ is an embedding
token for $\N_0$; moreover, $G_0(p(n),p(n^*))$ holds; so $s(W_1(n))(p(n)) =
s(W_1(n))(p(n^*))$.

Secondly, we have $G_1(W_1(n),W_1(n^*))$, so $\pi(W_1(n))=\pi(W_1(n^*))$, so
$s(W_1(n))=s(W_1(n^*))$.

Putting these two observations together,
$$ s'(n) = s(W_1(n))(p(n)) = s(W_1(n))(p(n^*)) = s(W_1(n^*))(p(n^*)) = s'(n^*)
$$
as required. It follows now that $u' = u \cdot s'$ is an embedding token for
$\N_1$. \qed

\subhead{4.4 Templates and saturation}
The concepts of an image, a template, and the correlation function $\rho_{I,T}$
are carried over from (2004, \S 4), with two modifications.

The first modification is intended to prevent two identical symbol tokens from
forming at the same place in the image, or more generally to prevent two or
more symbol tokens from claiming credit for the same patch of the image. If two
or more symbol tokens' templates overlap in the image plane, i.e., if there are
points $x$ in the image plane where $tem(\sigma)(u(\sigma)\inv(x)) > 0$ for two
or more symbol tokens $\sigma$, then the point $x$ should become \i{saturated}
and the contribution it makes to the correlation function should be reduced.
For this it is necessary to calculate the saturation $sat(x)$ of each point
$x$, which is roughly the sum of $tem(\sigma)(u(\sigma)\inv(x))$ over each
symbol token $\sigma$. (However, this needs modification for subsymbols to
avoid double-counting.) The formal definition of saturation follows.

Suppose we are given a definite network $\N=\network{}$, an embedding token $u$ for $\N$,
and a function $tem:\Sigma\to Tem$. The \i{(definite) saturation function}, 
$sat:\R^2\to\R$, is defined by
$$ \forall x\from\R^2\quad
sat(x) = \sum_{\sigma\in\Sigma} (1-g_\sigma) \, tem(\sigma)(u(\sigma)\inv(x)) $$
where $g_\sigma = \bigl|\comp{\sigma^*\from\Sigma}{G(\sigma^*,\sigma)}\bigr|$.
We call $sat(x)$ the \i{saturation at} $x$.

The correlation function $\rho_{I,T}$, between an image $I$ and a template $T$,
was defined in (2004, \S4.2) by
$$ \rho_{I,T}(g) = |det(\rep g)| \int T(u) \, (I(g(u))-I_0) \d^2u =
\int T(g\inv(x)) \, (I(x)-I_0) \d^2x $$
for any affine transformation $g$, where $\rep g$ is the matrix representation
of $g$ and $I_0$ is a positive real constant associated with $T$. This must now
be modified to take account of saturation:
$$ \rho_{I,T,sat}(g)
= |det(\rep g)| \int w(sat(g(u))) \, T(u) \, (I(g(u))-I_0) \d^2u
= \int w(sat(x)) \, T(g\inv(x)) \, (I(x)-I_0) \d^2x $$
where $w$ is a weighting function that suppresses the integrand at points $x$
where $sat(x)$ is above 1. A suitable definition of $w$ is
$$ \forall s\from\R\quad w(s) =
\cases{
1 & if $s \le 1$, \cr
(1.6-s)/0.6 & if $1 < s < 1.6$, \cr
0 & if $1.6 \le s$.
}$$

The second modification is to give the factor of $|\det(\rep g)|$ that
occurs in the formula for $\rho_{I,T,sat}(g)$ an adjustable exponent:
$$\eqalign{
\rho_{I,T,sat}(g)
&= |det(\rep g)|^{1-k} \int w(sat(g(u))) \, T(u) \, (I(g(u))-I_0) \d^2u \cr
&= |\det(\rep g)|^{-k} \int w(sat(x)) \, T(g\inv(x)) \, (I(x)-I_0) \d^2x
}$$
where $k$ is a constant characteristic of the template, with $0 \le k \le 1$
normally. 

\def\I{\Bbb I}
\def\intx#1{\int w(sat(x)) \, #1 \d^2x}
\def\intu#1{\int w(sat(g(u))) \, #1 \d^2u}

The calculation of template force in (2004, \S4.3) is affected by these two
changes as follows. For any $g\from\G$ and $A\from\A$,
$$\eqalign{
\rho_{I,T,sat}(g \cdot \exp A) 
&= |\det(\rep{g\cdot\exp A})|^{-k} \intx{T((g\cdot \exp A)\inv(x))(I(x)-I_0)}
\cr
&= |\det(\rep g\cdot\exp\rep A)|^{-k} \intx{\rep T((\rep g \exp\rep A)\inv\rep x)(I(x)-I_0)}
\cr
&= |\det(\rep g)|^{-k} e^{-k\tr(\rep A)} \intx{\rep T(\exp(-\rep A)\rep g\inv\rep x)(I(x)-I_0)}
\cr
&= |\det(\rep g)|^{-k} (\I-k\tr(\rep A) + o(A)) \kern-2pt \intx{\rep T((\I-\rep A+o(A))\rep g\inv\rep x)(I(x)-I_0)}
\cr
&= |\det(\rep g)|^{-k} (\I-k\tr(\rep A) + o(A)) \cdot
\cr&
\hskip63pt \intx{\bigl(\rep T(\rep g\inv\rep x) - (\rep\nabla T(g\inv x))\rep
A\rep g\inv\rep x + o(A)\bigr)(I(x)-I_0)}
\cr
&= \rho_{I,T,sat}(g) - k\tr(\rep A)\rho_{I,T,sat}(g)
\cr&\kern59pt 
- |\det(\rep g)|^{-k} \intx{\bigl((\rep\nabla T(g\inv x))\rep A\rep g\inv\rep
x\bigr)(I(x)-I_0)} + o(A)
}$$
where $\I$ is the $6\times6$ identity matrix.
Hence the derivative $\rho_{I,T,sat*}:\G \to (\A \to \R)$ is defined by
$$\eqalign{
\forall g\from\G\ \forall A\from\A\ \ \rho_{I,T,sat*}(g)(A) 
=& - k\tr(\rep A)\rho_{I,T,sat}(g)
\cr
& - |\det(\rep g)|^{-k} \intx{\bigl((\rep\nabla T(g\inv x))\rep A\rep g\inv\rep
x\bigr)(I(x)-I_0)} 
\cr
=& - k\tr(\rep A)\rho_{I,T,sat}(g)
\cr
& - |\det(\rep g)|^{1-k} \intu{\bigl((\rep\nabla T(u))\rep A\rep
u\bigr)(I(g(u))-I_0)}. 
}$$
This gives a matrix representation for the force,
$$\eqalign{
\forall g\from\G\ \ \rep{\rho_{I,T,sat*}(g)} 
=& 
- k\rho_{I,T,sat}(g)\I
- |\det(\rep g)|^{-k} \intx{\bigl(\rep g\inv \rep x(\rep\nabla
T(g\inv(x)))\bigr)(I(x)-I_0)}
\cr
=& 
- k\rho_{I,T,sat}(g)\I
- |\det(\rep g)|^{1-k} \intu{\bigl(\rep u(\rep\nabla T(u))\bigr)(I(g(u))-I_0)}.
}$$

\subhead{4.5 The definite match function}
The \i{definite match function} $DM$ measures how well a definite network
$\N=\network{}$ matches an image $I$, given an embedding token $u$ for $\N$, and
an embedding type $v=(sub,con,rel,symm,tem,in)$ for $\N$. It is defined by
$$\eqalign{
DM(I, \N, u, v)
=& \sum_{\sigma\in\Sigma} \rho_{I,tem(\sigma),sat}(u(\sigma))
\ - \ \theta |\Sigma\setdiff P(N)|
\ - \sum_{(\sigma,\sigma^*)\mid G(\sigma,\sigma^*)} \kern-15pt
E_{sub(\sigma,\sigma^*)}\bigl(u(\sigma)\inv \cdot u(\sigma^*)\bigr)
\cr&
\ - \ \sum_{n\in N} E_{con(n)}\bigl(u(W(n))\inv \cdot u(n)\bigr)
\ - \ \sum_{e\in E} E_{rel(e)}\bigl(u(A(S(e)))\inv \cdot u(A(F(e)))\bigr)
}$$
where $\theta$ is a positive real constant and $sat$ is the definite saturation
function, as defined in the previous section. 

The first term on the right-hand side is a sum over all symbols; $tem(\sigma)$
is the template for $\sigma$, and $\rho_{I,tem(\sigma),sat}(u(\sigma))$
measures the correlation between the template (embedded in the image using
$u(\sigma)$) and the image $I$.

The second term on the right-hand side applies a fixed penalty of $\theta$ for
each \ic{bare} symbol, i.e., each symbol that is not a part of another symbol.
This term encourages the symbols to connect themselves together rather than
remaining separate.

The third term measures how well each subsymbol matches its supersymbol
geometrically. The summation is over all pairs $(\sigma,\sigma^*)$ such that
$\sigma$ is a supersymbol of $\sigma^*$; $sub(\sigma,\sigma^*)$ is a fleximap
that defines what the geometric relationship between $\sigma^*$ and $\sigma$
should be; $u(\sigma)\inv \cdot u(\sigma^*)$ is the actual relationship between
them; the quadratic penalty function $E_\tau(G)$ calculates the penalty for the
deviation between an affine transformation $G$ and a fleximap $\tau$, as
defined in (2004, \S5.3).

The fourth term measures how well each part matches its whole geometrically. The summation
is over all nodes $n$; $P(n)$ is the part symbol and $W(n)$ is the whole
symbol. The node $n$ has its own embedding $u(n)$, which equals $u(P(n))$ up
to a symmetry; $u(W(n))\inv \cdot u(n)$ is the actual geometric relationship
between the part (or rather the node) and the whole; $con(n)$ is a fleximap
specifying what the relationship should be.

The final term measures how well each pair of siblings match geometrically.
The sum is over every edge $e$, representing a sibling relationship between two
nodes $A(F(e))$ and $A(S(e))$; $u(A(S(e)))\inv \cdot u(A(F(e)))$ is the actual
relationship and $rel(e)$ is the fleximap specifying what the relationship
should be.

All these fleximaps are provided by the embedding type $v$; the final
component $in$ of $v$ is not used yet.

The way $DM$ will be used in the statement of the recognition problem is as
follows. An embedding type $v$ for the grammar $\N_0$ is given at the outset.
The parsing homomorphism $p:\N_1\to\N_0$ induces an embedding type $v\circ p$
for $\N_1$. An embedding token $u$ for $\N_1$ is constructed by the parser,
satisfying the symmetry condition for $\N_1,u,v\circ p$. At the end of recognition,
when $\N_1$ is definite, we measure how well $u$ matches $v \circ p$ by
calculating $DM(I,\N_1,u,v\circ p)$.

\subhead{4.6 Invariance theorems}
Lemmas~1 and 2 from (2004, \S7) hold for the definite match function $DM$;
I shall restate them here, but with lemma~2 generalised from global symmetries
to local symmetries. I shall also add two new theorems on the affine invariance
of the $\rho$ and match functions.

\theorem 28. (Lemma~1 of (2004, \S7.3): invariance under affine transformation
of the symbols' internal frames of reference.) For any image $I$, definite
network $\N$,
embedding tokens $u,u'$ for $\N$, and embedding type $v$ for $\N$, then
$$ DM(I, \N, u\cdot u', v\cdot u') = DM(I, \N, u, v); $$

\proof The proof is very similar to the one in (2004), but I shall restate it in
full. Let $v=(sub_1, con_1, \allowbreak rel_1, \allowbreak symm_1, tem_1,in_1)$;
then $v\cdot u'=(sub_2, con_2,rel_2,symm_1,tem_2,in_2)$, where
$$\eqalign{
\forall \sigma,\sigma^* \from \Sigma \quad (G(\sigma,\sigma^*) \ \Rightarrow\
sub_2(\sigma,\sigma^*)
&= u'(\sigma)\inv \cdot sub_1(\sigma,\sigma^*) \cdot u'(\sigma^*))
\cr
\forall n\from N \quad con_2(n) &= u'(W(n))\inv \cdot con_1(n) \cdot u'(n)
\cr
\forall e\from E \quad rel_2(e) &= u'(A(S(e)))\inv \cdot rel_1(e) \cdot
u'(A(F(e))) \cr
\forall \sigma\from\Sigma \quad tem_2(\sigma) &= tem_1(\sigma) \circ
u'(\sigma)
\cr
\forall \sigma\from\Sigma \quad
in_2(\sigma) &= u'(\sigma)\inv \cdot in_1(\sigma) \cdot u'(\sigma)
}$$
Now, first, for any $\sigma\from\Sigma$,
$$ \rho_{I,tem_2(\sigma),sat}((u\cdot u')(\sigma))
= \rho_{I,tem_1(\sigma)\circ u'(\sigma),sat}(u(\sigma)\cdot u'(\sigma))
= \rho_{I,tem_1(\sigma),sat}(u(\sigma)) $$
using lemma~1 of (2004, \S4.2). Note that the saturation function $sat$ is
unchanged by the application of $u'$. This is because
$$ \forall \sigma\from\Sigma\ \forall x\from\R^2\quad\!\!
tem_2(\sigma)((u\cdot u')(\sigma)\inv(x))
= (tem_1(\sigma) \circ u'(\sigma))(u'(\sigma)\inv(u(\sigma)\inv(x)))
= tem_1(\sigma)(u(\sigma)\inv(x)) $$
and so the calculation of $sat(x)$ is unaffected.

Secondly, for any $\sigma,\sigma^* \from \Sigma$ such that $G(\sigma,\sigma^*)$,
$$\eqalign{
E_{sub_2(\sigma,\sigma^*)}((u\cdot u')(\sigma)\inv \cdot (u\cdot u')(\sigma^*))
&=
E_{u'(\sigma)\inv \cdot sub_1(\sigma,\sigma^*) \cdot u'(\sigma^*)}
(u'(\sigma)\inv \cdot u(\sigma)\inv \cdot u(\sigma^*) \cdot u'(\sigma^*))
\cr&
= E_{sub_1(\sigma,\sigma^*)}(u(\sigma)\inv \cdot u(\sigma^*))
}$$
by lemma~1 of (2004, \S5.3).

Thirdly, for any $n\from N$,
$$\eqalign{
E_{con_2(n)}((u\cdot u')&(W(n))\inv \cdot (u\cdot u')(n))
\cr&
= E_{u'(W(n))\inv \cdot con_1(n) \cdot u'(n)}
(u'(W(n))\inv \cdot u(W(n))\inv \cdot u(n) \cdot u'(n))
\cr&
= E_{con_1(n)}(u(W(n))\inv \cdot u(n))
}$$
by lemma~1 of (2004, \S5.3).

Fourthly, for any $e\from E$, using the abbreviations $n_1=A(F(e))$ and
$n_2=A(S(e))$,
$$\eqalign{
E_{rel_2(e)}((u\cdot u')(n_2)\inv \cdot (u\cdot u')(n_1))
&=E_{u'(n_2)\inv \cdot rel_1(e) \cdot u'(n_1)}
(u'(n_2)\inv \cdot u(n_2)\inv \cdot u(n_1) \cdot u'(n_1))
\cr&
= E_{rel_1(e)}(u(n_2)\inv \cdot u(n_1))
}$$
and, using the abbreviations $\sigma_1=W(A(F(e)))$ and $\sigma_2=W(A(S(e)))$,
$$\eqalign{
E_{in_2(\sigma_1)}((u\cdot u')(\sigma_2)\inv \cdot (u\cdot u')(\sigma_1))
&= E_{u'(\sigma_1)\inv \cdot in_1(\sigma_1) \cdot u'(\sigma_1)}
(u'(\sigma_2)\inv \cdot u(\sigma_2)\inv \cdot
u(\sigma_1) \cdot u'(\sigma_1))
\cr&
= E_{in_1(\sigma_1)}(u(\sigma_2)\inv \cdot u(\sigma_1))
}$$
by lemma~1 of (2004, \S5.3) again, using the assumption that $u'(\sigma_1) =
u'(\sigma_2)$ (which holds under the conditions of (i) or (ii)).

Thus each term of $DM(I, \N, u\cdot u', v\cdot u')$ equals the corresponding
term of $DM(I, \N, u, v)$. \qed

\theorem 29. (Invariance of $DM$ under a local symmetry.) Given
an image $I$, a semi-definite network $\N_0$, a definite network $\N_1$, 
a homomorphism
$p:\N_1\to\N_0$, an embedding token $u$ for $\N_1$, an embedding type $v$ for
$\N_0$, and a local symmetry $\pi$ of $\N_1$ with respect to $\N_0,p,v$, the
application of $\pi$ to $p,u$ produces a homomorphism $p':\N_1\to\N_0$ and an
embedding token $u'$ for $\N_1$.

Then 

(i) $DM(I, \N_1, u', v\circ p') = DM(I, \N_1, u, v\circ p)$,

(ii) The symmetry condition holds for $\N_1,u',v \circ p'$ iff it holds for
$\N_1,u,v \circ p$.

\proof We begin by recapitulating the relevant definitions and notation. Define
functions $a,s$ by $\forall\sigma\from\Sigma_1\
\pi(\sigma)=(a(\sigma),s(\sigma))$. Then $p'$ is given by
$$\eqalign{
&\forall \sigma\from\Sigma_1 \cr
&\forall n\from N_1 \cr
&\forall h\from H_1 \cr
&\forall e\from E_1 \cr
&\forall k\from K_1 \cr
}\ \ \eqalign{
p'(\sigma) &= a(\sigma)(p(\sigma)) \cr
p'(n) &= a(W_1(n))(p(n)) \cr
p'(h) &= a(W_1(A_1(h)))(p(h)) \cr
p'(e) &= a(W_1(A_1(F_1(e))))(p(e)) \cr
p'(k) &= a(W_1(A_1(F_1(C_1(k)))))(p(k)) \cr
} \eqno (1) $$
and $u' = u \cdot s'$, where $s'$ is an embedding token for $\N_1$ defined by
$$\eqalign{
\forall \sigma\from\Sigma_1 \cr
\forall n\from N_1
}\ \ \eqalign{
s'(\sigma) &= s(\sigma)(p(\sigma)) \cr
s'(n) &= s(W_1(n))(p(n)).
} \eqno (2) $$
Also, $v=(sub,con,rel,symm,tem,in)$, and, for any $\sigma^\dagger\from\Sigma_1$,
$(a(\sigma^\dagger),s(\sigma^\dagger))$ is a symmetry of $\N_0$ with respect to
$v$, so $v \circ a(\sigma^\dagger) = v \cdot s(\sigma^\dagger)$; in terms of
components this means
$$\eqalign{
&(sub^\ddagger, con \circ a(\sigma^\dagger),
rel \circ a(\sigma^\dagger), symm \circ a(\sigma^\dagger),
tem \circ a(\sigma^\dagger), in \circ a(\sigma^\dagger))
= v \circ a(\sigma^\dagger)
\cr
& = v \cdot s(\sigma^\dagger) =
(sub^\dagger,con^\dagger,rel^\dagger,symm,tem^\dagger,in^\dagger)
}\eqno (3) $$
where $sub^\ddagger,sub^\dagger,con^\dagger,rel^\dagger,tem^\dagger,in^\dagger$
are defined by
$$\eqalign{
\forall \sigma,\sigma^* \from \Sigma_0 \quad (G_0(\sigma,\sigma^*) \ \Rightarrow\
sub^\ddagger(\sigma,\sigma^*) &=
sub(a(\sigma^\dagger)(\sigma),a(\sigma^\dagger)(\sigma^*))) \cr
\forall \sigma,\sigma^* \from \Sigma_0 \quad (G_0(\sigma,\sigma^*) \ \Rightarrow\
sub^\dagger(\sigma,\sigma^*)
&= (s(\sigma^\dagger)(\sigma))\inv \cdot sub(\sigma,\sigma^*) \cdot
s(\sigma^\dagger)(\sigma^*)) \cr
\forall n\from N_0 \quad con^\dagger(n)
&= (s(\sigma^\dagger)(W_0(n)))\inv \cdot con(n) \cdot s(\sigma^\dagger)(n) \cr
\forall e\from E_0 \quad rel^\dagger(e)
&= (s(\sigma^\dagger)(A_0(S_0(e))))\inv \cdot rel(e) \cdot
s(\sigma^\dagger)(A_0(F_0(e))) \cr
\forall \sigma\from\Sigma_0 \quad tem^\dagger(\sigma)
&= tem(\sigma) \circ s(\sigma^\dagger)(\sigma) \cr
\forall \sigma\from\Sigma_0 \quad
in^\dagger(\sigma)
&= (s(\sigma^\dagger)(\sigma))\inv \cdot in(\sigma) \cdot
s(\sigma^\dagger)(\sigma).
} \eqno (4) $$
I claim that $v \circ p' = (v \circ p) \cdot s'$. To verify the claim we may
write the left-hand side as
$$ v \circ p'
= (sub', con \circ p', rel \circ p', symm \circ p', tem \circ p',
in \circ p') $$
where
$$ \forall\sigma,\sigma^*\from \Sigma_1 \quad (G_1(\sigma,\sigma^*) \Rightarrow
sub'(\sigma,\sigma^*) = sub(p'(\sigma),p'(\sigma^*))) \eqno (5) $$
and the right-hand side as
$$ (v \circ p) \cdot s' =
(sub'',con'',rel'',symm \circ p,tem'',in'') $$
where
$$\eqalign{
\forall \sigma,\sigma^* \from \Sigma_1 \quad 
(G_1(\sigma,\sigma^*) \ \Rightarrow\
sub''(\sigma,\sigma^*)
&= s'(\sigma)\inv \cdot sub(p(\sigma),p(\sigma^*)) \cdot s'(\sigma^*)) \cr
\forall n\from N_1 \quad con''(n) &= s'(W_1(n))\inv \cdot con(p(n)) \cdot
s'(n) \cr
\forall e\from E_1 \quad rel''(e) &= s'(A_1(S_1(e)))\inv \cdot rel(p(e))
\cdot s'(A_1(F_1(e))) \cr
\forall \sigma\from\Sigma_1 \quad tem''(\sigma) &= tem(p(\sigma)) \circ
s'(\sigma)
\cr
\forall \sigma\from\Sigma_1 \quad
in''(\sigma) &= s'(\sigma)\inv \cdot in(p(\sigma)) \cdot s'(\sigma).
} \eqno (6) $$
Now we can verify the claim by comparing the six components of $v \circ p'$ and
$(v \circ p) \cdot s'$.
$$\eqqalign{\ \ }{
\forall \sigma,\sigma^*\from\Sigma_1\ \ (G_1(\sigma,\sigma^*) \Rightarrow
\kern-30pt &
&\cr
sub'(\sigma,\sigma^*)
&= sub(p'(\sigma),p'(\sigma^*))
&\text{by (5)}\cr
&= sub\bigl(a(\sigma)(p(\sigma)),a(\sigma^*)(p(\sigma^*))\bigr)
&\text{by (1)}\cr
&= sub\bigl(a(\sigma)(p(\sigma)),a(\sigma)(p(\sigma^*))\bigr)
&\text{since $\pi$ is a local symmetry}\cr
&= sub^\ddagger(p(\sigma),p(\sigma^*))
&\text{by (4) with $\sigma^\dagger=\sigma$}\cr
&= sub^\dagger(p(\sigma),p(\sigma^*))
&\text{by (3)}\cr
&= \bigl(s(\sigma)(p(\sigma))\bigr)\inv \cdot sub(p(\sigma),p(\sigma^*)) \cdot
s(\sigma)(p(\sigma^*))
&\text{by (4)}\cr
&= \bigl(s(\sigma)(p(\sigma))\bigr)\inv \cdot sub(p(\sigma),p(\sigma^*)) \cdot
s(\sigma^*)(p(\sigma^*))
&\text{since $\pi$ is a local symmetry}\cr
&= s'(\sigma)\inv \cdot sub(p(\sigma),p(\sigma^*)) \cdot s'(\sigma^*)
&\text{by (2)}\cr
&= sub''(\sigma,\sigma^*))
&\text{by (6)}\cr
}$$

$$\eqqalign{\kern-5pt}{
\forall n \from N_1 \ \
(con \circ p')(n)
&= con(p'(n))
= con(a(W_1(n))(p(n)))
&\text{by (1)}\cr
&= con^\dagger(p(n))
&\text{by (3) with $\sigma^\dagger = W_1(n)$}\cr
&=\bigl(s(W_1(n))(W_0(p(n)))\bigr)\inv \!\cdot con(p(n)) \cdot s(W_1(n))(p(n))
&\kern5pt\text{by (4)}\cr
&=\bigl(s(W_1(n))(p(W_1(n)))\bigr)\inv \!\cdot con(p(n)) \cdot s(W_1(n))(p(n))
&\kern5pt\text{since $W_0 \circ p = p \circ W_1$}\cr
&=s'(W_1(n))\inv \cdot con(p(n)) \cdot s'(n)
&\text{by (2)}\cr
&= con''(n)
&\text{by (6)}\cr
}$$

$$\eqqalign{\kern-46pt}{
\forall e\from E_1 \ \ &(rel \circ p')(e)
= rel(p'(e))
= rel\bigl(a(W_1(A_1(F_1(e))))(p(e))\bigr)
&\text{by (1)}\cr
&= rel^\dagger(p(e))
&\text{by (3) with $\sigma^\dagger=W_1(A_1(F_1(e)))$}\cr
&= \bigl(s(\sigma^\dagger)(A_0(S_0(p(e))))\bigr)\inv \cdot rel(p(e))
\cdot s(\sigma^\dagger)(A_0(F_0(p(e))))
&\text{by (4)}\cr
&= \bigl(s(\sigma^\dagger)(p(A_1(S_1(e))))\bigr)\inv \cdot rel(p(e))
\cdot s(\sigma^\dagger)(p(A_1(F_1(e))))
&\text{since $p$ is a homomorphism}\cr
&= \bigl(s(W_1(A_1(S_1(e))))(p(A_1(S_1(e))))\bigr)\inv \cdot rel(p(e))
\cdot s(\sigma^\dagger)(p(A_1(F_1(e))))
&\cr&
&\text{since $\pi$ is a local symmetry}\cr
&= s'(A_1(S_1(e)))\inv \cdot rel(p(e)) \cdot s'(A_1(F_1(e)))
&\text{by (2)}\cr
&= rel''(e)
&\text{by (6)}\cr
}$$

$$\eqqalign\quad{
\forall\sigma\from\Sigma_1 \quad
(symm \circ p')(\sigma)
&= symm(p'(\sigma))
= symm(a(\sigma)(p(\sigma)))
&\text{by (1)}\cr
&= symm(p(\sigma))
&\text{by (3), with $\sigma^\dagger=\sigma$}\cr
&= (symm \circ p)(\sigma)
&\cr
}$$

$$\eqqalign\quad{
\forall\sigma\from\Sigma_1 \quad
(tem \circ p')(\sigma)
&= tem(p'(\sigma))
= tem(a(\sigma)(p(\sigma)))
&\text{by (1)}\cr
&= tem^\dagger(p(\sigma))
&\text{by (3) with $\sigma^\dagger=\sigma$}\cr
&= tem(p(\sigma)) \circ s(\sigma)(p(\sigma))
&\text{by (4)}\cr
&= tem(p(\sigma)) \circ s'(\sigma)
&\text{by (2)}\cr
&= tem''(\sigma)
&\text{by (6)}\cr
}$$

$$\eqqalign\quad{
\forall\sigma\from\Sigma_1 \quad
(in \circ p')(\sigma)
&= in(p'(\sigma))
= in(a(\sigma)(p(\sigma)))
&\text{by (1)}\cr
&= in^\dagger(p(\sigma))
&\text{by (3) with $\sigma^\dagger=\sigma$}\cr
&= (s(\sigma)(p(\sigma)))\inv \cdot in(p(\sigma)) \cdot
s(\sigma)(p(\sigma))
&\text{by (4)}\cr
&= s'(\sigma)\inv \cdot in(p(\sigma)) \cdot s'(\sigma)
&\text{by (2)}\cr
&= in''(\sigma)
&\text{by (6).}\cr
}$$
This completes the verification of the claim that $v \circ p' = (v \circ p)
\cdot s'$.

Now we are in a position to prove part (i) of the theorem:
$$\eqqalign\quad{
DM(I,\N_1,u',v \circ p')
&= DM(I,\N_1,u \cdot s', v \circ p')
&\cr
&= DM(I,\N_1,u \cdot s', (v \circ p) \cdot s')
&\text{by the claim}\cr
&= DM(I,\N_1,u,v \circ p)
&\text{by theorem~28(i).}\cr
}$$

For part (ii), consider any $n\from N_1$. Recall that, for any
$\sigma^\dagger\from\Sigma_1$, $symm \circ a(\sigma^\dagger) = symm$, by (3),
so, taking $\sigma^\dagger=P_1(n)$, $symm(a(P_1(n))(p(P_1(n)))) =
symm(p(P_1(n)))$ and hence
$$ symm(p'(P_1(n))) = symm(p(P_1(n))). \eqno(7) $$

Secondly, since $(a(P_1(n)),s(P_1(n)))$ is a symmetry of $\N_0$ with respect to
$v$,
$$ s(P_1(n))(p(P_1(n))) \in symm(p(P_1(n))) \eqno(8) $$
and, since $(a(W_1(n)),s(W_1(n)))$ is a symmetry of $\N_0$ with respect to $v$,
$$ s(W_1(n))(p(n)) \in symm(P_0(p(n))) = symm(p(P_1(n))). \eqno(9) $$

Now, suppose that the symmetry condition holds for $\N_1,u,v\circ p$. Then, for
any $n\from N_1$, $u(P_1(n))\inv \cdot u(n) \in symm(p(P_1(n)))$, so
$$\eqqalign\quad{
u'(P_1(n))\inv \cdot u'(n)
&= \bigl(s(P_1(n))(p(P_1(n)))\bigr)\inv \cdot u(P_1(n))\inv \cdot u(n) \cdot
s(W_1(n))(p(n))
&\cr
&\in symm(p(P_1(n)))
&\text{by (8) and (9)}\cr
&= symm(p'(P_1(n)))
&\text{by (7)}\cr
}$$
so the symmetry condition for $\N_1,u',v\circ p'$ holds. Conversely, suppose
that the symmetry condition for $\N_1,u',v\circ p'$ holds. Then, for any $n\from
N_1$, $u'(P_1(n))\inv \cdot u'(n) \in symm(p'(P_1(n))) = symm(p(P_1(n)))$, by
(7), so from
$$ u'(P_1(n))\inv \cdot u'(n)
= \bigl(s(P_1(n))(p(P_1(n)))\bigr)\inv \cdot u(P_1(n))\inv \cdot u(n) \cdot
s(W_1(n))(p(n)) $$
we have
$$\eqqalign\quad{
u(P_1(n))\inv \cdot u(n)
&= s(P_1(n))(p(P_1(n))) \cdot u'(P_1(n))\inv \cdot u'(n) \cdot
\bigl(s(W_1(n))(p(n))\bigr)\inv
&\cr
&\in symm(p(P_1(n)))
&\text{by (8) and (9)}\cr
}$$
so the symmetry condition for $\N_1,u,v\circ p$ holds. \qed

\theorem 30. (Affine invariance of the $\rho$ function.) For any template $T$,
any image $I$, and any affine transformations $g,g'$,
$$ \rho_{I\circ g\inv,T,sat\circ g\inv}(g\cdot g')
= |\det(\rep g)|^{1-k} \, \rho_{I,T,sat}(g').
$$

\medskip\f
(Recall that $\overline g$ is the matrix representation of $g$.)

\proof Recall the definition
$$ \rho_{I,T,sat}(g)
= |det(\rep g)|^{1-k} \int w(sat(g(u))) \, T(u) \, (I(g(u))-I_0) \d^2u. $$
Now,
$$\eqalign{
\rho_{I\circ g\inv,T,sat\circ g\inv}(g\cdot g')
&= |det(\rep{g\cdot g'})|^{1-k} \kern-3pt \int w((sat\circ g\inv)((g\cdot g')(u))) \, T(u) \,
((I\circ g\inv)((g\cdot g')(u))-I_0) \d^2u \cr
&= |det(\rep g)|^{1-k} \, |det(\rep{g'})|^{1-k} \kern-3pt \int w(sat(g'(u))) \, T(u) \,
(I(g'(u))-I_0) \d^2u \cr
&= |det(\rep g)|^{1-k} \, \rho_{I,T,sat}(g').
}\kern-5pt$$
\qed

\theorem 31. (Affine invariance of $DM$.) For any affine $g$
such that $|det(\overline g)|=1$, any image $I$, any definite network $\N=\network{}$,
any embedding token $u$ for $\N$, and any embedding type $v$ for $\N$, define a
new, affine-transformed image $I' = I \circ g\inv$, and a new,
affine-transformed embedding token $u'$ for $\N$ by $\forall x\from\Sigma\cup N\
u'(x) = g \cdot u(x)$. Then
$$ DM(I', \N, u', v) = DM(I, \N, u, v). $$

\proof Let $sat$ be the definite saturation function calculated using the 
embedding token $u$. Then the saturation function calculated using $u'$ is 
$sat'= sat \circ g\inv$, by the definition of $sat$ in \S4.4. By theorem~30
$$ \forall \sigma\from\Sigma \quad
\rho_{I',tem(\sigma),sat'}(u'(\sigma)) = \rho_{I,tem(\sigma),sat}(u(\sigma)). $$
Also,
$$ \forall \sigma,\sigma^*\from\Sigma \quad u'(\sigma)\inv \cdot u'(\sigma^*)
= u(\sigma)\inv \cdot g\inv \cdot g \cdot u(\sigma^*)
= u(\sigma)\inv \cdot u(\sigma^*) $$
and similarly
$$\eqalign{
\forall n\in N \quad u'(W(n))\inv \cdot u'(n)
&= u(W(n))\inv \cdot u(n)
\cr
\forall e\in E \quad u'(A(S(e)))\inv \cdot u'(A(F(e)))
&= u(A(S(e)))\inv \cdot u(A(F(e)))
\cr
\forall e\in E \quad u'(W(A(S(e))))\inv \cdot u'(W(A(F(e))))
&= u(W(A(S(e))))\inv \cdot u(W(A(F(e))))
}$$
Thus the each term of $DM(I', \N, u', v)$ equals the corresponding term of
$DM(I, \N, u, v)$. \qed

\subhead{4.7 The recognition problem -- definitive statement}
With the help of the theory developed so far we can now give a definitive
statement of the recognition problem, taking account of embeddings.

Given a semi-definite network $\N_0$ (representing a grammar), an embedding type
$v$ for $\N_0$, and an image $I$, the recognition problem is to construct a
definite network $\N_1$ (representing a pattern), a homomorphism
$p:\N_1\to\N_0$, and an embedding token $u$ for $\N_1$, maximising $DM(I, \N_1,
u, v\circ p)$, subject to the symmetry condition for $\N_1,u,v\circ p$.
