# Supplementary material for: A New Graph Grammar Formalism for Robust Syntactic Pattern Recognition
Source: arXiv:2504.15975 source file (2025-04-24)
Supplement: Supplementary file 5 [file supp5.tex]

\runninghead{5. Inclusion functions}

\head{5. Inclusion Functions}

\subhead{5.1 Introduction}
During recognition, when many competing grammatical possibilities are being
considered in parallel in the same pattern, some possibilities are evaluated as better than others.
That is, each symbol token $\sigma$ in the pattern has associated with it a real
number $i(\sigma) \from [0,1]$ (called an \i{inclusion value}) indicating the
algorithm's degree of confidence that $\sigma$ should be present in the final
pattern. If $i(\sigma)=1$ then the algorithm
has decided definitely to include it in the final pattern; if $i(\sigma)=0$ the
algorithm has decided definitely to prune it (but hasn't yet done so); 
intermediate values indicate
uncertainty about whether to keep it. Similarly each node token $n$ and edge token
$e$ has
an inclusion value $i(n)$ or $i(e)$ indicating the algorithm's degree of
confidence
that it should be included in the final pattern. (Hooks and facets do not need
their own inclusion values as they stand or fall with the symbol, node or edge
they belong to.)

The function $i$ is called an \i{inclusion function} and is accompanied by a
second inclusion function $j$, defined below.

By the end of the recognition process, each inclusion value have been driven to
the extremes, $0$ or $1$, and the symbols, nodes and edges with inclusion value
$0$ have all been pruned.

\subhead{5.2 Definition of inclusion functions}

\defn A pair of \i{inclusion functions} on a network $\N=\network{}$ is defined
as $(i,j)$, where $i:\Sigma\cup N \cup E \to [0,1]$ and $j:\Sigma\cup N\cup H
\cup (K\setdiff dom(G)) \to [0,1]$, such that
$$\eqalignno{
\forall \sigma\from\Sigma \quad i(\sigma)
&= j(\sigma) \ + \sum_{n\in P\preo\sigma} \hskip-3mm (1-g_n)i(n),
\qquad\text{where $g_n = \bigl|\comp{n^*\from N}{G(n^*,n)}\bigr|$} \qquad & (1)
\cr
\forall n \from N \quad i(W(n)) &= j(n) + i(n) & (2)
\cr
\forall h\from H \quad i(A(h)) &= j(h) \ + \sum_{e\in F\preo h} \hskip-3mm i(e)
\ + \sum_{e\in S\preo h} \hskip-3mm i(e) & (3)
\cr
\forall k \from K\setdiff dom(G) \quad
i(C(k)) &= j(k) + \sum_{k^* \mid G(k,k^*)} i(C(k^*)). & (4)
}$$
(This is a slightly modified version of the definition in (2004, \S7.2), taking
account of subsymbols. The summation notation in (4) means a sum
over all $k^*$ such that $G(k,k^*)$.)

This definition may be interpreted informally as follows. (In the following
explanation I shall use the future tense to state conditions that will hold 
at the end of recognition when the pattern is definite, and the present tense
for what holds during recognition when the pattern is indefinite.)

Line (1). At the end of recognition each symbol $\sigma$ will be either a \ic{bare} symbol (with $P\preo\sigma
=\emptyset$) or a part of one larger symbol (with $|P\preo\sigma| = 1$). 
Hence the nodes presently in $P\preo\sigma$ are in competition with one
another; at most one will survive to the end. $i(\sigma)$ is
interpreted as the degree of confidence in $\sigma$, $j(\sigma)$ is the degree
of confidence that $\sigma$ will be a bare symbol, and $i(n)$
is the degree of confidence in $n$. An exception to this competition is that if
$n$ is a subnode of $n^*$ (i.e., $G(n^*,n)$) then they may both be correct; 
the $1-g_n$ factor allows for this co-existence.

Line (2). $i(W(n))$ is the degree of confidence in $W(n)$, $j(n)$ is the
degree of confidence that $W(n)$ will survive to the end but $n$ will not, and
$i(n)$ is the degree of confidence in $n$.

Line (3) expresses the fact that each hook $h$ will have a single edge incident
to it (i.e., $|F\preo h| + |S\preo h| = 1$); hence the edges presently in
$F\preo h \cup S\preo h$ are in competition with one another. Thus $i(A(h))$
is the degree of confidence in the node or symbol $A(h)$, $i(e)$ is the degree
of confidence in $e$, and $j(h)$ is the degree of confidence that $A(h)$ will
survive to the end but that none of its present edges will (i.e., the correct
edge has yet to be created).

Line (4) expresses the fact that each facet $k$ that is not itself a sub-facet
will be glued to a single sub-facet. Hence if $k$ is presently glued to several
sub-facets then they are in competition with one another; $i(C(k^*))$ is the
degree of confidence in the edge $C(k^*)$, $j(k)$ is the degree of confidence
that $C(k)$ is correct but that none of $k$'s present sub-facets is.

\theorem 32. If $\N=\network{}$ is a definite network and $(i,j)$ is a pair of
inclusion functions on $\N$ satisfying $\forall x\from\Sigma\cup N \cup E\ i(x)
= 1$, then
$$ \forall\sigma\from\Sigma\ j(\sigma) =
\cases{0 & if $\sigma \in P(N)$\cr
1 & otherwise}, \quad
\forall n\from N\ j(n) = 0, \quad
\forall h\from H\ j(h) = 0, \quad
\forall k\from K\setdiff\dom(G)\ j(k) = 0. $$

\proof For any $\sigma\from\Sigma$,
$$ i(\sigma) = j(\sigma) \ + \sum_{n\in P\preo\sigma} \hskip-3mm (1-g_n)i(n) $$
where $g_n = \bigl|\comp{n^*\from N}{G(n^*,n)}\bigr|$, so
$$ 1 = j(\sigma) + |P\preo\sigma| - |G_N \circ id_{P\preo\sigma}|. $$
This implies $j(\sigma) \in \Z$, and since also $j(\sigma) \in [0,1]$ we
have $j(\sigma) \in \{0,1\}$. Now, for any $\sigma\in\Sigma$, if $\sigma\notin
P(N)$ then $P\preo\sigma=\emptyset$, which immediately gives $|P\preo\sigma| -
|G_N \circ id_{P\preo\sigma}| = 0$ and so $j(\sigma)=1$. Conversely, if
$j(\sigma) = 1$ then $|P\preo\sigma| - |G_N \circ id_{P\preo\sigma}| = 0$, so by
theorem~13(ii) (applied to $N,\Sigma,P,G_N$) $P\preo\sigma = \emptyset$, so
$\sigma\notin P(N)$. This shows that $j(\sigma) = 1$ if $\sigma \notin P(N)$ and
$j(\sigma) = 0$ if $\sigma \in P(N)$.

For any $n\from N$,
$$ i(\sigma) = j(n) + i(n) $$
and hence $j(n) = 0$.

For any $h\from H$,
$$ i(A(h)) = j(h) \ + \sum_{e\in F\preo h} \hskip-3mm i(e)
\ + \sum_{e\in S\preo h} \hskip-3mm i(e) $$
and, thanks to the sum diagram $E \buildrel F \over \rightarrow H \buildrel S
\over \leftarrow E$, there is a unique $e\from E$ such that either $F(e) = h$ or
$S(e) = h$; so $j(h) = 0$.

For any $k\from K\setdiff\dom(G)$,
$$ i(C(k)) = j(k) + \sum_{k^* \mid G(k,k^*)} i(C(k^*)). $$
By the definiteness condition $id_K = G_K \circ G_K\inv \cup G_K\inv \circ G_K$,
there exists $k^*\from K$ such that $G(k,k^*)$ (otherwise $(G_K \circ G_K\inv
\cup G_K\inv \circ G_K)(k,k)$ would not hold); moreover, this $k^*$ is unique
(for if there were a second, $k^{**}$, then $(G_K \circ G_K\inv \cup G_K\inv
\circ G_K)(k^*,k^{**})$ would hold). Thus $j(k) = 0$. \qed

\subhead{5.3 The recognition process}
With the help of the theory developed so far we can give an initial
description of the recognition process. It constructs a pattern $\N_1$, a homomorphism
$p:\N_1\to\N_0$ (where $\N_0$ is the grammar), and a pair of inclusion functions
$(i,j)$ on $\N_1$, by a sequence of structural operations on the pattern.

The recognition process must ensure that, at the end, the following conditions
hold.

\blob $\forall x\from \Sigma_1\cup N_1\cup E_1\ i(x) = 1$,

\blob $\N_1$ is definite.
