# Supplementary material for: A New Graph Grammar Formalism for Robust Syntactic Pattern Recognition
Source: arXiv:2504.15975 source file (2025-04-24)
Supplement: Supplementary file 6 [file supp6.tex]

\runninghead{6. The indefinite match function}

\head{6. The Indefinite Match Function}

\subhead{6.1 Introduction}
In section 4 we constructed the definite match function $DM$, which measures how
well a definite pattern (with an embedding token) matches the image, the grammar
and embedding type. Now we shall generalise it to the \i{indefinite match
function} $IM$, which applies to patterns that are not necessarily definite,
with inclusion functions. The affine invariance theorems of \S4.6 are generalised
to $IM$.

The recognition process attempts to maximise the value of $IM$ during
recognition, so that the final, definite pattern will maximise $DM$.

\subhead{6.2 Template matching}
The template matching function of \S4.4 is generalised as follows.

Suppose we are given a network $\N=\network{}$, an embedding token $u$ for $\N$,
a function $tem:\Sigma\to Tem$, and a pair $(i,j)$ of inclusion functions on
$\N$. The \i{(indefinite) saturation function}, $sat:\R^2\to\R$, is defined by
$$ \forall x\from\R^2\quad
sat(x) = \sum_{\sigma\in\Sigma} (1-g_\sigma) \, i(\sigma) \,
tem(\sigma)(u(\sigma)\inv(x)) $$
where $g_\sigma = \bigl|\comp{\sigma^*\from\Sigma}{G(\sigma^*,\sigma)}\bigr|$.

In the special case where the inclusion functions satisfy $\forall
\sigma\from\Sigma\ i(\sigma) = 1$, as at the end of recognition, the definition
of $sat$ reduces to the definite saturation function defined in \S4.4.

The correlation function $\rho_{I,T,sat}$ between an image $I$ and a 
template $T$ is as in \S4.4, except for using the indefinite saturation 
function,
$$\eqalign{
\rho_{I,T,sat}(g)
&= |det(\rep g)|^{1-k} \int w(sat(g(u))) \, T(u) \, (I(g(u))-I_0) \d^2u \cr
&= |\det(\rep g)|^{-k} \int w(sat(x)) \, T(g\inv(x)) \, (I(x)-I_0) \d^2x
}$$

\subhead{6.3 The indefinite match function}
The \i{indefinite match} function $IM$ measures how well a (not necessarily
definite) network $\N=\network{}$ matches an image $I$, given an embedding token
$u$ for $\N$, an embedding type $v=(sub,con,rel,\allowbreak symm, \allowbreak
tem,in)$ for $\N$, a pair of inclusion functions $(i,j)$ on $\N$, and a function
$B:\Sigma\cup H\cup (K\setdiff\dom(G))\to\closeopen{0,\infty}$. It is defined by
$$\eqalign{
& \kern-10pt IM(I, \N, u, v, i, j, B) = \cr
& \sum_{\sigma\in\Sigma}
\bigl( i(\sigma) \rho_{I,tem(\sigma),sat}(u(\sigma)) - j(\sigma) B(\sigma)
\bigr)
-\sum_{(\sigma,\sigma^*)\mid G(\sigma,\sigma^*)} \kern-15pt i(\sigma^*)
E_{sub(\sigma,\sigma^*)}(u(\sigma)\inv \cdot u(\sigma^*))
\cr&
- \sum_{n\in N} i(n) E_{con(n)}(u(W(n))\inv \cdot u(n))
- \sum_{h \in H} j(h) B(h)
- \sum_{k \in K\setdiff\dom(G)} \kern-12pt j(k) B(k)
\cr&
- \sum_{e\in E} i(e)
\bigl( E_{rel(e)}(u(A(S(e)))\inv \cdot u(A(F(e)))) +
E_{in(W(A(F(e))))}(u(W(A(S(e))))\inv \cdot u(W(A(F(e))))) \bigr)
}$$
where $sat$ is the indefinite saturation function. Observe that the $B$
function imposes a penalty for each \ic{bare} symbol, hook and facet, i.e.,
each symbol that is not a part of any other symbol ($j(\sigma)=1$), each hook
with no incident edges ($j(h)=1$), and each facet that should be glued to a
sub-facet but is not ($j(k)=1$). A function $B:\Sigma\cup H\cup
(K\setdiff\dom(G))\to\closeopen{0,\infty}$ is called a \i{bareness function}
for $\N$. The final term, $E_{in(W(A(F(e))))}(\cdots)$, has no counterpart in
$DM$; it is to penalise edges between two nodes belonging to different wholes
(see \S9.6).

The following theorem shows that $DM$ is a special case of $IM$.

\theorem 33. If

\item{(a)} $\N$ is definite,

\item{(b)} $\forall x\from\Sigma\cup N \cup E\ i(x) = 1$,

\item{(c)} $\forall\sigma\from\Sigma\setdiff P(N)\ B(\sigma)=\theta$,

\smallskip\f
then $IM(I,\N,u,v,i,j,B) = DM(I,\N,u,v)$.

\proof By theorem~32,
$$\forall\sigma\from\Sigma\ j(\sigma) =
\cases{0 & if $\sigma \in P(N)$\cr
1 & otherwise},\quad
\forall n\from N\ j(n) = 0, \quad
\forall h\from H\ j(h) = 0, \quad
\forall k\from K\setdiff\dom(G)\ j(k) = 0. $$
It follows that each term of $IM(I,\N,u,v,i,j,B)$ simplifies to the
corresponding term of $DM(I,\allowbreak\N,\allowbreak u,\allowbreak v)$ or
vanishes; in particular, for each $e\from E$, the term
$$ E_{in(W(A(F(e))))}(u(W(A(S(e))))\inv \cdot u(W(A(F(e))))) $$
vanishes since $W(A(S(e))) = W(A(F(e)))$ by the definiteness conditions. \qed

\medbreak

In the recognition process an embedding token $u$ for $\N_1$ is constructed,
along with $\N_1$ and $p$. An embedding type $v\circ p$ is induced using $p$ from
the given embedding type $v$ for $\N_0$. Throughout recognition we measure how
well $u$ matches $v\circ p$ by calculating $IM(I,\N_1,u,v\circ p,i,j,B)$, and we
seek to maximise this by continually adjusting $u$, subject to the symmetry
condition for $\N_1,u,v\circ p$.

\subhead{6.4 Invariance theorems}
I shall generalise the invariance theorems of \S4.6 from $DM$ to $IM$.

\theorem 34. (Lemma~1 of (2004, \S7.3): invariance under affine transformation
of the symbols' internal frames of reference.) For any image $I$, network $\N$,
embedding tokens $u,u'$ for $\N$, embedding type $v$ for $\N$, inclusion
functions $i,j$ on $\N$, and bareness function $B$ for $\N$,
$$ IM(I, \N, u\cdot u', v\cdot u', i, j, B) = IM(I, \N, u, v, i, j, B), $$
provided $u' \circ W \circ A \circ F = u' \circ W \circ A \circ S$.

\proof As in theorem~28, each term of $IM(I, \N, u\cdot u', v\cdot u', i,
j, B)$ equals the corresponding term of $IM(I, \N, u, v, i, j, B)$. \qed

\theorem 35. (Invariance of the match functions under a local symmetry.) Given
an image $I$, a semi-definite network $\N_0$, a network $\N_1$, a homomorphism
$p:\N_1\to\N_0$, an embedding token $u$ for $\N_1$, an embedding type $v$ for
$\N_0$, and a local symmetry $\pi$ of $\N_1$ with respect to $\N_0,p,v$, the
application of $\pi$ to $p,u$ produces a homomorphism $p':\N_1\to\N_0$ and an
embedding token $u'$ for $\N_1$.

(i) For any inclusion functions $i,j$ and bareness function $B$ for $\N_1$,
$IM(I, \N_1, u', v\circ p', i, j, B) \allowbreak = IM(I, \N_1, u, v\circ p, i,
j, B)$.

(ii) The symmetry condition holds for $\N_1,u',v \circ p'$ iff it holds for
$\N_1,u,v \circ p$.

\proof The argument of theorem~29 generalises:
$$\eqqalign\quad{
IM(I,\N_1,u',v \circ p',i,j,B)
&= IM(I,\N_1,u \cdot s', (v \circ p) \cdot s',i,j,B)
&\text{since $v \circ p' = (v \circ p) \cdot s'$}\cr
&= IM(I,\N_1,u,v \circ p,i,j,B)
&\text{by theorem~34.}\cr
}$$
To justify this use of theorem~34 we must check that $s' \circ W_1 \circ A_1
\circ F_1 = s' \circ W_1 \circ A_1 \circ S_1$. For any $e\from E_1$,
$$\eqqalign\quad{
s'(W_1(A_1(F_1(e))))
&= s(W_1(A_1(F_1(e))))(p(W_1(A_1(F_1(e)))))
&\cr
&= s(W_1(A_1(F_1(e))))(W_0(A_0(F_0(p(e)))))
&\text{since $p$ is a homomorphism}\cr
&= s(W_1(A_1(F_1(e))))(W_0(A_0(S_0(p(e)))))
&\text{since $\N_0$ is semi-definite}\cr
&= s(W_1(A_1(S_1(e))))(W_0(A_0(S_0(p(e)))))
&\text{since $\pi$ is a local symmetry}\cr
&= s(W_1(A_1(S_1(e))))(p(W_1(A_1(S_1(e)))))
&\text{since $p$ is a homomorphism}\cr
&= s'(W_1(A_1(S_1(e))))
&\cr
}$$
as required.

For part (ii), the proof in theorem~29 applies (it does not require $\N_1$ to be
definite). \qed

\theorem 36. (Affine invariance of the $\rho$ function.) For any template $T$,
any image $I$, and any affine transformations $g,g'$,
$$ \rho_{I\circ g\inv,T,sat\circ g\inv}(g\cdot g')
= |\det(\rep g)|^{1-k} \, \rho_{I,T,sat}(g').
$$

\medskip\f
(Recall that $\overline g$ is the matrix representation of $g$.)

\proof This is identical to theorem~30, except using the indefinite saturation
function. The same proof applies. \qed

\theorem 37. (Affine invariance of $IM$.) For any affine $g$ such that
$|det(\overline g)|=1$, any image $I$, any network $\N=\network{}$, any
embedding token $u$ for $\N$, and any embedding type $v$ for $\N$, define a new,
affine-transformed image $I' = I \circ g\inv$, and a new, affine-transformed
embedding token $u'$ for $\N$ by $\forall x\from\Sigma\cup N\ u'(x) = g \cdot
u(x)$.

For any inclusion functions $i,j$ and bareness function $B$ for $\N$,
$$ IM(I', \N, u', v, i, j, B) = IM(I, \N, u, v, i, j, B). $$
(The condition $|det(\overline g)|=1$ may be dropped if $k=1$.)

\proof Let $sat$ be the indefinite saturation function calculated using the
embedding token $u$.

As in the proof of theorem~31, each term of $IM(I', \N, u', v, i, j, B)$ equals
the corresponding term of $IM(I, \N, u, v, \allowbreak i, \allowbreak j,
\allowbreak B)$. \qed

\subhead{6.5 Adjustment of the embedding token}
During recognition the embeddings of all the symbols and nodes are continually
adjusted to maximise $IM(I, \N_1, u, v\circ p, i, j, B)$ (subject to the
symmetry condition). This is done by a process of gradient ascent, as defined in
(2004, \S\S7.6--7.8), but with the calculation of the derivative of the match
function in \S7.6 augmented to allow for the new terms in the match function. To
be precise, theorem~3 of \S7.6 is amended as follows. We make a small
change in the embedding token from $u$ to $u \cdot \Delta u$, where
$$\eqalign{
\forall\sigma\from\Sigma\ \ \Delta u(\sigma) &= \exp(\epsilon V_\sigma) \cr
\forall n\from N\ \ \Delta u(n) &= \exp(\epsilon V_n) \cr
}$$
where the increments $V_\sigma,V_n \in \A$ are linked by the symmetry
condition; then the value of $IM$ changes to
$$ IM(I, \N, u \cdot \Delta u, v, i, j, B) =
IM(I, \N, u, v, i, j, B) +
\epsilon \sum_{\sigma\in\Sigma} F_\sigma(V_\sigma) + o(\epsilon) $$
where, for each $\sigma\from\Sigma$,
$$\eqalign{
&F_\sigma = F^0_\sigma + F^1_\sigma + F^2_\sigma + F^3_\sigma + F^4_\sigma \cr
&F^0_\sigma, F^1_\sigma, F^2_\sigma, F^3_\sigma \text{ are as before} \cr
&F^4_\sigma = -\sum_{\sigma^*|G(\sigma,\sigma^*)}
Ad(Sub_{\sigma,\sigma^*}\inv)\adj(F_{\sigma,\sigma^*}) +
\sum_{\sigma^*|G(\sigma^*,\sigma)} F_{\sigma^*,\sigma}
}$$
and, for each $\sigma,\sigma^*\from\Sigma$ such that $G(\sigma,\sigma^*)$,
$$\eqalign{
F_{\sigma,\sigma^*} &= -i(\sigma^*)
E_{sub(\sigma,\sigma^*)*}(Sub_{\sigma,\sigma^*}) \cr
Sub_{\sigma,\sigma^*} &= u(\sigma)\inv \cdot u(\sigma^*).
}$$
The theorem is proved by the same methods as before.

\subhead{6.6 The recognition process}
During the recognition process $IM(I, \N_1, u, v\circ p, i, j, B)$ is 
maximised, and at the end the conditions of theorem~33
are satisfied, so $DM(I, \N_1, u, v\circ p)$ is maximised.
