# Supplementary material for: A New Graph Grammar Formalism for Robust Syntactic Pattern Recognition
Source: arXiv:2504.15975 source file (2025-04-24)
Supplement: Supplementary file 8 [file supp8.tex]

\runninghead{8. The structural operations}

\head{8. The Structural Operations}

\subhead{8.1 Introduction}
In this section I shall define the \i{structural operations} by which the pattern
is incrementally grown during recognition. There are four kinds:

\blob pruning operations,

\blob extension operations,

\blob merging two symbol tokens,

\blob partitioning a symbol token into two.

\subhead{8.2 Pruning operations}

\defn Given a network $\N=\network{}$ and a pair $(i,j)$ of inclusion
functions on $\N$, a \i{pruning operation} is a transformation from $\N$ to a
subnetwork $\N'=\network{'}$ such that
$$ \forall \sigma\from\Sigma\setdiff\Sigma'\ i(\sigma) = 0, \quad
\forall n\from N\setdiff N'\ i(n) = 0, \quad \forall e\from E\setdiff E'\ i(e)
= 0. $$
A pruning operation is \i{trivial} iff $\N'=\N$.

\theorem 38. For any pruning operation from $\N$ to $\N'$, given a
pair $(i,j)$ of inclusion functions on $\N$,

\item{(i)} $\forall \sigma\from\Sigma\setdiff\Sigma' \ j(\sigma) = 0, \quad
\forall h\from H\setdiff H'\ j(h) = 0, \quad
\forall k\from (K\setdiff\dom(G))\setdiff (K'\setdiff\dom(G'))\ j(k) = 0$,

\item{(ii)} $(i|_{\Sigma'\cup N'\cup E'}, j|_{\Sigma'\cup N'\cup H'\cup
(K'\setdiff\dom(G'))})$ is a pair of inclusion functions on $\N'$ (called the
\i{restriction of $(i,j)$ to $\N'$}).

\proof (i) For any $\sigma\from\Sigma\setdiff\Sigma'$,
$$ i(\sigma) = j(\sigma) \ + \sum_{n\in P\preo\sigma} \hskip-3mm (1-g_n)i(n) $$
where $i(\sigma)=0$; moreover, the condition $P(N') \subseteq \Sigma'$ implies
that each $n\from P\preo\sigma$ is in $N\setdiff N'$ and so $i(n)=0$. Hence
$j(\sigma)=0$.

For any $h\from H\setdiff H'$, we have $h \notin H'=A\pre{N'\cup\Sigma'}$, so
$A(h) \notin N'\cup\Sigma'$, which means $A(h) \in N\setdiff N' \ \cup\
\Sigma\setdiff\Sigma'$, so $i(A(h)) = 0$. By the condition
$$ i(A(h)) = j(h) \ + \sum_{e\in F\preo h} \hskip-3mm i(e) \ +
\sum_{e\in S\preo h} \hskip-3mm i(e) $$
this implies $j(h) = 0$.

For any $k\from (K\setdiff\dom(G))\setdiff (K'\setdiff\dom(G'))$, since
$\dom(G') \subseteq \dom(G)$ we have $k \notin K'=C\pre{E'}$, so $C(k) \in
E\setdiff E'$, so $i(C(k)) = 0$. By the condition
$$ i(C(k)) = j(k) + \sum_{k^* \mid G(k,k^*)} i(C(k^*)) $$
this implies $j(k) = 0$.

(ii) Define $i'=i|_{\Sigma'\cup N'\cup E'}$, $j'=j|_{\Sigma'\cup N'\cup H'\cup
(K'\setdiff\dom(G'))}$, and $I = id_{\Sigma'\cup N'\cup H' \cup E' \cup K'}$.
The condition
$$\forall \sigma\from\Sigma \quad i(\sigma)
= j(\sigma) \ + \sum_{n\in P\preo\sigma} \hskip-3mm (1-g_n)i(n) $$
implies the same condition for $(i',j')$ on $\N'$. We need to check that the
value of $g_n$ is the same in both cases, i.e., $\bigl|\comp{n^*\from
N'}{G'(n^*,n)}\bigr|=\bigl|\comp{n^*\from N}{G(n^*,n)}\bigr|$ for every $n\from
N'$. In fact, for any $n\from N'$, using $G' = G \circ I$,
$$ \bigl|\comp{n^*\from N'}{G'(n^*,n)}\bigr| = |G' \circ id_{\{n\}}|
= |G \circ I \circ id_{\{n\}}|
= |G \circ id_{\{n\}}|
= \bigl|\comp{n^*\from N}{G(n^*,n)}\bigr| $$
as required. Moreover, $\sum_{n\in P\preo\sigma} (1-g_n)i(n) = \sum_{n\in
P'{}\preo\sigma} (1-g_n)i'(n)$, since the right-hand side merely omits terms
$(1-g_n)i(n)$ for which $i(n)=0$.

Secondly, the condition
$$ \forall n \from N \quad i(W(n)) = j(n) + i(n) $$
implies the same condition for $(i',j')$ on $\N'$.

Thirdly, the condition
$$ \forall h\from H \quad i(A(h)) = j(h) \ +
\sum_{e\in F\preo h} \hskip-3mm i(e)
\ + \sum_{e\in S\preo h} \hskip-3mm i(e) $$
implies the same condition for $(i',j')$ on $\N'$. We have $\sum_{e\in F\preo h}
i(e) = \sum_{e\in F'{}\preo h} i'(e)$, since the right-hand side merely omits
terms $i(e)$ that are equal to $0$; and similarly $\sum_{e\in S\preo h} i(e) =
\sum_{e\in S'{}\preo h} i'(e)$.

Fourthly, the condition
$$ \forall k \from K\setdiff dom(G) \quad
i(C(k)) = j(k) + \sum_{k^* \mid G(k,k^*)} i(C(k^*)) $$
implies the same condition for $(i',j')$ on $\N'$. For any $k\from
K'\setdiff\dom(G')$, we have $k \in K\setdiff dom(G)$ by theorem~24(iii), so
$i(C(k)) = j(k) + \sum_{k^* \mid G(k,k^*)} i(C(k^*))$. Also,
$$ \comp{k^*}{G'(k,k^*)} = \comp{k^*}{G(k,k^*) \wedge k^* \in K'}
= \comp{k^*}{G(k,k^*) \wedge C(k^*) \in E'} $$
by $G' = G \circ I$. Thus $\comp{k^*}{G'(k,k^*)} \subseteq
\comp{k^*}{G(k,k^*)}$, and any $k^*$ in the latter set but not in the former has
$C(k^*) \notin E'$ and so $i(C(k^*))=0$. This shows that $\sum_{k^* \mid
G'(k,k^*)} i'(C'(k^*)) = \sum_{k^* \mid G(k,k^*)} i(C(k^*))$.

This completes the verification that $(i',j')$ is a pair of inclusion functions
on $\N'$. \qed

\medskip\f
In practice we may confine ourselves to elementary pruning operations,
involving removal of a single symbol, node or edge.

\defn Given a network $\N=\network{}$ and a pair of inclusion functions $(i,j)$
on $\N$, an \i{elementary pruning operation} is one of the following operations.

\medskip

\item{(i)} \i{Pruning a symbol $\sigma\from\Sigma$} transforms $\N$ to
$\N'=\network{'}$, where

$\Sigma' = \Sigma \setdiff \bigl( \{\sigma\} \cup
\comp{\sigma^*}{G(\sigma,\sigma^*)} \bigr)$, \quad $N' = W\pre{\Sigma'} \cap
P\pre{\Sigma'}$, \quad $H' = A\pre{N' \cup \Sigma'}$,

$E' = F\pre{H'} \cap S\pre{H'}$, \quad $K' = C\pre{E'}$,

$W' = W|_{N'\cup\Sigma'}$, \quad $P' = P|_{N'}$, \quad $A' = A|_{H'}$, \quad $F'
= F|_{E'}$, \quad $S' = S|_{E'}$, \quad $C' = C|_{K'}$,

$G' = id_{\Sigma'\cup N'\cup H'\cup E'\cup K'} \circ G \circ id_{\Sigma'\cup
N'\cup H'\cup E'\cup K'}$.

\item{} This operation is permitted provided
$\forall\sigma^*\from\Sigma\setdiff\Sigma'\ i(\sigma^*)=0$ and $\forall n\from
P\pre{\Sigma\setdiff\Sigma'}\ i(n)=0$.

\medskip

\item{(ii)} \i{Pruning a node $n\from N$} transforms $\N$ to $\N'=\network{'}$,
where

$\Sigma' = \Sigma$, \quad $N' = N \setdiff \bigl( \{n\} \cup
\comp{n^*}{G(n,n^*)} \bigr)$, \quad $H' = A\pre{N' \cup \Sigma'}$,

$E' = F\pre{H'} \cap S\pre{H'}$, \quad $K' = C\pre{E'}$,

$W' = W|_{N'\cup\Sigma'}$, \quad $P' = P|_{N'}$, \quad $A' = A|_{H'}$, \quad $F'
= F|_{E'}$, \quad $S' = S|_{E'}$, \quad $C' = C|_{K'}$,

$G' = id_{\Sigma'\cup N'\cup H'\cup E'\cup K'} \circ G \circ id_{\Sigma'\cup
N'\cup H'\cup E'\cup K'}$.

\item{} This operation is permitted provided $\forall n^*\from N\setdiff N'\
i(n^*)=0$.

\medskip

\item{(iii)} \i{Pruning an edge $e\from E$} transforms $\N$ to
$\N'=\network{'}$, where

$\Sigma' = \Sigma$, \quad $N' = N$, \quad $H' = H$, \quad $E' = E \setdiff
\bigl( \{e\} \cup \comp{e^*}{G(e,e^*)} \bigr)$, \quad $K' = C\pre{E'}$,

$W' = W$, \quad $P' = P$, \quad $A' = A$, \quad $F' = F|_{E'}$, \quad $S' =
S|_{E'}$, \quad $C' = C|_{K'}$,

$G' = id_{\Sigma'\cup N'\cup H'\cup E'\cup K'} \circ G \circ id_{\Sigma'\cup
N'\cup H'\cup E'\cup K'}$.

\item{} This operation is permitted provided $\forall e^*\from E\setdiff E'\
i(e^*)=0$.

\theorem 39. All elementary pruning operations are pruning operations.

\proof Let the network be $\N=\network{}$ and the inclusion functions be $i,j$.

(i) Consider pruning a symbol $\sigma\from\Sigma$, producing $\N'=\network{'}$.
We must show that $\N'$ is a subnetwork of $\N$. The only condition that is not
obvious is $G \circ id_{\Sigma'\cup N'\cup H'\cup E'\cup K'} \subseteq
id_{\Sigma'\cup N'\cup H'\cup E'\cup K'} \circ G$. This is proved in five parts.

First, $G \circ id_{\Sigma'} \subseteq id_{\Sigma'} \circ G$ is verified as
follows. For any $\sigma_1,\sigma_2\from\Sigma$, if $(G \circ
id_{\Sigma'})(\sigma_1,\sigma_2)$ then $G(\sigma_1,\sigma_2)$ and $\sigma_2 \in
\Sigma'$, so $\sigma_2 \ne \sigma$ and $G(\sigma,\sigma_2)$ does not hold. This
implies that $\sigma_1 \ne \sigma$ and $G(\sigma,\sigma_1)$ does not hold (by $G
\circ G = \bot$). This gives $\sigma_1 \in \Sigma'$, and hence $(id_{\Sigma'}
\circ G)(\sigma_1,\sigma_2)$, as required.

The condition $G \circ id_{N'} \subseteq id_{N'} \circ G$ is verified as
follows.
$$\eqqalign\quad{
G \circ id_{N'}
&= G \circ id_N \circ id_{N'}
= id_N \circ G \circ id_{N'}
\subseteq id_{N\cup\Sigma} \circ G \circ id_{N'} \kern-80pt
&\cr
&\subseteq \overline W\inv \circ G \circ \overline W \circ id_{N'}
&\text{from $\overline W \circ G \subseteq G \circ \overline W$ by
theorem~2(iv)}\cr
&\subseteq \overline W\inv \circ G \circ id_{\Sigma'} \circ \overline W
&\text{since $N' \subseteq W\pre{\Sigma'}$}\cr
&\subseteq \overline W\inv \circ id_{\Sigma'} \circ G \circ \overline W
&\text{since $G \circ id_{\Sigma'} \subseteq id_{\Sigma'} \circ G$}\cr
&= id_{W\pre{\Sigma'}} \circ \overline W\inv \circ G \circ \overline W
&\cr
}$$
so by theorem~4(vi)
$$ G \circ id_{N'} \subseteq id_{W\pre{\Sigma'}} \circ G $$
and similarly
$$ G \circ id_{N'} \subseteq id_{P\pre{\Sigma'}} \circ G $$
so
$$\eqqalign\quad{
G \circ id_{N'}
&\subseteq id_{W\pre{\Sigma'}} \circ G \ \cap\ id_{P\pre{\Sigma'}} \circ G
&\cr
&= id_{W\pre{\Sigma'}} \circ (G \cap id_{P\pre{\Sigma'}} \circ G)
&\text{by theorem~4(iv)}\cr
&= id_{W\pre{\Sigma'}} \circ id_{P\pre{\Sigma'}} \circ (G \cap G)
&\text{by theorem~4(iv)}\cr
&= id_{N'} \circ G.
&\cr
}$$

The condition $G \circ id_{H'} \subseteq id_{H'} \circ G$ is verified as
follows.
$$\eqqalign\quad{
G \circ id_{H'}
&= G \circ id_H \circ id_{H'}
= id_H \circ G \circ id_{H'} \kern-40pt
&\cr
&\subseteq \overline A\inv \circ G \circ \overline A \circ id_{H'}
&\text{from $\overline A \circ G \subseteq G \circ \overline A$ by
theorem~2(iv)}\cr
&= \overline A\inv \circ G \circ id_{N'\cup\Sigma'} \circ \overline A
&\text{since $H' = A\pre{N'\cup\Sigma'}$}\cr
&\subseteq \overline A\inv \circ id_{N'\cup\Sigma'} \circ G \circ \overline A
&\text{since $G \circ id_{\Sigma'} \subseteq id_{\Sigma'} \circ G$ and
$G \circ id_{N'} \subseteq id_{N'} \circ G$}\cr
&= id_{H'} \circ \overline A\inv \circ G \circ \overline A
&\text{since $H' = A\pre{N'\cup\Sigma'}$}\cr
}$$
so by theorem~4(vi)
$$ G \circ id_{H'} \subseteq id_{H'} \circ G. $$

The condition $G \circ id_{E'} \subseteq id_{E'} \circ G$ is verified as
follows.
$$\eqqalign\quad{
G \circ id_{E'}
&= G \circ id_E \circ id_{E'}
= id_E \circ G \circ id_{E'} \kern-40pt
&\cr
&\subseteq \overline F\inv \circ G \circ \overline F \circ id_{E'}
&\text{from $\overline F \circ G \subseteq G \circ \overline F$ by
theorem~2(iv)}\cr
&\subseteq \overline F\inv \circ G \circ id_{H'} \circ \overline F
&\text{since $E' \subseteq F\pre{H'}$}\cr
&\subseteq \overline F\inv \circ id_{H'} \circ G \circ \overline F
&\text{since $G \circ id_{H'} \subseteq id_{H'} \circ G$}\cr
&= id_{F\pre{H'}} \circ \overline F\inv \circ G \circ \overline F
&\cr
}$$
so by theorem~4(vi)
$$ G \circ id_{E'} \subseteq id_{F\pre{H'}} \circ G $$
and similarly
$$ G \circ id_{E'} \subseteq id_{S\pre{H'}} \circ G $$
so
$$\eqqalign\quad{
G \circ id_{E'}
&\subseteq id_{F\pre{H'}} \circ G \ \cap\ id_{S\pre{H'}} \circ G
&\cr
&= id_{F\pre{H'}} \circ (G \cap id_{S\pre{H'}} \circ G)
&\text{by theorem~4(iv)}\cr
&= id_{F\pre{H'}} \circ id_{S\pre{H'}} \circ (G \cap G)
&\text{by theorem~4(iv)}\cr
&= id_{E'} \circ G.
&\cr
}$$

Finally, the condition $G \circ id_{K'} \subseteq id_{K'} \circ G$ is verified
as follows.
$$\eqqalign\quad{
G \circ id_{K'}
&= G \circ id_K \circ id_{K'}
= id_K \circ G \circ id_{K'} \kern-40pt
&\cr
&\subseteq \overline C\inv \circ G \circ \overline C \circ id_{K'}
&\text{from $\overline C \circ G \subseteq G \circ \overline C$ by
theorem~2(iv)}\cr
&= \overline C\inv \circ G \circ id_{E'} \circ \overline C
&\text{since $K' = C\pre{E'}$}\cr
&\subseteq \overline C\inv \circ id_{E'} \circ G \circ \overline C
&\text{since $G \circ id_{E'} \subseteq id_{E'} \circ G$}\cr
&= id_{K'} \circ \overline C\inv \circ G \circ \overline C
&\text{since $K' = C\pre{E'}$}\cr
}$$
so by theorem~4(vi)
$$ G \circ id_{K'} \subseteq id_{K'} \circ G. $$
It follows then that $G \circ id_{\Sigma'\cup N'\cup H'\cup E'\cup K'} \subseteq
id_{\Sigma'\cup N'\cup H'\cup E'\cup K'} \circ G$ and hence $\N'$ is a
subnetwork of $\N$.

We also need to verify the conditions on the inclusion functions for a pruning
operation.

The first condition, $\forall\sigma^*\from\Sigma\setdiff\Sigma'\ i(\sigma^*)=0$,
is given.

The second condition, $\forall n\from N\setdiff N'\ i(n)=0$, is verified as
follows. For any $n\from N\setdiff N'$, we have $n \notin W\pre{\Sigma'}$ or
$n\notin P\pre{\Sigma'}$. In the former case, $W(n) \in \Sigma\setdiff\Sigma'$,
so $i(W(n))=0$, so, by the constraint $i(W(n)) = j(n) + i(n)$, we have $i(n)=0$
as required. In the latter case, $n \in P\pre{\Sigma\setdiff\Sigma'}$, so we are
given that $i(n)=0$ as required.

The third condition, $\forall e\from E\setdiff E'\ i(e)=0$, is verified as
follows. For any $e\from E\setdiff E'$, we have $e \notin F\pre{H'}$ or $e
\notin S\pre{H'}$. In the former case, $F(e) \notin H'$, so $A(F(e)) \notin N'
\cup \Sigma'$, so $i(A(F(e)))=0$. Hence by the constraint $\forall h\from H\
i(A(h)) = j(h) \ + \sum_{e\in F\preo h} i(e) \ + \sum_{e\in S\preo h} i(e)$ it
follows that $i(e)=0$ as required. The latter case is similar.

This completes the proof that pruning $\sigma$ is a pruning operation.

(ii) Consider pruning a node $n\from N$, producing $\N'=\network{'}$. The
verification that $\N'$ is a subnetwork of $\N$ is similar to the one in part
(i), but simpler. We also need to verify the conditions on the inclusion
functions for a pruning operation.

The first condition, $\forall\sigma\from\Sigma\setdiff\Sigma'\ i(\sigma)=0$, is
vacuously true because $\Sigma'=\Sigma$.

The second condition, $\forall n^*\from N\setdiff N'\ i(n^*)=0$, is given.

The third condition, $\forall e\from E\setdiff E'\ i(e)=0$, is verified exactly
as in part (i).

(iii) Consider pruning an edge $e\from E$, producing $\N'=\network{'}$. The
verification that $\N'$ is a subnetwork of $\N$ is similar to the one in part
(i), but simpler. We also need to verify the conditions on the inclusion
functions for a pruning operation.

The first two conditions, $\forall\sigma\from\Sigma\setdiff\Sigma'\ i(\sigma)=0$
and $\forall n\from N\setdiff N'\ i(n)=0$, are vacuously true because
$\Sigma'=\Sigma$ and $N'=N$.

The third condition, $\forall e^*\from E\setdiff E'\ i(e^*)=0$, is given. \qed

\medskip\f
The following theorem shows why it is sufficient to restrict attention to
elementary pruning operations.

\theorem 40. If any non-trivial pruning operation is possible on a network
then an elementary pruning operation is possible on it.

\proof Consider a network $\N=\network{}$ with inclusion functions $i,j$ and
suppose that a non-trivial pruning operation is possible on it, producing a
proper subnetwork $\N'=\network{'}$. Then there exists
$\sigma\from\Sigma\setdiff\Sigma'$ or $n\from N\setdiff N'$ or $h\from H\setdiff
H'$ or $e\from E\setdiff E'$ or $k\from K\setdiff K'$. However, note that if
$h\from H\setdiff H'$ then $A(h) \in N\setdiff N' \cup \Sigma\setdiff\Sigma'$,
since $H'=A\pre{N'\cup\Sigma'}$; and if $k\in K\setdiff K'$ then $C(k) \in
E\setdiff E'$ since $K'=C\pre{E'}$. So we can infer that there exists
$\sigma\from\Sigma\setdiff\Sigma'$ or $n\from N\setdiff N'$ or $e\from E\setdiff
E'$.

Consider the case where there exists $\sigma\from\Sigma\setdiff\Sigma'$. Then
$\forall\sigma^*\from\Sigma\ (G(\sigma,\sigma^*) \Rightarrow \sigma^* \in
\Sigma\setdiff\Sigma')$, by the condition $G \circ id_{\Sigma'\cup N'\cup H'\cup
E'\cup K'} \subseteq id_{\Sigma'\cup N'\cup H'\cup E'\cup K'} \circ G$. Defining
a set $\Sigma_0=\{\sigma\} \cup \comp{\sigma^*}{G(\sigma,\sigma^*)}$, we then
have $\Sigma_0 \subseteq \Sigma\setdiff\Sigma'$, so
$\forall\sigma^*\from\Sigma_0\ i(\sigma^*)=0$; moreover the condition
$P(N')\subseteq \Sigma'$ implies $P\pre{\Sigma_0} \subseteq N\setdiff N'$ and
hence $\forall n\from P\pre{\Sigma_0}\ i(n)=0$. Hence we can perform on $\N$ the
elementary pruning operation of pruning $\sigma$, giving a subnetwork
$\N''=\network{''}$, with $\Sigma''=\Sigma\setdiff\Sigma_0$.

Next consider the case where there exists $n\from N\setdiff N'$. Then $\forall
n^*\from N\ (G(n,n^*) \Rightarrow n^* \in N\setdiff N')$, by the condition $G
\circ id_{\Sigma'\cup N'\cup H'\cup E'\cup K'} \subseteq id_{\Sigma'\cup N'\cup
H'\cup E'\cup K'} \circ G$. Defining a set $N_0=\{n\} \cup
\comp{n^*}{G(n,n^*)}$, we then have $N_0 \subseteq N\setdiff N'$, so $\forall
n^*\from N_0\ i(n^*)=0$. Hence we can perform on $\N$ the elementary pruning
operation of pruning $n$, giving a subnetwork $\N''=\network{''}$, with
$N''=N\setdiff N_0$.

Finally consider the case where there exists $e\from E\setdiff E'$. Then
$\forall e^*\from E\ (G(e,e^*) \Rightarrow e^* \in E\setdiff E')$, by the
condition $G \circ id_{\Sigma'\cup N'\cup H'\cup E'\cup K'} \subseteq
id_{\Sigma'\cup N'\cup H'\cup E'\cup K'} \circ G$. Defining a set $E_0=\{e\}
\cup \comp{e^*}{G(e,e^*)}$, we then have $E_0 \subseteq E\setdiff E'$, so
$\forall e^*\from E_0\ i(e^*)=0$. Hence we can perform on $\N$ the elementary
pruning operation of pruning $e$, giving a subnetwork $\N''=\network{''}$, with
$E''=E\setdiff E_0$.

Hence in all cases an elementary pruning operation is possible. \qed

\theorem 41. If a pruning operation is carried out on a network $\N$, given a
pair of inclusion functions $(i,j)$ on $\N$, resulting in a subnetwork $\N'$,
then, for any image $I$ and any embedding token $u$, embedding type $v$ and
bareness function $B$ for $\N$,
$$ IM(I, \N', u', v', i', j', B') = IM(I, \N, u, v, i, j, B) $$
where $u',v',i',j',B'$ are the restrictions of $u,v,i,j,B$ to $\N'$. Moreover,
the symmetry condition holds for $\N',u',v'$ if it holds for $\N,u,v$.

\proof We use the usual notation, $\N=\network{}$, $\N'=\network{'}$,
$v=(sub,\allowbreak con,\allowbreak rel,\allowbreak symm,\allowbreak tem,
\allowbreak in)$, $v'=(sub',\allowbreak con',\allowbreak rel',\allowbreak
symm',\allowbreak tem', \allowbreak in')$. By the definition of a pruning
operation and theorem~38(i),
$$\eqalign{
&\forall\sigma\from\Sigma\setdiff\Sigma'\ i(\sigma) = 0 = j(\sigma), \quad
\forall n\from N\setdiff N'\ i(n) = 0, \quad
\forall h\from H\setdiff H'\ j(h) = 0,
\cr&
\forall e\from E\setdiff E'\ i(e) = 0, \quad
\forall k\from (K\setdiff\dom(G))\setdiff (K'\setdiff\dom(G'))\ j(k) = 0.
}$$
This implies that the pruning operation makes no difference to the value of
$IM$. The only term for which this is not obvious is
$\sum_{(\sigma,\sigma^*)\mid G(\sigma,\sigma^*)} i(\sigma^*)
E_{sub(\sigma,\sigma^*)}(u(\sigma)\inv \cdot u(\sigma^*))$. Since $G'_\Sigma =
G_\Sigma \circ id_{\Sigma'}$ (by theorem~24(i)), the difference
$$ \sum_{(\sigma,\sigma^*)\mid G(\sigma,\sigma^*)} i(\sigma^*)
E_{sub(\sigma,\sigma^*)}(u(\sigma)\inv \cdot u(\sigma^*))
\ - \sum_{(\sigma,\sigma^*)\mid G'(\sigma,\sigma^*)} i'(\sigma^*)
E_{sub'(\sigma,\sigma^*)}(u'(\sigma)\inv \cdot u'(\sigma^*)) $$
is the sum of $i(\sigma^*) E_{sub(\sigma,\sigma^*)}(u(\sigma)\inv \cdot
u(\sigma^*))$ over pairs $(\sigma,\sigma^*)$ having $\sigma^* \in
\Sigma\setdiff\Sigma'$, and for such pairs the term vanishes since $i(\sigma^*)
= 0$.

The symmetry condition for $\N',u',v'$ immediately follows from the one for
$\N,u,v$.\qed

\medbreak\f
Pruning is used in the recognition process as follows. We have a pattern
$\N_1$, a parse $p:\N_1\to\N_0$, an embedding token $u$ for $\N_1$, and a pair
of inclusion functions $(i,j)$ on $\N_1$. We carry out an elementary pruning
operation on $\N_1$ to give a subnetwork $\N_1'$, with a new parse
$p|_{\N_1'}:\N_1'\to\N_0$ (\S3.7), a new embedding token $u|_{\N_1'}$ (\S4.2),
and a new pair of inclusion functions, the restriction of $(i,j)$ to $\N_1'$
(theorem~38(ii)).

\subhead{8.3 Unprunability and its consequences}

\defn A network $\N=\network{}$ is \i{unprunable}, given a pair of
inclusion functions $(i,j)$ on $\N$, iff there is no proper subnetwork
$\N'=\network{'}$ of $\N$ satisfying
$$ \forall \sigma\from\Sigma\setdiff\Sigma'\ i(\sigma) = 0, \quad
\forall n\from N\setdiff N'\ i(n) = 0, \quad
\forall e\from E\setdiff E'\ i(e) = 0. $$

\medskip\f
(In other words, a network is unprunable iff no non-trivial pruning operation is
possible on it, or, equivalently by theorem~40, iff no elementary pruning
operation is possible on it.)

\theorem 42. If

\item{(a)} $\N_1=\network{_1}$ is a network,

\item{(b)} $p:\N_1\to\N_0$ is a homomorphism, where $\N_0$ is a semi-definite
network,

\item{(c)} $(i,j)$ is a pair of inclusion functions on $\N_1$ satisfying
$\forall x\from \Sigma_1 \cup N_1 \cup E_1 \ i(x) \in \{0, 1\}$,

\item{(d)} $\N_1$ is unprunable, given $(i,j)$,

\smallskip\f
then $\forall e\from E_1\ i(e) = 1$.

\proof Consider the pruning operation that transforms $\N_1$ to
$\N_2=\network{_2}$, where

$\Sigma_2 = \Sigma_1, \quad N_2 = N_1, \quad H_2 = H_1, \quad E_2 = \comp{e\from
E_1}{i(e)=1}, \quad K_2 = C_1\pre{E_2},$

$W_2 = W_1, \quad P_2 = P_1, \quad A_2 = A_1, \quad F_2 = F_1|_{E_2}, \quad S_2
= S_1|_{E_2}, \quad C_2 = C_1|_{K_2},$

$G_2 = id_{\Sigma_2\cup N_2\cup H_2\cup E_2\cup K_2} \circ G_1 \circ
id_{\Sigma_2\cup N_2\cup H_2\cup E_2\cup K_2}$.

\smallskip\f
I shall show that this is indeed a pruning operation, and then since $\N_1$ is
assumed unprunable it will follow that $\N_2=\N_1$.

First we check that $\N_2$ is a subnetwork of $\N_1$. The conditions
$$ W_1(N_2) \subseteq \Sigma_2, \quad P_1(N_2) \subseteq \Sigma_2, \quad
H_2 = A_1\pre{N_2\cup\Sigma_2}, \quad F_1(E_2) \subseteq H_2, \quad
S_1(E_2) \subseteq H_2 $$
are immediate, since $\Sigma_2=\Sigma_1$, $N_2=N_1$ and $H_2=H_1$. The condition
$K_2 = C_1\pre{E_2}$ holds by definition.

The functions $W_2,P_2,A_2,F_2,S_2,C_2$ are as they ought to be for a
subnetwork.

To verify $G_1 \circ id_{\Sigma_2\cup N_2\cup H_2\cup E_2 \cup K_2} \subseteq
id_{\Sigma_2\cup N_2\cup H_2\cup E_2\cup K_2} \circ G_1$ we need the following
derivations.

For every $k,k^*\from K_1$ such that $G_1(k,k^*)$, we have $k \in \ran(G_1)$, so
$k \notin \dom(G_1)$, so
$$ i(C_1(k)) = j(k) + \sum_{k'|G_1(k,k')} i(C_1(k')) \ge i(C_1(k^*)); $$
thus if $k^* \in K_2$ then $C_1(k^*) \in E_2$, so $i(C_1(k^*))=1$, so
$i(C_1(k))=1$, so $C_1(k) \in E_2$, so $k \in K_2$. This shows
$$ G_{1K} \circ id_{K_2} \subseteq id_{K_2} \circ G_{1K}. \eqno (1) $$
Next,
$$\eqqalignno\quad{
G_{1E} \circ id_{E_2}
&= \overline{C_1} \circ G_{1K} \circ \overline{C_1}\inv \circ id_{E_2}
&\text{by theorem~20(iv)} \cr
&= \overline{C_1} \circ G_{1K} \circ id_{K_2} \circ \overline{C_1}\inv
&\text{since $K_2 = C_1\pre{E_2}$} \cr
&\subseteq \overline{C_1} \circ id_{K_2} \circ G_{1K} \circ \overline{C_1}\inv
&\text{by (1)} \cr
&= id_{E_2} \circ \overline{C_1} \circ G_{1K} \circ \overline{C_1}\inv
&\text{since $K_2 = C_1\pre{E_2}$} \cr
&= id_{E_2} \circ G_{1E}
&\text{by theorem~20(iv).} \cr
}{(2)} $$
Next,
$$ G_1 \circ id_{\Sigma_2\cup N_2\cup H_2}
= G_{1\Sigma} \cup G_{1N} \cup G_{1H}
= id_{\Sigma_2\cup N_2\cup H_2} \circ G_1 \eqno(3) $$
since $\Sigma_2=\Sigma_1$, $N_2=N_1$ and $H_2=H_1$. Combining (1), (2) and (3)
gives
$$ G_1 \circ id_{\Sigma_2\cup N_2\cup H_2\cup E_2\cup K_2}
\subseteq id_{\Sigma_2\cup N_2\cup H_2\cup E_2\cup K_2} \circ G_1 $$
as required. Thus $\N_2$ is indeed a subnetwork of $\N_1$. The remaining
conditions for a pruning operation,
$$ \forall \sigma\from\Sigma_1\setdiff\Sigma_2\ i(\sigma) = 0, \quad
\forall n\from N_1\setdiff N_2\ i(n) = 0, \quad
\forall e\from E_1\setdiff E_2\ i(e) = 0, $$
hold by definition of $\Sigma_2,N_2,E_2$.

Since $\N_1$ is assumed unprunable, given $(i,j)$, it follows that $\N_2=\N_1$.
This means that $E_2=E_1$ and so $\forall e\from E_1\ i(e)=1$. \qed

\theorem 43. If

\item{(a)} $\N_1=\network{_1}$ is a network,

\item{(b)} $p:\N_1\to\N_0$ is a homomorphism, where $\N_0$ is a semi-definite
network,

\item{(c)} $(i,j)$ is a pair of inclusion functions on $\N_1$ satisfying

$\forall x\from \Sigma_1 \cup N_1 \cup E_1 \ i(x) \in \{0, 1\}, \quad \forall
h\from H_1\ j(h)=0, \quad \forall k\from K_1\setdiff\dom(G_1)\ j(k)=0$,

\item{(d)} $\N_1$ is unprunable, given $(i,j)$,

\smallskip\f
then

\smallskip

\item{(i)} $\forall e\from E_1\ i(e) = 1$,

\item{(ii)} $\forall n\from N_1\ i(n) = 1$,

\item{(iii)} $E_1 \buildrel F_1 \over \rightarrow A_1\pre{N_1\cup Y} \buildrel
S_1 \over \leftarrow E_1$ is a sum diagram in the category of sets, where
$Y=\comp{\sigma\from\Sigma_1}{i(\sigma)=1}$,

\item{(iv)} $\exists f:K_1\setdiff\dom(G_1) \to K_1 \ G_{1K}\inv = \overline
f$,

\item{(v)} $\forall n\from N_1\ i(W_1(n)) = 1 = i(P_1(n))$,

\item{(vi)} $\forall X \subseteq\Sigma_1\ |P_1\pre X| - |G_{1N} \circ
id_{P_1\pre X}| \le |X|$.

\proof (i) is given by theorem~42.

(ii) Consider the pruning operation that transforms $\N_1$ to
$\N_2=\network{_2}$, where

$\Sigma_2 = \Sigma_1, \quad N_2 = \comp{n\from N_1}{i(n)=1}, \quad H_2 =
A_1\pre{N_2\cup\Sigma_2}, \quad E_2 = E_1, \quad K_2 = K_1,$

$W_2 = W_1|_{N_2\cup\Sigma_2}, \quad P_2 = P_1|_{N_2}, \quad A_2 = A_1|_{H_2},
\quad F_2 = F_1, \quad S_2 = S_1, \quad C_2 = C_1,$

$G_2 = id_{\Sigma_2\cup N_2\cup H_2\cup E_2\cup K_2} \circ G_1 \circ
id_{\Sigma_2\cup N_2\cup H_2\cup E_2\cup K_2}$.

\smallskip\f
I shall show that this is indeed a pruning operation, and then since $\N_1$ is
assumed unprunable it will follow that $\N_2=\N_1$.

First we check that $\N_2$ is a subnetwork of $\N_1$. The conditions $W_1(N_2)
\subseteq \Sigma_2$ and $P_1(N_2) \subseteq \Sigma_2$, are immediate, since
$\Sigma_2=\Sigma_1$.

Define $Y=\comp{\sigma\from\Sigma_1}{i(\sigma)=1}$ (as in part (iii) in the
statement of the theorem). For any $h\from H_1$, we have the condition
$$ i(A_1(h)) = j(h) \ + \sum_{e\in F_1\preo h} \hskip-3mm i(e)
\ + \sum_{e\in S_1\preo h} \hskip-3mm i(e) $$
where $j(h)=0$; so $h \in A_1\pre{N_2 \cup Y}$ iff $i(A_1(h))=1$ iff there
exists $e\from F_1\preo h$ or $e\from S_1\preo h$ (where such an $e$ is unique
and belongs to just one of the two sets). This means that
$$ E_1 \buildrel F_1 \over \rightarrow A_1\pre{N_2\cup Y} \buildrel
S_1 \over \leftarrow E_1 \text{ is a sum diagram.} \eqno (1) $$
This implies $F_1(E_1) \subseteq A_1\pre{N_2\cup Y} \subseteq H_2$ and $S_1(E_1)
\subseteq A_1\pre{N_2\cup Y} \subseteq H_2$, as required.

The functions $W_2,P_2,A_2,F_2,S_2,C_2$ are as required for a subnetwork.

To verify $G_1 \circ id_{\Sigma_2\cup N_2\cup H_2\cup E_2 \cup K_2} \subseteq
id_{\Sigma_2\cup N_2\cup H_2\cup E_2\cup K_2} \circ G_1$ we need the following
derivations.

Since $\Sigma_2=\Sigma_1$, $E_2=E_1$ and $K_2=K_1$,
$$\eqalign{
G_1 \circ id_{\Sigma_2} &= G_{1\Sigma} = id_{\Sigma_2} \circ G_1, \cr
G_1 \circ id_{E_2} &= G_{1E} = id_{E_2} \circ G_1, \cr
G_1 \circ id_{K_2} &= G_{1K} = id_{K_2} \circ G_1.
} \eqno(2) $$
Next,
$$\eqqalignno{\kern3pt}{
G_{1H} \circ id_{A_1\pre{N_2}}
&\subseteq G_{1H} \circ id_{A_1\pre{N_2\cup Y}}
&\cr
&= G_{1H} \circ \bigl( \overline{F_1} \circ \overline{F_1}\inv \ \cup \
\overline{S_1} \circ \overline{S_1}\inv \bigr)
&\text{by theorem~7 and (1)} \cr
&= G_{1H} \circ \overline{F_1} \circ \overline{F_1}\inv \ \cup \
G_{1H} \circ \overline{S_1} \circ \overline{S_1}\inv
& \cr
&= G_1 \circ \overline{F_1} \circ \overline{F_1}\inv \ \cup \
G_1 \circ \overline{S_1} \circ \overline{S_1}\inv
& \cr
&= \overline{F_1} \circ G_1 \circ \overline{F_1}\inv \ \cup \
\overline{S_1} \circ G_1 \circ \overline{S_1}\inv
&\text{by theorem~20(ii)} \cr
&= \overline{F_1} \circ id_{E_1} \circ G_1 \circ \overline{F_1}\inv \ \cup \
\overline{S_1} \circ id_{E_1} \circ G_1 \circ \overline{S_1}\inv
& \cr
&\subseteq id_{H_2} \circ \overline{F_1} \circ G_1 \circ \overline{F_1}\inv \
\cup \ id_{H_2} \circ \overline{S_1} \circ G_1 \circ \overline{S_1}\inv
&\text{since $F_1(E_1) \subseteq H_2$} \cr
&= id_{H_2} \circ G_1 \circ \overline{F_1} \circ \overline{F_1}\inv
\ \cup \ id_{H_2} \circ G_1 \circ \overline{S_1} \circ \overline{S_1}\inv
&\text{by theorem~20(ii)} \cr
&\subseteq id_{H_2} \circ G_1 \circ id_{H_1} \ \cup \
id_{H_2} \circ G_1 \circ id_{H_1}
&\text{by theorem~2(i)} \cr
&= id_{H_2} \circ G_{1H}.
&\cr
}{\kern-30pt(3)}$$
Next, from $\overline{A_1} \circ G_1 \subseteq G_1 \circ \overline{A_1}$ we have
$$\eqqalign\quad{
G_{1H} \circ id_{A_1\pre{\Sigma_2}}
&\subseteq \overline{A_1}\inv \circ G_1 \circ \overline{A_1} \circ
id_{A_1\pre{\Sigma_2}}
&\text{by theorem~2(iv)}\cr
&= \overline{A_1}\inv \circ G_1 \circ id_{\Sigma_2} \circ \overline{A_1}
&\cr
&= \overline{A_1}\inv \circ id_{\Sigma_2} \circ G_1 \circ \overline{A_1}
&\text{by (2)}\cr
&\subseteq id_{H_2} \circ \overline{A_1}\inv \circ G_1 \circ \overline{A_1}
&\text{since $A_1\pre{\Sigma_2} \subseteq H_2$}\cr
}$$
so by theorem~4(vi)
$$ G_{1H} \circ id_{A_1\pre{\Sigma_2}} \subseteq id_{H_2} \circ G_{1H}. \eqno(4)
$$
Hence,
$$\eqqalignno\quad{
G_{1H} \circ id_{H_2}
&= G_{1H} \circ id_{A_1\pre{N_2 \cup \Sigma_2}}
&\cr
&= G_{1H} \circ id_{A_1\pre{N_2}} \ \cup\ G_{1H} \circ id_{A_1\pre{\Sigma_2}}
&\cr
&\subseteq id_{H_2} \circ G_{1H}
&\text{by (3) and (4).}\cr
}{(5)}$$
Next,
$$\eqqalignno\quad{
G_{1N} \circ id_{N_2}
&= id_{N_1} \circ \overline{A_1} \circ G_{1H} \circ \overline{A_1}\inv \circ
id_{N_2}
&\text{by theorem~20(iii)} \cr
&\subseteq id_{N_1} \circ \overline{A_1} \circ G_{1H} \circ id_{H_2} \circ
\overline{A_1}\inv
&\text{since $A_1\pre{N_2} \subseteq H_2$} \cr
&\subseteq id_{N_1} \circ \overline{A_1} \circ id_{H_2} \circ G_{1H} \circ
\overline{A_1}\inv
&\text{by (5)} \cr
&= id_{N_1} \circ id_{N_2\cup\Sigma_2} \circ \overline{A_1} \circ G_{1H} \circ
\overline{A_1}\inv
&\text{since $H_2 = A_1\pre{N_2\cup\Sigma_2}$} \cr
&= id_{N_2} \circ id_{N_1} \circ \overline{A_1} \circ G_{1H} \circ
\overline{A_1}\inv
& \cr
&= id_{N_2} \circ G_{1N}
&\text{by theorem~20(iii).} \cr
}{(6)}$$
From (2), (5) and (6),
$$ G_1 \circ id_{\Sigma_2\cup N_2\cup H_2\cup E_2\cup K_2} \subseteq
id_{\Sigma_2\cup N_2\cup H_2\cup E_2\cup K_2} \circ G_1. $$
Thus $\N_2$ is indeed a subnetwork of $\N_1$. The remaining conditions for a
pruning operation,
$$ \forall \sigma\from\Sigma_1\setdiff\Sigma_2\ i(\sigma) = 0, \quad
\forall n\from N_1\setdiff N_2\ i(n) = 0, \quad
\forall e\from E_1\setdiff E_2\ i(e) = 0, $$
hold by definition of $\Sigma_2,N_2,E_2$.

Since $\N_1$ is assumed unprunable, given $(i,j)$, it follows that $\N_2=\N_1$.
This means that $N_2=N_1$ and so $\forall n\from N_1\ i(n)=1$.

(iii) follows from (1), bearing in mind that $N_2=N_1$.

(iv) For any $k \from K_1 \setdiff \dom(G_1)$,
$$ i(C_1(k)) = j(k) + \sum_{k^*\mid G_1(k,k^*)} i(C_1(k^*)) $$
where $i(C_1(k)) = 1$, $j(k) = 0$, and each $i(C_1(k^*)) = 1$, by part (i) and
hypothesis~(c), so there exists a unique $k^*$ such that $G_1(k,k^*)$. Define
$f:K_1\setdiff\dom(G_1) \to K_1$ mapping $k$ to this $k^*$. On the other hand,
for any $k \from K_1 \wedge \dom(G_1)$, we have $k \notin \ran(G_1)$, so there
exists no $k^*$ such that $G_1(k,k^*)$. Thus $G_{1K}\inv = \overline f$.

(v) $\forall n\from N_1\ i(W_1(n)) = 1$ holds since, for any $n\from N_1$,
$$ i(W_1(n)) = j(n) + i(n) $$
where $i(n) = 1$ by part (ii), so $i(W_1(n)) = 1$.

The other equation, $\forall n\from N_1\ i(P_1(n)) = 1$, is proved using
theorem~21 and theorem~13. The hypotheses of theorem~21 hold, by parts (iii) and
(iv) just proved. Theorem~21 then tells us that $G_{1N}$ is acyclic. The next
step is to apply theorem~13 to the sets $N_1,\Sigma_1$, the function
$P_1:N_1\to\Sigma_1$ and the finite relation $G_{1N}$ on $N_1$. Let us check the
hypotheses of theorem~13.

Hypothesis (a): $G_{1N} \circ G_{1N} \subseteq G_1 \circ G_1 = \bot$ (since
$\N_1$ is a network).

Hypothesis (b): $G_{1N}$ is acyclic (as just shown).

Hypothesis (c): $\overline{P_1} \circ G_{1N} = \overline{P_1} \circ G_1
\subseteq \overline{P_1}$ (since $\N_1$ is a network).

\smallskip\f
Now, for any $\sigma\from\Sigma_1$ such that $i(\sigma)=0$, taking $X =
\{\sigma\}$ in theorem~13(i) gives
$$ |P_1\preo\sigma| - |G_{1N} \circ id_{P_1\preo\sigma}| \ge 0. $$
Moreover, (recalling the notation $g_n = \bigl|\comp{n^*\from
N_1}{G_1(n^*,n)}\bigr|$)
$$\eqalign{
0 = i(\sigma)
&= j(\sigma) \ + \sum_{n\in P_1\preo\sigma} \hskip-3mm (1-g_n)i(n)
= j(\sigma) \ + \sum_{n\in P_1\preo\sigma} \hskip-3mm (1-g_n)
\cr&
= j(\sigma) + |P_1\preo\sigma| -
|\comp{(n^*,n)\from N_1\times P_1\preo\sigma}{G_1(n^*,n)}|
\cr&
= j(\sigma) + |P_1\preo\sigma| - |G_{1N} \circ id_{P_1\preo\sigma}|
}$$
so $j(\sigma)=0$ and $|P_1\preo\sigma| - |G_{1N} \circ id_{P_1\preo\sigma}| =
0$. Then by theorem~13(ii) $P_1\preo\sigma = \emptyset$. The contrapositive of
this result is that if $P_1\preo\sigma \ne \emptyset$ then $i(\sigma)=1$. Thus
$\forall n\from N_1\ i(P_1(n)) = 1$, as required.

(vi) For any $\sigma\from\Sigma_1$,
$$\eqalign{
i(\sigma)
&= j(\sigma) \ + \sum_{n\in P_1\preo\sigma} \hskip-3mm (1-g_n)i(n)
= j(\sigma) + |P_1\preo\sigma| - |G_{1N} \circ id_{P_1\preo\sigma}|
}$$
as in part (v), where $i(\sigma) \in \{0,1\}$ and $j(\sigma) \in [0,1]$, so
$$ |P_1\preo\sigma| - |G_{1N} \circ id_{P_1\preo\sigma}| \le 1. $$
For any $X \subseteq\Sigma_1$, summing this inequality over all $\sigma\from X$
gives
$$ |P_1\pre X| - |G_{1N} \circ id_{P_1\pre X}| \le |X| $$
as required. \qed

\theorem 44. If

\item{(a)} $\N_1=\network{_1}$ is a network,

\item{(b)} $p:\N_1\to\N_0$ is a homomorphism, where $\N_0$ is a semi-definite
network,

\item{(c)} $(i,j)$ is a pair of inclusion functions on $\N_1$ satisfying

\smallskip

$\forall x\from \Sigma_1 \cup N_1 \cup E_1 \ i(x) \in \{0, 1\}$,\quad $\forall
h\from H_1 \ j(h) = 0$,\quad $\forall k\from K_1 \setdiff \dom(G_1)\ j(k) = 0$,

\smallskip

\item{(d)} $\N_1$ is unprunable, given $(i,j)$,

\item{(e)} $E_1 \doublearrow{A_1 \circ F_1}{A_1 \circ S_1} N_1\cup\Sigma_1
\buildrel W_1 \over \rightarrow \Sigma_1$ is a coequaliser diagram in the
category of sets,

\smallskip\f
then

\smallskip

\item{(i)} $\forall x\from \Sigma_1\cup N_1\cup E_1\ i(x) = 1$,

\item{(ii)} $\N_1$ is definite.

\proof The hypotheses of this theorem include those of theorem~43, so we can
apply theorem~43.

(i) From theorem~43(i),(ii) we already have $\forall e\from E_1\ i(e) = 1$ and
$\forall n\from N_1\ i(n) = 1$. Consider the pruning operation that transforms
$\N_1$ to $\N_2=\network{_2}$, where

$\Sigma_2 = \comp{\sigma\from\Sigma_1}{i(\sigma)=1}, \quad N_2 = N_1, \quad H_2=
A_1\pre{N_2\cup\Sigma_2}, \quad E_2 = E_1, \quad K_2 = K_1,$

$W_2 = W_1|_{N_2\cup\Sigma_2}, \quad P_2 = P_1, \quad A_2 = A_1|_{H_2}, \quad
F_2 = F_1, \quad S_2 = S_1, \quad C_2 = C_1,$

$G_2 = id_{\Sigma_2\cup N_2\cup H_2\cup E_2\cup K_2} \circ G_1 \circ
id_{\Sigma_2\cup N_2\cup H_2\cup E_2\cup K_2}$.

\smallskip\f
I shall show that this is indeed a pruning operation, and then since $\N_1$ is
assumed unprunable it will follow that $\N_2=\N_1$.

First we check that $\N_2$ is a subnetwork. The first two conditions, $W_1(N_2)
\subseteq \Sigma_2$ and $P_1(N_2) \subseteq \Sigma_2$ follow from
theorem~43(v).

Theorem~43(iii) tells us that
$$ E_1 \buildrel F_1 \over \rightarrow H_2 \buildrel
S_1 \over \leftarrow E_1 \text{ is a sum diagram} \eqno (1) $$
since $H_2 = A_1\pre{N_2\cup\Sigma_2} = A_1\pre{N_1\cup Y}$. This implies
$F_1(E_2) \subseteq H_2$ and $S_1(E_2) \subseteq H_2$, as required.

The functions $W_2,P_2,A_2,F_2,S_2,C_2$ are as required for a subnetwork.

Next we verify the condition $G_1 \circ id_{\Sigma_2\cup N_2\cup H_2\cup E_2\cup
K_2} \subseteq id_{\Sigma_2\cup N_2\cup H_2\cup E_2\cup K_2} \circ G_1$.

The hypotheses of theorem~22 are satisfied (with $Y=\Sigma_2$). Theorem~22(iii)
gives
$$ G_1 \circ id_{\Sigma_2} \subseteq id_{\Sigma_2} \circ G_1. \eqno(2) $$
The conditions
$$\eqalignno{
G_1 \circ id_{N_2} &= id_{N_2} \circ G_1 &(3)\cr
G_1 \circ id_{E_2} &= id_{E_2} \circ G_1 &(4)\cr
G_1 \circ id_{K_2} &= id_{K_2} \circ G_1 &(5)
}$$
hold trivially, since $N_2=N_1$, $E_2=E_1$ and $K_2=K_1$. Also,
$$\eqqalign\quad{
G_1 \circ id_{H_2}
&= id_{H_1} \circ G_1 \circ id_{H_2}
&\text{since $H_2 \subseteq H_1$}\cr
&\subseteq \overline{A_1}\inv \circ G_1 \circ \overline{A_1} \circ id_{H_2}
&\text{from $\overline{A_1} \circ G_1 \subseteq G_1 \circ \overline{A_1}$ by
theorem~2(iv)}\cr
&= \overline{A_1}\inv \circ G_1 \circ id_{N_2\cup \Sigma_2} \circ
\overline{A_1}
&\text{since $H_2 = A_1\pre{N_2\cup\Sigma_2}$}\cr
&\subseteq \overline{A_1}\inv \circ id_{N_2\cup \Sigma_2} \circ G_1 \circ
\overline{A_1}
&\text{by (3) and (2)}\cr
&= id_{H_2} \circ \overline{A_1}\inv \circ G_1 \circ \overline{A_1}
&\text{since $H_2 = A_1\pre{N_2\cup\Sigma_2}$}\cr
}$$
and hence by theorem~4(vi)
$$ G_1 \circ id_{H_2} \subseteq id_{H_2} \circ G_1. \eqno(6) $$
From (2), (3), (4), (5) and (6) we derive $G_1 \circ id_{\Sigma_2\cup N_2\cup
H_2\cup E_2\cup K_2} \subseteq id_{\Sigma_2\cup N_2\cup H_2\cup E_2\cup K_2}
\circ G_1$. Hence $\N_2$ is indeed a subnetwork of $\N_1$.

The conditions
$$\forall \sigma\from\Sigma_1\setdiff\Sigma_2\ i(\sigma) = 0, \quad
\forall n\from N_1\setdiff N_2\ i(n) = 0, \quad
\forall e\from E_1\setdiff E_2\ i(e) = 0 $$
follow immediately from the definitions of $\Sigma_2,N_2,E_2$. This completes
the verification that we have a pruning operation.

Since $\N_1$ is assumed to be unprunable, given $(i,j)$, the pruning operation
must be the trivial one, with $\N_2=\N_1$. This means that $\Sigma_2=\Sigma_1$
and so $\forall\sigma\from\Sigma_1\ i(\sigma)=1$, as required.

(ii) We shall apply theorem~23; let us check its hypotheses.

Hypothesis (a) holds by theorem~43(vi).

Hypothesis (b), that $E_1 \buildrel F_1 \over \rightarrow H_1 \buildrel S_1
\over \leftarrow E_1$ is a sum diagram, follows from (1) and the fact that
$\N_2=\N_1$.

Hypothesis (c) holds by theorem~27(iv).

Hypothesis (d) holds by hypothesis (e) of this theorem.

Thus it follows by theorem~23 that $\N_1$ is definite. \qed

\subhead{8.4 Extension operations}
Given a grammar $\N_0$, a pattern $\N_1$, a homomorphism $p:\N_1\to\N_0$, and an
embedding token $u$ for $\N_1$, an \i{extension} of $(\N_1,p,u)$ is a triple
$(\N_1',p',u')$ where $\N_1$ is a subnetwork of $\N_1'$, $p':\N_1'\to\N_0$ is a
homomorphism such that $p = p'|_{\N_1}$, and $u'$ is an embedding token for
$\N_1'$ such that $u = u'|_{\N_1}$.

$(\N_1',p',u')$ is a \i{minimal} extension of $(\N_1,p,u)$ satisfying a
condition $P$ iff

\smallskip

\item{(i)} $(\N_1',p',u')$ is an extension of $(\N_1,p,u)$ satisfying $P$;

\item{(ii)} for any extension $(\N_1'',p'',u'')$ of $(\N_1,p,u)$ satisfying $P$,
$|\N_1'| \le |\N_1''|$,

\smallskip\f
where the cardinality $|\N|$ of a network $\N$ is defined by $|\network{}| =
|\Sigma| + |N| + |H| + |E| + |K|$.

An extension is \i{trivial} iff $\N_1'=\N_1$.

\medbreak\f
Using these notions we can define the extension operations used in the
algorithm. The notation is as usual: we have a grammar $\N_0=\network{_0}$
and an embedding type $v = (sub,\allowbreak
con,\allowbreak rel,\allowbreak symm,\allowbreak tem, \allowbreak in)$ on
$\N_0$, a pattern $\N_1=\network{_1}$ with a parse $p:\N_1\to\N_0$, an embedding
token $u$, a pair of inclusion functions $(i,j)$, and a bareness function
$B$ for $\N_1$; we shall produce an extended network $\N_1'=\network{_1'}$
with a new parse $p':\N_1'\to\N_0$ and embedding token $u'$. The
threshold $\theta$ is the positive constant used in the $DM$ function (see
\S4.5); the thresholds $\theta_0,\theta_1,\theta_2,\theta_3,\theta_4$ are 
used only in the extension operations and may be made dependent on parameters
such as temperature.

In the extension operations the following additional conditions, referred to
collectively as \i{the extension conditions}, will be imposed.

\blob $\forall\sigma\from\Sigma_1\ ({P_1'}\preo\sigma \not\subseteq N_1 \imp 
j(\sigma) > \theta_0 \and B(\sigma) < \theta)$,

\blob $\forall h\from H_1\ ({F_1'}\preo h \cup {S_1'}\preo h
\not\subseteq E_1 \imp j(h) > \theta_0)$,

\blob $\forall e\from E_1'\ (A_1'(F_1'(e)) \notin N_1 \OR
A_1'(S_1'(e)) \notin N_1 \imp W_1'(A_1'(F_1'(e))) = W_1'(A_1'(S_1'(e))))$,

\blob $\forall n \in N_1'\setdiff N_1 \ \
E_{con(p'(n))}(u'(W_1'(n))\inv \cdot u'(n)) < \theta_1$,

\blob the symmetry condition for $\N_1',u',v \circ p'$.

\medskip\f
The \i{extension operations} are as follows (see figure~1 below). For each one,
the extension conditions are checked at the end and the operation is cancelled
if they do not hold. (Note that no consistent pair of inclusion functions
$(i',j')$ can be specified for the extended pattern $\N_1'$, so we recalculate 
them as in \S7.4, using the old inclusion functions $(i,j)$ as a starting 
point.)

\medskip\f
(a) (Joining two symbols.) Given symbols $\sigma_1,\sigma_2 \from \Sigma_1$, an
edge $e_0 \from E_0$, and affine transformations $s_1 \from symm(p(\sigma_1))$
and $s_2 \from symm(p(\sigma_2))$ such that

\blob $P_0(A_0(F_0(e_0))) = p(\sigma_1)$ and $P_0(A_0(S_0(e_0))) = p(\sigma_2)$,

\blob $E_{rel(e_0)}(s_2\inv \cdot u(\sigma_2)\inv \cdot u(\sigma_1) \cdot s_1)
< \theta_2$,

\medskip\f
construct a minimal extension $(\N_1',p',u')$ of $(\N_1,p,u)$ (if one exists)
such that $\N_1'$ contains nodes $n_1,n_2$ and an edge $e$ for which

\blob $p'(e)=e_0$, $A_1'(F_1'(e))=n_1$, $A_1'(S_1'(e)) = n_2$,
$P_1'(n_1) = \sigma_1$ and $P_1'(n_2) = \sigma_2$,

\blob $u'(n_1) = u(\sigma_1) \cdot s_1$ and $u'(n_2) = u(\sigma_2) \cdot s_2$.

\medskip\f
(b) (Joining three symbols.) Given symbols
$\sigma_1,\sigma_2,\sigma_3\from\Sigma_1$, edges $e_{01},e_{02}\from E_0$,
$s_1\from symm(p(\sigma_1))$, $s_2\from symm(p(\sigma_2))$ and $s_3\from
symm(p(\sigma_3))$ such that

\blob $A_0(S_0(e_{01}))=A_0(F_0(e_{02}))$, $P_0(A_0(F_0(e_{01})))=p(\sigma_1)$,
$P_0(A_0(S_0(e_{01})))=p(\sigma_2)$ and
$P_0(A_0(S_0(e_{02})))\allowbreak=p(\sigma_3)$,

\blob $E_{rel(e_{01})}(s_2\inv \cdot u(\sigma_2)\inv\cdot u(\sigma_1) \cdot s_1)
+ E_{rel(e_{02})}(s_3\inv \cdot u(\sigma_3)\inv \cdot u(\sigma_2) \cdot s_2) <
\theta_3$,

\medskip\f
construct a minimal extension $(\N_1',p',u')$ of $(\N_1,p,u)$ (if one exists)
such that $\N_1'$ contains nodes $n_1,n_2,n_3$ and edges $e_1,e_2$ for which

\blob $p'(e_1)=e_{01}$, $p'(e_2)=e_{02}$, $A_1'(F_1'(e_1)) = n_1$,
$A_1'(S_1'(e_1))=n_2=A_1'(F_1'(e_2))$, $A_1'(S_1'(e_2))=n_3$,
$P_1'(n_1)=\sigma_1$, $P_1'(n_2)=\sigma_2$ and $P_1'(n_3)=\sigma_3$,

\blob $u'(n_1)=u(\sigma_1)\cdot s_1$, $u'(n_2)=u(\sigma_2)\cdot s_2$ and
$u'(n_3)=u(\sigma_3)\cdot s_3$.

\medskip\f
(There are also variations of operation~(b), in which the directions of $e_{01}$
and $e_1$ are reversed, or the directions of $e_{02}$ and $e_2$ are reversed.)

\medskip\f
(c) (Extending from a hook.) Given a hook $h\from H_1$, construct a minimal
extension $(\N_1',p',u')$ of $(\N_1,p,u)$ such that

\blob $p'({F_1'}\inv(\{h\})) = F_0\inv(p(\{h\}))$ and $p'({S'_1}\inv(\{h\})) =
S_0\inv(p(\{h\}))$,

\blob $\forall e\from E_1'\setdiff E_1\ \ E_{rel(p'(e))}(u'(A_1'(S_1'(e)))\inv
\cdot u'(A_1'(F_1'(e)))) = 0$.

\medskip\f
(d) (Extending from a facet.) Given a facet $k\from K_1$ such that

\blob $W_1(A_1(F_1(C_1(k))))=W_1(A_1(S_1(C_1(k))))$

\blob $j(k) > \theta_0$,

\medskip\f
construct a minimal extension $(\N_1',p',u')$ of $(\N_1,p,u)$ such that

\blob $\overline{p'} \circ {G_1'}\inv \circ id_{\{k\}} = G_0\inv \circ
\overline p \circ id_{\{k\}}$.

\medskip\f
(e) (Extending from a part to a whole.) Given a symbol $\sigma\from\Sigma_1$,
construct a minimal extension $(\N_1',p',u')$ of $(\N_1,p,u)$ such that

\blob $p'({P_1'}\pre{\{\sigma\}}) = P_0\pre{p(\{\sigma\})}$,

\blob $\forall n\from N_1'\setdiff N_1\ E_{con(p'(n))}(u'(W_1'(n))\inv \cdot
u'(n)) = 0$.

\medskip\f
(f) (Filling in a missing part between two parts.) Given nodes $n_1,n_3\from
N_1$, hooks $h_1,h_3\from H_1$, edges $e_{01},e_{02}\from E_0$ and an affine
transformation $f$ such that

\blob $W_1(n_1)=W_1(n_3)$, $A_1(h_1)=n_1$, $A_1(h_3)=n_3$,
$A_0(S_0(e_{01}))=A_0(F_0(e_{02}))$, $F_0(e_{01})=p(h_1)$ and
$S_0(e_{02})=p(h_3)$,

\blob $E_{rel(e_{01})}(f\inv \cdot u(n_1)) + E_{rel(e_{02})}(u(n_3)\inv \cdot f)
< \theta_4$,

\medskip\f
construct a minimal extension $(\N_1',p',u')$ of $(\N_1,p,u)$ (if one exists)
such that $\N_1'$ contains edges $e_1,e_2$ and a node $n_2$ for which

\blob $p'(e_1) = e_{01}$, $p'(e_2) = e_{02}$, $F'_1(e_1) = h_1$,
$A'_1(S'_1(e_1))=n_2=A'_1(F'_1(e_2))$ and $S'_1(e_2) = h_3$,

\blob if $n_2\notin N_1$ then $u'(n_2)=f$.

\medskip\f
(There are also variations of operation~(f), in which the directions of $e_{01}$
and $e_1$ are reversed, or the directions of $e_{02}$ and $e_2$ are reversed.)

\medskip\f
(g) (Filling in a symbol between part and whole.) Given symbols
$\sigma_1,\sigma_3\from\Sigma_1$, symbols \newline
$\sigma_{01},\sigma_{02},\sigma_{03}\from\Sigma_0$, nodes $n_{01},n_{02}\from
N_0$, $s\from symm(\sigma_{03})$, and an affine transformation $f$ such that

\blob $p(\sigma_1)=\sigma_{01}$, $p(\sigma_3)=\sigma_{03}$,
$W_0(n_{01})=\sigma_{01}$, $P_0(n_{01})=\sigma_{02}=W_0(n_{02})$ and
$P_0(n_{02})=\sigma_{03}$,

\blob $E_{con(n_{01})}(u(\sigma_1)\inv \cdot f) +
E_{con(n_{02})}(f\inv \cdot u(\sigma_3) \cdot s) < \theta_4$,

\smallskip\f
construct a minimal extension $(\N_1',p',u')$ of $(\N_1,p,u)$ such that $\N_1'$
contains a symbol $\sigma_2$ and nodes $n_1,n_2$ for which

\blob $p'(n_1)=n_{01}$, $p'(n_2)=n_{02}$, $W_1'(n_1)=\sigma_1$,
$P_1'(n_1)=\sigma_2=W_1(n_2)$ and $P_1'(n_2)=\sigma_3$,

\blob if $n_1 \notin N_1$ then $u'(n_1)=u'(\sigma_2)=f$,

\blob if $n_2 \notin N_1$ then $u'(n_2)=u(\sigma_3)\cdot s$.

\medskip\f
These extension operations are applied concurrently, in a fair order, controlled
by probabilities; the probability is low in cases where new symbols would be
created (particularly operations~(a) and (e)), to avoid the creation of too many
new symbols.

These operations are depicted in figure~1. In this figure rectangles
represent symbols, circles represent nodes, small filled discs represent hooks, lines
with arrowheads halfway along represent edges, and small crosses represent
facets (shown only for operation~(e)); the $W$ and $P$ functions, which map each
node to the whole and part symbols, are represented by lines with arrowheads at
the end. For each operation solid lines are used for the symbols, nodes, etc.,
assumed to be present in the pattern before the extension operation; dashed
lines are used for the symbols, nodes, etc., added by the extension operation
(if they are not already present in $\N_1$). Thus, for example, operation~(g)
adds one symbol and two nodes (and their associated hooks), unless a suitable
symbol or suitable nodes already exist in $\N_1$. Note, however, that whenever
an edge is added the appropriate number of superedges must also be added, in
order that $p'$ satisfy the conditions for a homomorphism; and the same applies
to symbols, nodes, etc.; these are not shown in the figure.

\def\twofigures#1#2#3#4#5{\centerline{\percentsize{#1}\epsfbox{#2}{\hskip #3}
\percentsize{#4}\epsfbox{#5}}\epsfxsize=\hsize}

\def\threefigures#1#2#3#4#5#6#7#8{\centerline{\percentsize{#1}\epsfbox{#2}
{\hskip #3}\percentsize{#4}\epsfbox{#5}{\hskip #6}
\percentsize{#7}\epsfbox{#8}}\epsfxsize=\hsize}

\bigskip

\goodbreak

\twofigures{30}{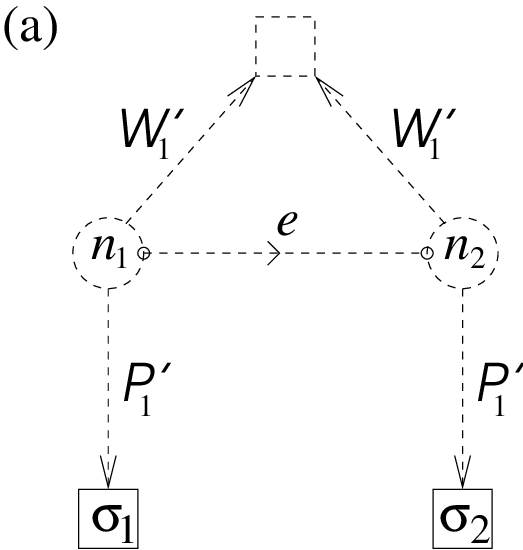}{50pt}{50}{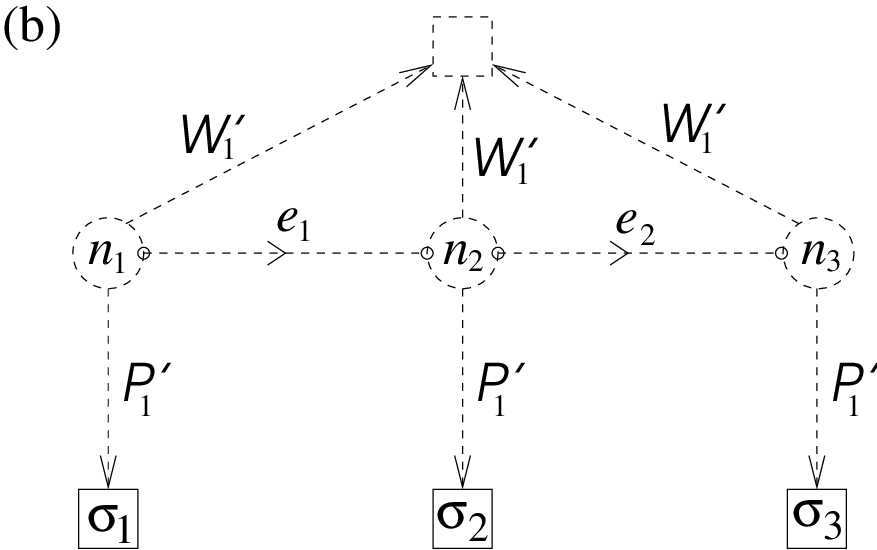}

\bigskip\null\bigskip\null\bigskip

\twofigures{35}{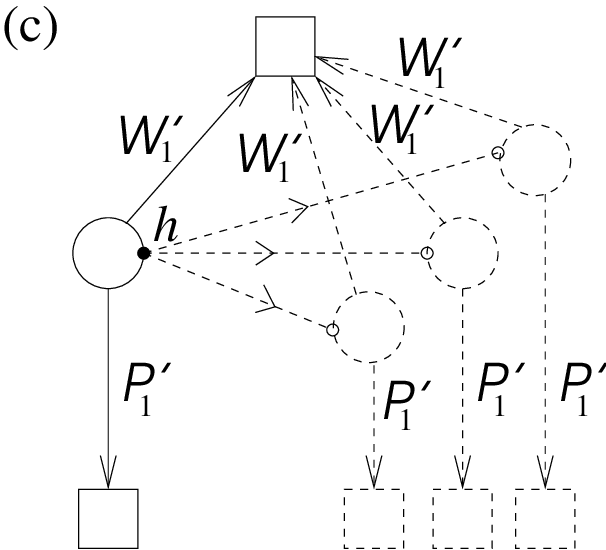}{50pt}{40}{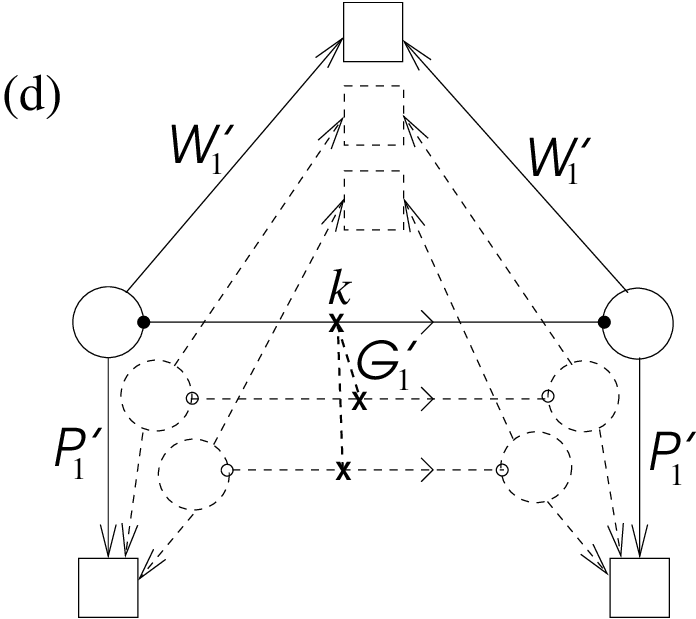}

\bigskip\null\bigskip\null\bigskip

{\nobreak

\threefigures{26}{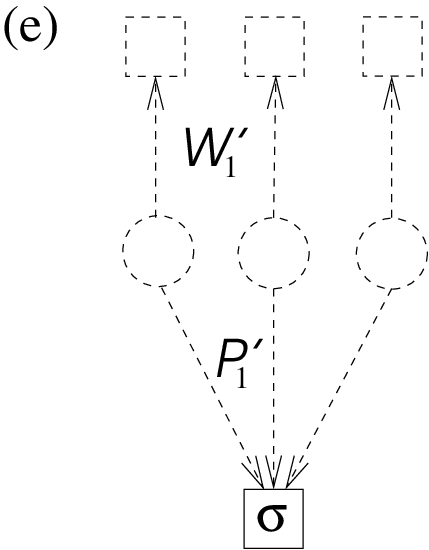}{35pt}{50}{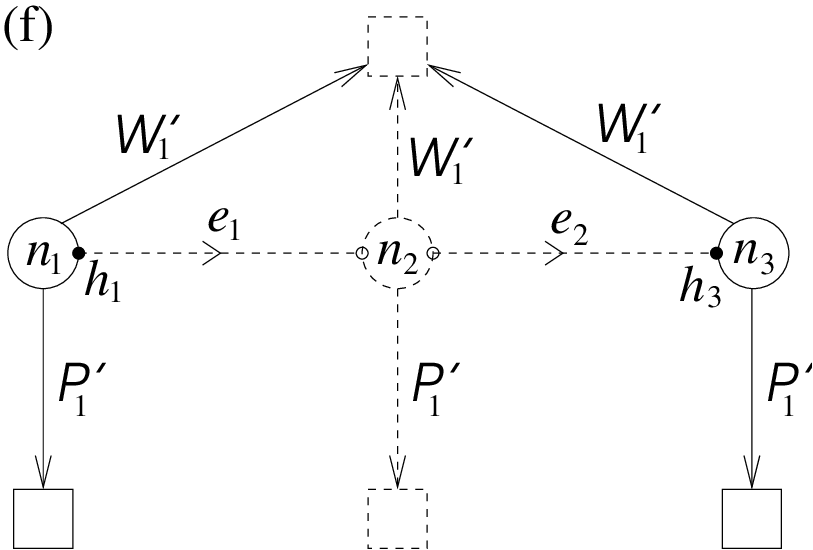}{15pt}{14}{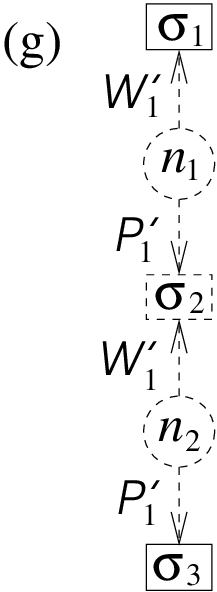}

\bigskip

\longcaption{Figure 1. The extension operations. The figure shows the relevant
parts of the pattern $\N_1'$ after each extension operation. Solid lines depict
what must be present before the operation; dashed lines depict what is added if
not already present.}

}

\subhead{8.5 Inextendability and its consequences}

\defn $(\N_1,p,u)$ is \i{inextendable}, given $i,j,v,B$, iff none of the
extension operations can be applied to it, other than ones giving a trivial
extension.

\theorem 45. If

\item{(a)} $\N_1=\network{_1}$ is a network with an embedding token $u$ and a
bareness function $B$,

\item{(b)} $p:\N_1\to\N_0$ is a homomorphism, where $\N_0$ is a semi-definite
network with an embedding type $v$,

\item{(c)} $(i,j)$ is a pair of inclusion functions on $\N_1$ satisfying
$\forall x\from \Sigma_1 \cup N_1\ i(x) \in \{0, 1\}$ and $\forall e\from E_1\
i(e) = 1$,

\item{(d)} $(\N_1,p,u)$ is inextendable, given $i,j,v,B$,

\item{(e)} $W_1 \circ A_1 \circ F_1 = W_1 \circ A_1 \circ S_1$,

\smallskip\f
then $\forall h\from H_1\ j(h)=0$ and $\forall k\from K_1\setdiff\dom(G_1)\
j(k)=0$.

\proof For any $h\from H_1$, we have
$$ i(A(h)) = j(h) \ + \sum_{e\in F_1\preo h} \hskip-3mm i(e)
\ + \sum_{e\in S_1\preo h} \hskip-3mm i(e). \eqno(1) $$
This implies that $j(h)$ is an integer, and hence must be $0$ or $1$. Suppose
$j(h)=1$. Then the operation of extending from $h$ (extension operation~(c)) is
possible, giving an extension $(\N_1',p',u')$ such that $p'({F_1'}\inv(\{h\})) =
F_0\inv(p(\{h\}))$ and $p'({S'_1}\inv(\{h\})) = S_0\inv(p(\{h\}))$. However, we
are assuming $(\N_1,p,u)$ is inextendable, so $(\N_1',p',u')=(\N_1,p,u)$. Thus
$p(F_1\inv(\{h\})) = F_0\inv(p(\{h\}))$ and $p(S_1\inv(\{h\})) =
S_0\inv(p(\{h\}))$.

Now, $\N_0=\network{_0}$ is semi-definite and so satisfies $F_0(E_0) \cup
S_0(E_0) = H_0$. This means that $F_0\inv(p(\{h\})) \ne \emptyset$ or
$S_0\inv(p(\{h\})) \ne \emptyset$. Hence $p(F_1\inv(\{h\})) \ne \emptyset$ or
$p(S_1\inv(\{h\})) \ne \emptyset$. Hence $F_1\inv(\{h\}) \ne \emptyset$ or
$S_1\inv(\{h\}) \ne \emptyset$. Any edge $e$ in these sets has $i(e)=1$, by
hypothesis (c), so by (1) $i(A(h)) \ge 2$, which is impossible. This
contradiction establishes that $j(h)=0$ as required.

For any $k\from K_1 \setdiff \dom(G_1)$, we have
$$ i(C(k)) = j(k) + \sum_{k^* \mid G_1(k,k^*)} i(C(k^*)). $$
This implies that $j(k)$ is an integer, and hence must be $0$ or $1$. Suppose
$j(k)=1$. Then $\sum_{k^* \mid G_1(k,k^*)} i(C(k^*))=0$, and hence by
hypothesis~(c) there are no $k^*$ such that $G_1(k,k^*)$ holds. This can be
expressed as
$$ G_1\inv \circ id_{\{k\}} = \bot. \eqno(2) $$
Also, since $k\notin \dom(G_1)$ we have
$$ G_1 \circ id_{\{k\}} = \bot. \eqno (3) $$
Now, by hypothesis~(e) and since $j(k)=1$, the operation of extending from $k$
(extension operation~(d)) is possible, giving an extension $(\N_1',p',u')$ such
that $\overline{p'} \circ {G_1'}\inv \circ id_{\{k\}} = G_0\inv \circ \overline
p \circ id_{\{k\}}$. However, we are assuming $(\N_1,p,u)$ is inextendable,
hence $(\N_1',p',u')=(\N_1,p,u)$. Thus
$$ \overline p \circ G_1\inv \circ id_{\{k\}} = G_0\inv \circ \overline p \circ
id_{\{k\}}. \eqno(4) $$
Since $\N_0$ is semi-definite, $G_0$ is minimal relative to $\N_0$ and hence
$id_{K_0} \subseteq G_{0K} \circ G_{0K}\inv \cup G_{0K}\inv \circ G_{0K}$. Then
$$\eqqalign{\kern-9pt}{
\overline p \circ id_{\{k\}}
&\subseteq G_{0K} \circ G_{0K}\inv \circ \overline p \circ id_{\{k\}}\ \cup\
G_{0K}\inv \circ G_{0K} \circ \overline p \circ id_{\{k\}}
&\cr
&\subseteq G_0 \circ G_0\inv \circ \overline p \circ id_{\{k\}}\ \cup\
G_0\inv \circ G_0 \circ \overline p \circ id_{\{k\}}
&\cr
&= G_0 \circ \overline p \circ G_1\inv \circ id_{\{k\}} \ \cup\
G_0\inv \circ \overline p \circ G_1 \circ id_{\{k\}}
&\text{by (4) and since $p$ is a homomorphism}\cr
&= \bot \ \cup \bot = \bot
&\text{by (2) and (3).}\cr
}$$
But this is absurd, since $(\overline p \circ id_{\{k\}})(p(k),k)$ holds. This
contradiction establishes that $j(k)=0$, as required. \qed

\subhead{8.6 Merging two symbol tokens}
We may merge two symbol tokens of the same type that have similar embedding
transformations (up to a symmetry transformation). Two symbol tokens
$\sigma_1,\sigma_2\from\Sigma_1$ of type $\sigma_0\from\Sigma_0$ are considered
to have similar embeddings up to a symmetry transformation iff there exists
$s\in symm(\sigma_0)$ such that $E_{in(\sigma_0)}(s\inv \cdot u(\sigma_2)\inv
\cdot u(\sigma_1))$ is below a threshold. If this condition holds then the
symmetry $s$ is applied to $\sigma_2$ (this is a local symmetry operation; the
other symbols are unchanged); $\sigma_1$ and $\sigma_2$ are replaced by a single
symbol; and the nodes and edges of $\sigma_1$ and $\sigma_2$ are pooled.
Local symmetry operations have already been defined in \S4.3. The merging
itself is formally defined as follows.

\defn Given a network $\N_1=\network{_1}$, and a homomorphism $p:\N_1\to\N_0$,
and two symbols $\sigma_1,\sigma_2\from\Sigma_1$ such that
$p(\sigma_1)=p(\sigma_2)$, 
the operation of \i{merging $\sigma_1$ and $\sigma_2$} produces a new network
$\N_1'=\network{_1'}$ and a homomorphism $\mu:\N_1\to\N_1'$ defined as follows.
First note that there are bijections $p|_{A_1\preo{\sigma_1}}:
A_1\preo{\sigma_1} \to A_0\preo{p(\sigma_1)}$ and
and
$p|_{A_1\preo{\sigma_2}}:
A_1\preo{\sigma_2} \to A_0\preo{p(\sigma_1)}$
and hence a bijection
$\gamma = p|_{A_1\preo{\sigma_1}}\inv \circ p|_{A_1\preo{\sigma_2}}:
A_1\preo{\sigma_2} \to A_1\preo{\sigma_1}$. Now define

$\Sigma_1' = \Sigma_1 \setminus \set{\sigma_2}$,
$N_1' = N_1$,
$H_1' = H_1 \setminus A_1\preo{\sigma_2}$,
$E_1' = E_1$,
$K_1' = K_1$,

\smallskip

$\forall\sigma\from\Sigma_1\ \mu(\sigma) = \cases{
\sigma_1 & if $\sigma=\sigma_2$ \cr
\sigma & otherwise
}$,
$\forall h\from H_1\ \mu(h) = \cases{
\gamma(h) & if $A_1(h) = \sigma_2$ \cr
h & otherwise}$,

\smallskip

$\forall x\from N_1\cup E_1\cup K_1\ \mu(x) = x$

$\forall\sigma\from\Sigma_1'\ W_1'(\sigma) = \sigma$,
$\forall n\from N_1'\ W_1'(n) = \mu(W_1(n))$,

$P_1' = \mu \circ P_1$,
$A_1' = A_1|_{H_1'}$,
$F_1' = \mu \circ F_1$,
$S_1' = \mu \circ S_1$,
$C_1' = C_1$,

$G_1' = \overline\mu \circ G_1 \circ \overline\mu\inv$.

\medbreak\f
This gives the network $\N_1'$ and homomorphism $\mu:\N_1\to\N_1'$. 

Note that $\mu$ is surjective and satisfies 
$\forall x,y\from\Sigma_1\cup N_1\cup H_1\cup
E_1\cup K_1\ (\mu(x)=\mu(y) \imp p(x)=p(y))$, so there exists a unique
function $p'$ such that $p'\circ\mu = p$; this $p'$ is a homomorphism from
$\N_1'$ to $\N_0$. This is the new parse.

If $u$ is the old embedding token on $\N_1$, we can define a new embedding
token $u'$ on $\N_1'$ by
$$ \forall\sigma\from\Sigma_1'\ u'(\sigma) = \cases{
G & if $\sigma=\sigma_1$ \cr
u(\sigma) & otherwise},
\quad
\forall n\from N_1'\ u'(n) = u(n) $$
where $G$ is an affine transformation intermediate between $u(\sigma_1)$ and
$u(\sigma_2) \cdot s$. This is calculated as follows. Find $A\from\A$ such that 
$u(\sigma_2) \cdot s \cdot u(\sigma_1)\inv = \exp(A)$; then choose $G
= \exp(A/2) \cdot u(\sigma_1) = \exp(-A/2) \cdot u(\sigma_2) \cdot s$.

No consistent pair of inclusion functions
$(i',j')$ can be specified for the new network $\N_1'$, so we recalculate 
them as in \S7.4, using the restriction of the old inclusion functions $(i,j)$
to $\N_1'$ as a starting point.

\subhead{8.7 Partitioning a symbol token into two}
Consider any pattern $\N_1=\network{_1}$.
For any $\sigma_0\from\Sigma_1$, if the nodes
and symbol in $W_1\preo{\sigma_0}$ can be partitioned into two disjoint non-empty
subsets $T_1,T_2$, such that there is no edge between any element $T_1$ and
any element of $T_2$, then $\sigma_0$ may be replaced by two symbols, 
$(\sigma_0,1)$ and
$(\sigma_0,2)$, with $(\sigma_0,1)$ getting the nodes of $T_1$ and
$(\sigma_0,2)$ getting the nodes of $T_2$. The subsymbols of $\sigma_0$ are
glued to $(\sigma_0,1)$ or $(\sigma_0,2)$ as appropriate (or duplicated if
necessary). The nodes above $\sigma_0$
must be duplicated; i.e., $n$ is replaced by $(n,i)$ and $(n,j)$, for
two indices $i,j$, and
likewise for their hooks, edges and facets.
This operation is called
\i{partitioning $\sigma_0$}. It is roughly the inverse of the merging operation.

\defn In a network $\network{}$, a symbol $\sigma_0\from\Sigma$ is 
\i{partitionable} iff there exist sets $T_1,T_2$ such that 
$T_1 \cup T_2 = W\preo{\sigma_0}$ and $T_1 \cap T_2 = \emptyset$ and
$T_1,T_2 \ne \emptyset$
and 
$F\pre{A\pre{T_1}} \cap S\pre{A\pre{T_2}} = \emptyset$ and 
$S\pre{A\pre{T_1}} \cap F\pre{A\pre{T_2}} = \emptyset$.

The network $\network{}$ is \i{partitionable} iff at least one symbol in
$\Sigma$ is partitionable; otherwise it is \i{unpartitionable}.

\defn If a symbol $\sigma_0$ is partitionable in $\N=\network{}$, with sets
$T_1,T_2$, then \i{partitioning $\sigma_0$} is the construction of a new
network $\N'$ as follows.

First define a function $I$ on $\Sigma\cup N\cup E$ by

\blob $I(\sigma_0) = \set{1,2}$,

\blob $\forall n\from N \cap T_1\ (I(n) = \set 1 \times I(P(n)) \and \forall n^*\ (G(n,n^*)
\imp I(n^*) = I(n)))$

\blob $\forall n\from N \cap T_2\ (I(n) = \set 2  \times I(P(n))\and \forall n^*\ (G(n,n^*)
\imp I(n^*) = I(n)))$

\blob $\forall \sigma^*\ (G(\sigma_0,\sigma^*) \imp I(\sigma^*) =
\bigcup_{n\in N \cap W\preo{\sigma^*}} proj_1(I(n)))$

\blob for all other $\sigma\from\Sigma$, $I(\sigma) = \set 0$,

\blob for all other $n\from N$, $I(n) = I(W(n)) \times I(P(n))$,

\blob $\forall e\from E\ I(e) = I(A(F(e))) \times I(A(S(e)))$,

\medskip\f where the function $proj_1$ is defined by $\forall(i,j)\
proj_1(i,j) = i$.

Define the new network $\N'=\network{'}$, by

\blob $\Sigma' = \comp{(\sigma,i)}{\sigma\from\Sigma \and i \in I(\sigma)}$,
$N' = \comp{(n,i)}{n\from N \and i \in I(n)}$,

\blob $H' = \comp{(h,i)}{h\from H \and i \in I(A(h))}$,
$E' = \comp{(e,i)}{e\from E \and i \in I(e)}$,

\blob $K' = \comp{(k,i)}{k\from K \and i \in I(C(k))}$,

\blob $\forall(\sigma,i)\from\Sigma'\ W'(\sigma,i) = (\sigma,i)$,
$\forall(n,(i,j))\from N'\ W'(n,(i,j)) = (W(n),i)$,

\blob $\forall(n,(i,j))\from N'\ P'(n,(i,j)) = (P(n),j)$,
$\forall(h,i)\from H'\ A'(h,i) = (A(h),i)$,

\blob $\forall(e,(i,j))\from E'\ F'(e,(i,j)) = (F(e),i)$,
$\forall(e,(i,j))\from E'\ S'(e,(i,j)) = (S(e),j)$,

\blob $\forall(k,i)\from K'\ C'(k,i) = (C(k),i)$,

\blob $\forall(\sigma,i),(\sigma^*,j)\from \Sigma'\ (G'((\sigma,i),(\sigma^*,j))
\iff G(\sigma,\sigma^*) \and c(i,j))$,

\blob $\forall(n,i),(n^*,j)\from N'\ (G'((n,i),(n^*,j)) 
\iff G(n,n^*) \and c_2(i,j))$,

\blob $\forall(h,i),(h^*,j)\from H'\ (G'((h,i),(h^*,j)) 
\iff G(h,h^*) \and c_2(i,j))$,

\blob $\forall(e,i),(e^*,j)\from E'\ (G'((e,i),(e^*,j)) 
\iff G(e,e^*) \and c_4(i,j))$,

\blob $\forall(k,i),(k^*,j)\from K'\ (G'((k,i),(k^*,j)) 
\iff G(k,k^*) \and c_4(i,j))$,

\medskip\f
where 
$$\eqalign{
c(i,j) \ &\iff\  i=j \OR i=0 \cr
c_2((i,j),(k,l)) \ &\iff\  c(i,k) \and c(j,l) \cr
c_4((i,j),(k,l)) \ &\iff\  c_2(i,k) \and c_2(j,l). \cr
}$$
\medskip\f
Define a homomorphism $\pi:\N'\to\N$ by
$\forall(x,i)\from \Sigma'\cup N' \cup H' \cup E' \cup K'\
\pi(x,i) = x$.

\medbreak

During the recognition process any partitionable symbol in the pattern $\N_1$
may be partitioned, producing a new network $\N_1'$, with a homomorphism
$\pi:\N_1'\to\N_1$. The parse $p:\N_1\to\N_0$ becomes $p\circ\pi:\N_1'\to\N_0$
and the embedding token $u$ becomes $u \circ \pi$.
The new pair of inclusion functions is $(i\circ\pi,j\circ\pi)$.

\ignore{
In a network $\N=\network{}$, with an embedding token $u$, if a symbol
$\sigma\from\Sigma$ is partitionable then the operation of \i{partitioning
$\sigma$} produces a network $\N'=\network{'}$ and an embedding token $u'$
defined as follows.

$\Sigma' = (\Sigma_1\setminus\{\sigma\}) \cup \set{(\sigma,1),(\sigma,2)}$, 

$N' = (N \setminus N^*) \ \cup\ \comp{(n,1),(n,2)}{n \in N^*}$, 
where $N^* = P\preo\sigma$

$H' = (N \setminus H^*) \ \cup\ \comp{(h,1),(h,2)}{h \in H^*}$, 
where $H^* = A\pre{N^*}$.

$E' = (E \setminus E^*)
\ \cup\ \comp{(e,1),(e,2)}{e \in E^*}$,
where $E^* = F\pre{H^*} \cup S\pre{H^*}$

$K' = (K \setminus K^*)
\ \cup\ \comp{(k,1),(k,2)}{k \in K^*}$,
where $K^* = C\pre{E^*}$

Define $W':N'\cup\Sigma'\to\Sigma'$ by
$$\eqalign{
\forall n\from N\ W_1'(n) &= \cases{
(\sigma,1) & if $n \in N_1$ \cr
(\sigma,2) & if $n \in N_2$ \cr
\sigma & if $n \notin W\preo\sigma$
} \cr
\forall \sigma\from\Sigma'\ W'(\sigma) &= \sigma
}$$

Define $P':N'\to\Sigma'$ by

Again.

Define an index-generating function $I:\Sigma\cup N\cup E \to 
{\Cal P}({\Bbb N})$ by
$$\eqalign{
\forall \sigma^* \from \Sigma\ I(\sigma^*) &= \cases{
\set{1,2} & if $\sigma^*=\sigma$ \cr
\set{0} & if $\sigma^*\ne\sigma$
} \cr
\forall n\from N\ I(n) &= \cases{
\set{1,2} & if $n\in N^*$, where $N^* = P\preo\sigma$ \cr
\set{1} & if $n\in N_1$ \cr
\set{2} & if $n\in N_2$ \cr
\set{0} & otherwise
} \cr
\forall e\from E\ I(e) &= \cases{
\set{1,2} & if $e\in E^*$, where $E^* = F\pre{H^*} \cup S\pre{H^*}$ \cr
\set{0} & if $e \notin E^*$
}
}$$
Then define
$$\eqalign{
\Sigma' &= \comp{(\sigma^*,i)}{\sigma^* \in \Sigma \and i \in
I(\sigma^*)} \cr
N' &= \comp{(n,i)}{n \in N \and i \in I(n)} \cr
H' &= \comp{(h,i)}{h \in H \and i \in I(A(h))} \cr
E' &= \comp{(e,i,j)}{e \in E \and i \in I(A(F(e))) \and j \in I(A(S(e)))} \cr
K' &= \comp{(k,i,j)}{k \in K \and (C(k),i,j) \in E'}
}$$
Define $W':N'\cup\Sigma'\to\Sigma'$ by 
$$ \forall (n,i)\from N'\cup\Sigma'\ W'(n,i) = (W(n),i). $$
Define $P':N'\to\Sigma'$ by *** WRONG
$$ \forall (n,i)\from\Sigma'\ P'(n,i) = (P(n),i). $$
Define $A':H'\to N'\cup\Sigma'$ by
$$ \forall (h,i)\from H'\ A'(h,i) = (A(h),i). $$ 
Define $F':E'\to H'$ by
$$ \forall (e,i,j)\from E'\ F'(e,i,j) = (F(e),i). $$ 
Define $S':E'\to H'$ by
$$ \forall (e,i,j)\from E'\ S'(e,i,j) = (S(e),j). $$ 
Define $C':K'\to E'$ by
$$ \forall (k,i)\from K'\ C'(k,i) = (C(k),i). $$ 

DON'T FORGET G!

Define the new embedding token $u':N'\cup\Sigma'\to\G$ by 
$$\eqalign{
\forall (n,i) \from N'\ u'(n,i) &= u(n) \cr
\forall (\sigma,i) \from \Sigma'\ u'(\sigma,i) &= u(\sigma).
}$$

ignore}

\theorem 46. If $\N=\network{}$ is an unpartitionable network satisfying the
condition $W \circ A \circ F = W \circ A \circ S$ then
$E \doublearrow{A \circ F}{A \circ S}
N\cup\Sigma \buildrel W \over \rightarrow \Sigma$ is a coequaliser
diagram in the category of sets.

\proof Consider any set $X$ and function $\alpha:N\cup\Sigma\to X$ such that
$\alpha \circ A \circ F = \alpha \circ A \circ S$. We must show that
there exists a unique function $\mu:\Sigma\to X$ such that $\alpha = 
\mu \circ W$.

Define $\mu = \alpha|_\Sigma$. 
Consider any symbol $\sigma\from\Sigma$. 

Define $T_1 = \comp{x\from
W\preo\sigma}{\alpha(x)=\alpha(\sigma)}$ and $T_2 = \comp{x\from
W\preo\sigma}{\alpha(x)\ne\alpha(\sigma)}$. Then $T_1 \cup T_2 = 
W\preo\sigma$ and $T_1 \cap T_2 = \emptyset$.
Note also that $\sigma \in T_1$, so $T_1 \ne \emptyset$.

Since $W \circ A \circ F = W \circ A \circ S$ and
$\alpha \circ A \circ F = \alpha \circ A \circ S$ we have, for any
$e\from E$,
$$\eqalign{
e \in F\pre{A\pre{T_1}} \ &\iff\ A(F(e)) \in T_1 
\ \iff\ W(A(F(e))) = \sigma \and \alpha(A(F(e))) = \alpha(\sigma)
\cr
\ &\iff\ W(A(S(e))) = \sigma \and \alpha(A(S(e))) = \alpha(\sigma)
\ \iff\ A(S(e)) \in T_1
\cr
\ &\iff\ e \in S\pre{A\pre{T_1}}  
}$$
so $F\pre{A\pre{T_1}} = S\pre{A\pre{T_1}}$, and similarly
$F\pre{A\pre{T_2}} = S\pre{A\pre{T_2}}$.
Then
$$\eqalign{
F\pre{A\pre{T_1}} \cap S\pre{A\pre{T_2}}
&= F\pre{A\pre{T_1}} \cap F\pre{A\pre{T_2}}
= F\pre{A\pre{T_1 \cap T_2}}
\cr&
= F\pre{A\pre{\emptyset}}
= \emptyset 
}$$
and similarly $S\pre{A\pre{T_1}} \cap F\pre{A\pre{T_2}} = \emptyset$.

So all the conditions for $\sigma$ to be partitionable have been verified,
except $T_2 \ne \emptyset$. But $\sigma$ is not partitionable, by hypothesis,
so $T_2 = \emptyset$. This means that
$\forall n\from W\preo\sigma\ \alpha(n)=\alpha(\sigma) = \mu(W(n))$.

Since we have shown this for arbitrary $\sigma\from\Sigma$ we have
$\forall n\from N \cup \Sigma\ \alpha(n) = \mu(W(n))$, i.e.,
$\alpha = \mu \circ W$, as required.

Conversely, consider any function $\mu:\Sigma\to X$ such that 
$\alpha = \mu \circ W$. Then $\forall\sigma\from\Sigma\ \alpha(\sigma) =
\mu(W(\sigma)) = \mu(\sigma)$, so $\mu = \alpha|_{\Sigma}$. This shows
that $\mu$ is unique. 

This completes the verification of the coequaliser condition. \qed

\subhead{8.8 The outcome of the recognition process}
The recognition process must ensure that, at the end, the pattern $\N_1$,
the homomorphism $p:\N_1\to\N_0$, the inclusion functions $i,j$, and the
embedding token $u$ satisfy the conditions

\blob $\forall x\from \Sigma_1 \cup N_1 \cup E_1 \ i(x) \in \{0, 1\}$,

\blob $\N_1$ is unprunable, given $(i,j)$,

\blob $(\N_1,p,u)$ is inextendable, given $i,j,v,B$,

\blob $\N_1$ is unpartitionable,

\blob $W_1 \circ A_1 \circ F_1 = W_1 \circ A_1 \circ S_1$,

\blob $\forall\sigma\from\Sigma_1\setdiff P_1(N_1)\ B(\sigma) = \theta$.

\medskip\f
It will be shown in \S9.6 that these conditions imply that $\forall
x\from\Sigma_1\cup N_1\cup E_1\ i(x) = 1$ and $\N_1$ is definite; hence the
recognition process is finished.
