# Supplementary material for: A New Graph Grammar Formalism for Robust Syntactic Pattern Recognition
Source: arXiv:2504.15975 source file (2025-04-24)
Supplement: Supplementary file 9 [file supp9.tex]

\runninghead{9. The whole recognition process}

\head{9. The Whole Recognition Process}

\subhead{9.1 Introduction}
This section completes the account of recognition by filling in some missing
details: the line operations, the determination of
temperature, the determination of the bareness function, and the halting
condition.

At the end of recognition the pattern should be definite and all the symbols',
nodes' and edges' inclusion values should be $1$. Previous sections have stated
various sufficient conditions for this to be the case. Now I shall show that
(under some mild assumptions) these conditions are indeed satisfied at the end
of recognition, and that the definite match function $DM$ is maximised.

\subhead{9.2 Line operations}
I shall assume the grammar contains a symbol type
called \i{line}; symbol tokens of this type are called lines. Geometrically
they are infinitely thin line segments, and their embeddings are always
similarities. Parsing starts with a set of randomly arranged lines, symbols of
other types being built up from there. There is no necessary reason to start
with lines, but it is convenient for a wide range of examples, so I shall
provide some special operations for dealing with lines.

\item{(a)} Create a line. A line symbol token $\sigma$ is created; its
initial embedding $u(\sigma)$ is chosen by a random search aiming to maximise
$\rho_{I,T,sat}(u(\sigma))$. This operation is applied throughout recognition
(though mostly at the start when most of the image is not covered by symbol
tokens).

\item{(b)} Randomise a line. If a line's inclusion value falls too low, and
it is bare (not part of another symbol token), a new random embedding transformation is
chosen for it by the same method as in (a).

\item{(c)} Remove a bare line. If a line is not part of another symbol and
its temperature falls below a threshold, it has a small probability of being
removed. The purpose of this is to tidy up the pattern by removing lines that
have not been incorporated into higher-level symbols.

\item{(d)} Glue two lines together, end to end. If two lines are nearly
collinear, with an end of one line close to an end of the other, as measured by
a fleximap, the two lines are replaced by a single large line. Their bars are
connected together, end to end.

\ignore{

\itemitem{(e)} Split a line. A line is divided into two lines. This occurs if
its template value $\rho_{I',tem(\sigma),sat}(u(\sigma))$ would be improved by
doing so and it is not part of another symbol.

}

\def\spread{\mathrel{\mapstochar\Rightarrow}}
\def\sspread{\mathrel{\Leftarrow\kern-3pt\mapstochar\kern-2pt\Rightarrow}}

\subhead{9.3 How temperature is determined}
Every symbol token, node token, hook token, edge token and facet token has a
temperature. These change continually by the following three processes. (There 
are two parameters controlling the spread of temperature across the network,
$\beta=0.3$ and $\gamma=0.2$. The notation $X \spread
Y$ means the assignment statement $Y \assign \max(X,Y)$, and $X \sspread Y$
means $X \spread Y$ and $Y \spread X$.)

\medskip

\item{1.} Every symbol, node, hook, edge or facet token created by a line
operation or an extension operation is given a high initial temperature.

\medskip

\item{2.} Temperature is spread through the pattern by applying the following
operations periodically.

\blob For every hook $h\from H_1$, do $T_{A_1(h)} \spread T_h$; $\beta T_h \spread
T_{A_1(h)}$.

\blob For every edge $e\from E_1$, do $T_{F_1(e)} \sspread T_e$; $T_{S_1(e)}
\sspread T_e$.

\blob For every node $n\from N_1$, do

\indent\indent $T_{P_1(n)} \spread T_n$; $\gamma T_n \spread T_{W_1(n)}$;

\indent\indent if $n\in\dom(G_1)$ then
$\gamma T_{W_1(n)} \spread T_n$ else $\gamma T_n \spread T_{P_1(n)}$.

\blob For every pair $k,k^*\from K_1$ such that $G_1(k,k^*)$, do $T_k \sspread
T_{k^*}$.

\blob For each $k\from K_1$, do $T_{C_1(k)} \sspread T_k$.

\medskip

\item{3.} Periodically each temperature $T$ declines by the formula
$$ T \assign a + \eta T $$
where the constant $\eta$ is slightly below $1$ and the constant $a$ is small
and positive. In the absence of other temperature changes all temperatures will
converge to $T_{min}=a/(1-\eta)$. The value of $a$ is chosen so as to give a 
desired minimum temperature, $T_{min}$.

\medskip\f
The temperatures perform a simulated annealing function. Wherever the structure
of the pattern changes, temperature is increased, by process~1\ignore{; wherever
the geometry changes, temperature is increased, by process 2}. These increases
in temperatures are spread to neighbouring parts of the pattern, by process~2.
In the absence of changes in the structure the temperature will decline, by
process~3. The general effect of this is that rapidly changing areas of the
pattern will be hot, and areas that have settled down will become cold.

Where the pattern is hot the inclusion values will take mid-range values; this
allows rival grammatical possibilities to co-exist. Where the pattern is cold
the inclusion values tend to be driven towards $0$ or $1$, and this forces a
choice to be made between the rival grammatical possibilities, leading to a
definite pattern.

As recognition finishes, structural and geometric changes cease and the temperature
declines to $T_{min}$ throughout the pattern. All the inclusion values are
likely to approach $0$ or $1$. However, this is not guaranteed; it is possible
to construct a network in which there is no consistent final assignment of $0$
or $1$ inclusion values, except for the trivial solution in which all inclusion
values are $0$ (consider, for example, the case of an edge that is connected to
the same hook at both ends where the hook has no other incident edges).
Nevertheless, in realistic cases the inclusion values do go to $0$ or $1$, and
this will be assumed in what follows.

\subhead{9.4 How the bareness function $B$ is determined}
For each $h\from H_1$, $B(h)$ is initially $0$ and increases by a fixed amount
every time an extension operation is applied that adds edges to $F_1\preo h \cup
S_1\preo h$.

For each $k\from K_1$, $B(k)$ is initially $0$ and increases by a fixed amount
every time an extension operation is applied that adds facets to $\comp{k^*\from
K_1}{G_1(k,k^*)}$.

For each $\sigma\from\Sigma_1$, if $P_0\pre{p(\{\sigma\})} = \emptyset$ then
$B(\sigma)$ is initially set to $\theta$ (where $\theta$ is the constant used in
the $DM$ function), and never changes thereafter. If $P_0\pre{p(\{\sigma\})} \ne
\emptyset$ then $B(\sigma)$ is initially set to a positive value $\theta_0 <
\theta$; $B(\sigma)$ is increased by a fixed amount every time extension
operation (a), (b), (e) or (g) is applied that adds nodes to $P_1\preo\sigma$.
The increment is chosen so that $\theta-\theta_0$ is a multiple of the
increment.

The purpose of all this is to prevent the recognition algorithm from getting stuck
in an infinite loop by trying the same thing over and over again. Suppose a hook
$h$ is bare, and then edges are added to it by the operation of extending from
$h$, then the edges are removed by a pruning operation; and this is repeated
indefinitely. The value of $B(h)$ will increase each time edges are added,
making the algorithm more and more unwilling to remove all the edges and leave
the hook bare. Eventually the algorithm will either keep an edge or remove the
node $A(h)$ altogether; either way, the infinite loop is averted. Likewise, the
monotonic increase in $B(k)$ prevents the algorithm from repeatedly adding and
removing sub-facets to $k$ forever.

The monotonic increase in $B(\sigma)$ prevents the algorithm from making any
further attempts to add nodes above $\sigma$ using extension operations (a),
(b), (e) or (g), once $B(\sigma)$ has increased to $\theta$. It follows that
$B(\sigma)$ can never increase above $\theta$. Throughout recognition we have 
$$ \forall\sigma\from\Sigma_1\ B(\sigma) \le \theta, \text{ with equality if }
P_0\pre{p(\{\sigma\})} = \emptyset. \eqno(1) $$
At the end of recognition all the $B(\sigma)$ values for bare symbol tokens
$\sigma$ should equal $\theta$. This is ensured by the following theorem.

\theorem 47. If

\item{(a)} $\N_1=\network{_1}$ is a definite network satisfying
$W_1 \circ A_1 \circ F_1 = W_1 \circ A_1 \circ S_1$,

\item{(b)} $p:\N_1\to\N_0$ is a homomorphism, where $\N_0=\network{_0}$ is a
semi-definite network,

\item{(c)} $(i,j)$ is a pair of inclusion functions on $\N_1$ satisfying
$\forall x\from \Sigma_1\cup N_1\cup E_1\ i(x) = 1$,

\item{(d)} $u$ is an embedding token for $\N_1$ and $v$ is an embedding type
for $\N_0$,

\item{(e)} $B$ is a bareness function for $\N_1$ satisfying
$\forall\sigma\from\Sigma_1\ B(\sigma) \le \theta, \text{ with equality if }
P_0\pre{p(\{\sigma\})} = \emptyset$,

\item{(f)} $(\N_1,p,u)$ is inextendable, given $i,j,v,B$,

\smallskip\f
then

\smallskip

\item{} $\forall\sigma\from\Sigma_1\setdiff P_1(N_1)\ B(\sigma) = \theta$.

\proof Consider any $\sigma\from\Sigma_1\setdiff P_1(N_1)$. In view of
hypotheses (a) and (c), and the fact that $\sigma\notin P_1(N_1)$, theorem~32 tells
us that $j(\sigma)=1$. Now, if $P_0\pre{p(\{\sigma\})} = \emptyset$ then
$B(\sigma)=\theta$ by hypothesis~(e). Suppose, on the other hand,
$P_0\pre{p(\{\sigma\})} \ne \emptyset$. Then hypothesis~(e) gives
$B(\sigma)\le\theta$. Suppose that $B(\sigma) < \theta$. Then, since
$j(\sigma)=1$, extension operation~(e) is possible, giving an extension
$(\N_1',p',u')$ of $(\N_1,p,u)$ such that $p'({P_1'}\pre{\{\sigma\}}) =
P_0\pre{p(\{\sigma\})}$. However hypothesis~(f) tells us that this is a
trivial extension, so 
$(\N_1',p',u')=(\N_1,p,u)$. This means $p(P_1\pre{\{\sigma\}}) =
P_0\pre{p(\{\sigma\})}$. But this is impossible: the left-hand side is empty,
since $\sigma\notin P_1(N_1)$, but the right-hand side is non-empty. This
contradiction establishes that $B(\sigma)=\theta$, as required. \qed

\subhead{9.5 Summary of the entire recognition process}
The input to the parser is an image $I$, a semi-definite network $\N_0$
(representing a grammar), and an embedding type $v$ for $\N_0$. During 
recognition, a network $\N_1$ (representing a pattern), a homomorphism $p:\N_1\to\N_0$, a
pair of inclusion functions $(i,j)$, an embedding token $u$, and a bareness
function $B$ for $\N_1$ are constructed.

The recognition process is a sequence of steps, called \i{cycles}. In each
cycle,

\blob $i$ and $j$ are recalculated (\S7.4);

\blob $u$ is adjusted (subject to the symmetry condition) to increase
$IM(I, \N_1, u, v\circ p, i, j, B)$ (\S6.5);

\blob all temperatures spread and decline a little (\S9.3);

\blob structural operations are applied to $\N_1$ if the conditions are
satisfied (elementary pruning
operations, extension operations, merging two symbol tokens, and partitioning
a symbol token into two); every new symbol, node, hook, edge or facet is given
a high temperature (\S9.3), and some bareness values are increased
after an extension operation (\S9.4);

\blob line operations are applied to $\N_1$ (\S9.2).

\medskip\f
The algorithm halts when

\blob no further structural operations are possible (except for trivial
extensions);

\blob the temperatures have declined very close to the minimum $T_{min}$.

\subhead{9.6 The outcome of recognition}
At the end of recognition, condition (1) will hold (since it holds throughout
recognition); also, the pattern $\N_1=\network{_1}$ and the inclusion functions
$i,j$ are likely to satisfy the condition
$$ \forall x\from \Sigma_1 \cup N_1 \cup E_1 \ i(x) \in \{0, 1\}. \eqno(2) $$
This is likely because the lowering of temperature at the end of recognition pushes
all inclusion values to $0$ or $1$.

Also, the condition
$$ W_1 \circ A_1 \circ F_1 = W_1 \circ A_1 \circ S_1. \eqno(3) $$
is likely to hold. This is because the term
$E_{in(p(W_1(A_1(F_1(e)))))}(u(W_1(A_1(S_1(e))))\inv \cdot u(W_1(A_1(F_1(e)))))$
in $IM(I, \N_1, u, v\circ p, i, j, B)$ penalises any edge $e\from E_1$ for which
$W_1(A_1(F_1(e))) \ne W_1(A_1(S_1(e)))$. The penalty is large and increases in
effect as temperature falls. This term generates a force that pulls the two
symbols $W_1(A_1(F_1(e)))$ and $W_1(A_1(S_1(e)))$ closer together; eventually,
either they will merge or $i(e)$ will fall so low that $e$ is pruned.

Conditions (2) and (3) are not guaranteed to hold, but they can be expected to
hold in practice. Assuming they do hold we can apply the following theorem.

\theorem 48. If

\item{(a)} $\N_1=\network{_1}$ is a network satisfying
$W_1 \circ A_1 \circ F_1 = W_1 \circ A_1 \circ S_1$,

\item{(b)} $p:\N_1\to\N_0$ is a homomorphism, where $\N_0=\network{_0}$ is a
semi-definite network,

\item{(c)} $(i,j)$ is a pair of inclusion functions on $\N_1$ satisfying
$\forall x\from \Sigma_1 \cup N_1 \cup E_1 \ i(x) \in \{0, 1\}$,

\item{(d)} $u$ is an embedding token for $\N_1$ and $v$ is an embedding type
for $\N_0$,

\item{(e)} $B$ is a bareness function for $\N_1$ satisfying
$\forall\sigma\from\Sigma_1\ B(\sigma) \le \theta, \text{ with equality if }
P_0\pre{p(\{\sigma\})} = \emptyset$,

\item{(f)} $\N_1$ is unprunable, given $(i,j)$,

\item{(g)} $(\N_1,p,u)$ is inextendable, given $i,j,v,B$,

\item{(h)} $\N_1$ is unpartitionable,

\smallskip\f
then

\smallskip

\item{(1)} $\N_1$ is definite,

\item{(2)} $\forall x\from \Sigma_1\cup N_1\cup E_1\ i(x) = 1$,

\item{(3)} $IM(I,\N,u,v,i,j,B) = DM(I,\N,u,v)$.

\proof Theorem~46, using hypotheses~(a,h), tells us that

\item{(i)} $E_1 \doublearrow{A_1 \circ F_1}{A_1 \circ S_1}
N_1\cup\Sigma_1 \buildrel W_1 \over \rightarrow \Sigma_1$ is a coequaliser
diagram in the category of sets. 

\smallskip\f
Theorem~42, using hypotheses~(c,f), gives 

\item{(j)} $\forall e\from E_1\ i(e)=1$. 

\smallskip\f
So theorem~45, using hypotheses~(a,c,g) and (j), gives

\item{(k)}
$\forall h\from H_1\ j(h)=0$ and $\forall k\from K_1\setdiff\dom(G_1)\ j(k)=0$.

\smallskip\f
Then theorem~44, using hypotheses~(c,f) and (i,k), gives conclusions~(1,2).

\smallskip\f
Theorem~47, using hypotheses~(a,e,g) and (1,2), then gives

\item{(l)} $\forall\sigma\from\Sigma_1\setdiff P_1(N_1)\ B(\sigma) = \theta$.

\smallskip\f
Conclusion~(3) then follows by theorem~33, using (l) and (1,2). \qed

\medskip\f
As explained in \S6.6 and \S7.5, the algorithm has attempted throughout to
choose $i,j$ to maximise $E$ and to choose $u$ to maximise $IM(I,\N_1,u,v\circ
p,i,j,B)$; as recognition ends this amounts to choosing $i,j,u$ to maximise
$IM(I,\N_1,u,v\circ p,i,j,B)$, and this amounts to
maximising $DM(I,\N_1,u,v\circ p)$ at the end of recognition. Thus the recognition
problem is solved.

It should be noted that there is a number of ways in which recognition can fail.
The core of the theory is provably correct, but the more peripheral parts of
the algorithm are supported only by heuristic arguments (which I have
indicated throughout by use of the word \ic{likely}).

\item{(i)} The algorithm for determining the inclusion functions (\S7.4) is not
guaranteed to halt. It finds only a local maximum of $E$, not a global
maximum.

\item{(ii)} Even for low temperature, maximising $E$ is not precisely the
same as maximising $IM(I, \N_1, \allowbreak u, \allowbreak v\circ p, 
\allowbreak i, \allowbreak j, B)$.

\item{(iii)} The monotonic raising of the bareness function may cut off possible
structural extensions prematurely.

\item{(iv)} Symbol tokens may be merged or not merged, or partitioned or not
partitioned, wrongly. (Errors in merging can be corrected by partitioning and
vice versa.)

\item{(v)} The whole algorithm is not guaranteed to halt.

\item{(vi)} It is not guaranteed that very low temperature will force all
inclusion values to $0$ or $1$.

\item{(vii)} Incoherent edges may survive to the end.

\item{(viii)} Some portions of the image may have been overlooked. 

\medbreak\f
In practice it is only (iii), (iv), (v) and (viii) that matter.
