# Supplementary material for: A New Graph Grammar Formalism for Robust Syntactic Pattern Recognition
Source: arXiv:2504.15975 source file (2025-04-24)
Supplement: Supplementary file 11 [file supp3.tex]

\runninghead{3. Networks and homomorphisms}

\head{3. Networks and Homomorphisms}

\subhead{3.1 Introduction}
My aim is to state formally the \i{recognition problem} (the problem of
interpreting an image using a grammar) and to define the \i{recognition process}
that solves the problem. Because the theory is
complex I shall develop it by stepwise refinement, beginning in this section
with an outline statement of the recognition problem and refining it in the
following section, then building up the recognition process incrementally.

A grammar will be represented by a formal structure called a \i{network},
containing symbol types. Parsing consists of constructing another network called
a \i{pattern}, containing symbol tokens, and establishing a homomorphism from
the pattern network to the grammar network. The grammar must satisfy certain
conditions: it must be a \i{semi-definite} network. The pattern is not bound by
these conditions during recognition, but by the end it must satisfy a
stronger set of conditions: it must be a \i{definite} network. All these
concepts are defined in this section.


\subhead{3.2 Definition of network and homomorphism}

\defn A \i{network} is a 12-tuple $\network{}$, where $\Sigma,N,H,E,K$ are
disjoint finite sets; $W:N\cup\Sigma\to\Sigma$, $P:N\to\Sigma$, $A:H\to
N\cup\Sigma$, $F,S:E\to H$ and $C:K\to E$ are functions such that $\forall
\sigma\from\Sigma\ W(\sigma)=\sigma$; and $G$ is a relation on $\Sigma \cup N
\cup H \cup E \cup K$ such that

\item{(1)} $id_\Sigma \circ G = G \circ id_\Sigma$, $id_N \circ G = G \circ id_N$,
$id_H \circ G = G \circ id_H$, $id_E \circ G = G \circ id_E$, $id_K \circ G = G
\circ id_K$;

\item{(2)} 
$\overline W \circ G = G \circ \overline W$, \ $\overline P \circ G
\subseteq \overline P$, \ $\overline A \circ G \subseteq G \circ \overline A$, \
$\overline F \circ G \subseteq G \circ \overline F$, \ $\overline S \circ G
\subseteq G \circ \overline S$, \ $\overline C \circ G \subseteq G \circ
\overline C$;

\item{(3)} $G_H$ and $G_H\inv$ are minimal relative to $A$;
$G_K$ and $G_K\inv$ are minimal relative to $C$; $G_E$ and $G_E\inv$ are minimal
relative to $F$ and $S$ (where $G_H = G \circ id_H$, $G_K = G \circ id_K$ and
$G_E = G \circ id_E$);

\item{(4)} $G \circ G = \bot$.

\medskip\f
The elements of $\Sigma,N,H,E,K$ are called \i{symbols}, \i{nodes}, \i{hooks},
\i{edges} and \i{facets}, respectively. $G$ is called the \i{gluing relation};
$G(x,y)$ means that $y$ is glued to $x$, i.e., $y$ is a subsymbol, subnode, 
subhook, subedge or subfacet of $x$, i.e., $x$ is a supersymbol, supernode, 
superhook, superedge or superfacet of $y$.
The functions $W,P,A,F,S,C$ express the incidence relations: a node $n$
connects a part $P(n)$ to a whole $W(n)$; a hook $h$ is attached to a node (or
possibly a symbol)
$A(h)$; an edge $e$ runs from its \i{first} hook $F(e)$ to its \i{second} hook
$S(e)$; a facet $k$ belongs to the edge $C(k)$.

The clauses of the definition may be paraphrased informally as follows. 

(1) The gluing relation $G$ may be considered as the disjoint union of a
relation $G_\Sigma = G \circ id_\Sigma$ on symbols, a relation $G_N = G \circ
id_N$ on nodes, a relation $G_H = G \circ id_H$ on hooks, a relation $G_E = G
\circ id_E$ on edges, and a relation $G_K = G \circ id_K$ on facets. I shall
always use similar notation below for the parts of a gluing relation of a
network: e.g., if $\network{_2}$ is a network then $G_{2\Sigma} = G_2 \circ
id_{\Sigma_2}$ (the symbol part of $G_2$), $G_{2N} = G_2 \circ id_{N_2}$ (the
node part of $G_2$), etc..

(2) $G$ preserves incidence. e.g., if a hook $h_1$ is glued to a hook $h_2$
then the node $A(h_1)$ is glued to the node $A(h_2)$.  (The first equation also
says that every node of a subsymbol is a subnode.)

(3) A hook is glued to at most one hook of any given node; a facet is glued to
at most one facet of any given edge; and an edge is glued to at most one edge
of any given hook (for each edge direction).

(4) A subsymbol, subnode, subhook, subedge or subfacet cannot be also be a
supersymbol, supernode, superhook, superedge or superfacet.


\defn If $\N_1=\network{_1}$ and $\N_0=\network{_0}$ are networks, a
\i{homomorphism} $p:\N_1\to\N_0$ is a function from $\Sigma_1 \cup N_1 \cup H_1
\cup E_1 \cup K_1$ to $\Sigma_0 \cup N_0 \cup H_0 \cup E_0 \cup K_0$ such that

\item{(1)} $p(\Sigma_1) \subseteq \Sigma_0$, \quad $p(N_1) \subseteq N_0$, \quad
$p(H_1) \subseteq H_0$, \quad $p(E_1) \subseteq E_0$, \quad $p(K_1) \subseteq
K_0$;

\item{(2)} $W_0 \circ p = p \circ W_1$, \quad $P_0 \circ p = p \circ P_1$, \quad
$F_0 \circ p = p \circ F_1$, \quad $S_0 \circ p = p \circ S_1$;

\smallskip

\item{(3)}
$\bigrectangleA{N_0\cup\Sigma_0}{N_1\cup\Sigma_1}{H_0}{H_1}
{p|_{N_1\cup\Sigma_1}}{A_0}{A_1}{p|_{H_1}}$ and
$\bigrectangleA{E_0}{E_1}{K_0}{K_1}{p|_{E_1}}{C_0}{C_1}{p|_{K_1}}$ \ are pullbacks in
the category of sets;

\medskip

\item{(4)} $\overline p \circ G_1 = G_0 \circ \overline p$;

\item{(5)} $G_1$ is minimal relative to $p$.

\medbreak\f
The clauses of this definition may be paraphrased informally as follows. 

(1) $p$ maps symbols to symbols, nodes to nodes, hooks to hooks, edges to
edges, and facets to facets.

(2) $p$ preserves the $W,P,F,S$ incidence functions.

(3) $p$ maps the hooks of any node $n$ bijectively onto
the hooks of $p(n)$, and maps the facets of any edge $e$ bijectively onto the
facets of $p(e)$.

(4) $p$ preserves gluing (i.e., if $G_1(x,y)$ then
$G_0(p(x),p(y))$), and if $p(x)$ is a subsymbol, subnode, subhook, subedge or
subfacet then so is $x$.

(5) The gluings in $\N_1$ are induced by those in $\N_0$, i.e., two things are
glued in $\N_1$ only if they are forced to be by condition~(4).


\theorem 15. If $p:\N_1\to\N_0$ and $q:\N_2 \to \N_1$ are homomorphisms then
so is $p\circ q:\N_2\to\N_0$.

\proof

First,
$$\eqalign{
p(q(\Sigma_2)) &\subseteq p(\Sigma_1) \subseteq \Sigma_0, \quad
p(q(N_2)) \subseteq p(N_1) \subseteq N_0, \quad
p(q(H_2)) \subseteq p(H_1) \subseteq H_0, \quad
\cr
p(q(E_2)) &\subseteq p(E_1) \subseteq E_0, \quad
p(q(K_2)) \subseteq p(K_1) \subseteq K_0,
}$$
as required.

Secondly,
$$\eqalign{
W_0 \circ p \circ q &= p \circ W_1 \circ q = p \circ q \circ W_2, \quad
P_0 \circ p \circ q = p \circ P_1 \circ q = p \circ q \circ P_2, \quad
\cr
F_0 \circ p \circ q &= p \circ F_1 \circ q = p \circ q \circ F_2, \quad
S_0 \circ p \circ q = p \circ S_1 \circ q = p \circ q \circ S_2,
}$$
as required.

Thirdly, $\bigrectangleA{N_0\cup\Sigma_0}{N_1\cup\Sigma_1}{H_0}{H_1}
{p|_{N_1\cup\Sigma_1}}{A_0}{A_1}{p|_{H_1}}$ and
$\bigrectangleA{N_1\cup\Sigma_1}{N_2\cup\Sigma_2}{H_1}{H_2}
{q|_{N_2\cup\Sigma_2}}{A_1}{A_2}{q|_{H_2}}$ are pullbacks, and therefore so is
$\bigrectangleA{N_0\cup\Sigma_0}{N_2\cup\Sigma_2}{H_0}{H_2} {(p\circ
q)|_{N_2\cup\Sigma_2}}{A_0}{A_2}{(p\circ q)|_{H_2}}$. This is proved as follows.
We have
$$ A_0 \circ (p\circ q)|_{H_2}
= A_0 \circ p|_{H_1} \circ q|_{H_2}
= p|_{N_1\cup\Sigma_1} \circ A_1 \circ q|_{H_2}
= p|_{N_1\cup\Sigma_1} \circ q|_{N_2\cup\Sigma_2} \circ A_2
= (p\circ q)|_{N_2\cup\Sigma_2} \circ A_2. $$
Also, for any set $X$ and functions $f:X \to H_0$ and $g:X \to N_2 \cup
\Sigma_2$ such that $A_0 \circ f = (p\circ q)|_{N_2\cup\Sigma_2} \circ g$, by
the first pullback there exists a unique $i:X \to H_1$ such that $p|_{H_1} \circ
i = f$ and $A_1 \circ i = q|_{N_2\cup\Sigma_2} \circ g$. Then, by the second
pullback, there exists a unique $j:X \to H_2$ such that $q|_{H_2} \circ j = i$
and $A_2 \circ j = g$. Thus $j$ satisfies the desired equations $(p \circ
q)|_{H_2} \circ j = f$ and $A_2 \circ j = g$. To show that $j$ is the only such
function, consider any function $k:X \to H_2$ such that $(p \circ q)|_{H_2}
\circ k = f$ and $A_2 \circ k = g$. Then $p|_{H_1} \circ q|_{H_2} \circ k = f$
and $A_1 \circ q|_{H_2} \circ k = q|_{N_2\cup\Sigma_2} \circ A_2 \circ k =
q|_{N_2\cup\Sigma_2} \circ g$, so, by the uniqueness clause in the first
pullback, $q|_{H_2} \circ k = i$. Then, by the uniqueness clause in the second
pullback, $k=j$. This verifies the required pullback condition.

Similarly, $\bigrectangleA{E_0}{E_1}{K_0}{K_1}{p|_{E_1}}{C_0}{C_1}{p|_{K_1}}\ \
$ and $\bigrectangleA{E_1}{E_2}{K_1}{K_2}{q|_{E_2}}{C_1}{C_2}{q|_{K_2}}\ \ $ are
pullbacks, and hence so is $\bigrectangleA{E_0}{E_2}{K_0}{K_2} {(p\circ
q)|_{E_2}}{C_0}{C_2}{(p\circ q)|_{K_2}}\ $.

Fourthly, $\overline{p\circ q} \circ G_2 = \overline p \circ \overline q \circ
G_2 = \overline p \circ G_1 \circ \overline q = G_0 \circ \overline p \circ
\overline q = G_o \circ \overline{p\circ q}$.

Fifthly, $G_1$ is minimal relative to $p$ and $G_2$ is minimal relative to $q$;
we must show that $G_2$ is minimal relative to $p\circ q$. By theorem~14,
$\overline p\inv \circ \overline p \ \cap\ G_1 \circ G_1\inv \subseteq
id_{\Sigma_1\cup N_1\cup H_1\cup E_1\cup K_1}$ and $\overline q\inv \circ
\overline q \ \cap\ G_2 \circ G_2\inv \subseteq id_{\Sigma_2\cup N_2\cup H_2\cup
E_2\cup K_2}$. Hence,
$$\kern60pt\eqqalign\quad{
&\kern-60pt\overline{p\circ q}\inv \circ \overline{p\circ q} \ \cap\ G_2\circ
G_2\inv
&\cr
&= \overline q\inv \circ \overline p\inv \circ \overline p \circ \overline q
\ \cap\ G_2\circ G_2\inv
&\cr
&\subseteq \overline q\inv \circ \bigl( \overline p\inv \circ \overline p
\ \cap\ \overline q \circ G_2 \circ G_2\inv \circ \overline q\inv \bigr)
\circ \overline q
&\text{by theorem~4(i),(ii)}\cr
&= \overline q\inv \circ \bigl( \overline p\inv \circ \overline p
\ \cap\ G_1 \circ \overline q \circ \overline q\inv \circ G_1\inv \bigr)
\circ \overline q
&\text{since $q$ is a homomorphism}\cr
&\subseteq \overline q\inv \circ \bigl( \overline p\inv \circ \overline p
\ \cap\ G_1 \circ G_1\inv \bigr) \circ \overline q
&\text{by theorem~2(i)}\cr
&\subseteq \overline q\inv \circ id_{\Sigma_1\cup N_1\cup H_1\cup E_1\cup K_1}
\circ \overline q
&\cr
&= \overline q\inv \circ \overline q.
&\cr
}$$
Hence
$$\eqalign{
\overline{p\circ q}\inv \circ \overline{p\circ q} \ \cap\ G_2\circ G_2\inv
&\subseteq \overline q\inv \circ \overline q \ \cap\ G_2\circ G_2\inv
\cr
&\subseteq id_{\Sigma_2\cup N_2\cup H_2\cup E_2\cup K_2}.
}$$
By theorem~14 again, $G_2$ is minimal relative to $p\circ q$, as required. \qed


\theorem 16. If $f:\N\to\N'$ is a homomorphism and is also a bijective
function then the inverse function $f\inv:\N'\to\N$ is a homomorphism (called
the \i{inverse homomorphism} of $f$).

\proof First, the condition $f\inv(\Sigma') \subseteq \Sigma$ follows from
$f(N) \subseteq N'$, $f(H) \subseteq H'$, $f(E) \subseteq E'$ and $f(K)
\subseteq K'$. The similar conditions $f\inv(N') \subseteq N$, $f\inv(H')
\subseteq H$, $f\inv(E') \subseteq E$ and $f\inv(K') \subseteq K$ follow
similarly.

Secondly, the condition $W \circ f\inv = f\inv \circ W'$ is verified by $W \circ
f\inv = f\inv \circ f \circ W \circ f\inv = f\inv \circ W' \circ f \circ f\inv =
f\inv \circ W'$. The similar conditions $P \circ f\inv = f\inv \circ P'$, $F
\circ f\inv = f\inv \circ F'$ and $S \circ f\inv = f\inv \circ S'$ follow
similarly.

Thirdly, the pullback $\rectangleA{N\cup\Sigma}{N'\cup\Sigma'}{H}{H'}
{f\inv|_{N'\cup\Sigma'}}{A}{A'}{f\inv|_{H'}}$ is verified as follows. The
equation $A \circ f\inv|_{H'} = f\inv|_{N'\cup\Sigma'} \circ A'$ is verified as
in the previous paragraph. To verify the other half of the pullback property,
given any set $X$ and functions $p:X\to H$ and $q:X\to N'\cup\Sigma'$ such that
$A \circ p = f\inv|_{N'\cup\Sigma'} \circ q$, define $i=f|_H\circ p:X\to H'$,
giving $f\inv|_{H'} \circ i = f\inv|_{H'} \circ f|_H \circ p = p$ and $A' \circ
i = A' \circ f|_H \circ p = f|_{N\cup\Sigma} \circ A \circ p = f|_{N\cup\Sigma}
\circ f\inv|_{N'\cup\Sigma'} \circ q = q$, as required. To show $i$ is unique,
consider any $j:X\to H'$ such that $f\inv|_{H'} \circ j = p$ and $A' \circ j =
q$; then $j = f|_{H} \circ p = i$, as required.

The pullback $\rectangleA{E}{E'}{K}{K'}{f\inv|_{E'}}{C}{C'}{f\inv|_{K'}}$ is
verified similarly.

\smallskip

Fourthly, the condition $\overline{f\inv} \circ G' = G \circ \overline{f\inv}$
is verified by
$$ \overline{f\inv} \circ G'
= \overline{f\inv} \circ G' \circ \overline{f \circ f\inv}
= \overline{f\inv} \circ G' \circ \overline{f} \circ \overline{f\inv}
= \overline{f\inv} \circ \overline{f} \circ G \circ \overline{f\inv}
= \overline{f\inv \circ f} \circ G \circ \overline{f\inv}
= G \circ \overline{f\inv}. $$

Finally the condition that $G'$ be minimal relative to $f\inv$ is verified as
follows. For any relation $R^* \subseteq G'$, if $\overline{f\inv} \circ R^* =
\overline{f\inv} \circ G'$ then $\overline f \circ \overline{f\inv} \circ R^* =
\overline f \circ \overline{f\inv} \circ G'$, so, since $\overline f \circ
\overline{f\inv} = \overline{f \circ f\inv} = id_{\Sigma'\cup N'\cup H'\cup
E'\cup K'}$, we have $R^*=G'$, as required. \qed


\defn An \i{isomorphism} is a homomorphism $f:\N\to\N'$ with an inverse
homomorphism $f^{-1}:\N'\to\N$. An \i{automorphism} of $\N$ is an isomorphism
from $\N$ to $\N$.


\subhead{3.3 Minimal relations relative to a network}

\defn If $\N=\network{}$ is a network then its gluing relation $G$ is
\i{minimal} relative to $\N$ iff
$$ id_K \subseteq G_K \circ G_K\inv \cup G_K\inv \circ G_K $$
and, for any relation $G^* \subseteq G$ such that

\blob $\overline W \circ G^* \subseteq G^* \circ \overline W$, \ 
$\overline P \circ G^*
\subseteq \overline P$, \ $\overline A \circ G^* \subseteq G^* \circ \overline
A$, \ $\overline F \circ G^* \subseteq G^* \circ \overline F$, \ $\overline S
\circ G^* \subseteq G^* \circ \overline S$, \ $\overline C \circ G^* \subseteq
G^* \circ \overline C$,

\blob $id_K \subseteq G^*_K \circ {G^*_K}\inv \cup {G^*_K}\inv
\circ G^*_K$ (where $G^*_K = G^* \circ id_K$),

\medskip\f
we have $G^* = G$.

\medskip\f
(Informally, the condition that $G$ be minimal relative to $\N$ means that every
facet is glued to another facet (i.e., it is either a subfacet or a
superfacet) and $G$ is as small as it can be, subject to this constraint.)


\theorem 17. For any network $\N=\network{}$,

\item{(i)} if $G$ is minimal relative to $\N$ then
$$\eqqalign\quad{
G_\Sigma &= \overline W \circ G_N \circ \overline W\inv
\ \cup\ id_\Sigma \circ \overline A \circ G_H \circ \overline A\inv,
&G_N = id_N \circ \overline A \circ G_H \circ \overline A\inv,
\cr
G_H &= \overline F \circ G_E \circ \overline F\inv \ \cup\
\overline S \circ G_E \circ \overline S\inv,
&G_E = \overline C \circ G_K \circ \overline C\inv;
\cr} \eqno(*)$$

\item{(ii)} if $G_K \circ G_K\inv \subseteq id_K \subseteq G_K \circ G_K\inv
\cup G_K\inv \circ G_K$ then the converse of (i) holds, i.e., equations $(*)$
imply that $G$ is minimal relative to $\N$.

\proof (i) Suppose $G$ is minimal relative to $\N$. Define a relation $G^* =
G^*_K \cup G^*_E \cup G^*_H \cup G^*_N \cup G^*_\Sigma$, where
$$\eqalign{
G^*_K &= G_K \cr
G^*_E &= \overline C \circ G^*_K \circ \overline C\inv \cr
G^*_H &=
\overline F \circ G^*_E \circ \overline F\inv \cup
\overline S \circ G^*_E \circ \overline S\inv \cr
G^*_N &= id_N \circ \overline A \circ G^*_H \circ \overline A\inv \cr
G^*_\Sigma &= \overline W \circ G^*_N \circ \overline W\inv
\ \cup\ id_\Sigma \circ \overline A \circ G^*_H \circ \overline A\inv.
}$$

First I shall show that $G^* \subseteq G$. We already have $G^*_K = G_K$, but
also
$$\eqalign{
G^*_E
&= \overline C \circ G^*_K \circ \overline C\inv
= \overline C \circ G_K \circ \overline C\inv
= \overline C \circ G \circ \overline C\inv
\subseteq G \circ \overline C \circ \overline C\inv
\subseteq G \circ id_E
= G_E
\cr
G^*_H
&= \overline F \circ G^*_E \circ \overline F\inv \cup
\overline S \circ G^*_E \circ \overline S\inv
\subseteq \overline F \circ G_E \circ \overline F\inv \cup
\overline S \circ G_E \circ \overline S\inv
= \overline F \circ G \circ \overline F\inv \cup
\overline S \circ G \circ \overline S\inv
\cr&
\subseteq G \circ \overline F \circ \overline F\inv \cup
G \circ \overline S \circ \overline S\inv
\subseteq G \circ id_H \cup G \circ id_H
= G_H
\cr
G^*_N
&= id_N \circ \overline A \circ G^*_H \circ \overline A\inv
\subseteq id_N \circ \overline A \circ G_H \circ \overline A\inv
= id_N \circ \overline A \circ G \circ \overline A\inv
\subseteq id_N \circ G \circ \overline A \circ \overline A\inv
\cr&
\subseteq id_N \circ G \circ id_{N\cup\Sigma}
= G_N
\cr
G^*_\Sigma
&= \overline W \circ G^*_N \circ \overline W\inv
\ \cup\ id_\Sigma \circ \overline A \circ G^*_H \circ \overline A\inv
\subseteq \overline W \circ G_N \circ \overline W\inv
\ \cup\ id_\Sigma \circ \overline A \circ G_H \circ \overline A\inv
\cr&
\subseteq \overline W \circ G \circ \overline W\inv
\ \cup\ id_\Sigma \circ \overline A \circ G \circ \overline A\inv
\subseteq G \circ \overline W \circ \overline W\inv
\ \cup\ id_\Sigma \circ G \circ \overline A \circ \overline A\inv
\cr&
\subseteq G \circ id_\Sigma
\ \cup\ id_\Sigma \circ G \circ id_{N\cup\Sigma}
= G_\Sigma \cup G_\Sigma
= G_\Sigma.
}$$
Thus $G^* \subseteq G$ as claimed. Note also that $G^*_K$ is on $K$, $G^*_E$ is
on $E$, $G^*_H$ is on $H$, $G^*_N$ is on $N$, and $G^*_\Sigma$ is on $\Sigma$.

Secondly I shall show that $G^*$ is homomorphic. This follows from
$$\eqqalign\ {
\overline W \circ G^*
&= \overline W \circ (G^*_\Sigma \cup G^*_N) \circ id_{\Sigma \cup N}
&\cr
&\subseteq \overline W \circ (G^*_\Sigma \cup G^*_N) \circ \overline W\inv
\circ \overline W
&\text{by theorem~2(ii)}\cr
&= \overline W \circ G^*_\Sigma \circ \overline W\inv \circ \overline W
\ \cup\ \overline W \circ G^*_N \circ \overline W\inv \circ \overline W
&\text{by theorem~3(i),(ii)} \cr
&\subseteq id_\Sigma \circ G^*_\Sigma \circ id_\Sigma \circ \overline W
\ \cup\ G^*_\Sigma \circ \overline W
&\text{since $\overline{W|_\Sigma}=id_\Sigma$ and $\overline W
\circ G^*_N \circ \overline W\inv \subseteq G^*_\Sigma$} \cr
&= G^*_\Sigma \circ \overline W \ \cup\ G^*_\Sigma \circ \overline W
&\cr
&= G^* \circ \overline W
&\cr
}$$
and
$$\eqqalign\quad{
\overline A \circ G^*
&= id_{N\cup\Sigma} \circ \overline A \circ G^*_H \circ id_H
&\cr
&\subseteq id_{N\cup\Sigma} \circ \overline A \circ G^*_H \circ \overline A\inv
\circ \overline A
&\text{by theorem~2(ii)}\cr
&\subseteq id_N \circ \overline A \circ G^*_H \circ \overline A\inv \circ
\overline A \ \cup\
id_\Sigma \circ \overline A \circ G^*_H \circ \overline A\inv \circ \overline A
&\text{by theorem~3(i)}\cr
&\subseteq G^*_N \circ \overline A \ \cup\ G^*_\Sigma \circ \overline A
&\text{by definition of $G^*_N$ and $G^*_\Sigma$}\cr
&= G^* \circ \overline A
&\cr
}$$
and
$$\eqalign{
\overline P \circ G^*
&\subseteq \overline P \circ G
\subseteq \overline P
\cr
\overline F \circ G^*
&= \overline F \circ G^*_E \circ id_E
\subseteq \overline F \circ G^*_E \circ \overline F\inv \circ \overline F
\subseteq G^*_H \circ \overline F
= G^* \circ \overline F
\cr
\overline S \circ G^*
&= \overline S \circ G^*_E \circ id_E
\subseteq \overline S \circ G^*_E \circ \overline S\inv \circ \overline S
\subseteq G^*_H \circ \overline S
= G^* \circ \overline S
\cr
\overline C \circ G^*
&= \overline C \circ G^*_K \circ id_K
\subseteq \overline C \circ G^*_K \circ \overline C\inv \circ
\overline C
= G^*_E \circ \overline C
= G^* \circ \overline C.
}$$

The relation $G^*$ satisfies the condition
$$ id_K \subseteq
G^*_K \circ {G^*_K}\inv \cup {G^*_K}\inv \circ G^*_K $$
just like $G$. Hence, by the minimality condition, $G^*=G$. This shows that $G$
satisfies the equations $(*)$.

(ii) Suppose that $G_K \circ G_K\inv \subseteq id_K \subseteq G_K \circ G_K\inv
\cup G_K\inv \circ G_K$ and $G$ satisfies the equations $(*)$; we must show that
$G$ is minimal relative to $\N$. Consider any homomorphic relation $G^*
\subseteq G$; we can split $G^*$ into its five parts, $G^*_K = G^* \circ id_K
\subseteq G_K$, $G^*_E = G^* \circ id_E \subseteq G_E$, $G^*_H = G^* \circ id_H
\subseteq G_H$, $G^*_N = G^* \circ id_N \subseteq G_N$, and $G^*_\Sigma = G^*
\circ id_\Sigma \subseteq G_\Sigma$, which are on $K$, $E$, $H$, $N$ and
$\Sigma$ respectively. Assume that $id_K \subseteq G^*_K \circ {G^*_K}\inv \cup
{G^*_K}\inv \circ G^*_K$. We must show $G^* = G$.

First we show $G^*_K=G_K$. This follows from $G^*_K \subseteq G_K$ and
$$\eqqalign\quad{
G_K
&= G_K \circ id_K
\subseteq G_K \circ (G^*_K \circ {G^*_K}\inv \cup {G^*_K}\inv \circ G^*_K)
&\text{since $id_K \subseteq G^*_K \circ {G^*_K}\inv \cup {G^*_K}\inv \circ
G^*_K$}\cr
&= G_K \circ G^*_K \circ {G^*_K}\inv \ \cup\ G_K \circ {G^*_K}\inv \circ G^*_K
&\cr
&\subseteq G \circ G \circ {G^*_K}\inv \ \cup\ G_K \circ G_K\inv \circ G^*_K
&\cr
&\subseteq \bot \ \cup\ id_K \circ G^*_K
&\text{since $G \circ G = \bot$ and $G_K \circ G_K\inv \subseteq id_K$}\cr
&=G^*_K.
&\cr
}$$
Next we have $G^*_E = G_E$, since $G^*_E \subseteq G_E$ and
$$ G_E = \overline C \circ G_K \circ \overline C\inv
= \overline C \circ G^*_K \circ \overline C\inv
= \overline C \circ G^* \circ \overline C\inv
\subseteq G^* \circ \overline C \circ \overline C\inv
\subseteq G^* \circ id_E
= G^*_E. $$
Then $G^*_H = G_H$, since $G^*_H \subseteq G_H$ and
$$\eqalign{
G_H &= \overline F \circ G_E \circ \overline F\inv \cup
\overline S \circ G_E \circ \overline S\inv
= \overline F \circ G^*_E \circ \overline F\inv \cup
\overline S \circ G^*_E \circ \overline S\inv
= \overline F \circ G^* \circ \overline F\inv \cup
\overline S \circ G^* \circ \overline S\inv
\cr&
\subseteq G^* \circ \overline F \circ \overline F\inv \cup
G^* \circ \overline S \circ \overline S\inv
\subseteq G^* \circ id_H \cup G^* \circ id_H
= G^*_H.
}$$
Then $G^*_N = G_N$, since $G^*_N \subseteq G_N$ and
$$\eqalign{
G_N &= id_N \circ \overline A \circ G_H \circ \overline A\inv
= id_N \circ \overline A \circ G^*_H \circ \overline A\inv
= id_N \circ \overline A \circ G^* \circ \overline A\inv
\subseteq id_N \circ G^* \circ \overline A \circ \overline A\inv
\cr&
\subseteq id_N \circ G^* \circ id_{N\cup\Sigma}
= G^*_N.
}$$
Then $G^*_\Sigma = G_\Sigma$, since $G^*_\Sigma \subseteq G_\Sigma$ and
$$\eqalign{
G_\Sigma &= \overline W \circ G_N \circ \overline W\inv
\ \cup\ id_\Sigma \circ \overline A \circ G_H \circ \overline A\inv
= \overline W \circ G^*_N \circ \overline W\inv
\ \cup\ id_\Sigma \circ \overline A \circ G^*_H \circ \overline A\inv
\cr&
\subseteq \overline W \circ G^* \circ \overline W\inv
\ \cup\ id_\Sigma \circ \overline A \circ G^* \circ \overline A\inv
\subseteq G^* \circ \overline W \circ \overline W\inv
\ \cup\ id_\Sigma \circ G^* \circ \overline A \circ \overline A\inv
\cr&
\subseteq G^* \circ id_\Sigma
\ \cup\ id_\Sigma \circ G^* \circ id_{N\cup\Sigma}
= G^*_\Sigma \ \cup G^*_\Sigma
= G^*_\Sigma.
}$$
This completes the proof that $G^* = G$, and so verifies that $G$ is minimal
relative to $\N$. \qed


\subhead{3.4 Semi-definite and definite networks}

\defn A network $\network{}$ is \i{semi-definite} iff

\item{(1a)} $W \circ A \circ F = W \circ A \circ S$,

\item{(3)} $G_N$ is acyclic,

\item{(4a)} $H = F(E) \cup S(E)$,

\item{(5a)} $G_K \circ G_K\inv \subseteq id_K$,

\item{(6)} $G$ is minimal relative to $\N$,

\item{(7a)} $\overline F \circ G = G \circ \overline F$ and
$\overline S \circ G = G \circ \overline S$,

\item{(8a)} $\forall R\ \ (\overline A\inv \circ R = (\overline F \cup \overline S)
\circ R \ \Rightarrow\ G_{\Sigma} \circ R \subseteq \overline W \circ G_N \circ
R \ \cup \ id_\Sigma \circ \overline A \circ G_H \circ \overline A\inv \circ
R)$.


\defn A network $\network{}$ is \i{definite} iff

\item{(1b)} $E \doublearrow{A \circ F}{A \circ S} N\cup\Sigma \buildrel W \over
\rightarrow \Sigma$ is a coequaliser diagram in the category of sets,

\smallskip

\item{(2b)} $G_N$ is connected relative to $P$,

\item{(3)} $G_N$ is acyclic,

\item{(4b)} $E \buildrel F \over \rightarrow H \buildrel S \over \leftarrow E$ is a
sum diagram in the category of sets,

\item{(5b)} $id_K = G_K \circ G_K\inv \cup G_K\inv \circ G_K$,

\item{(6)} $G$ is minimal relative to $\N$.

\medskip\f
The grammar is required to be semi-definite, whereas the pattern is required to
be definite.

The clauses of these two definitions may be paraphrased informally as follows.

(1a) The two nodes at the ends of any edge belong to the same whole. 

(1b) The nodes and edges belonging to any whole form a \i{connected} graph.

(2b) Two nodes share the same part only when they are
glued together (directly or indirectly). (This condition prevents the same
symbol from being interpreted as part of two unrelated wholes.)

(3) There is no cyclic sequence of gluings. This is a
technical condition for ensuring that condition~(2b) holds in the pattern at
the end of recognition (see \S3.6).

(4a) Every hook has at least one incident edge. 

(4b) Every hook has exactly one incident edge.

(5a) Every facet has at most one superfacet. 

(5b) Every facet has exactly one subfacet or superfacet.

(6) Every facet is glued to another facet, but the gluings are minimal subject
to this constraint.

(7a) If any hook is a subhook then all its incident edges are subedges.

(8a) Whenever a subsymbol is glued to a supersymbol, there are sufficiently
many nodes and hooks belonging to the subsymbol that are glued to nodes and
hooks belonging to the supersymbol. This is another technical condition for
ensuring that condition~(2b) holds in the pattern at the end of recognition (it
is used directly in theorem~22 below).

The definiteness conditions subsume the semi-definiteness conditions, as the
following theorem shows.


\theorem 18. Any definite network is semi-definite.

\proof Consider any definite network $\N=\network{}$. We shall verify each of
the conditions for semi-definiteness in turn (reordering them to leave the
harder ones until last).

\medskip\f
$\underline{W \circ A \circ F = W \circ A \circ S.}$ This follows from the fact
that $E \doublearrow{A \circ F}{A \circ S} N\cup\Sigma \buildrel W \over
\rightarrow \Sigma$ is a coequaliser diagram.

\medskip\f
$\underline{\text{$G_N$ is acyclic.}}$ This is given.

\medskip\f
$\underline{H = F(E) \cup S(E).}$ This follows from the fact that $E \buildrel F
\over \rightarrow H \buildrel S \over \leftarrow E$ is a sum diagram.

\medskip\f
$\underline{G_K \circ G_K\inv \subseteq id_K.}$ This follows from the given
condition $id_K = G_K \circ G_K\inv \cup G_K\inv \circ G_K$.

\medskip\f
$\underline{\text{$G$ is minimal relative to $\N$.}}$ This is given.

\medskip\f
$\underline{\text{$\overline F \circ G = G \circ \overline F$ and $S \circ G = G
\circ \overline S$.}}$ This follows by
$$\eqqalign\quad{
G \circ \overline F
&= G \circ id_H \circ \overline F
&\cr
&= G_H \circ \overline F
&\cr
&= \bigl( \overline F \circ G_E \circ \overline F\inv \ \cup\
\overline S \circ G_E \circ \overline S\inv \bigr) \circ \overline F
&\text{by theorem~17 ($G$ is minimal relative to $\N$)}\cr
&= \overline F \circ G_E \circ \overline F\inv \circ \overline F \ \cup\
\overline S \circ G_E \circ \overline S\inv \circ \overline F
&\cr
&= \overline F \circ G_E \circ id_E \ \cup\
\overline S \circ G_E \circ \bot
&\text{by theorem~7 ($E \buildrel F \over \rightarrow H \buildrel S \over
\leftarrow E$ is a
sum)}\cr
&= \overline F \circ G
&\cr
}$$
with a similar proof for $\overline S \circ G = G \circ \overline S$.

\medskip\f
$\underline{\forall R\ \ (\overline A\inv \circ R = (\overline F \cup
\overline S) \circ R \ \Rightarrow\ G_{\Sigma} \circ R \subseteq \overline W
\circ G_N \circ R\ \cup \ id_\Sigma \circ \overline A \circ G_H \circ \overline
A\inv \circ R).}$ Consider any \goodbreak relation $R$ such that $\overline A\inv \circ R =
(\overline F \cup \overline S) \circ R$. Then
$$\eqqalign\quad{
\overline F\inv \circ \overline A\inv \circ R
&= \overline F\inv \circ (\overline F \cup \overline S) \circ R
&\cr
&= \overline F\inv \circ \overline F \circ R \ \cup\
\overline F\inv \circ \overline S \circ R
&\cr
&= id_E \circ R \ \cup\ \bot \circ R
&\text{by theorem~7 ($E \buildrel F \over \rightarrow H \buildrel S \over
\leftarrow E$ is a sum)}\cr
&= id_E \circ R
&\cr
}$$
and similarly $\overline S\inv \circ \overline A\inv \circ R = id_E \circ R$.
Consequently $\overline F\inv \circ \overline A\inv \circ R = \overline S\inv
\circ \overline A\inv \circ R$.

Define a function $f:N \cup \Sigma \to \Cal P(\dom(R))$ (where $\Cal P(\dom(R))$
is the power-set of $\dom(R)$) by
$$ \forall x \from N\cup\Sigma \quad f(x) = \comp{y}{R(x,y)}. $$
Then
$$\eqalign{
\forall e\from E \quad
f(A(F(e)))
&= \comp{y}{R(A(F(e)),y)}
= \comp{y}{(\overline F\inv \circ \overline A\inv \circ R)(e,y)}
\cr&
= \comp{y}{(\overline S\inv \circ \overline A\inv \circ R)(e,y)}
= \comp{y}{R(A(S(e)),y)}
= f(A(S(e)))
}$$
i.e., $f \circ A \circ F = f \circ A \circ S$. Since $E \doublearrow{A \circ
F}{A \circ S} N\cup\Sigma \buildrel W \over \rightarrow \Sigma$ is a coequaliser
diagram, there exists a unique function $i: \Sigma \to \Cal P(\dom(R))$ such
that $i \circ W = f$. Bearing in mind that $\forall \sigma\from\Sigma\
W(\sigma)=\sigma$, this implies
$$\eqalign{
\forall n\from N \quad
\comp{y}{(\overline W\inv \circ R)(n,y)}
&= \comp{y}{R(W(n),y)}
= f(W(n))
= i(W(W(n)))
= i(W(n))
\cr&
= f(n)
= \comp{y}{R(n,y)}
}$$
so $id_N \circ \overline W\inv \circ R = id_N \circ R$, so $\overline W \circ G
\circ id_N \circ \overline W\inv \circ R = \overline W \circ G \circ id_N \circ
R$, i.e., $\overline W \circ G_N \circ \overline W\inv \circ R = \overline W
\circ G_N \circ R$.

Also, $G$ is minimal relative to $\N$, and therefore, by theorem~17,
$$ G_\Sigma = \overline W \circ G_N \circ \overline W\inv
\ \cup\ id_\Sigma \circ \overline A \circ G_H \circ \overline A\inv. $$

Hence
$$ G_\Sigma \circ R
= \overline W \circ G_N \circ \overline W\inv \circ R
\ \cup\ id_\Sigma \circ \overline A \circ G_H \circ \overline A\inv \circ R
= \overline W \circ G_N \circ R
\ \cup\ id_\Sigma \circ \overline A \circ G_H \circ \overline A\inv \circ R
$$
which is stronger than the required condition. \qed


\subhead{3.5 Properties preserved by homomorphisms}
Parsing involves constructing a pattern network $\N_1$ and a homomorphism $p$
from $\N_1$ to the grammar network $\N_0$. The fact that $\N_1$ and $\N_0$ are
linked by a homomorphism implies some tight relationships between the two
networks; these relationships are stated in theorem~19 below. In particular, the
fact that $\N_0$ is semi-definite implies that some of the semi-definiteness
properties are carried over to $\N_1$, as shown in theorem~20; these properties
therefore hold true for the pattern throughout recognition, not just at the
end.


\theorem 19. If $p:\N_1\to\N_0$ is a homomorphism from a network
$\N_1=\network{_1}$ to a network $\N_0=\network{_0}$ then

\item{(i)} $\overline p\inv \circ \overline p \ \cap\ G_1 \circ G_1\inv
\subseteq id_{\Sigma_1\cup N_1 \cup H_1 \cup E_1 \cup K_1}$,

\item{(ii)} $\overline p\inv \circ G_{0H} \circ \overline p \ \cap\ \overline
{A_1}\inv \circ (G_{1N} \cup G_{1\Sigma}) \circ \overline{A_1} = G_{1H}$,

\item{(iii)} $\overline p\inv \circ G_{0K} \circ \overline p \ \cap\ \overline
{C_1}\inv \circ G_{1E} \circ \overline{C_1} = G_{1K}$,

\item{(iv)} $\overline{A_0}\inv \circ \overline p = \overline p \circ
\overline{A_1}\inv$,

\item{(v)} $\overline{C_0}\inv \circ \overline p = \overline p \circ
\overline{C_1}\inv$.

\proof (i) This follows by theorem~14 since $G_1$ is minimal relative to $p$
(by the definition of a homomorphism).

(ii) I shall use the abbreviations $G_{1N\Sigma} = G_{1N} \cup G_{1\Sigma}$ and
$p_H = p|_{H_1}$ (so $\overline{p_H} = \overline p \circ id_{H_1} = id_{H_0}
\circ \overline p$).

$\underline{G_{1H} \subseteq \overline p\inv \circ G_{0H} \circ \overline p \
\cap\ \overline {A_1}\inv \circ G_{1N\Sigma} \circ \overline{A_1}}$. The
definition of a homomorphism gives $\overline p \circ G_1 = G_0 \circ \overline
p$ and hence $\overline p \circ G_{1H} = G_{0H} \circ \overline p$ (in detail,
$\overline p \circ G_{1H} = \overline p \circ id_{H_1} \circ G_1 = id_{H_0}
\circ \overline p \circ G_1 = id_{H_0} \circ G_0 \circ \overline p = G_{0H}
\circ \overline p$). Hence by theorem~2(iv) $G_{1H} \subseteq \overline p\inv
\circ G_{0H} \circ \overline p$. Also, by the definition of a network,
$\overline{A_1} \circ G_1 \subseteq G_1 \circ \overline{A_1}$, hence by
theorem~2(iv) $id_{H_1} \circ G_1 \subseteq \overline{A_1}\inv \circ G_1 \circ
\overline{A_1}$, i.e., $G_{1H} \subseteq \overline{A_1}\inv \circ G_{1N\Sigma}
\circ \overline{A_1}$. Combining these two gives $G_{1H} \subseteq \overline
p\inv \circ G_{0H} \circ \overline p \ \cap\ \overline {A_1}\inv \circ
G_{1N\Sigma} \circ \overline{A_1}$.

$\underline{\overline p\inv \circ G_{0H} \circ \overline p \ \cap\ \overline
{A_1}\inv \circ G_{1N\Sigma} \circ \overline{A_1} \subseteq G_{1H}}$. Now,
$$\eqqalignno\quad{
\overline p\inv \circ G_{0H} \circ \overline p
&= \overline p\inv \circ id_{H_0} \circ G_0 \circ \overline p
&\cr
&= \overline{p_H}\inv \circ id_{H_0} \circ \overline p \circ G_1
&\text{since $G_0 \circ \overline p = \overline p \circ G_1$ ($p$ is a
homomorphism)} \cr
&= \overline{p_H}\inv \circ \overline{p_H} \circ id_{H_1} \circ G_1
&\cr
&= \overline{p_H}\inv \circ \overline{p_H} \circ G_{1H}.
&\cr
}{(1)}$$
Also, from the definition of a network, $\overline{A_1} \circ G_1 \subseteq G_1
\circ \overline{A_1}$, so by theorem~2(iii),(iv) $id_{H_1} \circ G_1 \circ
\overline{A_1}\inv \subseteq \overline{A_1}\inv \circ G_1 \circ
id_{N_1\cup\Sigma_1}$, i.e., $G_{1H} \circ \overline{A_1}\inv \subseteq
\overline{A_1}\inv \circ G_{1N\Sigma}$. Inverting this gives
$$ \overline{A_1} \circ G_{1H}\inv\subseteq G_{1N\Sigma}\inv \circ
\overline{A_1}. \eqno (2) $$
Furthermore,
$$\eqqalignno\quad{
\overline{p_H}\inv \circ \overline{p_H}
&= \overline p\inv \circ id_{H_0} \circ \overline p &\cr
&\subseteq \overline p\inv \circ \overline{A_0}\inv \circ \overline{A_0}
\circ \overline p &\text{by theorem~2(ii)}\cr
&= \overline{A_1}\inv \circ \overline p\inv \circ \overline p \circ
\overline{A_1}
&\text{since $A_0 \circ p = p \circ A_1$ ($p$ is a homomorphism).}\cr
}{(3)}$$
Using (1)--(3),
$$\eqqalign{\kern-40pt}{
&\kern-20pt \overline p\inv \circ G_{0H} \circ \overline p \ \cap\
\overline{A_1}\inv \circ G_{1N\Sigma} \circ \overline{A_1} &\cr
&= \overline{p_H}\inv \circ \overline{p_H} \circ G_{1H} \ \cap\
\overline{A_1}\inv \circ G_{1N\Sigma} \circ \overline{A_1}
&\text{by (1)}\cr
&\subseteq (\overline{p_H}\inv \circ \overline{p_H} \ \cap\ \overline{A_1}\inv
\circ G_{1N\Sigma} \circ \overline{A_1} \circ G_{1H}\inv) \circ G_{1H}
&\text{by theorem~4(i)}\cr
&\subseteq (\overline{p_H}\inv \circ \overline{p_H} \ \cap\ \overline{A_1}\inv
\circ G_{1N\Sigma} \circ G_{1N\Sigma}\inv \circ \overline{A_1}) \circ G_{1H}
&\text{by (2)}\cr
&= (\overline{p_H}\inv \circ \overline{p_H} \ \cap \
\overline{A_1}\inv \circ \overline p\inv \circ
\overline p \circ \overline{A_1} \ \cap\ \overline{A_1}\inv
\circ G_{1N\Sigma} \circ G_{1N\Sigma}\inv \circ \overline{A_1}) \circ G_{1H}
&\hskip40pt\text{by (3)}\cr
&= \bigl(\overline{p_H}\inv \circ \overline{p_H} \ \cap \
\overline{A_1}\inv \circ (\overline p\inv \circ
\overline p \ \cap\ G_{1N\Sigma} \circ G_{1N\Sigma}\inv) \circ \overline{A_1}
\bigr) \circ G_{1H}
&\text{by theorem~3(v),(vi)}\cr
&\subseteq \bigl(\overline{p_H}\inv \circ \overline{p_H} \ \cap \
\overline{A_1}\inv \circ (\overline p\inv \circ
\overline p \ \cap\ G_1 \circ G_1\inv) \circ \overline{A_1} \bigr) \circ G_{1H}
&\cr
&\subseteq (\overline{p_H}\inv \circ \overline{p_H} \ \cap \
\overline{A_1}\inv \circ id_{\Sigma_1\cup N_1\cup H_1\cup E_1\cup K_1} \circ
\overline{A_1}) \circ G_{1H}
&\text{by part (i)} \cr
&= (\overline{p_H}\inv \circ \overline{p_H} \ \cap \
\overline{A_1}\inv \circ \overline{A_1}) \circ G_{1H} &\cr
&\subseteq id_{H_1} \circ G_{1H}
&\hskip-80pt\strut\text{by theorem~6 ($p$ is a homomorphism)}\cr
&= G_{1H} &\cr
}$$
as required.

(iii) The argument is as in part (ii), with hooks replaced by facets,
$G_{1N\Sigma}$ replaced by $G_{1E}$, and $id_{N_1\cup\Sigma_1}$ replaced by
$id_{E_1}$.

(iv) We have
$$\eqqalign\quad{
\overline{A_0}\inv \circ \overline p
&= \overline{A_0}\inv \circ id_{N_0\cup\Sigma_0} \circ \overline p
&\text{since $A_0:H_0 \to N_0 \cup \Sigma_0$} \cr
&= \overline{A_0}\inv \circ \overline p \circ id_{N_1\cup\Sigma_1}
&\text{since $N_1\cup\Sigma_1 = p\pre{N_0\cup\Sigma_0}$} \cr
&= \overline{A_0}\inv \circ \overline{p|_{N_1\cup\Sigma_1}}
&\cr
&= \overline{p|_{H_1}} \circ \overline{A_1}\inv
&\text{by theorem~6 ($p$ is a homomorphism)} \cr
&= \overline p \circ id_{H_1} \circ \overline{A_1}\inv
&\cr
&= \overline p \circ \overline{A_1}\inv
&\text{since $A_1:H_1 \to N_1 \cup \Sigma_1$.} \cr
}$$

(v) The argument is as in part (iv). \qed


\theorem 20. If $p:\N_1\to\N_0$ is a homomorphism from a network
$\N_1=\network{_1}$ to a \i{semi-definite} network $\N_0$, then

\item{(i)} $G_{1K} \circ G_{1K}\inv \subseteq id_{K_1}$,

\item{(ii)} $\overline{F_1} \circ G_1 = G_1 \circ \overline{F_1}$ and
$\overline{S_1} \circ G_1 = G_1 \circ \overline{S_1}$,

\item{(iii)} $G_{1N} = id_{N_1} \circ \overline{A_1} \circ G_{1H} \circ
\overline A_1\inv$,

\item{(iv)} $G_{1E} = \overline{C_1} \circ G_{1K} \circ \overline{C_1}\inv$.

\proof We shall use the usual notation, $\N_0=\network{_0}$.

(i) Now,
$$\eqqalign{\kern-30pt}{
G_{1K} \circ G_{1K}\inv
&= id_{\Sigma_1\cup N_1 \cup H_1 \cup E_1 \cup K_1} \circ G_1 \circ id_{K_1}
\circ G_1\inv \circ id_{\Sigma_1\cup N_1 \cup H_1 \cup E_1 \cup K_1}
&\cr
&\subseteq \overline p\inv \circ \overline p \circ G_1 \circ id_{K_1} \circ
G_1\inv \circ \overline p\inv \circ \overline p
&\text{by theorem~2(ii)}\cr
&= \overline p\inv \circ G_0 \circ \overline p \circ id_{K_1} \circ
\overline p\inv \circ G_0\inv \circ \overline p
&\kern-45pt\text{since $\overline p \circ G_1 = G_0 \circ \overline p$ ($p$ is a
homomorphism)} \cr
&= \overline p\inv \circ G_0 \circ id_{K_0} \circ \overline p \circ
\overline p\inv \circ G_0\inv \circ \overline p
&\text{since $K_1 = p\pre{K_0}$} \cr
&\subseteq \overline p\inv \circ G_0 \circ id_{K_0} \circ
id_{\Sigma_0\cup N_0 \cup H_0 \cup E_0 \cup K_0} \circ G_0\inv \circ \overline p
&\text{by theorem~2(i)}\cr
&= \overline p\inv \circ G_{0K} \circ G_{0K}\inv \circ \overline p
&\cr
&\subseteq \overline p\inv \circ\overline p
&\kern-45pt\text{since $G_{0K} \circ G_{0K}\inv \subseteq id_{K_0}$ ($\N_0$ is
semi-definite)} \cr
}$$
so
$$\eqqalign\quad{
G_{1K} \circ G_{1K} \inv
&= \overline p\inv \circ \overline p \ \cap\ G_{1K} \circ G_{1K} \inv
&\cr
&= id_{K_1} \circ \bigl( \overline p\inv \circ \overline p \ \cap\ G_1 \circ
G_1\inv \bigr) \circ id_{K_1}
&\text{by theorem~4(iii),(iv)}\cr
&\subseteq id_{K_1} \circ id_{\Sigma_1\cup N_1\cup H_1\cup E_1\cup K_1} \circ
id_{K_1}
&\text{by theorem~19(i)}\cr
&= id_{K_1}
&\cr
}$$
as required.

(ii) I shall just show $\overline{F_1} \circ G_1 = G_1 \circ \overline{F_1}$;
the proof for $\overline{S_1} \circ G_1 = G_1 \circ \overline{S_1}$ is similar.
First,
$$\eqqalign\ {
G_1 \circ \overline{F_1}
&= id_{\Sigma_1 \cup N_1 \cup H_1 \cup E_1 \cup K_1} \circ G_1 \circ
\overline{F_1} &\cr
&\subseteq \overline p\inv \circ \overline p \circ G_1 \circ \overline{F_1}
&\text{by theorem~2(ii)} \cr
&= \overline p\inv \circ G_0 \circ \overline p \circ \overline{F_1}
&\text{since $\overline p \circ G_1 = G_0 \circ \overline p$ ($p$ is a
homomorphism)} \cr
&= \overline p\inv \circ G_0 \circ \overline{F_0} \circ \overline p
&\text{since $p \circ F_1 = F_0 \circ p$ ($p$ is a homomorphism)} \cr
&= \overline p\inv \circ \overline{F_0} \circ G_0 \circ \overline p
&\text{since $G_0 \circ \overline{F_0} = \overline{F_0} \circ G_0$
($\N_0$ is semi-definite)} \cr
&= \overline p\inv \circ \overline{F_0} \circ \overline p \circ G_1
&\text{since $G_0 \circ \overline p = \overline p \circ G_1$ ($p$ is a
homomorphism)} \cr
&= \overline p\inv \circ \overline p \circ \overline{F_1} \circ G_1
&\text{since $F_0 \circ p = p \circ F_1$ ($p$ is a homomorphism).} \cr
}$$
Hence
$$\eqqalign{\kern-1pt}{
G_1 \circ \overline{F_1}
&= \overline p\inv \circ \overline p \circ \overline{F_1} \circ G_1 \ \cap\
G_1 \circ \overline{F_1} &\cr
&\subseteq (\overline p\inv \circ \overline p \ \cap\
G_1 \circ \overline{F_1} \circ (\overline{F_1} \circ G_1)\inv)
\circ \overline{F_1} \circ G_1
&\text{by theorem~4(i)} \cr
&\subseteq (\overline p\inv \circ \overline p \ \cap\
G_1 \circ \overline{F_1} \circ (G_1 \circ \overline{F_1})\inv)
\circ \overline{F_1} \circ G_1
&\text{since $\overline{F_1} \circ G_1 \subseteq G_1 \circ \overline{F_1}$
($\N_1$ is a network)} \cr
&= (\overline p\inv \circ \overline p \ \cap\
G_1 \circ \overline{F_1} \circ \overline{F_1}\inv \circ G_1\inv)
\circ \overline{F_1} \circ G_1 &\cr
&\subseteq (\overline p\inv \circ \overline p \ \cap\
G_1 \circ id_{H_1} \circ G_1\inv)
\circ \overline{F_1} \circ G_1
&\text{by theorem~2(i)} \cr
&\subseteq (\overline p\inv \circ \overline p \ \cap\
G_1 \circ G_1\inv) \circ \overline{F_1} \circ G_1 &\cr
&\subseteq id_{\Sigma_1 \cup N_1 \cup H_1 \cup E_1 \cup K_1} \circ
\overline{F_1} \circ G_1
&\text{by theorem~19(i)} \cr
&= \overline{F_1} \circ G_1. &\cr
}$$
Since the converse $\overline{F_1} \circ G_1 \subseteq G_1 \circ \overline{F_1}$
is given by the definition of a network, this establishes that $\overline{F_1}
\circ G_1 = G_1 \circ \overline{F_1}$, as required.

(iii) The definition of a network gives $\overline{A_1} \circ G_1 \subseteq G_1
\circ \overline{A_1}$, and hence by theorem~2(iii) $\overline{A_1} \circ G_1
\circ \overline{A_1}\inv \subseteq G_1 \circ id_{N_1\cup\Sigma_1}$, and hence
$id_{N_1} \circ \overline{A_1} \circ G_{1H} \circ \overline{A_1}\inv \subseteq
G_{1N}$.

For the converse, the fact that $p$ is a homomorphism gives $\overline p \circ
G_1 = G_0 \circ \overline p$, and hence $\overline p \circ G_{1N} = G_{0N} \circ
\overline p$. Thus
$$\eqqalign\quad {
G_{1N}
&\subseteq \overline p\inv \circ G_{0N} \circ \overline p
&\text{by theorem~2(iv)} \cr
&= \overline p\inv \circ id_{N_0} \circ \overline{A_0} \circ G_{0H}
\circ \overline{A_0}\inv \circ \overline p
&\text{by theorem~17 ($\N_0$ is semi-definite)} \cr
&\subseteq \overline p\inv \circ \overline{A_0} \circ G_{0H}
\circ \overline{A_0}\inv \circ \overline p
&\cr
&= \overline{A_1} \circ \overline p\inv \circ G_{0H} \circ \overline p \circ
\overline{A_1}\inv
&\text{by theorem~19(iv).}\cr
}$$
Hence
$$\eqqalign\quad{
G_{1N}
&= \overline{A_1} \circ \overline p\inv \circ G_{0H} \circ \overline p \circ
\overline{A_1}\inv \ \cap\ G_{1N}
&\cr
&\subseteq \bigl( \overline{A_1} \circ \overline p\inv \circ G_{0H} \circ
\overline p \ \cap\ G_{1N}\circ \overline{A_1} \bigr) \circ \overline{A_1}\inv
&\text{by theorem~4(i)} \cr
&\subseteq \overline{A_1} \circ \bigl( \overline p\inv \circ G_{0H} \circ
\overline p \ \cap\ \overline{A_1}\inv \circ G_{1N}\circ \overline{A_1}
\bigr) \circ \overline{A_1}\inv
&\text{by theorem~4(ii)} \cr
&\subseteq \overline{A_1} \circ \bigl( \overline p\inv \circ G_{0H} \circ
\overline p \ \cap\ \overline{A_1}\inv \circ (G_{1N} \cup G_{1\Sigma}) \circ
\overline{A_1} \bigr) \circ \overline{A_1}\inv
&\cr
&= \overline{A_1} \circ G_{1H} \circ \overline{A_1}\inv
&\text{by theorem~19(ii)} \cr
}$$
so $G_{1N} = id_{N_1} \circ G_{1N} \subseteq id_{N_1} \circ \overline{A_1} \circ
G_{1H} \circ \overline{A_1}\inv$, as required.

(iv) The argument is similar to part (iii), with hooks replaced by facets, nodes
replaced by edges, $A_1,A_0$ replaced by $C_1,C_0$, and with $id_{N_1}$,
$id_{N_0}$ and $G_{1\Sigma}$ removed. \qed


\subhead{3.6 Theorems on definiteness}
The recognition process aims to achieve a definite pattern $\N_1$. Theorem~23
below provides sufficient conditions through which definiteness is ensured. 
Theorem~21 and theorem~22 are more general results, with weaker hypotheses and
conclusions, which are used in the proof of theorem~23 and also later in \S8.


\theorem 21. If $p:\N_1\to\N_0$ is a homomorphism from a network
$\N_1=\network{_1}$ to a semi-definite network $\N_0$, and $Y$ is a set, such
that

\smallskip

\item{(a)} $Y \subseteq \Sigma_1$ and $E_1 \buildrel F_1 \over \rightarrow
A_1\pre{N_1\cup Y} \buildrel S_1 \over \leftarrow E_1$ is a sum diagram in the
category of sets,

\item{(b)} $\exists f:K_1\setdiff dom(G_1) \to K_1 \ G_{1K}\inv=\overline f$,

\smallskip\f
then

\smallskip

\item{(i)} $G_1 \circ id_{A_1\pre{N_1\cup Y}} = \overline{F_1} \circ G_{1E}
\circ \overline{F_1}\inv \cup \overline{S_1} \circ G_{1E} \circ
\overline{S_1}\inv$,

\item{(ii)} $id_{K_1} = G_{1K} \circ G_{1K}\inv \ \cup \ G_{1K}\inv \circ
G_{1K}$,

\item{(iii)} $\overline p\inv \circ \overline p \ \cap \ G_{1E}\inv \circ
G_{1E} \subseteq id_{E_1}$,

\item{(iv)} $\overline p\inv \circ \overline p \ \cap \ id_{A_1\pre{N_1}} \circ
G_1\inv \circ G_1 \circ id_{A_1\pre{N_1}} \subseteq id_{A_1\pre{N_1}}$,

\item{(v)} $\overline p\inv \circ \overline p \ \cap \ G_{1N}\inv \circ
G_{1N} \subseteq id_{N_1}$,

\item{(vi)} $G_{1N}$ is acyclic.

\proof We shall use the usual notation, $\N_0=\network{_0}$.

(i) We have
$$\eqqalign\quad{
G_1 \circ id_{A_1\pre{N_1\cup Y}}
&= G_1 \circ \bigl( \overline{F_1} \circ \overline{F_1}\inv \ \cup\
\overline{S_1} \circ \overline{S_1}\inv \bigr)
&\text{by theorem~7 and hypothesis (a)} \cr
&= G_1 \circ \overline{F_1} \circ \overline{F_1}\inv \ \cup\
G_1 \circ \overline{S_1} \circ \overline{S_1}\inv
&\text{by theorem~3(ii)} \cr
&= \overline{F_1} \circ G_1 \circ \overline{F_1}\inv \ \cup\
\overline{S_1} \circ G_1 \circ \overline{S_1}\inv
& \text{by theorem~20(ii)} \cr
&= \overline{F_1} \circ G_{1E} \circ \overline{F_1}\inv \ \cup\
\overline{S_1} \circ G_{1E} \circ \overline{S_1}\inv
&\text{since $F_1,S_1:E_1 \to H_1$.}\cr
}$$

\medskip

(ii) By hypothesis (b) there is a function $f:K_1\setdiff \dom(G_1) \to K_1$
such that $G_{1K}\inv = \overline f$. Hence
$$\eqalign{
G_{1K}\inv \circ G_{1K} &\subseteq id_{K_1}, \cr
id_{K_1\setdiff \dom(G_1)} &\subseteq G_{1K} \circ G_{1K}\inv
}$$
by theorem~2(i),(ii). But we also have
$$\eqqalign\quad{
id_{\dom(G_{1K})} &\subseteq G_{1K}\inv \circ G_{1K}
&\text{since this holds for all relations,} \cr
G_{1K} \circ G_{1K}\inv &\subseteq id_{K_1}
&\text{by theorem~20(i).} \cr
}$$
Combining these four in pairs gives
$$\eqalign{
G_{1K} \circ G_{1K}\inv \ \cup \ G_{1K}\inv \circ G_{1K}
&\subseteq id_{K_1}, \cr
id_{K_1} = id_{K_1\setdiff \dom(G_1)} \cup id_{\dom(G_{1K})}
&\subseteq G_{1K} \circ G_{1K}\inv \ \cup\ G_{1K}\inv \circ G_{1K}
}$$
and hence $id_{K_1} = G_{1K} \circ G_{1K}\inv \ \cup \ G_{1K}\inv \circ G_{1K}$,
as required.

\medskip

(iii) Theorem~20(iv) says $G_{1E} = \overline{C_1} \circ G_{1K} \circ
\overline{C_1}\inv$, and hence
$$ G_{1E}\inv = \overline{C_1} \circ G_{1K}\inv \circ \overline{C_1}\inv.
\eqno(1) $$
Also, from the definition of a homomorphism, $\overline p \circ G_{1K} = G_{0K}
\circ \overline p$, and hence by theorem~2(iii),(iv),
$$ G_{1K} \circ \overline p\inv \subseteq \overline p\inv \circ G_{0K}.
\eqno(2) $$
This gives
$$\eqqalign{}{
&\kern-3pt\overline p\inv \circ \overline p \ \cap \ G_{1E}\inv \circ G_{1E}
&\cr
&= \overline p\inv \circ \overline p \ \cap \
\overline{C_1} \circ G_{1K}\inv \circ \overline{C_1}\inv \circ G_{1E}
&\text{by (1)}\cr
&\subseteq \overline{C_1} \circ \bigl( \overline{C_1}\inv \circ
\overline p\inv \circ \overline p \ \cap \ G_{1K}\inv \circ \overline{C_1}\inv
\circ G_{1E} \bigr)
&\text{by theorem~4(ii)}\cr
&= \overline{C_1} \circ \bigl( \overline p\inv \circ \overline{C_0}\inv \circ
\overline p \ \cap \ G_{1K}\inv \circ \overline{C_1}\inv \circ G_{1E} \bigr)
&\kern-40pt\text{since $p \circ C_1 = C_0 \circ p$ ($p$ is a homomorphism)}\cr
&= \overline{C_1} \circ \bigl( \overline p\inv \circ \overline p \circ
\overline{C_1}\inv \ \cap \ G_{1K}\inv \circ \overline{C_1}\inv \circ G_{1E}
\bigr)
&\text{by theorem~19(v)}\cr
&\subseteq \overline{C_1} \circ \bigl( \overline p\inv \circ \overline p
\ \cap \ G_{1K}\inv \circ \overline{C_1}\inv \circ G_{1E} \circ
\overline{C_1} \bigr) \circ \overline{C_1}\inv
&\text{by theorem~4(i)}\cr
&\subseteq \overline{C_1} \circ G_{1K}\inv \circ \bigl( G_{1K} \circ
\overline p\inv \circ \overline p \ \cap \
\overline{C_1}\inv \circ G_{1E} \circ \overline{C_1} \bigr) \circ
\overline{C_1}\inv
&\text{by theorem~4(ii)}\cr
&\subseteq \overline{C_1} \circ G_{1K}\inv \circ \bigl( \overline p\inv \circ
G_{0K} \circ \overline p \ \cap \
\overline{C_1}\inv \circ G_{1E} \circ \overline{C_1} \bigr) \circ
\overline{C_1}\inv
&\text{by (2)}\cr
&= \overline{C_1} \circ G_{1K}\inv \circ G_{1K} \circ \overline{C_1}\inv
&\text{by theorem 19(iii)}\cr
&\subseteq \overline{C_1} \circ id_{K_1} \circ \overline{C_1}\inv
&\text{by part (ii)}\cr
&= \overline{C_1} \circ \overline{C_1}\inv
&\text{since $C_1:K_1\to E_1$}\cr
&\subseteq id_{E_1}
&\text{by theorem~2(i).}\cr
}$$

\medskip

(iv) First, the definition of a homomorphism gives $\overline p \circ G_{1E} =
G_{0E} \circ \overline p$, and so by theorem~2(iii),(iv)
$$ G_{1E} \circ \overline p\inv \subseteq \overline p\inv \circ G_{0E}. \eqno(3)
$$
This is used in the following:
$$\eqqalignno\quad{
&\kern-10pt\overline{F_1}\inv \circ \overline p\inv \circ \overline p
\circ \overline{F_1} \ \cap\ G_{1E}\inv \circ G_{1E}
&\cr
&= \overline p\inv \circ \overline{F_0}\inv \circ \overline{F_0} \circ
\overline p \ \cap\ G_{1E}\inv \circ G_{1E}
&\kern-96pt\text{since $p \circ F_1 = F_0 \circ p$ ($p$ is a homomorphism)}\cr
&\subseteq \overline p\inv \circ \bigl( \overline{F_0}\inv \circ \overline{F_0}
\ \cap\ \overline p \circ G_{1E}\inv \circ G_{1E} \circ \overline p\inv
\bigr) \circ \overline p
&\text{by theorem~4(i),(ii)}\cr
&\subseteq \overline p\inv \circ \bigl( \overline{F_0}\inv \circ \overline{F_0}
\ \cap\ G_{0E}\inv \circ \overline p \circ \overline p\inv \circ G_{0E}
\bigr) \circ \overline p
&\text{by (3)}\cr
&\subseteq \overline p\inv \circ \bigl( \overline{F_0}\inv \circ \overline{F_0}
\ \cap\ G_{0E}\inv \circ id_{\Sigma_0\cup N_0\cup H_0\cup E_0\cup K_0} \circ
G_{0E} \bigr) \circ \overline p
&\text{by theorem~2(i)}\cr
&= \overline p\inv \circ \bigl( \overline{F_0}\inv \circ \overline{F_0}
\ \cap\ G_{0E}\inv \circ G_{0E} \bigr) \circ \overline p
&\cr
&\subseteq \overline p\inv \circ id_{E_0} \circ \overline p
&\kern-96pt\text{by theorem~14 ($G_{0E}\inv$ is minimal relative to $F_0$)}\cr
&\subseteq \overline p\inv \circ \overline p.
&\cr
}{(4)}$$
Using this we derive
$$\kern20pt\eqqalignno{\kern-20pt}{
&\kern-30pt
\overline p\inv \circ \overline p \ \cap\ \overline{F_1} \circ G_{1E}\inv
\circ G_{1E} \circ \overline{F_1}\inv
&\cr
&\subseteq \overline{F_1} \circ \bigl( \overline{F_1}\inv \circ \overline p\inv
\circ \overline p \circ \overline{F_1} \ \cap\ G_{1E}\inv \circ G_{1E}
\bigr) \circ \overline{F_1}\inv
&\text{by theorem~4(i),(ii)}\cr
&= \overline{F_1} \circ \bigl(
\overline{F_1}\inv \circ \overline p\inv \circ
\overline p \circ \overline{F_1} \ \cap\
G_{1E}\inv \circ G_{1E}\ \cap\
G_{1E}\inv \circ G_{1E} \bigr) \circ \overline{F_1}\inv
&\cr
&\subseteq \overline{F_1} \circ (\overline p\inv \circ \overline p \ \cap\
G_{1E}\inv
\circ G_{1E}) \circ \overline{F_1}\inv
&\text{by (4)}\cr
&\subseteq \overline{F_1} \circ id_{E_1} \circ \overline{F_1}\inv
&\text{by part (iii)}\cr
&= \overline{F_1} \circ \overline{F_1}\inv
&\text{since $F_1:E_1\to H_1$}\cr
&\subseteq id_{H_1}
&\text{by theorem~2(i).}\cr
}{(5)}$$
By a similar argument,
$$ \overline p\inv \circ \overline p \ \cap\ \overline{S_1} \circ G_{1E}\inv
\circ G_{1E} \circ \overline{S_1}\inv \subseteq id_{H_1}. \eqno(6) $$
We also have, using the abbreviation $I = id_{A_1\pre{N_1}}$,
$$\kern-10pt\eqqalignno{\kern-175pt}{
I \circ G_1\inv \circ G_1 \circ I
&\subseteq id_{A_1\pre{N_1\cup Y}} \circ G_1\inv \circ G_1 \circ
id_{A_1\pre{N_1\cup Y}}
&\cr
&= \bigl( \overline{F_1} \circ G_{1E}\inv \circ \overline{F_1}\inv \
\cup\ \overline{S_1} \circ G_{1E}\inv \circ \overline{S_1}\inv \bigr) \circ
\bigl( \overline{F_1} \circ G_{1E} \circ \overline{F_1}\inv \ \cup\
\overline{S_1} \circ G_{1E} \circ \overline{S_1}\inv \bigr)
&\cr&&\text{by part (i)}\cr
&= \overline{F_1} \circ G_{1E}\inv \circ id_{E_1} \circ G_{1E} \circ
\overline{F_1}\inv \ \cup\ \bot \ \cup\ \bot \ \cup\
\overline{S_1} \circ G_{1E}\inv \circ id_{E_1} \circ G_{1E} \circ
\overline{S_1}\inv&\cr&&\text{by theorem~7 and hypothesis (a)}\cr
&= \overline{F_1} \circ G_{1E}\inv \circ G_{1E} \circ
\overline{F_1}\inv \ \cup\ \overline{S_1} \circ G_{1E}\inv \circ G_{1E} \circ
\overline{S_1}\inv.
&\cr
}{\kern-10pt(7)}$$
Then, by (5), (6) and (7),
$$ \overline p\inv \circ \overline p \ \cap\
I \circ G_1\inv \circ G_1 \circ I
\subseteq id_{H_1} \eqno(8)$$
and so
$$\eqqalign\quad{
\overline p\inv \circ \overline p \ \cap\ I \circ G_1\inv \circ G_1 \circ I
&= \overline p\inv \circ \overline p \ \cap\ I \circ G_1\inv \circ G_1 \circ I
\circ I
&\cr
&= \bigl( \overline p\inv \circ \overline p \ \cap\ I \circ G_1\inv \circ G_1
\circ I
\bigr) \circ I
&\text{by theorem~4(iii)}\cr
&\subseteq id_{H_1} \circ I
&\text{by $(8)$}\cr
&= I
&\text{since $A_1\pre{N_1} \subseteq H_1$}\cr
}$$
as required.

\medskip

(v) From the definition of a homomorphism, $\overline p \circ G_{1H} = G_{0H}
\circ \overline p$, and hence by theorem~2(iii),(iv),
$$ G_{1H} \circ \overline p\inv \subseteq \overline p\inv \circ G_{0H}.
\eqno(9) $$
Also (with $I = id_{A_1\pre{N_1}}$ again),
$$\eqqalign\quad{
I \circ G_1
&= I \circ id_{H_1} \circ G_1
&\text{since $A_1\pre{N_1} \subseteq H_1$}\cr
&\subseteq I \circ \overline{A_1}\inv \circ \overline{A_1}
\circ G_1
&\text{by theorem~2(ii)}\cr
&\subseteq I \circ \overline{A_1}\inv \circ G_1 \circ \overline{A_1}
&\text{since $\overline{A_1} \circ G_1 \subseteq G_1 \circ \overline{A_1}$
($\N_1$ is a network)}\cr
&= \overline{A_1}\inv \circ id_{N_1} \circ G_1 \circ \overline{A_1}
&\text{since $I=id_{A_1\pre{N_1}}$}\cr
&= \overline{A_1}\inv \circ G_1 \circ id_{N_1} \circ \overline{A_1}
&\cr
&= \overline{A_1}\inv \circ G_1 \circ \overline{A_1} \circ I
&\text{since $I = id_{A_1\pre{N_1}}$}\cr
}$$
so by theorem~4(v)
$$ I \circ G_1 \subseteq G_1 \circ I $$
and inverting this gives
$$ G_1\inv \circ I \subseteq I \circ
G_1\inv. \eqno(10) $$
Also, theorem~20(iii) says $G_{1N} = id_{N_1} \circ \overline{A_1} \circ G_{1H}
\circ \overline{A_1}\inv$, and hence
$$ G_{1N}\inv = \overline{A_1} \circ G_{1H}\inv \circ
\overline{A_1}\inv \circ id_{N_1}. \eqno(11) $$
Then,
$$\kern0pt\eqqalignno\ {
&\kern-10pt\overline p\inv \circ \overline p \ \cap \
G_{1H}\inv \circ \overline{A_1}\inv \circ G_{1N} \circ \overline{A_1}
&\cr
&= \overline p\inv \circ \overline p \ \cap \
\overline p\inv \circ \overline p \ \cap \
G_{1H}\inv \circ \overline{A_1}\inv \circ id_{N_1} \circ G_{1N} \circ id_{N_1}
\circ \overline{A_1}
&\cr
&= \overline p\inv \circ \overline p \ \cap \
\overline p\inv \circ \overline p \ \cap \
G_{1H}\inv \circ I \circ \overline{A_1}\inv \circ G_{1N}
\circ \overline{A_1} \circ I
&\text{since $I = id_{A_1\pre{N_1}}$}\cr
&\subseteq \overline p\inv \circ \overline p \ \cap \
G_{1H}\inv \circ \bigl( G_{1H} \circ \overline p\inv \circ \overline p \ \cap \
I \circ \overline{A_1}\inv \circ G_{1N} \circ \overline{A_1} \circ I \bigr)
&\text{by theorem~4(ii)}\cr
&= \overline p\inv \circ \overline p \ \cap \
G_{1H}\inv \circ I \circ \bigl( G_{1H} \circ \overline p\inv \circ \overline p \
\cap \
\overline{A_1}\inv \circ G_{1N} \circ \overline{A_1}
\bigr) \circ I
&\text{by theorem~4(iii),(iv)}\cr
&\subseteq \overline p\inv \circ \overline p \ \cap \
G_{1H}\inv \circ I \circ \bigl( \overline p\inv \circ G_{0H} \circ \overline p \
\cap \
\overline{A_1}\inv \circ G_{1N} \circ \overline{A_1}
\bigr) \circ I
&\text{by (9)}\cr
&\subseteq \overline p\inv \circ \overline p \ \cap \
G_{1H}\inv \circ I \circ G_{1H} \circ I
&\text{by theorem~19(ii)}\cr
&= \overline p\inv \circ \overline p \ \cap \ G_1\inv \circ I \circ G_1 \circ I
&\text{since $id_{H_1} \circ I = I$}\cr
&\subseteq \overline p\inv \circ \overline p \ \cap \
I \circ G_1\inv \circ G_1 \circ I
&\text{by $(10)$}\cr
&\subseteq I
&\text{by part (iv).}\cr
}{\kern-10pt(12)}$$
This gives
$$\kern15pt\eqqalign\ {
&\kern-15pt
\overline p\inv \circ \overline p \ \cap \ G_{1N}\inv \circ G_{1N}
&\cr
&= \overline p\inv \circ \overline p \ \cap \
\overline{A_1} \circ G_{1H}\inv \circ \overline{A_1}\inv \circ id_{N_1} \circ
G_{1N}
&\text{by (11)}\cr
&= \overline p\inv \circ \overline p \ \cap \
\overline{A_1} \circ G_{1H}\inv \circ \overline{A_1}\inv \circ G_{1N}
&\cr
&\subseteq \overline{A_1} \circ \bigl( \overline{A_1}\inv \circ \overline p\inv
\circ \overline p \ \cap \ G_{1H}\inv \circ \overline{A_1}\inv \circ G_{1N}
\bigr)
&\text{by theorem~4(ii)}\cr
&= \overline{A_1} \circ \bigl( \overline p\inv \circ \overline{A_0}\inv \circ
\overline p \ \cap \ G_{1H}\inv \circ \overline{A_1}\inv \circ G_{1N} \bigr)
&\kern-25pt\text{since $p \circ A_1 = A_0 \circ p$ ($p$ is a
homomorphism)}\cr
&= \overline{A_1} \circ \bigl( \overline p\inv \circ \overline p \circ
\overline{A_1}\inv \ \cap \ G_{1H}\inv \circ \overline{A_1}\inv \circ G_{1N}
\bigr)
&\text{by theorem~19(iv)}\cr
&\subseteq \overline{A_1} \circ \bigl( \overline p\inv \circ \overline p
\ \cap \ G_{1H}\inv \circ \overline{A_1}\inv \circ G_{1N} \circ \overline{A_1}
\bigr) \circ \overline{A_1}\inv
&\text{by theorem~4(i)}\cr
&\subseteq \overline{A_1} \circ I \circ \overline{A_1}\inv
&\text{by (12)}\cr
&= id_{N_1} \circ \overline{A_1} \circ \overline{A_1}\inv
&\text{since $I = id_{A_1\pre{N_1}}$}\cr
&\subseteq id_{N_1} \circ id_{N_1 \cup \Sigma_1}
&\text{by theorem~2(i)}\cr
&= id_{N_1}
&\cr
}$$
as required.

\medskip

(vi) Define $p_N = p|_{N_1}$. We already know the following.
$$\kern15pt\eqqalign{}{
&\overline{p_N} \circ G_{1N} = G_{0N} \circ \overline{p_N}
&\text{since $p$ is a homomorphism;} \cr
&\overline{p_N}\inv \circ \overline{p_N} \ \cap\ G_{1N}\inv \circ G_{1N}
\subseteq \overline p\inv \circ \overline p \ \cap\ G_{1N}\inv \circ G_{1N}
&\cr
&\phantom{\overline{p_N}\inv \circ \overline{p_N} \ \cap\ G_{1N}\inv \circ
G_{1N}} \subseteq id_{N_1}
&\text{by part (v);} \cr
&\overline{p_N}\inv \circ \overline{p_N} \ \cap\ G_{1N} \circ G_{1N}\inv
= id_{N_1} \circ \bigl( \overline p\inv \circ \overline p \ \cap\ G_1 \circ
G_1\inv \bigr) \circ id_{N_1}
&\text{by theorem~4(iii),(iv)}\cr
&\phantom{\overline{p_N}\inv \circ \overline{p_N} \ \cap\ G_{1N} \circ
G_{1N}\inv}\subseteq id_{N_1}
&\text{by theorem~19(i);} \cr
&G_{0N} \text{ is acyclic}
&\text{since $\N_0$ is semi-definite.} \cr
}$$
Then by theorem~12 $G_{1N}$ is also acyclic. \qed


\theorem 22. If $p:\N_1\to\N_0$ is a homomorphism from a network
$\N_1=\network{_1}$ to a semi-definite network $\N_0$, and $Y$ is a set, such
that

\smallskip

\item{(a)} $W_1(N_1) \subseteq Y \subseteq \Sigma_1$ and $E_1 \buildrel F_1
\over \rightarrow A_1\pre{N_1\cup Y} \buildrel S_1 \over \leftarrow E_1$ is a
sum diagram in the category of sets,

\item{(b)} $W_1 \circ A_1 \circ F_1 = W_1 \circ A_1 \circ S_1$,

\smallskip\f
then

\smallskip

\item{(i)} $id_{\Sigma_1} \circ \overline{A_1} \circ G_{1H} \circ
\overline{A_1}\inv = \overline{A_1} \circ G_{1H} \circ \overline{A_1}\inv \circ
id_{\Sigma_1}$,

\item{(ii)} $G_1 \circ id_Y = \bigl( \overline{W_1} \circ G_{1N} \circ
\overline{W_1}\inv \ \cup \ id_{\Sigma_1} \circ \overline{A_1} \circ G_{1H}
\circ \overline{A_1}\inv \bigr) \circ id_Y$,

\item{(iii)} $G_1 \circ id_Y \subseteq id_Y \circ G_1$.

\proof We shall use the usual notation, $\N_0=\network{_0}$. We begin with two
observations.

First, note that $W_1(N_1) \subseteq Y$ and $W_1(Y) = Y$, so $N_1 \cup Y
\subseteq W_1\pre Y$. Conversely, any element of $W_1\pre Y$ is either a node or
a symbol in Y, so $W_1\pre Y \subseteq N_1 \cup Y$. Hence
$$ W_1\pre Y = N_1 \cup Y. \eqno(1) $$

Secondly, from $\overline{A_1} \circ G_1 \subseteq G_1 \circ \overline{A_1}$,
theorem~2(iii) implies $\overline{A_1} \circ G_1 \circ \overline{A_1}\inv
\subseteq G_1 \circ id_{N_1\cup\Sigma_1}$, and hence
$$ id_{\Sigma_1} \circ \overline{A_1} \circ G_1 \circ \overline{A_1}\inv
\subseteq id_{\Sigma_1} \circ G_1 \circ id_{N_1\cup\Sigma}. $$
which may be rewritten as
$$ id_{\Sigma_1} \circ \overline{A_1} \circ G_{1H} \circ \overline{A_1}\inv
\subseteq G_1 \circ id_{\Sigma_1}. \eqno(2) $$

(i) Applying theorem~4(v) to (2),
$$ id_{\Sigma_1} \circ \overline{A_1} \circ G_{1H} \circ \overline{A_1}\inv
\subseteq \overline{A_1} \circ G_{1H} \circ \overline{A_1}\inv \circ
id_{\Sigma_1}. $$
The converse is proved similarly, and hence
$$ id_{\Sigma_1} \circ \overline{A_1} \circ G_{1H} \circ \overline{A_1}\inv
= \overline{A_1} \circ G_{1H} \circ \overline{A_1}\inv \circ id_{\Sigma_1} $$
as required.

(ii) From $\overline{W_1} \circ G_1 = G_1 \circ \overline{W_1}$,
theorem~2(iii) implies
$$ \overline{W_1} \circ G_{1N} \circ \overline{W_1}\inv
\subseteq \overline{W_1} \circ G_1 \circ \overline{W_1}\inv
= G_1 \circ \overline{W_1} \circ \overline{W_1}\inv
\subseteq G_1 \circ id_{\Sigma_1}. $$
Combining this with (2),
$$ \overline{W_1} \circ G_{1N} \circ \overline{W_1}\inv \ \cup\
id_{\Sigma_1} \circ \overline{A_1} \circ G_{1H} \circ \overline{A_1}\inv
\subseteq G_1 \circ id_{\Sigma_1}
\subseteq G_1. \eqno(3) $$

Define a relation $R = \overline p \circ \overline{W_1}\inv \circ id_Y \cup
\overline p \circ \overline{W_1 \circ A_1 \circ F_1}\inv$. Then
$$\eqqalignno\ {
id_{N_0\cup\Sigma_0} \circ R
&= id_{N_0\cup\Sigma_0} \circ \overline p \circ \overline{W_1}\inv \circ id_Y
\ \cup\ id_{N_0\cup\Sigma_0} \circ \overline p \circ
\overline{W_1 \circ A_1 \circ F_1}\inv
&\cr
&= \overline p \circ id_{N_1\cup\Sigma_1} \circ id_{N_1\cup Y} \circ
\overline{W_1}\inv \ \cup\
\overline p \circ id_{N_1\cup\Sigma_1} \circ id_{E_1} \circ
\overline{W_1 \circ A_1 \circ F_1}\inv
&\text{by (1)}\cr
&= \overline p \circ id_{N_1\cup Y} \circ \overline{W_1}\inv \ \cup\
\bot
&\cr
&= \overline p \circ \overline{W_1}\inv \circ id_Y
&\text{by (1).}\cr
}{(4)}$$
$$\eqqalignno\ {
id_{N_0} \circ R
&= id_{N_0} \circ id_{N_0\cup\Sigma_0} \circ R
&\cr
&= id_{N_0} \circ \overline p \circ \overline{W_1}\inv \circ id_Y
&\text{by (4)}\cr
&= \overline p \circ id_{N_1} \circ \overline{W_1}\inv \circ id_Y.
&\cr
}{(5)}$$
$$\eqqalignno\ {
id_{\Sigma_0} \circ R
&= id_{\Sigma_0} \circ id_{N_0\cup\Sigma_0} \circ R
&\cr
&= id_{\Sigma_0} \circ \overline p \circ \overline{W_1}\inv \circ id_Y
&\text{by (4)}\cr
&= \overline p \circ id_{\Sigma_1} \circ \overline{W_1}\inv \circ id_Y
&\cr
&= \overline p \circ id_{\Sigma_1} \circ id_Y
&\text{since $\forall\sigma\from\Sigma_1\ W_1(\sigma) = \sigma$}\cr
&= \overline p \circ id_Y.
&\cr
}{(6)}$$
$$\eqqalignno\ {
id_{E_0} \circ R
&= id_{E_0} \circ \overline p \circ \overline{W_1}\inv \circ id_Y
\ \cup\ id_{E_0} \circ \overline p \circ \overline{W_1 \circ A_1 \circ F_1}\inv
&\cr
&= \overline p \circ id_{E_1} \circ id_{N_1\cup Y} \circ \overline{W_1}\inv
\ \cup\ \overline p \circ id_{E_1} \circ \overline{W_1 \circ A_1 \circ F_1}\inv
&\text{by (1)}\cr
&= \bot
\ \cup\ \overline p \circ \overline{W_1 \circ A_1 \circ F_1}\inv
&\cr
&= \overline p \circ \overline{W_1 \circ A_1 \circ F_1}\inv.
&\cr
}{(7)}$$
Hence
$$\eqqalign{\kern-30pt}{
\overline{A_0}\inv \circ R
&= \overline{A_0}\inv \circ id_{N_0\cup\Sigma_0} \circ R
&\cr
&= \overline{A_0}\inv \circ \overline p \circ \overline{W_1}\inv \circ id_Y
&\text{by (4)}\cr
&= \overline p \circ \overline{A_1}\inv \circ id_{N_1\cup Y} \circ
\overline{W_1}\inv
&\text{by theorem~19(iv) and (1)}\cr
&= \overline p \circ id_{A_1\pre{N_1\cup Y}} \circ \overline{A_1}\inv \circ
\overline{W_1}\inv
&\cr
&= \overline p \circ \bigl( \overline{F_1} \circ
\overline{F_1}\inv \cup \overline{S_1} \circ \overline{S_1}\inv \bigr) \circ
\overline{A_1}\inv \circ \overline{W_1}\inv
&\text{by theorem~7 and (a)}\cr
&= \overline p \circ \overline{F_1} \circ \overline{F_1}\inv \circ
\overline{A_1}\inv \circ \overline{W_1}\inv \ \cup\
\overline p \circ \overline{S_1} \circ \overline{S_1}\inv \circ
\overline{A_1}\inv \circ \overline{W_1}\inv
&\cr
&= \overline{F_0} \circ \overline p \circ \overline{W_1 \circ A_1 \circ F_1}\inv
\ \cup\
\overline{S_0} \circ \overline p \circ \overline{W_1 \circ A_1 \circ S_1}\inv
&\text{since $p$ is a homomorphism}\cr
&= \overline{F_0} \circ \overline p \circ \overline{W_1 \circ A_1 \circ F_1}\inv
\ \cup\
\overline{S_0} \circ \overline p \circ \overline{W_1 \circ A_1 \circ F_1}\inv
&\text{by hypothesis (b)}\cr
&= \bigl( \overline{F_0} \cup \overline{S_0} \bigr) \circ \overline p \circ
\overline{W_1 \circ A_1 \circ F_1}\inv
&\cr
&= \bigl( \overline{F_0} \cup \overline{S_0} \bigr) \circ id_{E_0} \circ R
&\text{by (7)}\cr
&= \bigl( \overline{F_0} \cup \overline{S_0} \bigr) \circ R.
&\cr
}$$
Since $\N_0$ is semi-definite we may infer
$$ G_{0\Sigma} \circ R
\subseteq \overline{W_0} \circ G_{0N} \circ R \ \cup\
id_{\Sigma_0} \circ \overline{A_0} \circ G_{0H} \circ
\overline{A_0}\inv \circ R. \eqno(8) $$
Then
$$\kern10pt\eqqalignno{\kern-65pt}{
&\kern-10pt\overline p \circ G_1 \circ id_Y
&\cr
&= G_0 \circ \overline p \circ id_Y
&\text{since $p$ is a homomorphism}\cr
&= G_0 \circ id_{\Sigma_0} \circ R
&\text{by (6)}\cr
&= G_{0\Sigma} \circ R
&\cr
&\subseteq \overline{W_0} \circ G_{0N} \circ R \ \cup\
id_{\Sigma_0} \circ \overline{A_0} \circ G_{0H} \circ \overline{A_0}\inv \circ R
&\text{by (8)}\cr
&= \overline{W_0} \circ G_0 \circ id_{N_0} \circ R \ \cup\
id_{\Sigma_0} \circ \overline{A_0} \circ G_0 \circ \overline{A_0}\inv
\circ id_{N_0\cup\Sigma_0} \circ R
&\cr
&= \overline{W_0} \circ G_0 \circ \overline p \circ id_{N_1} \circ
\overline{W_1}\inv \circ id_Y \ \cup\
id_{\Sigma_0} \circ \overline{A_0} \circ G_0 \circ \overline{A_0}\inv
\circ \overline p \circ \overline{W_1}\inv \circ id_Y
&\cr&&\text{by (5) and (4)}\cr
&= \overline{W_0} \circ G_0 \circ \overline p \circ id_{N_1} \circ
\overline{W_1}\inv \circ id_Y \ \cup\
id_{\Sigma_0} \circ \overline{A_0} \circ G_0 \circ \overline p \circ
\overline{A_1}\inv \circ \overline{W_1}\inv \circ id_Y
&\cr&&\text{by theorem~19(iv)}\cr
&= \overline p \circ \overline{W_1} \circ G_1 \circ id_{N_1} \circ
\overline{W_1}\inv \circ id_Y \ \cup\
\overline p \circ id_{\Sigma_1} \circ \overline{A_1} \circ G_1 \circ
\overline{A_1}\inv \circ \overline{W_1}\inv \circ id_Y
&\cr&&\text{since $p$ is a homomorphism}\cr
&= \overline p \circ \bigl( \overline{W_1} \circ G_{1N} \circ
\overline{W_1}\inv \ \cup\
id_{\Sigma_1} \circ \overline{A_1} \circ G_{1H} \circ \overline{A_1}\inv
\circ \overline{W_1}\inv \bigr) \circ id_Y
&\cr
&= \overline p \circ \bigl( \overline{W_1} \circ G_{1N} \circ
\overline{W_1}\inv \ \cup\
\overline{A_1} \circ G_{1H} \circ \overline{A_1}\inv
\circ id_{\Sigma_1} \circ \overline{W_1}\inv \bigr) \circ id_Y
&\kern20pt\text{by part (i)}\cr
&= \overline p \circ \bigl( \overline{W_1} \circ G_{1N} \circ
\overline{W_1}\inv \ \cup\
\overline{A_1} \circ G_{1H} \circ \overline{A_1}\inv
\circ id_{\Sigma_1} \bigr) \circ id_Y
&\text{since $\forall\sigma\from\Sigma_1\ W_1(\sigma)=\sigma$}\cr
&= \overline p \circ \bigl( \overline{W_1} \circ G_{1N} \circ
\overline{W_1}\inv \ \cup\
id_{\Sigma_1} \circ \overline{A_1} \circ G_{1H} \circ \overline{A_1}\inv
\bigr) \circ id_Y
&\text{by part (i).}\cr
}{\kern-15pt(9)}$$
Define a relation
$$ G^* = \bigl( \overline{W_1} \circ G_{1N} \circ \overline{W_1}\inv \ \cup\
id_{\Sigma_1} \circ \overline{A_1} \circ G_{1H} \circ \overline{A_1}\inv \bigr)
\circ id_Y \ \cup\
G_1 \circ id_{(\Sigma_1\setdiff Y) \cup N_1 \cup H_1 \cup E_1 \cup K_1}. $$
Comparing $G^*$ with $G_1=G_1 \circ id_Y \ \cup\ G_1 \circ id_{(\Sigma_1\setdiff
Y) \cup N_1 \cup H_1 \cup E_1 \cup K_1}$, we have $G^* \subseteq G_1$ by (3),
and hence $\overline p \circ G^* \subseteq \overline p \circ G_1$, but also
$\overline p \circ G_1 \subseteq \overline p \circ G^*$ by (9), and hence
$\overline p \circ G^* = \overline p \circ G_1$. Since $p$ is a homomorphism,
$G_1$ is minimal relative to $p$, so $G^* = G_1$. Hence
$$ G_1 \circ id_Y = G^* \circ id_Y
= \bigl( \overline{W_1} \circ G_{1N} \circ \overline{W_1}\inv \ \cup\
id_{\Sigma_1} \circ \overline{A_1} \circ G_{1H} \circ \overline{A_1}\inv
\bigr) \circ id_Y $$
as required.

\medskip

(iii) We have
$$\eqqalignno{}{
G_1 \circ id_Y
&= \overline{W_1} \circ G_{1N} \circ \overline{W_1}\inv \circ id_Y
\ \cup\ id_{\Sigma_1} \circ \overline{A_1} \circ G_{1H} \circ
\overline{A_1}\inv \circ id_Y
&\text{by part (ii)}\cr
&= \overline{W_1} \circ G_{1N} \circ id_{N_1 \cup Y} \circ \overline{W_1}\inv
\ \cup\ id_{\Sigma_1} \circ \overline{A_1} \circ G_{1H} \circ id_{A_1\pre Y}
\circ \overline{A_1}\inv
&\text{by (1)}\cr
&\subseteq \overline{W_1} \circ G_{1N} \circ \overline{W_1}\inv
\ \cup\ id_{\Sigma_1} \circ \overline{A_1} \circ G_{1H} \circ
\overline{F_1} \circ \overline{F_1}\inv \circ \overline{A_1}\inv
&\cr&\phantom{{}\subseteq{}}
\cup\ id_{\Sigma_1} \circ \overline{A_1} \circ G_{1H} \circ
\overline{S_1} \circ \overline{S_1}\inv \circ \overline{A_1}\inv
&\kern-65pt\text{by theorem~7 and (a).}\cr
}{\kern-5pt(10)}$$
Let us consider each of the three terms on the right-hand side in turn. First,
$$\eqqalign\quad{
\overline{W_1} \circ G_{1N} \circ \overline{W_1}\inv
&= \overline{W_1} \circ id_{N_1 \cup Y} \circ G_{1N} \circ
\overline{W_1}\inv
&\cr
&= id_Y \circ \overline{W_1} \circ G_{1N} \circ \overline{W_1}\inv
&\text{by (1).}\cr
}$$
Secondly,
$$\kern42pt\eqqalign\ {
&\kern-42pt id_{\Sigma_1} \circ \overline{A_1} \circ G_{1H} \circ
\overline{F_1} \circ \overline{F_1}\inv \circ \overline{A_1}\inv
&\cr
&= id_{\Sigma_1} \circ \overline{A_1} \circ G_1 \circ
\overline{F_1} \circ \overline{F_1}\inv \circ \overline{A_1}\inv
&\text{since $F_1:E_1\to H_1$}\cr
&= id_{\Sigma_1} \circ \overline{A_1}\circ
\overline{F_1} \circ G_1 \circ \overline{F_1}\inv \circ \overline{A_1}\inv
&\text{by theorem~20(ii)}\cr
&= id_{\Sigma_1} \circ \overline{A_1}\circ id_{A_1\pre{N_1\cup Y}} \circ
\overline{F_1} \circ G_1 \circ \overline{F_1}\inv \circ \overline{A_1}\inv
&\text{since $\ran(F_1) \subseteq A_1\pre{N_1\cup Y}$, by (a)}\cr
&= id_{\Sigma_1} \circ id_{N_1\cup Y} \circ \overline{A_1} \circ
\overline{F_1} \circ G_1 \circ \overline{F_1}\inv \circ \overline{A_1}\inv
&\cr
&= id_Y \circ \overline{A_1} \circ \overline{F_1} \circ G_1 \circ
\overline{F_1}\inv \circ \overline{A_1}\inv.
&\cr
}$$
By a similar argument,
$$ id_{\Sigma_1} \circ \overline{A_1} \circ G_{1H} \circ
\overline{S_1} \circ \overline{S_1}\inv \circ \overline{A_1}\inv
= id_Y \circ \overline{A_1} \circ
\overline{S_1} \circ G_1 \circ \overline{S_1}\inv \circ \overline{A_1}\inv. $$
Using these last three equations in (10),
$$ G_1 \circ id_Y
\subseteq id_Y \circ \bigl(
\overline{W_1} \circ G_{1N} \circ \overline{W_1}\inv \ \cup\
\overline{A_1} \circ
\overline{F_1} \circ G_1 \circ \overline{F_1}\inv \circ \overline{A_1}\inv
\ \cup\
\overline{A_1} \circ
\overline{S_1} \circ G_1 \circ \overline{S_1}\inv \circ \overline{A_1}\inv
\bigr). $$
Hence by theorem~4(vi)
$$ G_1 \circ id_Y \subseteq id_Y \circ G_1 $$
as required. \qed


\theorem 23. If $p:\N_1\to\N_0$ is a homomorphism from a network $\N_1=
\network{_1}$ satisfying

\item{(a)} $\forall X \subseteq\Sigma_1\ |P_1\pre X| - |G_{1N} \circ id_{P_1\pre
X}| \le |X|$,

\item{(b)} $E_1 \buildrel F_1 \over \rightarrow H_1 \buildrel S_1
\over \leftarrow E_1$ is a sum diagram in the category of sets,

\item{(c)} $\exists f:K_1\setdiff dom(G_1) \to K_1 \ G_{1K}\inv=\overline f$,

\item{(d)} $E_1 \doublearrow{A_1 \circ F_1}{A_1 \circ S_1} N_1\cup\Sigma_1
\buildrel W_1 \over \rightarrow \Sigma_1$ is a coequaliser diagram in the
category of sets,

\smallskip\f
to a semi-definite network $\N_0$, then $\N_1$ is definite.


\proof We shall use the usual notation, $\N_0=\network{_0}$.

First note that the hypotheses of theorem~21 and theorem~22 hold, taking $Y =
\Sigma_1$ (since $H_1 = A_1\pre{N_1\cup\Sigma_1}$), so we can apply these
theorems in what follows. In particular, theorem~22 gives
$$\eqqalignno\quad{
G_{1\Sigma}
&= G_1 \circ id_{\Sigma_1}
&\cr
&= \bigl( \overline{W_1} \circ G_{1N} \circ \overline{W_1}\inv \ \cup \
id_{\Sigma_1} \circ \overline{A_1} \circ G_{1H} \circ \overline{A_1}\inv \bigr)
\circ id_{\Sigma_1}
&\text{by theorem~22(ii)}\cr
&= \overline{W_1} \circ G_{1N} \circ \overline{W_1}\inv \circ id_{\Sigma_1}
\ \cup \
id_{\Sigma_1} \circ \overline{A_1} \circ G_{1H} \circ \overline{A_1}\inv
\circ id_{\Sigma_1}
&\cr
&= \overline{W_1} \circ G_{1N} \circ \overline{W_1}\inv
\ \cup \
id_{\Sigma_1} \circ \overline{A_1} \circ G_{1H} \circ \overline{A_1}\inv
&\text{by theorem~22(i)}\cr
}{(1)}$$
and theorem~21(i) gives
$$ G_{1H} = G_1 \circ id_{H_1}
= \overline{F_1} \circ G_{1E} \circ \overline{F_1}\inv \ \cup\
\overline{S_1} \circ G_{1E} \circ \overline{S_1}\inv.
\eqno (2) $$

Next we shall show that $G_{1N}$ is connected relative to $P_1$. We already know
the following.
$$\eqqalign\quad{
G_{1N} &\text{ is finite}
&\text{since $N_1$ is finite} \cr
G_{1N} \circ G_{1N} &\subseteq G_1 \circ G_1 = \bot
&\text{since $\N_1$ is a network} \cr
G_{1N} &\text{ is acyclic}
&\text{by theorem~21(vi)} \cr
\overline{P_1} \circ G_{1N} &\subseteq \overline{P_1} \circ G_1
\subseteq \overline{P_1}
&\text{since $\N_1$ is a network} \cr
\forall X \subseteq\Sigma_1\ |P_1\pre X| - |G_{1N} \circ id_{P_1\pre X}|
&\le |X|
&\text{by hypothesis (a)} \cr
}$$
So $G_{1N}$ is connected relative to $P_1$, by theorem~13(iii).

Next we shall show that $G_1$ is minimal relative to $\N_1$. We already know the
following.
$$\eqqalign\quad{
G_{1K} \circ G_{1K}\inv &\subseteq id_{K_1}
\subseteq G_{1K} \circ G_{1K}\inv \cup G_{1K}\inv \circ G_{1K}
&\text{by theorem~21(ii)} \cr
G_{1\Sigma} &= \overline{W_1} \circ G_{1N} \circ \overline{W_1}\inv \ \cup\
id_{\Sigma_1} \circ \overline{A_1} \circ G_{1H} \circ \overline{A_1}\inv
&\text{by (1)}\cr
G_{1N} &= id_{N_1} \circ \overline{A_1} \circ G_{1H} \circ \overline{A_1}\inv
&\text{by theorem~20(iii)} \cr
G_{1H} &= \overline{F_1} \circ G_{1E} \circ \overline{F_1}\inv \cup
\overline{S_1} \circ G_{1E} \circ \overline{S_1}\inv
&\text{by (2)} \cr
G_{1E} &= \overline{C_1} \circ G_{1K} \circ \overline{C_1}\inv
&\text{by theorem~20(iv)} \cr
}$$
Then $G_1$ is minimal relative to $\N_1$ by theorem~17.

Finally we shall check the conditions for $\N_1$ to be definite.
$$\eqqalign\quad{
&E_1 \doublearrow{A_1 \circ F_1}{A_1 \circ S_1} N_1\cup\Sigma_1 \buildrel W_1
\over \rightarrow \Sigma_1
\text{ is a coequaliser diagram}
&\text{by hypothesis (d)} \cr
&G_{1N} \text{ is connected relative to } P_1
&\text{as just shown} \cr
&G_{1N} \text{ is acyclic}
&\text{by theorem~21(vi)} \cr
&E_1 \buildrel F_1 \over \rightarrow H_1 \buildrel S_1 \over \leftarrow E_1
\text{ is a sum diagram}
&\text{by hypothesis (b)} \cr
&id_{K_1} = G_{1K} \circ G_{1K}\inv \cup G_{1K}\inv \circ G_{1K}
&\text{by theorem~21(ii)}\cr
&G_1 \text{ is minimal relative to $\N_1$}
&\text{as just shown} \cr
}$$
Thus $\N_1$ is definite. \qed




\subhead{3.7 Subnetworks}

\defn If $\N=\network{}$ is a network, a \i{subnetwork} of $\N$ is a 12-tuple
$\network{'}$, where

$\Sigma' \subseteq \Sigma, \quad N' \subseteq N, \quad H' \subseteq H, \quad E'
\subseteq E, \quad K' \subseteq K$

$W(N') \subseteq \Sigma', \quad P(N') \subseteq \Sigma', \quad H' =
A\pre{N'\cup\Sigma'}, \quad F(E') \subseteq H', \quad S(E') \subseteq H', \quad
K' = C\pre{E'}$

$W' = W|_{N'\cup\Sigma'}, \quad P' = P|_{N'}, \quad A' = A|_{H'}, \quad F' =
F|_{E'}, \quad S' = S|_{E'}, \quad C' = C|_{K'}$

$G \circ id_{\Sigma'\cup N'\cup H'\cup E' \cup K'} \subseteq id_{\Sigma'\cup
N'\cup H' \cup E' \cup K'} \circ G, \quad G' = id_{\Sigma'\cup N'\cup H' \cup E'
\cup K'} \circ G \circ id_{\Sigma'\cup N'\cup H'\cup E' \cup K'}$.

\medskip\f
A \i{proper} subnetwork of $\N$ is a subnetwork $\N'$ such that $\N'\ne\N$.


\theorem 24. If $\N=\network{}$ is a network and $\N'=\network{'}$ is a
subnetwork of $\N$ then

\item{(i)} $G' = G \circ id_{\Sigma'\cup N'\cup H' \cup E' \cup K'}$,

\item{(ii)} $\N'$ is a network,

\item{(iii)} $K'\setdiff\dom(G') \subseteq K\setdiff\dom(G)$,

\item{(iv)} the function $f:\Sigma'\cup N'\cup H'\cup E'\cup K' \to
\Sigma\cup N\cup H\cup E\cup K$ defined by $\forall
x\from\Sigma'\cup N'\cup H'\cup E'\cup K' \ f(x) = x$ is a homomorphism from
$\N'$ to $\N$, called the \i{inclusion homomorphism}.

\proof Define $I = id_{\Sigma'\cup N'\cup H' \cup E' \cup K'}$.

(i) By definition, $G' = I \circ G \circ I$, which equals $G \circ I$ by
$$ I \circ G \circ I \subseteq G \circ I = G \circ I \circ I
\subseteq I \circ G \circ I. $$

(ii) The conditions
$$ W(N') \subseteq \Sigma', \quad P(N') \subseteq \Sigma', \quad
H' = A\pre{N'\cup\Sigma'}, \quad F(E') \subseteq H', \quad
S(E') \subseteq H', \quad K' = C\pre{E'}, $$
together with $\forall \sigma\from\Sigma\ W(\sigma)=\sigma$, give us
$$ W':N'\cup\Sigma'\to\Sigma', \quad P':N'\to\Sigma', \quad
A':H'\to N'\cup\Sigma', \quad F',S':E'\to H', \quad C':K'\to E' $$
and $\forall \sigma\from\Sigma'\ W'(\sigma)=\sigma$. Note for later use that
these conditions can also be expressed in relation notation as
$$\eqalign{
\overline{W'} &= \overline W \circ I \subseteq I \circ \overline W, \quad
\overline{P'} = \overline P \circ I \subseteq I \circ \overline P, \quad
\overline{A'} = \overline A \circ I = I \circ \overline A, \cr
\overline{F'} &= \overline F \circ I \subseteq I \circ \overline F, \quad
\overline{S'} = \overline S \circ I \subseteq I \circ \overline S, \quad
\overline{C'} = \overline C \circ I = I \circ \overline C. 
}$$
Hence 
$$ I \circ \overline W \circ I \subseteq \overline W \circ I 
= \overline W \circ I \circ I \subseteq I \circ \overline W \circ I, $$
so $W' = \overline W \circ I = I \circ \overline W \circ I$.

Since $G' = I \circ G \circ I$, $G'$ is a relation on $\Sigma'\cup N'\cup H'\cup
E'\cup K'$.

To verify $id_{\Sigma'} \circ G' = G' \circ id_{\Sigma'}$:
$$ id_{\Sigma'} \circ G'
= id_{\Sigma'} \circ I \circ G \circ I
= I \circ id_\Sigma \circ G \circ I
= I \circ G \circ id_\Sigma \circ I
= I \circ G \circ I \circ id_{\Sigma'}
= G' \circ id_{\Sigma'} $$
and similarly for the conditions $id_{N'} \circ G' = G' \circ id_{N'}$, $id_{H'}
\circ G' = G' \circ id_{H'}$, $id_{E'} \circ G' = G' \circ id_{E'}$ and $id_{K'}
\circ G' = G' \circ id_{K'}$.

To verify that $G'$ preserves incidence:
$$ \overline{W'} \circ G'
= \overline W \circ I \circ G \circ I
= \overline W \circ G'
= \overline W \circ G \circ I
= G \circ \overline W \circ I 
= G \circ I \circ \overline W \circ I
= G' \circ \overline{W'} $$
and
$$ \overline{P'} \circ G'
= \overline P \circ I \circ G \circ I
= \overline P \circ G'
= \overline P \circ G \circ I
\subseteq \overline P \circ I
= \overline{P'} $$
and
$$ \overline{F'} \circ G'
= \overline F \circ I \circ G \circ I
= \overline F \circ G'
= \overline F \circ G \circ I
\subseteq G \circ \overline F \circ I
= G \circ \overline F \circ I \circ I
\subseteq G \circ I \circ \overline F \circ I
= G' \circ \overline{F'} $$
and similarly for the conditions for $A$, $S$ and $C$.

Next we verify the minimality conditions. We have
$$\eqqalign\quad{
\overline{A'}\inv \circ \overline{A'} \ \cap\ G'_H \circ {G'}_H\inv
&= id_{H'} \circ \overline A\inv \circ \overline A \circ id_{H'} \ \cap\
G'_H \circ {G'}_H\inv
&\cr
&= id_{H'} \circ \bigl( \overline A\inv \circ \overline A \ \cap\
G'_H \circ {G'}_H\inv \bigr) \circ id_{H'}
&\text{by theorem~4(iii),(iv)}\cr
&\subseteq id_{H'} \circ \bigl( \overline A\inv \circ \overline A \ \cap\
G_H \circ G_H\inv \bigr) \circ id_{H'}
&\cr
&\subseteq id_{H'} \circ id_H \circ id_{H'}
&\text{by theorem~14}\cr
&= id_{H'}
&\cr
}$$
so by theorem~14 $G'_H$ is minimal relative to $A'$. The other minimality
conditions follow similarly.

For the final condition, $G' \circ G' \subseteq G \circ G = \bot$.

(iii) Using $G' = G \circ I$,
$$ \dom(G') \cap K' = \dom(G' \circ id_{K'}) = \dom(G \circ I \circ id_{K'})
= \dom(G \circ id_{K'}) = \dom(G) \cap K' $$
so $K' \setdiff \dom(G') = K' \setdiff \dom(G) \subseteq K \setdiff \dom(G)$, as
required.

(iv) The conditions
$$ f(\Sigma') \subseteq \Sigma, \quad f(N') \subseteq N, \quad
f(H') \subseteq H, \quad f(E') \subseteq E, \quad f(K') \subseteq
K $$
are immediate, as are
$$ W \circ f = f \circ W', \quad P \circ f = f \circ P', \quad
F \circ f = f \circ F', \quad S \circ f = f \circ S'. $$

The pullback $\bigrectangleA{N\cup\Sigma}{N'\cup\Sigma'}{H}{H'}
{f|_{N'\cup\Sigma'}}{A}{A'}{f|_{H'}}$ is verified as follows. First, $A \circ
f|_{H'} = A|_{H'} = A' = f|_{N'\cup\Sigma'} \circ A'$. Secondly, given any set
$X$ and functions $p:X\to H$ and $q:X\to N'\cup\Sigma'$ such that $A \circ p =
f|_{N'\cup\Sigma'} \circ q$, this means $A \circ p = q$, so $A(p(X)) \subseteq
N'\cup\Sigma'$, so $p(X) \subseteq A\pre{N'\cup\Sigma'} = H'$, so $p: X \to H'$
and $A' \circ p = q$, so there exists a unique function $i:X \to H'$ such that
$f|_{H'} \circ i = p$ and $A' \circ i = q$, namely $i = p$.

The pullback $\rectangleA{E}{E'}{K}{K'}{f|_{E'}}{C}{C'}{f|_{K'}}$ is verified
similarly.

Note that $\overline f = I$, and so, using $G' = G \circ I = I \circ G \circ I$,
$$ \overline f \circ G'
= I \circ G \circ I
= G \circ I
= G \circ \overline f $$
as required.

To verify that $G'$ is minimal relative to $f$, consider any relation $R
\subseteq G'$ such that $\overline f \circ R = \overline f \circ G'$. Now, $G'$
is on $\Sigma'\cup N'\cup H'\cup E'\cup K'$ and therefore so is $R$. Hence $R =
I \circ R = \overline f \circ R = \overline f \circ G' = I \circ G' = G'$, as
required. \qed


\defn If $\N'=\network{'}$ is a subnetwork of $\N$, with inclusion
homomorphism $f:\N'\to\N$, the \i{restriction} of a homomorphism $p:\N\to\N^*$
to $\N'$, denoted $p|_{\N'}:\N'\to\N^*$, is defined as $p \circ f =
p|_{\Sigma'\cup N'\cup H'\cup E'\cup K'}$; this is a homomorphism by theorem~15.


\subhead{3.8 The recognition problem and process (initial statement)}
A grammar and a pattern are both represented as networks. Given a semi-definite
network $\N_0$ (representing a grammar) and an image, the recognition problem is
to construct a definite network $\N_1$ (representing a pattern) and a
homomorphism $p:\N_1\to\N_0$ (called the \i{parse}). (This statement will be 
refined in \S4.7.)

The pattern is constructed by a process of successive extension, pruning,
merging and partitioning; the pattern is not definite during this process but
at the end the hypotheses of theorem~23 are satisfied and so the pattern is
definite.
